# Supplementary material for: COVID-19 incidence in the Republic of Ireland: A case study for network-based time series models
Source: arXiv:2307.06199 source file (2024-06-05)
Supplement: Supplementary file 1 [file Discussion.tex]

\section{Discussion}
\label{chapter: discussion}
\as{Do we require a summary of the claims of the paper in the discussion and the conclusion part? Would it make sense to merge the two?}

% In this paper, we modelled the COVID-19 incidence across the 26 counties in the Republic of Ireland by fitting GNAR models, leveraging different networks to represent spatial dependence between the counties. 
% These models can be used for predictions.
% We found that the GNAR model have higher predictive accuracy on data collected during pandemic phases with inter-county movement restrictions than data gathered during less restricted phases.
% Sparse networks perform better for the restricted data set, while denser networks achieve lower BIC for the unrestricted data set, \as{Not sure if this really implies the following conclusion: implying higher spatial correlation in COVID-19 incidence during pandemic periods with fewer restrictions.}

A key challenge for modelling is that COVID data is characterised by high uncertainty e.g due to testing hesitancy, low testing capacity and double counting \cite{bertozzi2020challenges, HPSC_covid_report_2020/21, ioannidis2020forecasting}. 
In general, such uncertainty is typical for data of spreads of epidemics \cite{wang2022prediction}.
For COVID-19 in particular, incidence data is extremely erratic due to its tendency for fast and sudden local outbreaks and due to many unreported cases \cite{li2020substantial, IE_timeline_pandemic}. 
In our analysis, the Queen's contiguity network best captured the restrictive phase. 
Intuitively, this network allows travel across county borders via any means possible. 
During the restricted phase, adding information about the nearest economic hub did not increase the model fit. 
In contrast, in the unrestricted phase the best-fitting model was a 21-nearest neighbour model, indicating almost, but not quite, homogeneous mixing across all of Ireland.
\as{As the model performance showed only small differences across networks, we refrain from further interpretation of the networks.}

The ARIMA models require a large number of parameters compared to s.
The global-$\alpha$ GNAR model outperforms the county-specific ARIMA models in predictive accuracy and model parsimony. 
High dimensionality in model coefficients can result in high instability in the form of large standard deviation \cite{zhou2020network}. 
In GNAR models, the model parametrisation relies on the underlying networks, guaranteeing parsimonious models and providing inherent parameter dimensionality reduction \cite{zhou2020network}. 
Moreover, the GNAR model is able to capture joint effects by modelling the evolution of the time series in all counties simultaneously.
The parameter estimates for the GNAR model are consistent and asymptotically Gaussian under Gaussian error \footnote{For the Gaussian assumption, consistency and asymptotic normality follow easily from the equivalence between the EGLS estimator and Maximum Likelihood estimator \cite{Lutkepohl1991Itmt}.}.
For more complex continuous error structures, computationally more intensive approaches, such as the Newton-Raphson method \cite{MyersRaymondH2002Glm:} or the Iteratively Reweighted Least Squares method \cite{HastieTrevor2009Teos}, ensure consistency and correct inference.  
In light of the discrete nature of the COVID-19 case counts and the challenge of structural misreporting, alternative error structures, e.g.\,according to a Poisson process, are plausible \cite{rehms2022bayesian}.
To the best of our knowledge, methods to estimate model coefficients while assuming such error structures in the context of GNAR models have not yet been developed.

% \subsection{Interpreting the model fit}
% The fitted GNAR models have different coefficients for the restricted and for the unrestricted phase.
% The effect of COVID-19 restrictions is not systematically detectable in the $\beta$-order, e.g.\,restricting inter-county travel leading to lower stage neighbourhoods or even $\beta = 0$. 
% % The effectiveness of restrictions can also not be verified in the development of the $\beta$-coefficients for the best performing model across restrictions.
% However, the change of restrictions is reflected in the change in values of the $\alpha$- and $\beta$-order coefficients in the subset-specific models. 
% The modelling approach should depend on the research question; this study focuses on prediction.
% There are alternative COVID-19 models available which are tailored to capture the effectiveness of COVID-19 regulations without taking the network effect into account, see e.g.\,\cite{bertozzi2020challenges, flaxman2020estimating, gabler2022effectiveness}. 

% The best performing GNAR models have larger $\alpha$- and $\beta$-order, than the GNAR models commonly implemented, e.g.\,in \cite{knight2019generalised, knight2016modelling, urrutia2022sars}.
% It is possible that the higher orders hint at stronger temporal and spatial dependence. 
% The fitted GNAR models benefit from leveraging values further back in history as well as the historic values of neighbours.
% The spatial dependence decreases over time, leading to smaller stage neighbourhoods for larger lags.   

For model selection, the differences in BIC and tend to be larger than the differences in MASE regarding the comparison between GNAR and ARIMA model and may not select the exact same model.
This observation emphasises the importance of choosing a criterion for model selection which corresponds to the desired task. 
To predict the COVID-19 incidence, the MASE contains more information to assess model accuracy. 
The BIC value weighs the likelihood of the data given a certain parametrisation of the GNAR model %up 
against the number of parameters fitted in the model. 
The BIC computation in the GNAR package assumes the error term, and hence $X_t$, to be Gaussian \cite{source_code_GNAR}. 
As detailed in Section \ref{chapter: phases}, we could not validate this assumption for the unrestricted phase and the deviation from the assumption might explain the poor performance of the BIC in identifying models with high predictive accuracy.
