# Supplementary material for: COVID-19 incidence in the Republic of Ireland: A case study for network-based time series models
Source: arXiv:2307.06199 source file (2024-06-05)
Supplement: Supplementary file 2 [file FULL_LitRev.tex]

\section{Definitions and a short introduction to Time Series Analysis}
\label{app:definition}
The temporal relationship within a time series is measured by the \textit{autocovariance} (or \textit{autocorrelation}), i.e. the covariance (or correlation) between $X_{t_1}$ and $X_{t_2}$ at some time points $t_1$ and $t_2$, observed for the same statistical unit (w.l.o.g. $t_1 < t_2$),
\begin{align*}
    AC(X_{t_1}, X_{t_2}) & = \mathbb{C}ov(X_{t_1}, X_{t_2}) \\
    & = \mathbb{E}\left( (X_{t_1} - \mu) (X_{t_2} - \mu) \right) \\
    ACor(X_{t_1}, X_{t_2}) & = \mathbb{C}orr(X_{t_1}, X_{t_2}) \\
    & = \frac{\mathbb{E}\left( (X_{t_1} - \mu) (X_{t_2} - \mu) \right)}{\sqrt{\mathbb{V}(X_{t_1})} \sqrt{\mathbb{V}(X_{t_2})}} \; .
\end{align*}

\textit{Stationarity} implies that, as time progresses, the distribution of the observations converges to a certain distribution, i.e. is independent of time.  \\
\textit{Weak stationarity} or \textit{Covariance-stationarity} is defined by a time-independent, constant mean and a time-independent covariance whose values only depends on the size of the lag $k$, not on time $t$ \cite{HamiltonJamesDouglas2020TSAe}, $\forall t \in \{1, ..., T\}, k \in \{0, ..., T-t \}$
\begin{align*}
    \mathbb{E}(X_t) & = \mu  \\
    \mathbb{C}ov(X_t, X_{t + k}) & = \gamma_k \; .
\end{align*}
A weakly stationary time series is symmetric, in the sense that due to the time-independence and symmetry of the covariance, 
\begin{align}
\label{equ:symmetry_covariance}
    \gamma_k & = \mathbb{C}ov(X_t, X_{t+k}) \\
    &  = \mathbb{C}ov(X_{t-k}, X_{(t - k) + k}) \\
    & = \mathbb{C}ov(X_t, X_{t-k}) \\
    & = \gamma_{-k} \; .
\end{align}

A time series is \textit{strictly stationary} if the joint distribution for $(X_t, X_{t + k_1}, ..., X_{t + k_n})$ is independent of time $t$ and only depends on the time intervals $k_i$ between subsequent observations \cite{wei2006time}. \\
% Weak stationarity follows from strict stationarity if the second moment is finite \cite{wei2006time}. 

\section{Literature review for network-based time series models}
\label{app:lit_rev_network_models}
Network time series models expand multivariate time series by incorporating non-temporal dependencies.
Such dependencies are represented by a network.
An edge indicates a certain relationship between the variables which are represented by the two vertices.  
The output variable at each vertex is modelled to depend on its own past values as well as the past values of its neighbouring vertices which are determined by the network underlying the model.
A myriad of methods for multivariate time series analysis exist \cite{HamiltonJamesDouglas2020TSAe}. \\
\\
\noindent \textbf{Spatial Autoregressive and Moving Average models} \\
% - spatial moving average: Ord 1975, Mur 1999
\cite{ord1975estimation} developed the \textit{spatial autoregressive(-regressive) model} (SAR).
$X_i$ denotes the weighted average across the location set $J(i)$. 
The location set includes any vertices to which vertex $i$ has some relationship. 
\begin{align}
\label{equ:ar_ord}
    X_{i} = \beta_0 + \rho \sum_{j \in J(i)} \omega_{i, j} X_{j} + \varepsilon_{i} \; .
\end{align}
The weights $\omega_{ij}$ are non-negative and by convention we do not regress $X_i$ onto itself, i.e. $\omega_{ii} = 0$. 
The model (\ref{equ:ar_ord}) can be expanded to a \textit{mixed regressive-autoregressive model} which incorporates exogenous variables $Y$. \\
For matrices $X = [X_i^T]_{i = 1}^N$, $W = [\omega_{i, j}]_{i,j = 1}^N$ and $\varepsilon = (\varepsilon_1, ..., \varepsilon_N)$, 
\begin{align*}
    X = Y \beta + \rho W X + \varepsilon \; .
\end{align*}
\cite{doreian1981estimating} utilises this model to account for "the geography of social phenomena" (\cite{doreian1981estimating}, p. 359-360). 
The relevance of modeling spatial dependence is determined either by conceptual deliberation or by a statistical test for spatial autocorrelation \cite{doreian1981estimating}. \\
\cite{ord1975estimation} also introduces an alternative model relying on autoregression in the error term, 
\begin{align*}
    X = Y \beta + \varepsilon \\
    \varepsilon = \rho W X + \nu \; .
\end{align*}
\cite{mur1999testing} introduces spatial equivalents to the MA and \code{ARIMA} models.
A \textit{spatial moving average model} (SMA) describes $X_{i, t}$ as a weighted average of spatially related error terms.
\begin{align}
\label{equ:ma_mur}
    X_{i, t} = \varepsilon_t + \sum_{j = 1}^N \theta_j \varepsilon_{j, t} \; .
\end{align}
By convention, $\theta_i = 0$. 

Combining (\ref{equ:ar_ord}) and (\ref{equ:ma_mur}) obtains a \textit{spatial autoregressive moving average model} (SARMA) (\cite{mur1999testing}).  \\
The essential - and novel - component of network autoregressive models is the weight matrix $W$ which encodes the spatial dependencies. 
Ideally, "W is supposed to represent the theory a researcher has about the structure of the influence processes in the network" (\cite{leenders2002modeling}, p. 22). 
SAR and SMA models have been - under varying names - explored in numerous papers (e.g.\,\cite{doreian1980linear},  \cite{white1981sexual}, \cite{dow1982network}, \cite{loftin1983spatial}, \cite{doreian1989models} and \cite{doreian1989network}).
All above mentioned models do not rely on time, i.e. they are applicable to any ordering, and require Gaussian error term with homoscedastic variance.  
Additionally, they are restricted to lag 0 and do not acknowledge any temporal dependence into account \cite{leeming2019new}. \\
\\
\textbf{m-STAR model} \\
The \textit{m-STAR model} by \cite{hays2010spatial} is a spatiotemporal model which includes estimating the weight matrix $\hat{W} = \sum_{c = 1}^C \rho_c [\omega_{i, j, c}^{(t)}]_{i, j = 1}^N$,  
\begin{align*}
    X_{i, t} = Y_i^T \beta + \alpha X_{i, t-1} + \sum_{j = 1}^N \sum_{c = 1}^C \rho_c \omega_{i, j, c}^{(t)} X_{j, t} + \varepsilon_{i, t} 
\end{align*}
where $Y_i$ are vertex-specific exogenous variables. \\
The error term is iid.\,Gaussian and the model is restricted to 1-lag autoregression.
The $C$ sets of spatial weights represent network interdependence between vertices on different contextual levels, i.e. geographic proximity, EU co-membership and economic interdependence for modelling active labour market policies \cite{hays2010spatial}.
The great benefit of the m-STAR model is its "simultaneous estimation of net interdependencies and the effects of those interdependencies" (\cite{hays2010spatial}, p. 425). \\
\\
\noindent \textbf{STCAR model} \\
The \textit{spatial temporal conditional autoregressive model} (STCAR) is a continuous Markov random field with a Gaussian conditional probability density function.
Its distributions rely on a space-time autoregressive matrix which accounts for both spatial and temporal dependencies. 
Based on the autoregressive matrix, the parameters for the spatial and temporal relationship are computed via Maximum-Likelihood and Weighted Least Squares. 
A Gibbs sampler is applied to sample from the conditional probability density function.
STCAR models acknowledge spatial distance between vertices when determining the influence of vertices on another \cite{mariella2010spatial}. 
In general, it is possible to model spatial dependence by Markov random fields in combination with a network component (e.g.\,on genetics data in \cite{wei2007markov}). \\
\\
\noindent \textbf{Vector autoregression models} \\
A popular model choice is a \textit{vector autoregression model} (VAR). 
A VAR model regresses a vector at time $t \in \{1, ..., T\}$ on its values at previous time points.  \\
For a $p^{th}$-order Gaussian autoregression model, let $\mathcal{X} = \{ X_t \}_{t = 1}^T$ denote a network time series, where $X_t \in \mathbb{R}^n$ is vector summarising the values for all $n$ vertices on the network.
For $i \in \mathcal{V}$ and time $t$ , 
\begin{align}
\label{equ:var}
    X_{i, t} = \beta_0 + \sum_{i = 1}^p \beta_i X_{t-i} + \varepsilon_{t}
\end{align}
where $\varepsilon_t \sim N(0, \Omega)$. \\
The Maximum Likelihood estimates for $\beta$ are computed according to an Ordinary Least Squares (OLS) regression with input variables $X_{t-p}, ..., X_{t-1}$ and an intercept $\beta_0$\footnote{Proof in \cite{HamiltonJamesDouglas2020TSAe}, Chapter 11, p. 294}.
Equivalently to structural equation models, non-existent edges imply $\beta_{i, j} = 0$ \cite{HamiltonJamesDouglas2020TSAe}.
The likelihood for $\mathcal{X} = (X_1, ..., X_T)$ across time is the product of the conditional likelihoods, 
\begin{align*}
    p(\mathcal{X}) = \prod_{t = 1}^T p(X_t | X_{t-1}, ..., X_{t-p}) \; .
\end{align*}
For $t < p$, non-existent X are dropped in the condition. 
For $t = 1$, an initial distribution is assumed, $p(X_1) = \mu(X_1)$. 
The number of parameters to estimate is large and hence the order of VAR is restricted by the size of the data set \cite{leeming2019new}, \cite{jiang2020autoregressive}. 
Theoretical deliberations on how observations across time depend on each other impose restrictions on (\ref{equ:var}). \\
\\
\noindent \textbf{1-stage network autoregression model with exogenous variables} \\
\cite{zhu2017network} established a similar model, the \textit{network autoregression model}.
It includes an intercept and exogenous variables while being restricted to lag 1. 
Network autoregression stands in tradition with SMA and SAR models but incorporate historic values of the vertex in question and its $1^{st}$-stage neighbourhood. 
$A = [a_{ij}]_{i, j = 1}^N$ denotes the adjacency matrix. 
\begin{align}
\label{equ:zhu_ar}
    X_{i, t} = \beta_0 + Y_i^T \gamma + \beta_1 \cdot \frac{1}{n_i} \sum_{j = 1}^N a_{ij} X_{j, t-1} + \beta_2 X_{i, t-1} + \varepsilon_{i, t} \; .
\end{align}
The regression coefficients are constant across neighbour and vertices.
The effect can be distinguished between the nodal impact, $\beta_0 + Z_i^T \gamma$, and the network effect, $\beta_1$. 
The latter is assumed to be homogeneous across vertices. 
The model is only applicable for continuous data on a static network.
If the network is only observed partially, the model estimates suffer from bias \cite{zhu2017network}. 
To ensure less sensitivity to outliers in the data and incorporate heteroscedasticity, the paper \cite{zhu2019network} expanded the model to \textit{network quantile autoregression} \cite{zhu2019network}. 
The paper \cite{zhu2020grouped} further develops the \textit{grouped network autoregressive model} (groupNAR)\footnote{The paper \cite{zhu2020grouped} uses the abbreviation "GNAR". To avoid misunderstandings, we refer to the grouped network autoregressive model from \cite{zhu2020grouped} as "groupNAR" and to the model by \cite{knight2016modelling} as "GNAR".} which breaks the homogeneity by attributing each vertex to a group and estimating group-specific coefficients.   
We introduce the latent variable $z_i \in \{1, ..., C \}$ which denotes the class of vertex i and the indicator variable,
\begin{align*}
    \mathbb{I}_c(z_i) = \begin{cases}
    1 & \text{if } z_i = c \\
    0 & \text{otherwise} \; .
    \end{cases}
\end{align*}

\begin{align}
\label{equ:zhou_gnar}
    X_{i, t} = \sum_{c = 1}^C \mathbb{I}_c(z_{i}) \cdot \left( \beta_{0, c} + Y_i^T \gamma_c + \beta_{1, c} \cdot \frac{1}{n_i} \sum_{j = 1}^N a_{ij} X_{j, t-1} + \beta_{2, c} X_{i, t-1} + \sigma_c \varepsilon_{i, t} \right)
\end{align}
where $\varepsilon_{i, t} \sim N(0, 1)$. 
Due to the multiplication with the indicator variable, the parameters are considered random. 
This as well as the heterogeneous effect for each individual vertex "makes the [groupNAR] model [...] more flexible and realistic" (\cite{zhu2020grouped}, p. 1441).
The groupNAR(p) model incorporates values further back in history. 
\begin{align}
\label{equ:zhou_gnar_p}
    X_{i, t} = \sum_{c = 1}^C \mathbb{I}_c(z_{i}) \cdot \left\{ \sum_{k = 1}^p \left( \beta_{0, c}^{(k)} + \beta_{1, c}^{(k)} \cdot \frac{1}{n_i} \sum_{j = 1}^N a_{ij} X_{j, t-k} + \beta_{2, c}^{(k)} X_{i, t-k} \right) + Y_i^T \gamma_c + \sigma_c \varepsilon_{i, t} \right\} \; .
\end{align}
The classification of the vertices is learned simultaneously with the parameter estimation.
The number of classes has to be pre-specified \cite{zhu2020grouped}. \\
\\
\noindent \textbf{Network autoregression model} \\
Similarly to the 1-stage network autoregressive model, the network autoregression model \code{NAR(p,s)} includes historic values of the observation itself as well as its neighbours. 
However, we are not limited to 1 lag and the $1^{st}$-stage neighbourhood. 
In its plain form, the NAR model does not incorporate any exogenous variables.
The NAR(p, s) model is determined by two parameters: the scalar $p \in \mathbb{N}$, indicating the order or lag of the model, and the neighbourhood stage vector $s \in \mathbb{N}_0^p$, indicating the maximum neighbourhood stage %we include 
in the model. 
The $r^{\,th}$-stage neighbourhood must never be empty $\forall i \in \mathcal{V}$, imposing an indirect restriction on the choice of $s$ \cite{knight2019generalised}.
The current value $X_{i, t}$ is modelled as a autoregressive component, i.e. the sum of its own past values, and the sum  of past values for neighbouring vertices. %\\
The model for one vertex $i$ at time $t$ is then
\begin{align}
\label{equ:NAR}
    X_{i, t} = \sum_{j = 1}^p \left( \alpha_j X_{i, t-j} + \sum_{r = 1}^{s_j} \sum_{q \in N^{(r)}(i)} \beta_{j, r} X_{q, t-j} \right) + \varepsilon_{i, t} 
\end{align}
where $\varepsilon_{i, t} \sim N(0, \sigma^2)$ are taken to be independent and identically distributed (iid).
The model assumes stationarity and spatial network homogeneity, since $\beta_{j, r}$ depends on neither time $t$, nor on vertex $i$ or on $q$.  \\
\\
\noindent \textbf{Network integrated moving average model} \\
The \textit{network autoregressive (integrated) moving average model} (NARIMA) resemble restricted vector autoregressive (VAR) models but apply to the model parametrisation directly due to the underlying network the restrictions \cite{knight2019generalised}, \cite{knight2016modelling}.
NARIMA models facilitate dimensionality reduction\footnote{It reduces the computational complexity for calculating model coefficients from $\mathcal{O}(n^2)$ for VAR models to $\mathcal{O}(n)$ for NARIMA models.} and allow great flexibility in modelling spatial and temporal dependencies \cite{leeming2019new}, \cite{knight2019generalised}. \\
A NARIMA model consists of a NAR component, $X_t$, and a moving average component of order q (\code{MA(q)}), $\sum_{l = 1}^q \eta_l \varepsilon_{i, t-l}$ 
\begin{align}
\label{equ:NARMA}
X_{i, t} = \sum_{j = 1}^p \left( \alpha_j X_{i, t-j} + \sum_{r = 1}^{s_j} \sum_{q \in N^{(r)}(i)} \beta_{j, r} X_{q, t-j} \right) + \sum_{l = 1}^q \eta_l \varepsilon_{i, t-l} + \varepsilon_{i, t} \; .
\end{align}
% The coefficients are symmetrical, i.e. $\beta_{j, r, q} = \beta_{i, r, q}$. 
% A sufficient condition for \textit{weak stationarity} in a \code{NARIMA(p,q)} model is\footnote{Proof in \cite{knight2019generalised}, p. 32-34}
% \begin{align*}
%     \sum_{j = 1}^p \left( |\alpha_j| + \sum_{r = 1}^{s_j} \sum_{q \in N^{(r)}(i)} |\beta_{j, r, q}| \right) < 1 \; \; \forall i \in \mathcal{V} \; .
% \end{align*}
The relevance of vertices is acknowledged by vertex-specific weights \cite{knight2016modelling}.
The choice of weights strongly depends on the scenario and content the model is applied to \cite{leenders2002modeling}.
\begin{align}
\label{equ:NARMA_weighted}
X_{i, t} = \sum_{j = 1}^p \left( \alpha_j X_{i, t-j} + \sum_{r = 1}^{s_j} \sum_{q \in N^{(r)}(i)} \beta_{j, r} \omega_{i, q} X_{q, t-j} \right) + \sum_{l = 1}^q \eta_l \varepsilon_{i, t-l} + \varepsilon_{i, t} \; .
\end{align}

The gNARIMA model generalises (\ref{equ:NARMA}) by incorporating time dependent weights $\omega_{i, q, t}$ such that "nodes can drop-out and reappear" (\cite{knight2016modelling}, p. 6). 
All above models do not incorporate any exogenous variables and can only integrate one network \cite{knight2016modelling}, \cite{leeming2019new}.
