# Supplementary material for: COVID-19 incidence in the Republic of Ireland: A case study for network-based time series models
Source: arXiv:2307.06199 source file (2024-06-05)
Supplement: Supplementary file 3 [file GNAR_subsets.tex]

\section{GNAR models for subsets}
The decrease in inter-county dependence due to COVID-19 restrictions in theory should results in decreasing values for the $\beta$-coefficients in the GNAR model. 
This hypothesis cannot be verified when fitting the GNAR model which performed best for each network on the entire data set to each data subset (see Figures \ref{fig:parameter_delaunay} and in the Supplementary Material  \ref{app:development_coefficients}). 
We cannot detect a systematic decrease in $\beta$-coefficient for the first and second regulation (country-specific lockdowns and Level-5 lockdown). 
However, a pattern in absolute values is visible.  
During phases with strict mobility limitations, i.e. dataset 1 and 3, the coefficients lie closer to zero, while during periods of lenient or no restrictions, the $\beta$-coefficients are larger in absolute value.
The change in $\alpha$-coefficients behaves very similar across networks and in accordance with the pattern observed for the $\beta$-coefficients. 
For dataset 1, 3 and 5 the COVID-19 ID seems more erratic and less temporally dependent on historic values.
For the extremely restrictive Level-5 lockdown, the 1-lag historic values is most influential. 
\begin{figure}[h!]
\centering
\begin{subfigure}{\textwidth}
  \centering
  \includegraphics[width = 0.7\textwidth]{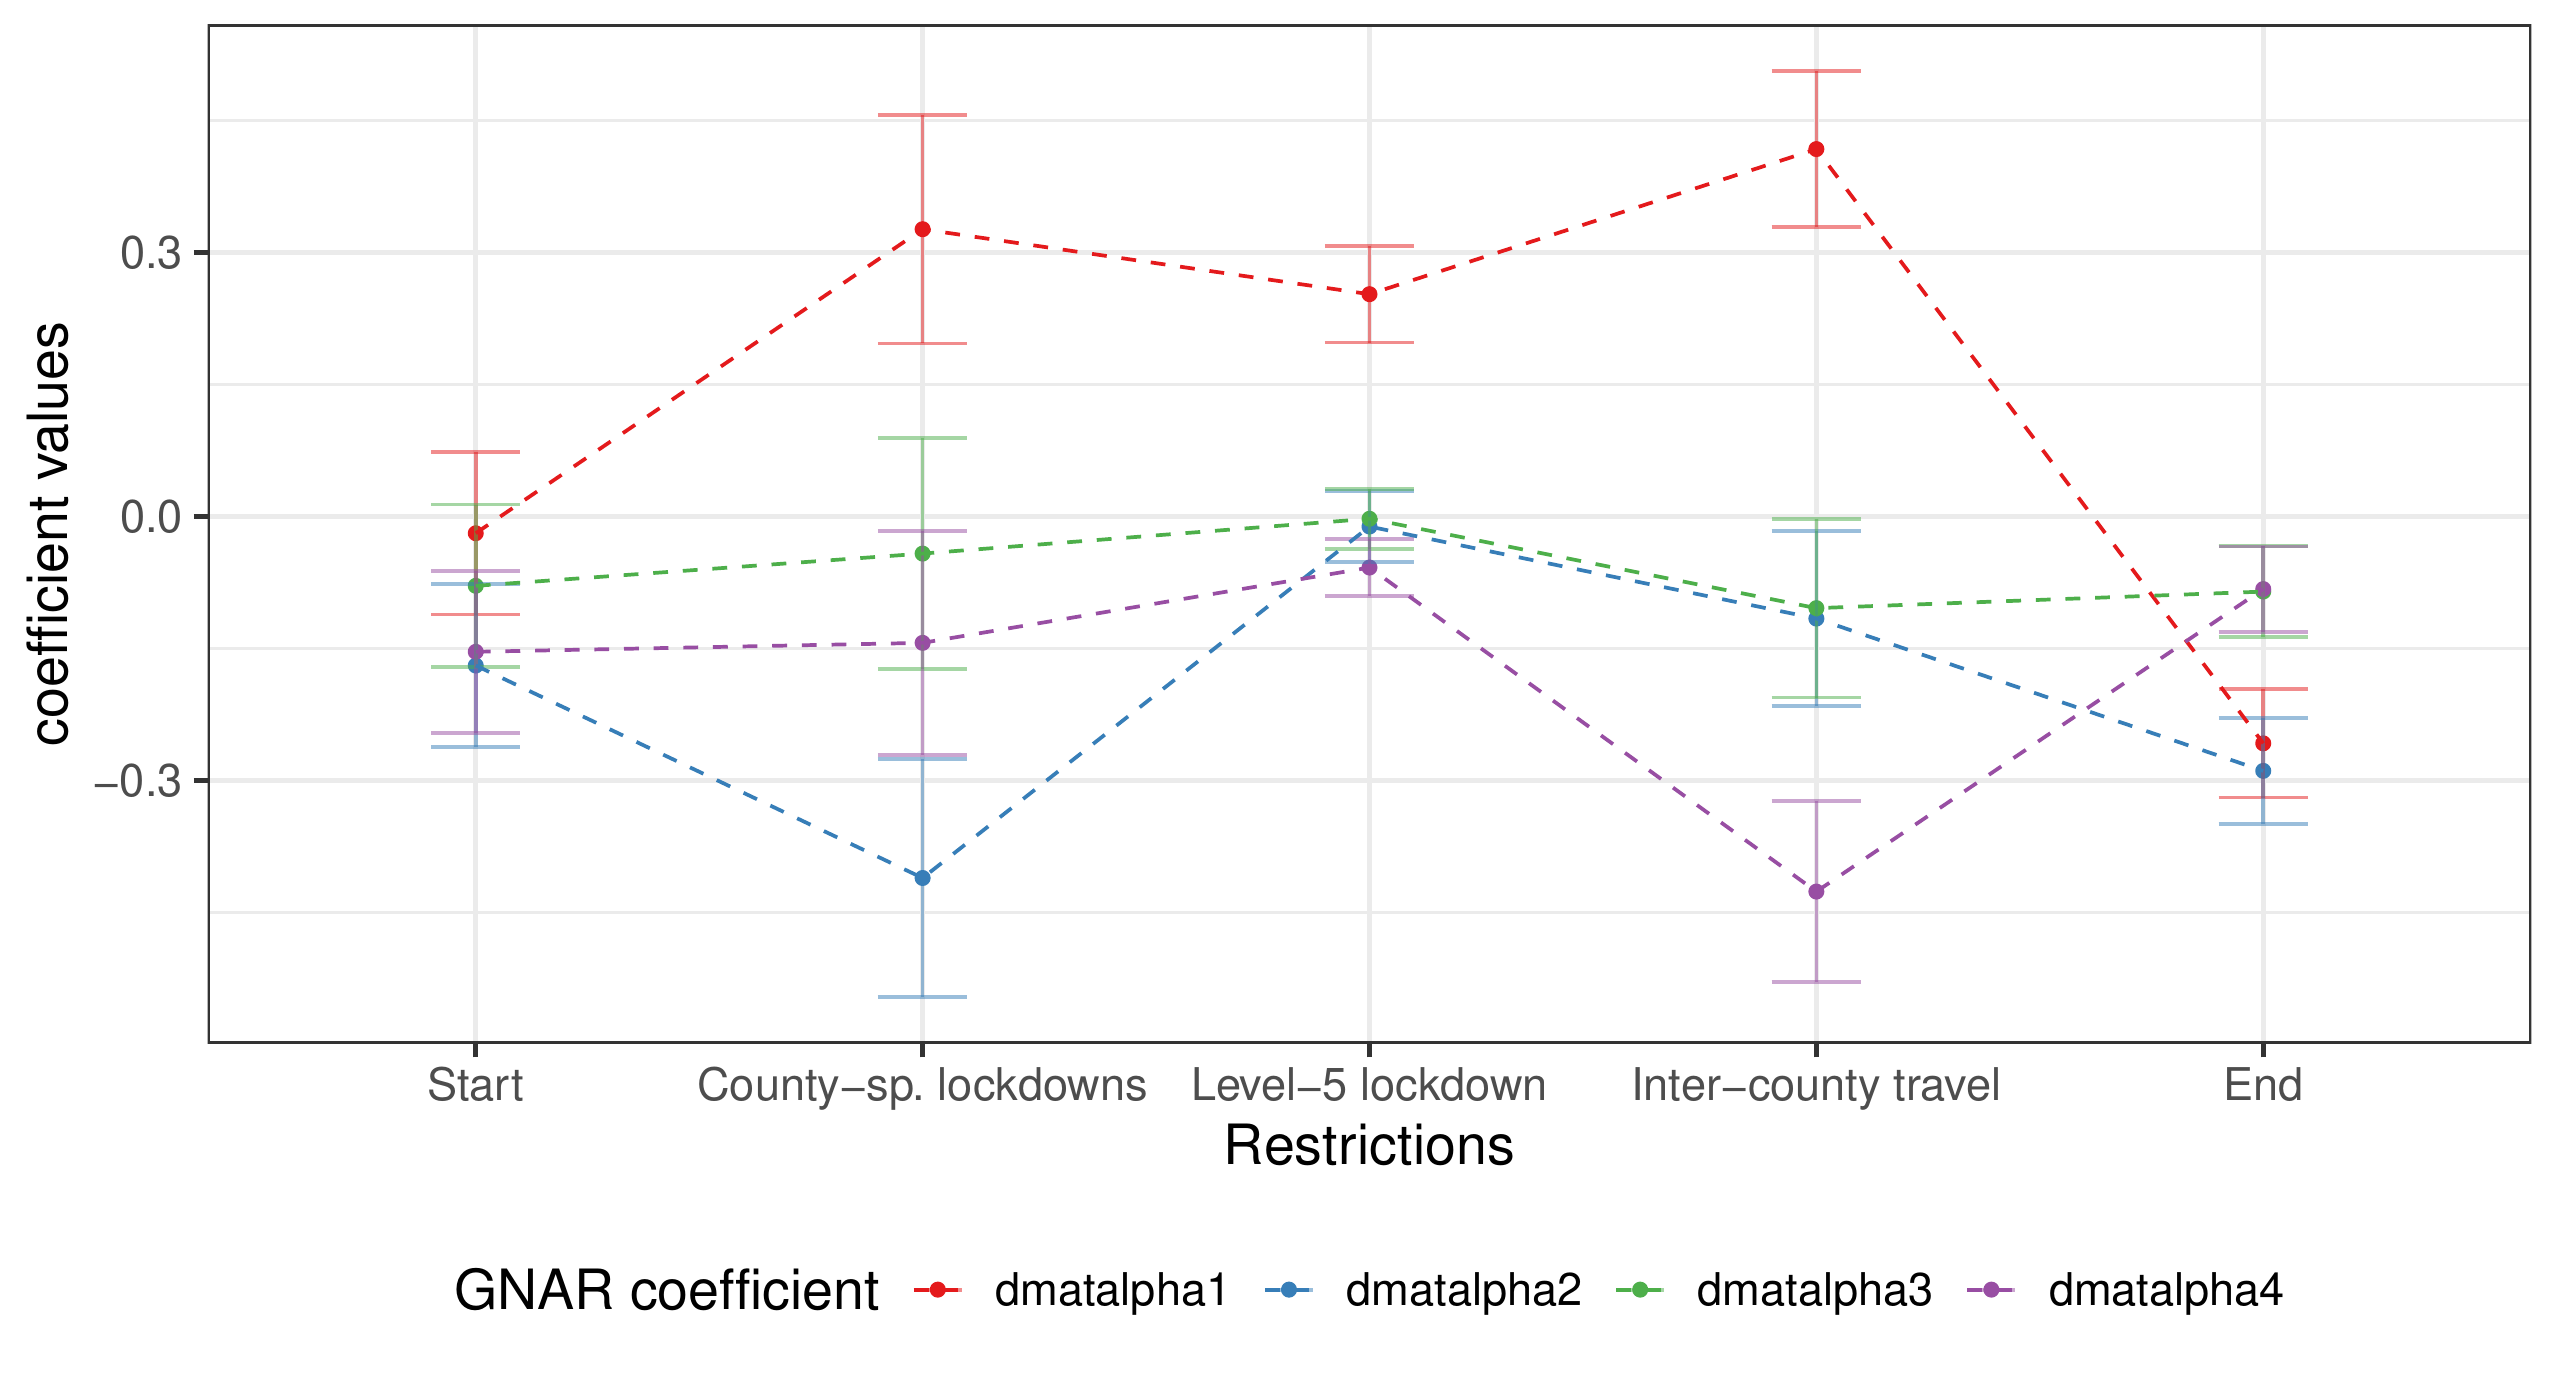}
  \caption{$\alpha$-order}
\end{subfigure}
\begin{subfigure}{\textwidth}
  \centering
  \includegraphics[width = 0.7\textwidth]{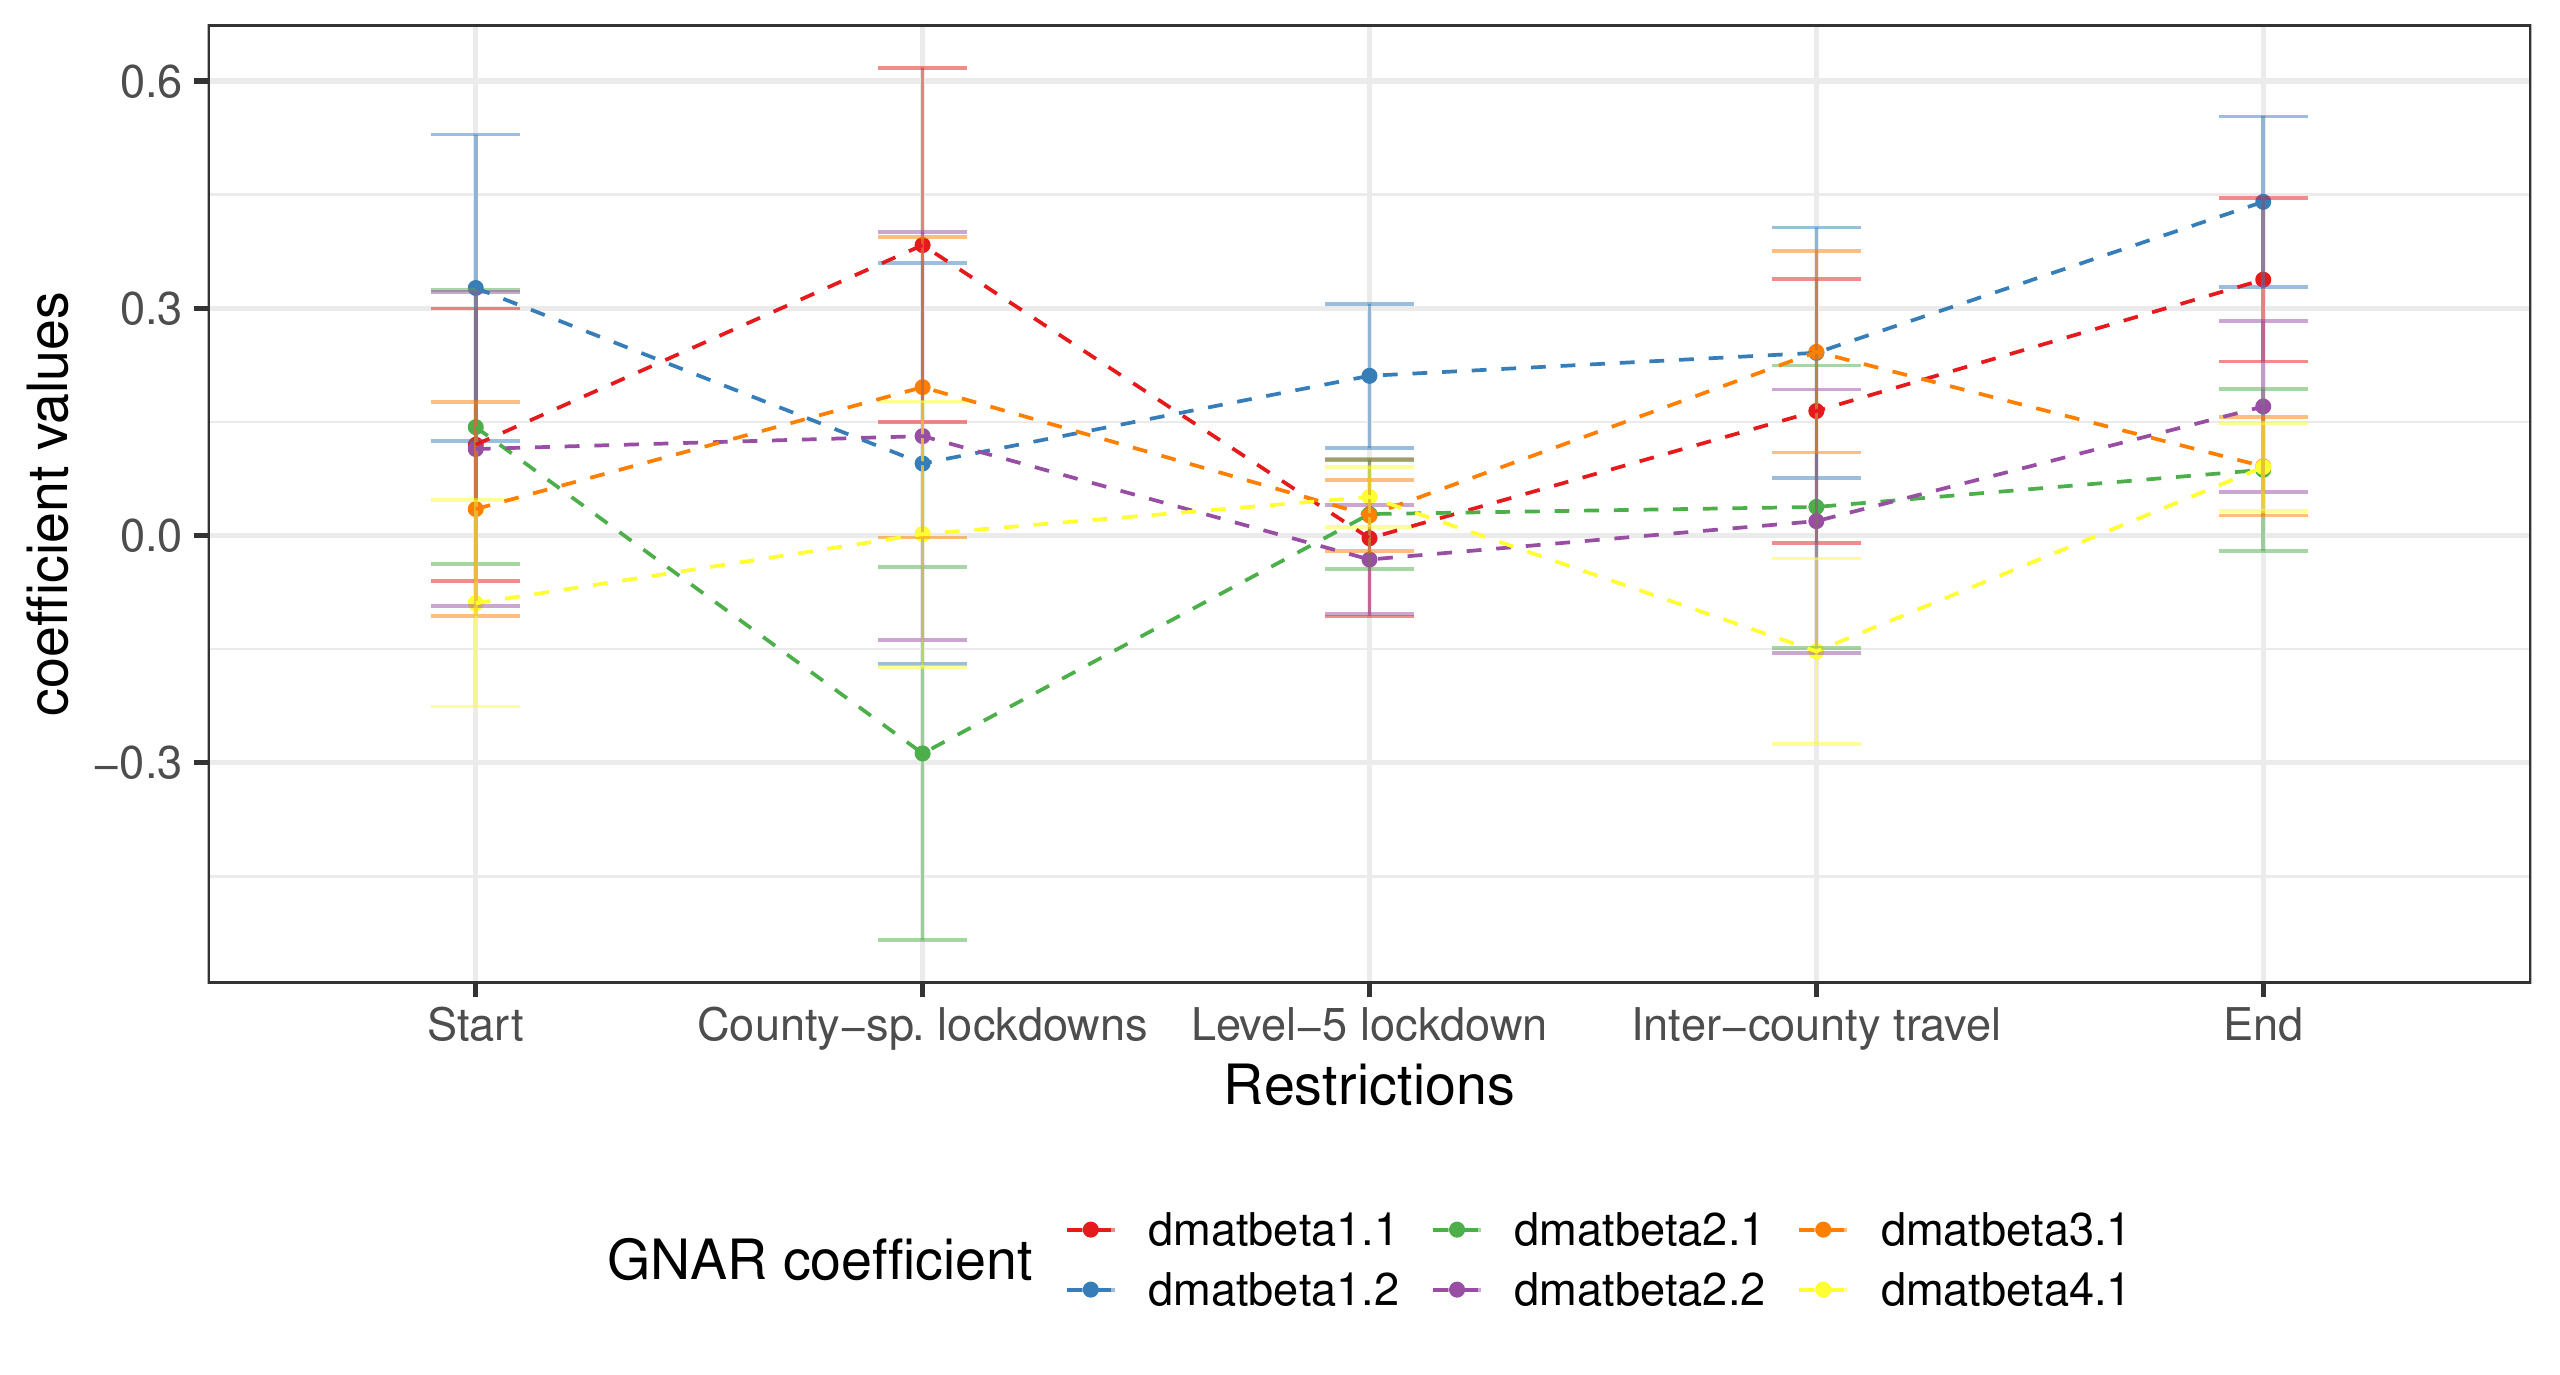}
  \caption{$\beta$-order}
\end{subfigure}
\caption[Change in GNAR model coefficients for COVID-19 regulations for Delaunay triangulation network]{Development of GNAR model coefficients for the global-$\alpha$ \code{GNAR(4,[2,2,1,1])} model across COVID-19 regulations for the \textbf{Delaunay triangulation} network}
\label{fig:parameter_delaunay}
\end{figure}

We fit a GNAR model for each network to each subset 1-5 individually and predict the last five weeks within each subset to obtain a mean absolute squared error (MASE) \cite{hyndman2006another}, \cite{leeming2019new}\footnote{See the Supplementary Material \ref{app:definition} for a definition of the MASE.}. 
The KNN network is tuned for each data subset.
We observe that the more variable the 1-lag COVID-19 ID is, the denser the KNN network.
The density of the KNN networks is partially compensated by a lower stage neighbourhood.  
In the DNN network, the more prominent and sharp a peak in 1-lag COVID-19 ID, the smaller the distance threshold $d$, i.e. the sparser the DNN network. 
\begin{table}[ht]
\small
\centering
\begin{tabular}{l|rrrr}
  \toprule 
 Network & data subset & k / d [in km] & GNAR model & BIC \\
 \midrule 
 \textbf{KNN} &   1 & 7.00 & GNAR-5-41100-TRUE & -280.73 \\ 
   &   2 & 7.00 & GNAR-5-22221-TRUE & -483.91 \\ 
   &   3 & 15.00 & GNAR-5-10000-TRUE & -429.43 \\ 
   &   4 & 25.00 & GNAR-5-11111-TRUE & 181.79 \\ 
   &   5 & 17.00 & GNAR-5-11100-TRUE & 145.33 \\ 
   \\
  \textbf{DNN} &   1 & 300.00 & GNAR-5-10000-TRUE & -284.88 \\ 
   &   2 & 175.00 & GNAR-5-11111-TRUE & -486.56 \\ 
   &   3 & 100.00 & GNAR-5-22221-TRUE & -428.27 \\ 
   &   4 & 250.00 & GNAR-3-111-TRUE & 181.45 \\ 
   &   5 & 300.00 & GNAR-5-11110-TRUE & 145.59 \\ 
   \bottomrule 
\end{tabular}
\caption{Overview over the best performing model and optimal 
neighbourhood size $k$ / distance threshold $d$ for the KNN and DNN network} 
\label{tab:best_model_knn_dnn_subsets}
\end{table}

A-priori, we might assume that restrictions in inter-county movement lead to the selection of smaller neighbourhood stages, independent of the network topology. 
This assumption cannot be verified.
Which network performs best varies strongly between the data subsets (see Table \ref{tab:best_model_datasets}).
Under more rigid movement restrictions, the $\beta$-order decreases in complexity, i.e. it has more zero entries. 
The GNAR models for pandemic phases in which inter-county travel was less or not limited show spatial dependence further back in the past.
 
The performance of the GNAR model depends on the pandemic situation.
After easing the inter-county restrictions, the BIC for dataset 4 and 5 increase drastically. 
However, the BIC proves uninformative to assess predictive accuracy, equally evident for the entire data set. 
Regarding the average MASE, data sets 2 and 4 which have less strict or no COVID-19 regulations have larger values than data sets 1 and 3 with strict regulations. 
This implies that GNAR models should be preferred to predict pandemic phases with strict movement regulations and are less suitable to model complex pandemic spread without restrictions. 
The GNAR model for the dataset 5 achieve high predictive performance. 
The average residual is large in absolute value for periods with many peaks.
Periods in which the COVID-19 ID oscillates around zero have a smaller average residual. 

As the variance in the data subsets increase, we can observe a tendency of sparser networks and more complex $\beta$-order.

\begin{table}[ht]
\small
\centering
\begin{tabular}{l|rrrrr}
  \toprule 
 Data subset & network & GNAR model &  BIC  & $\Bar{\varepsilon}$ & av. MASE \\
 \midrule 
   1 & DNN-300 & GNAR-5-10000-TRUE & -284.88 & 1.02 & 0.74 \\ 
    2 & DNN-175 & GNAR-5-11111-TRUE & -486.56 & 25.80 & 4.36 \\ 
    3 & Queen & GNAR-5-40000-TRUE & -432.91 & 14.31 & 0.89 \\ 
    4 & DNN-250 & GNAR-3-111-TRUE & 181.45 & 181.28 & 0.92 \\ 
    5 & Gabriel & GNAR-5-42220-TRUE & 144.77 & -14.38 & 0.83 \\ 
   \bottomrule 
\end{tabular}
\caption{Overview over the best performing model and network for every 
COVID-19 data subset; including the mean residual $\Bar{\varepsilon}$ and the average (av.) MASE; the values for AIC are very similar to the BIC values $AIC = (-285.18, -487, -433.33, 181.19, 144.14)$} 
\label{tab:best_model_datasets}
\end{table}

2-lag differencing 
\begin{table}[ht]
\centering
\begin{tabular}{l|rrrrr}
  \toprule 
 Data subset & network & \code{GNAR} model & 
                                          BIC  & mean residual & mean MASE \\
 \midrule 
   1 & SOI & GNAR-5-20000-TRUE & -272.78 & -0.74 & 0.72 \\ 
    2 & SOI & GNAR-5-22220-TRUE & -485.61 & 67.87 & 6.36 \\ 
    3 & KNN-15 & GNAR-5-11111-TRUE & -417.44 & 6.73 & 0.53 \\ 
    4 & DNN-325 & GNAR-5-11110-TRUE & 183.63 & 2.90 & 0.62 \\ 
    5 & KNN-9 & GNAR-5-22220-TRUE & 152.83 & -7.26 & 0.48 \\ 
   \bottomrule 
\end{tabular}
\caption{Overview over the best performing model and network for every 
COVID-19 data subset} 
\label{tab:best_model_datasets}
\end{table}

For data subsets 1, 2, 3 and 5, $\alpha = 5$ is chosen.
For data subset 4, the optimal GNAR model has $\alpha = 3$. 
During periods of more lenient COVID-19 regulations and stronger human movement within and between counties, the value for the $\alpha$-coefficients increase, showing that the trajectory of COVID-19 incidence depends more strongly on its history.
The large values for the $\beta$-order coefficients indicate a particularly strong spatial dependence in 1-lag COVID-19 ID for dataset 2 and 4.
The increase in absolute value for the $\beta$-coefficients during periods with more lenient or no restrictions hints at the efficiency of COVID-19 restrictions. 

\begin{figure}[h!]
\centering
\begin{subfigure}{\textwidth}
  \centering
  \includegraphics[width = 0.7\textwidth]{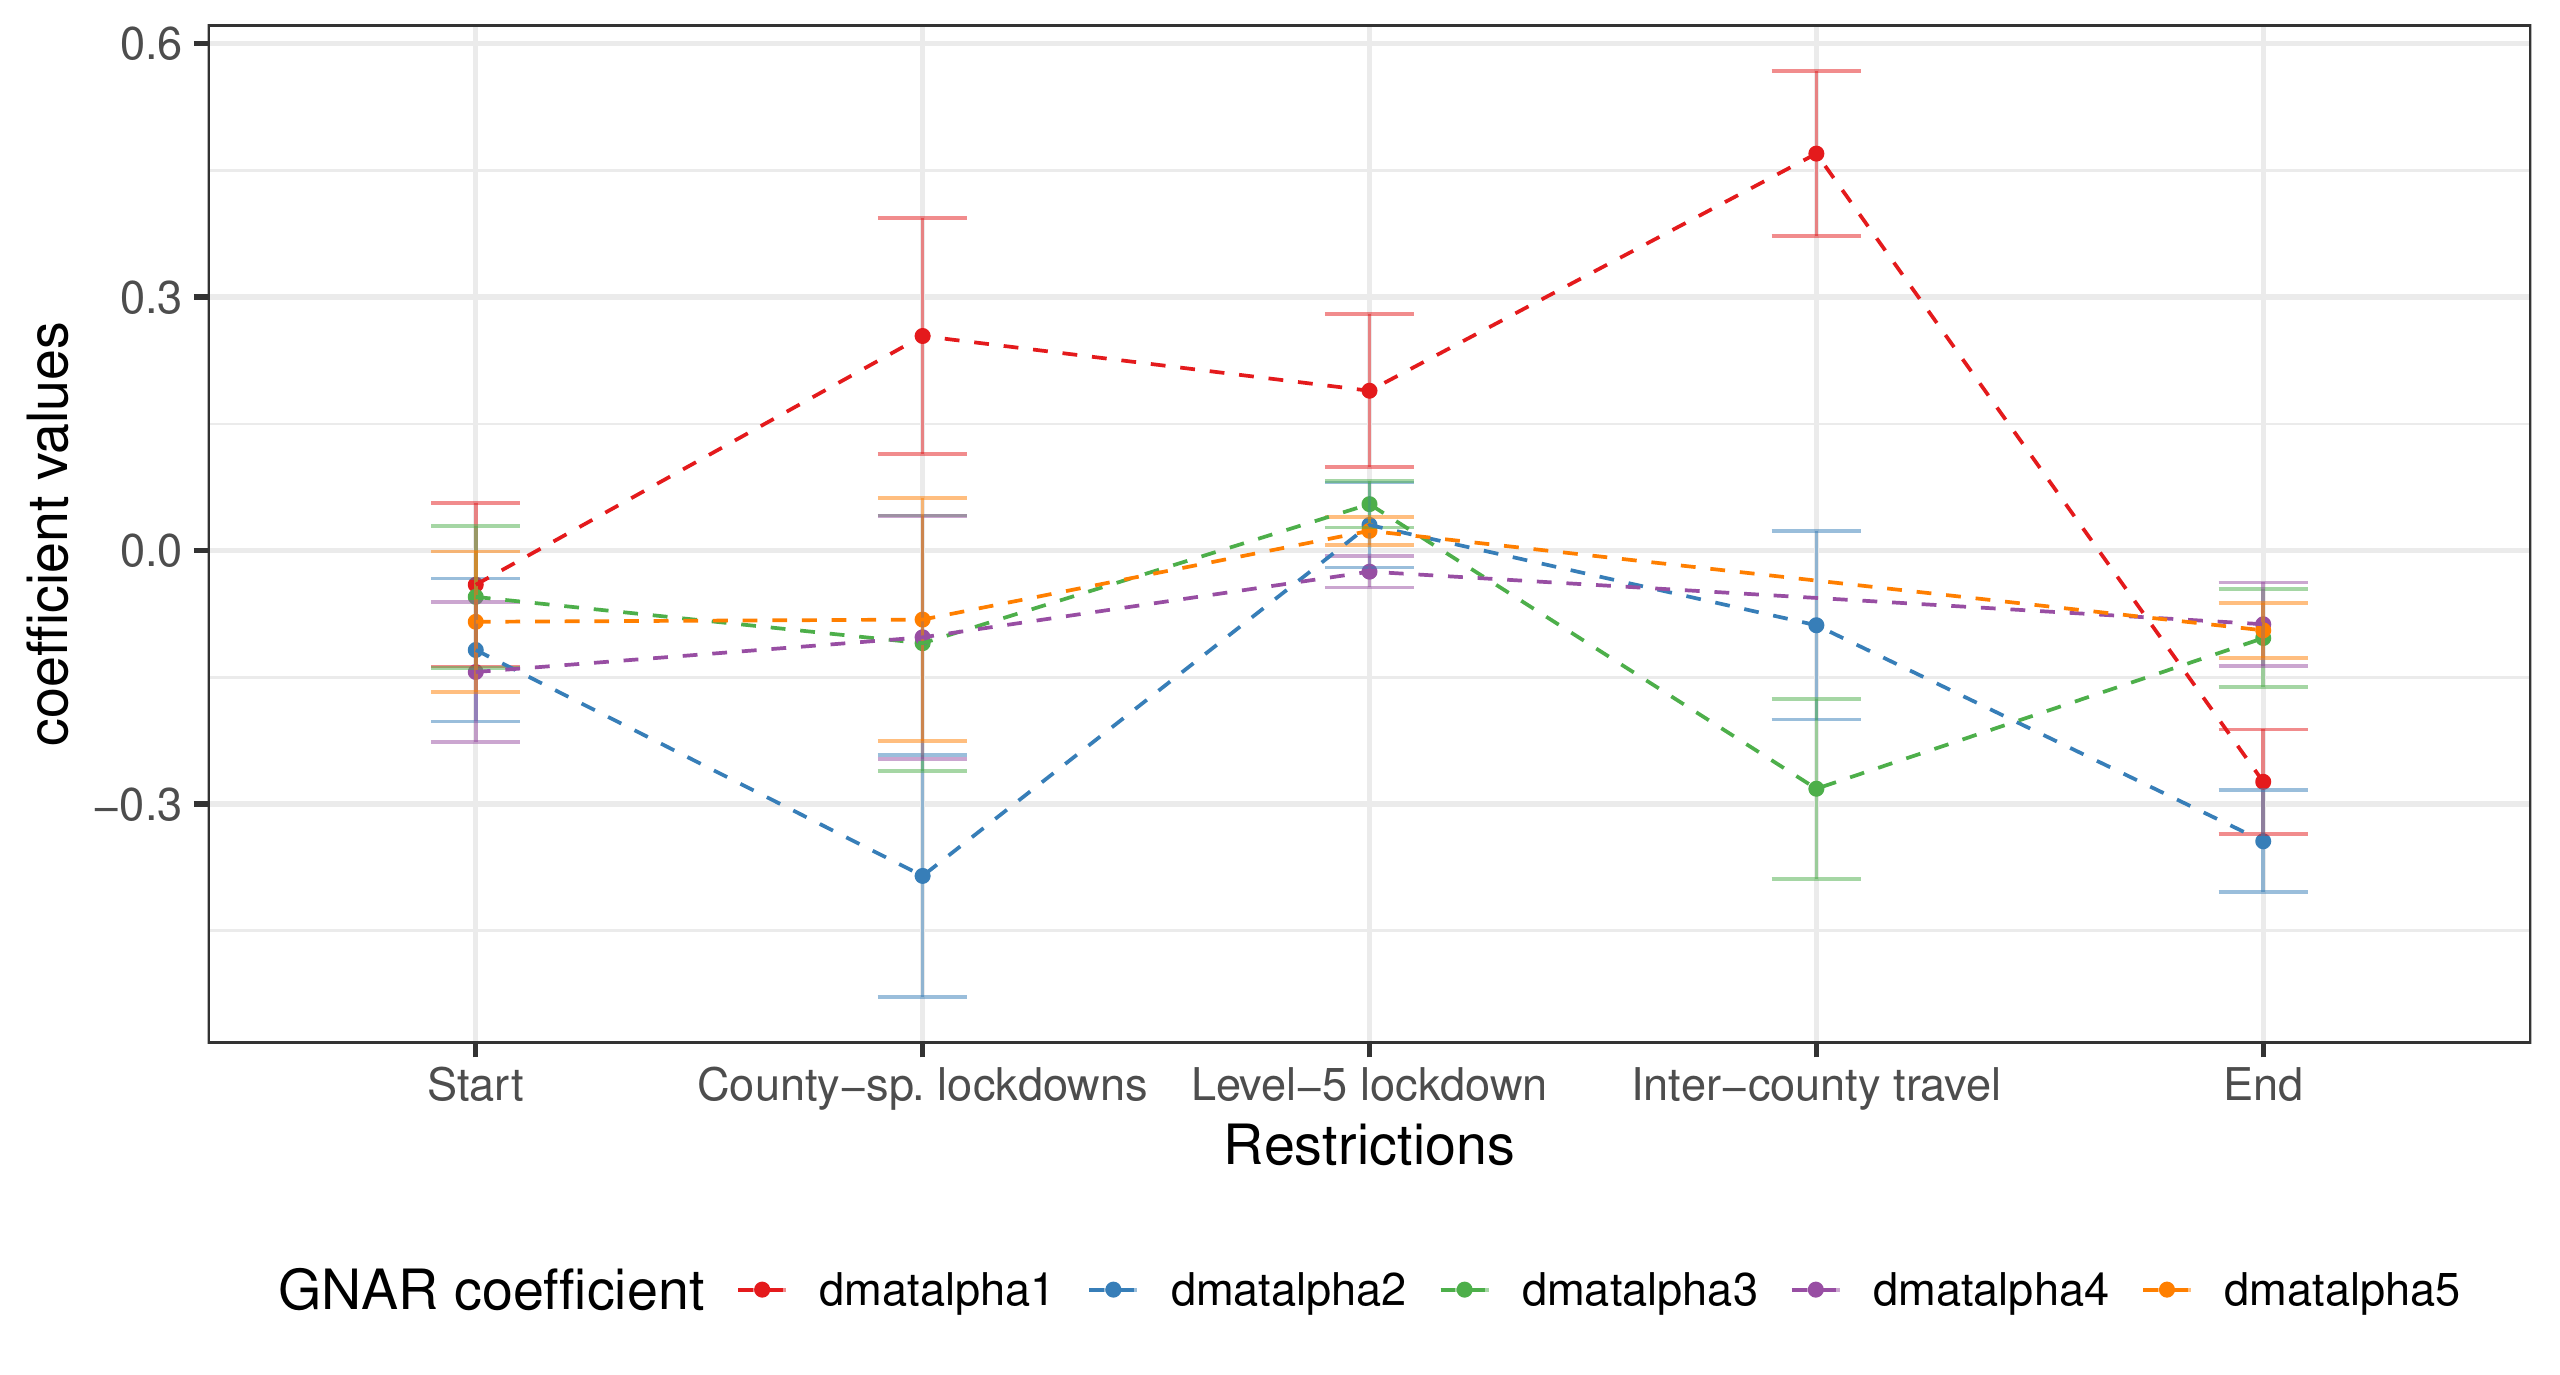}
  \caption{$\alpha$-order}
\end{subfigure}
\begin{subfigure}{\textwidth}
  \centering
  \includegraphics[width = 0.7\textwidth]{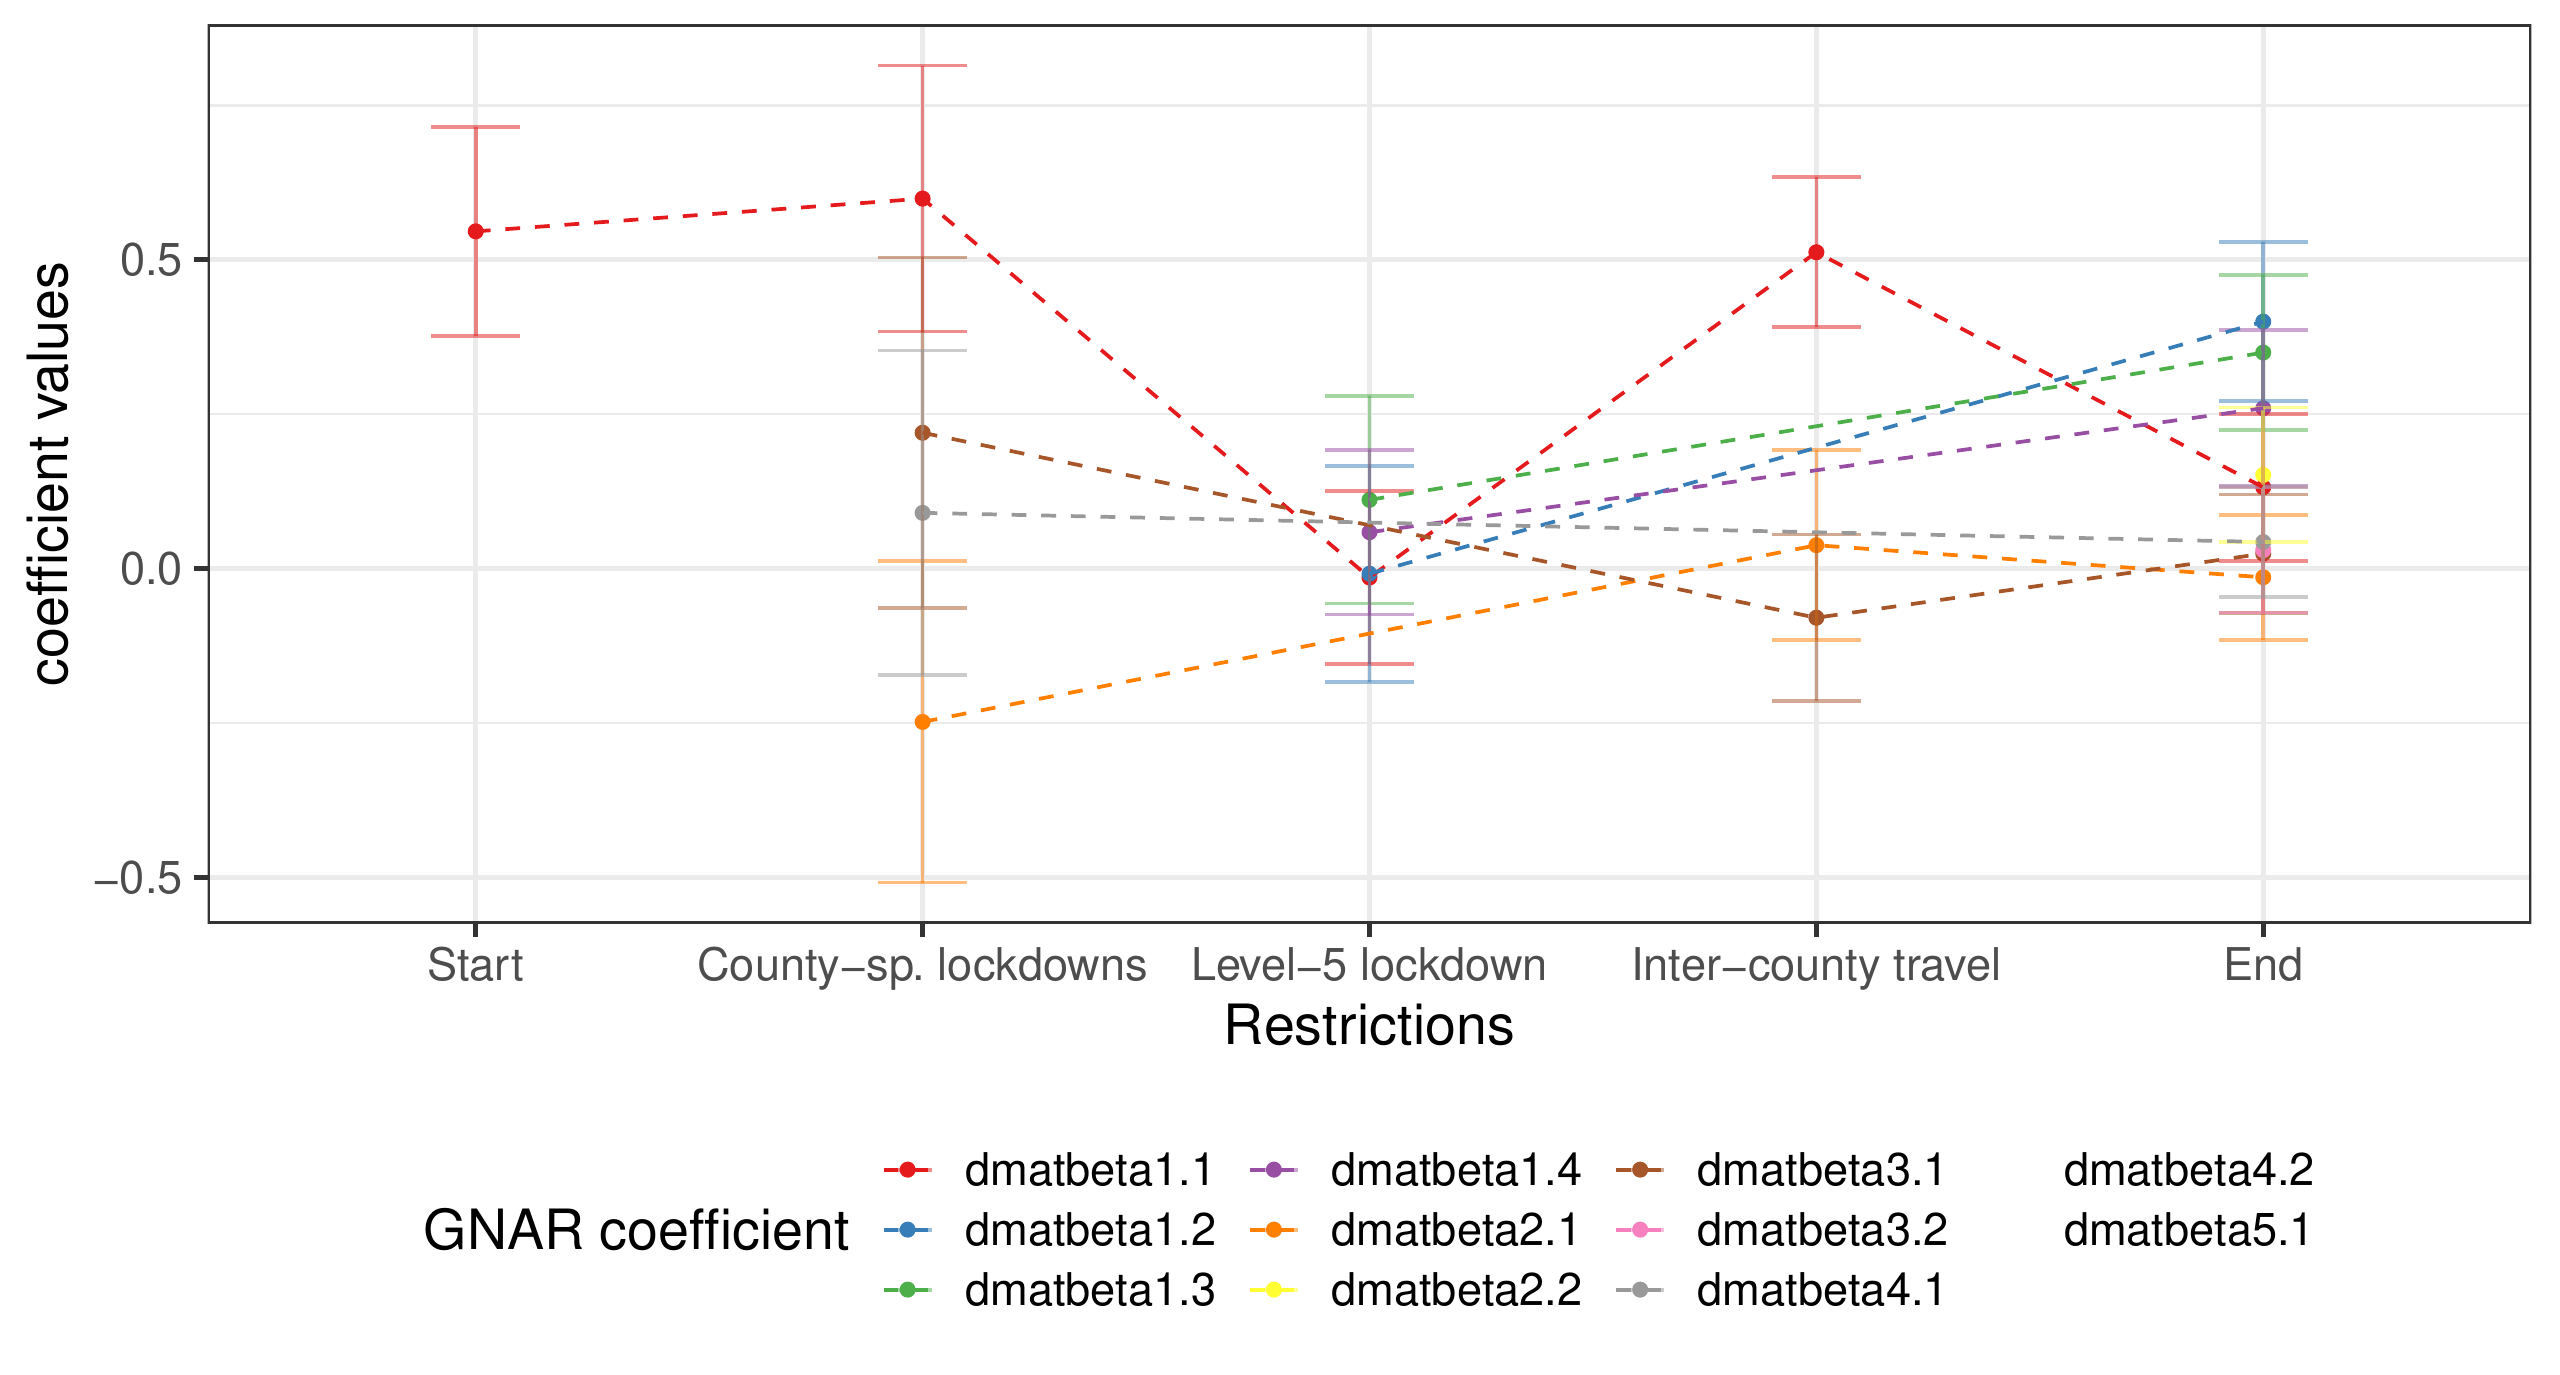}
  \caption{$\beta$-order}
\end{subfigure}
\caption{Development of GNAR model coefficients for optimal GNAR models for datasets 1-5}
\label{fig:coefficient_dev_subsets}
\end{figure}

For each data set, we compare the performance of the best models for all networks when predicting the weekly 1-lag COVID-19 ID for the last 5 weeks in the observed time period.
During time periods with strict COVID-19 regulations, the difference in predictive performance between the different networks is less prominent than for periods with fewer restrictions, since the COVID-19 incidence becomes more erratic as human mobility and interaction increases.

\begin{figure}[h!]
\centering
\begin{subfigure}{\textwidth}
  \centering
  \includegraphics[width = 0.7\textwidth]{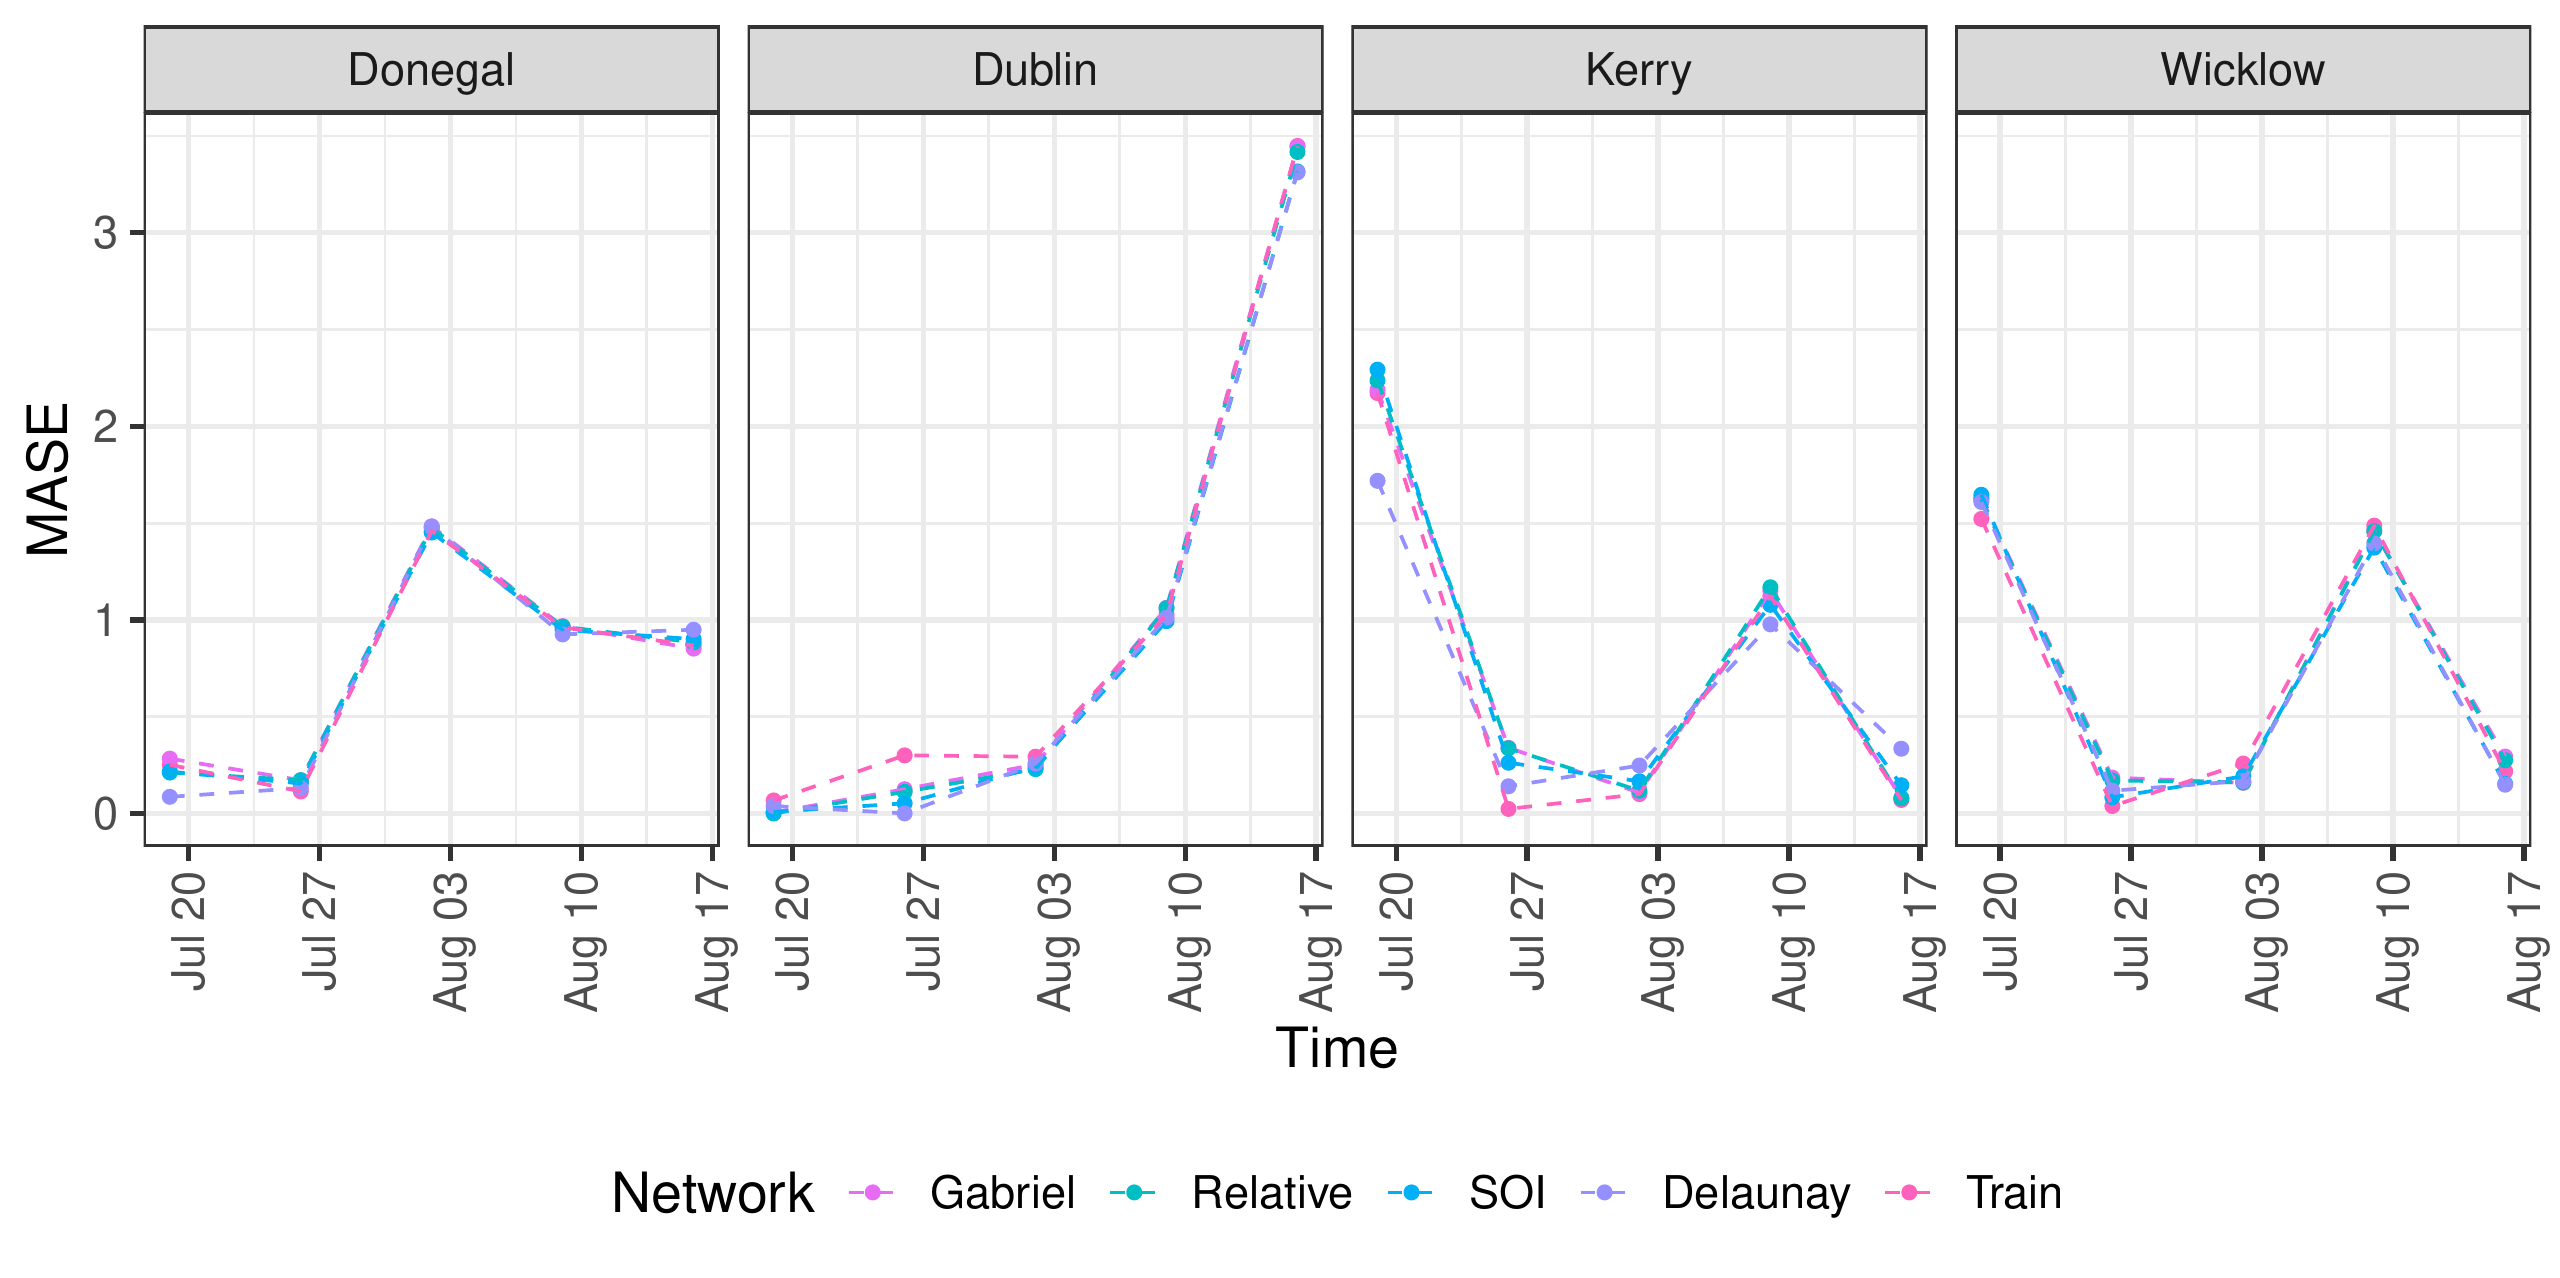}
  \caption{\textbf{Delaunay triangulation}, \textbf{Gabriel}, \textbf{Relative neighbourhood}, \textbf{SOI} and \textbf{Railway-based} network}
\end{subfigure}
\begin{subfigure}{\textwidth}
  \centering
  \includegraphics[width = 0.7\textwidth]{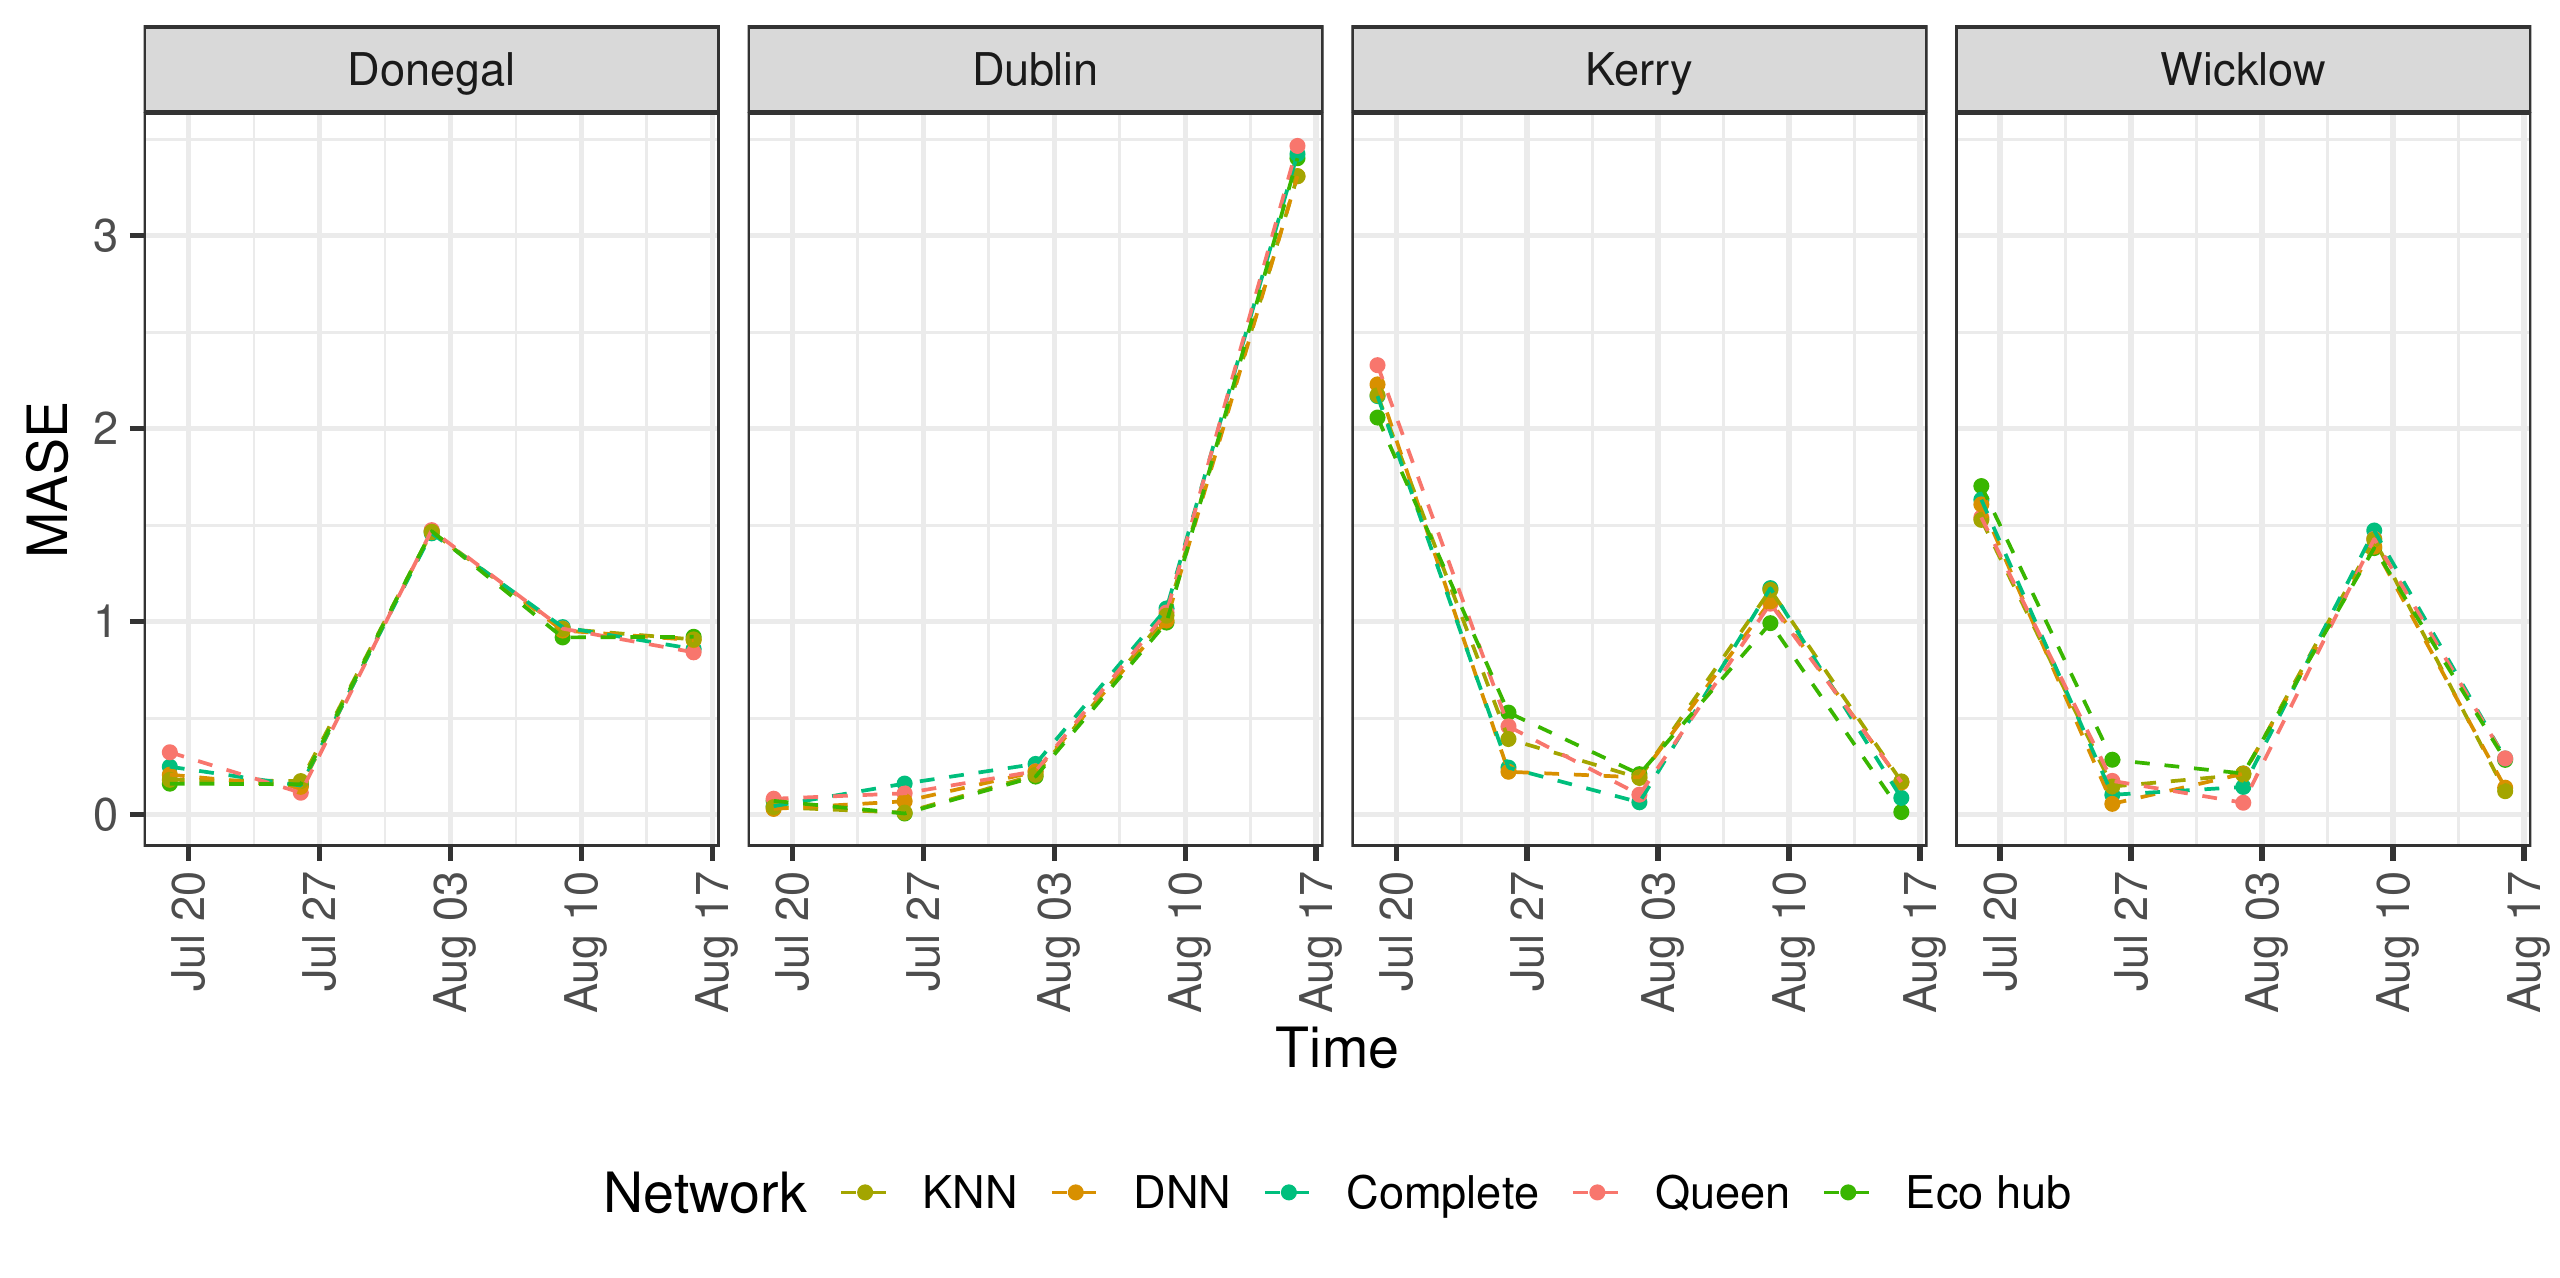}
  \caption{\textbf{KNN}, \textbf{DNN}, \textbf{Complete}, \textbf{Queen's contiguity} and \textbf{Economic hub} network}
\end{subfigure}
\caption{MASE values for data subset 1}
\label{fig:mase_subset_1}
\end{figure}

For data set 2, the DNN network performs surprisingly badly, while the Tailway-based network predicts surprisingly well. 
\begin{figure}[h!]
\centering
\begin{subfigure}{\textwidth}
  \centering
  \includegraphics[width = 0.7\textwidth]{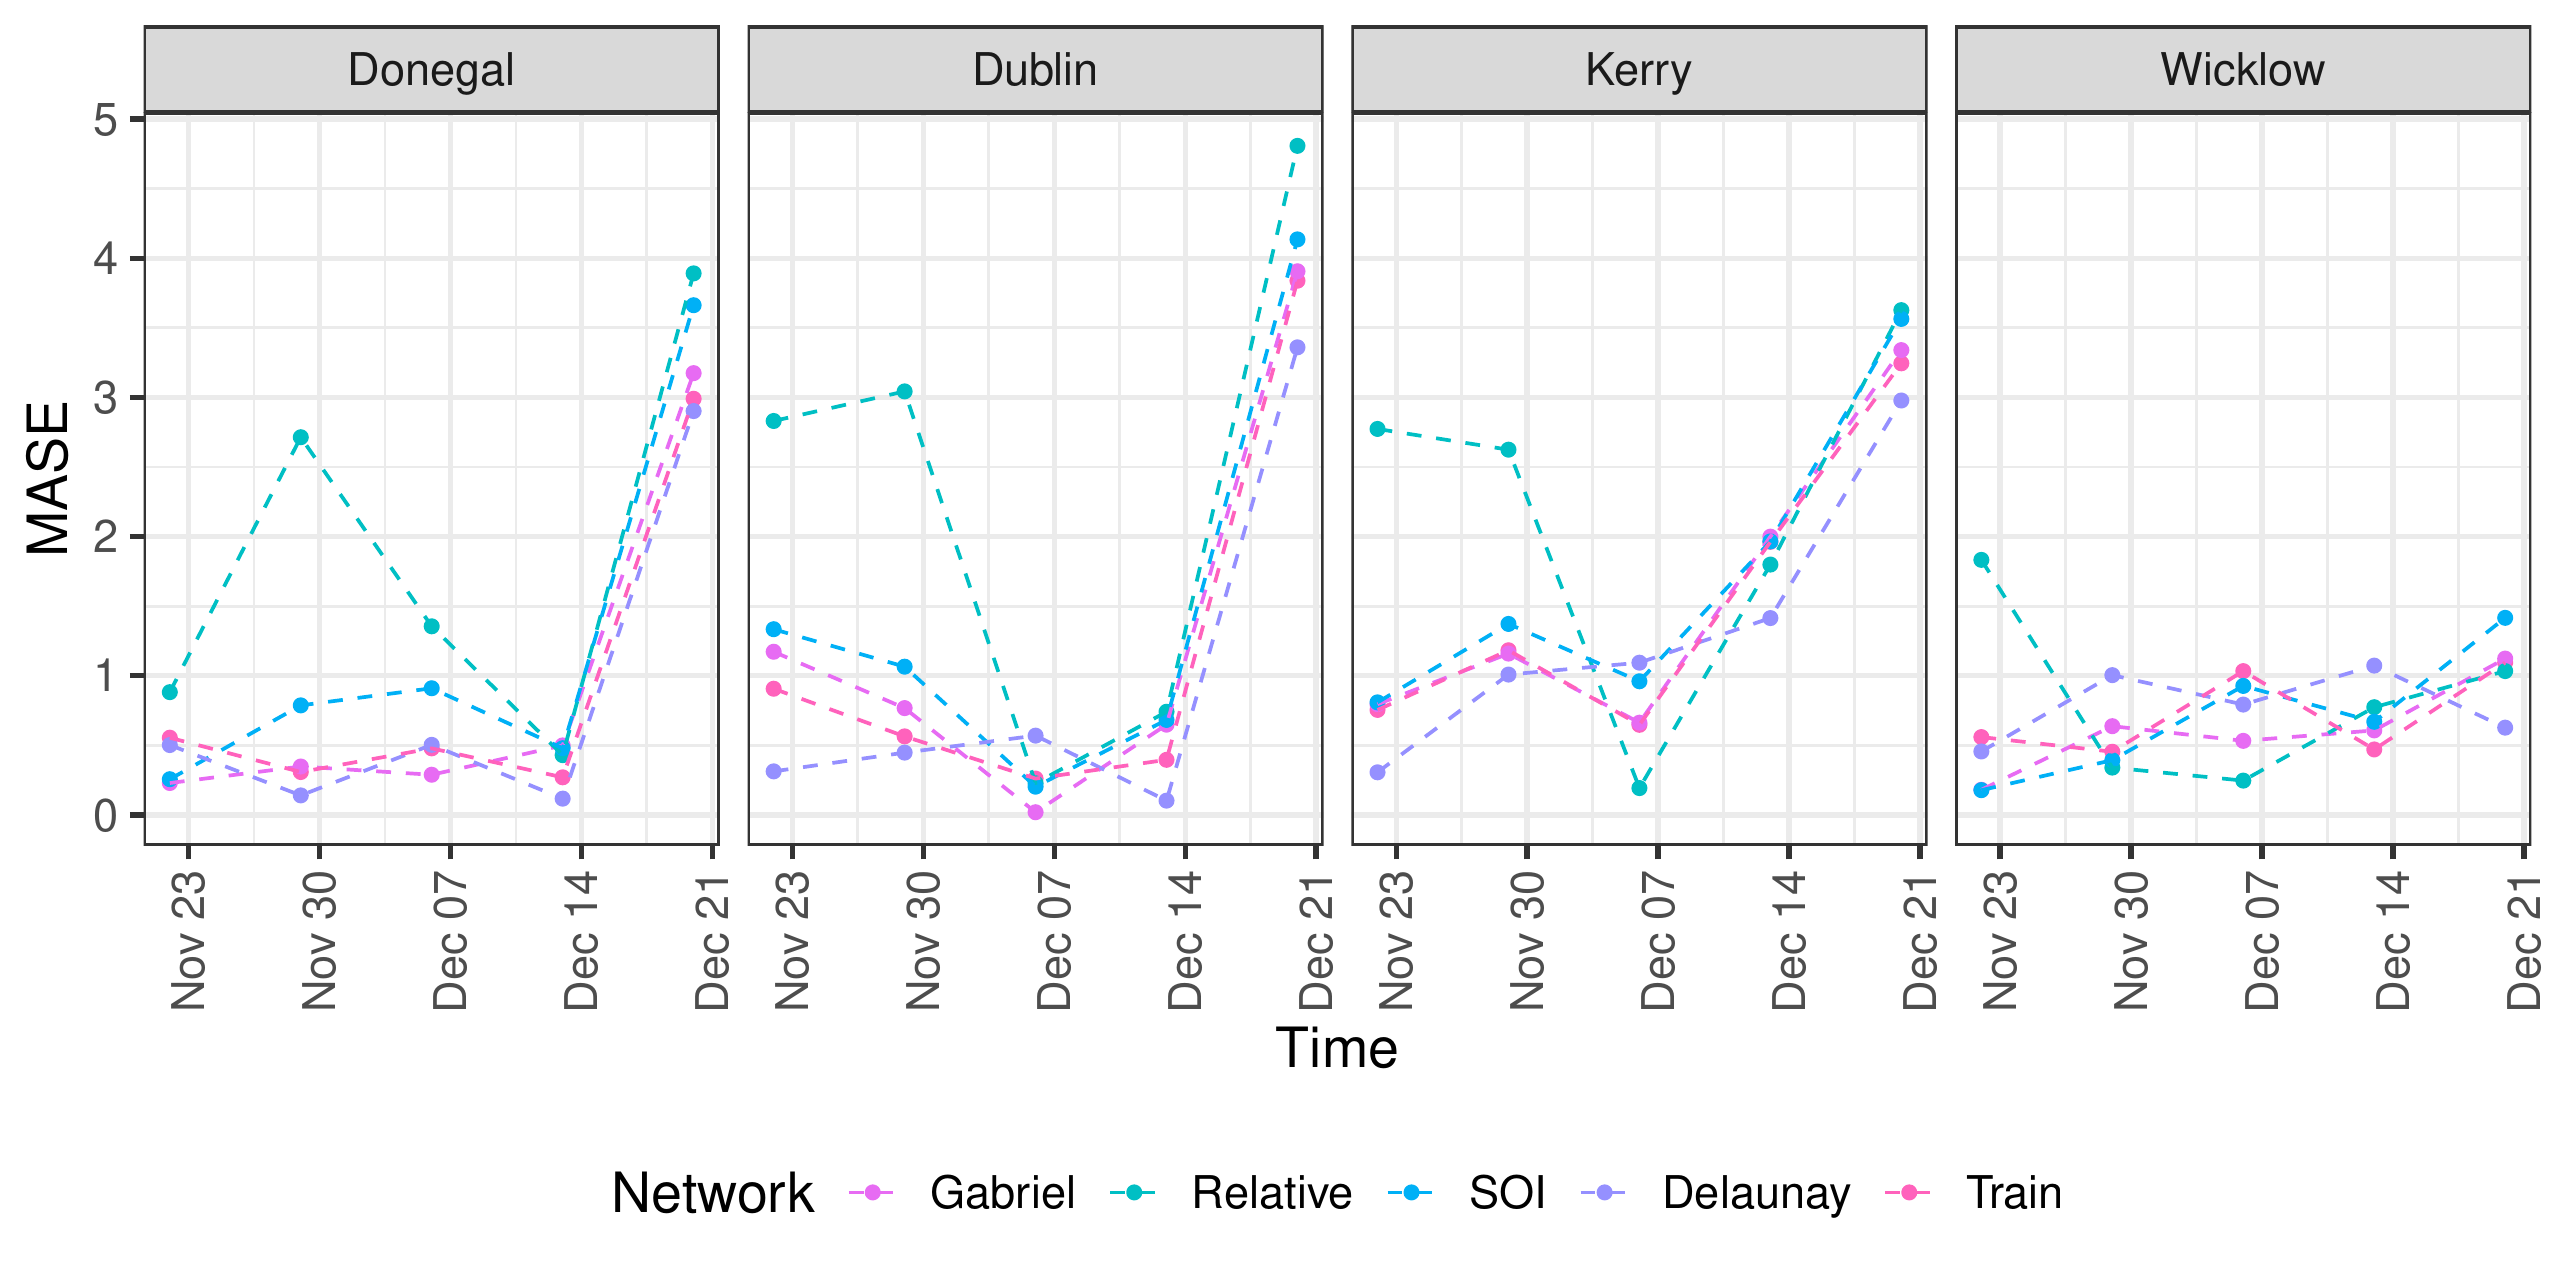}
  \caption{\textbf{Delaunay triangulation}, \textbf{Gabriel}, \textbf{Relative neighbourhood}, \textbf{SOI} and \textbf{Railway-based} network}
\end{subfigure}
\begin{subfigure}{\textwidth}
  \centering
  \includegraphics[width = 0.7\textwidth]{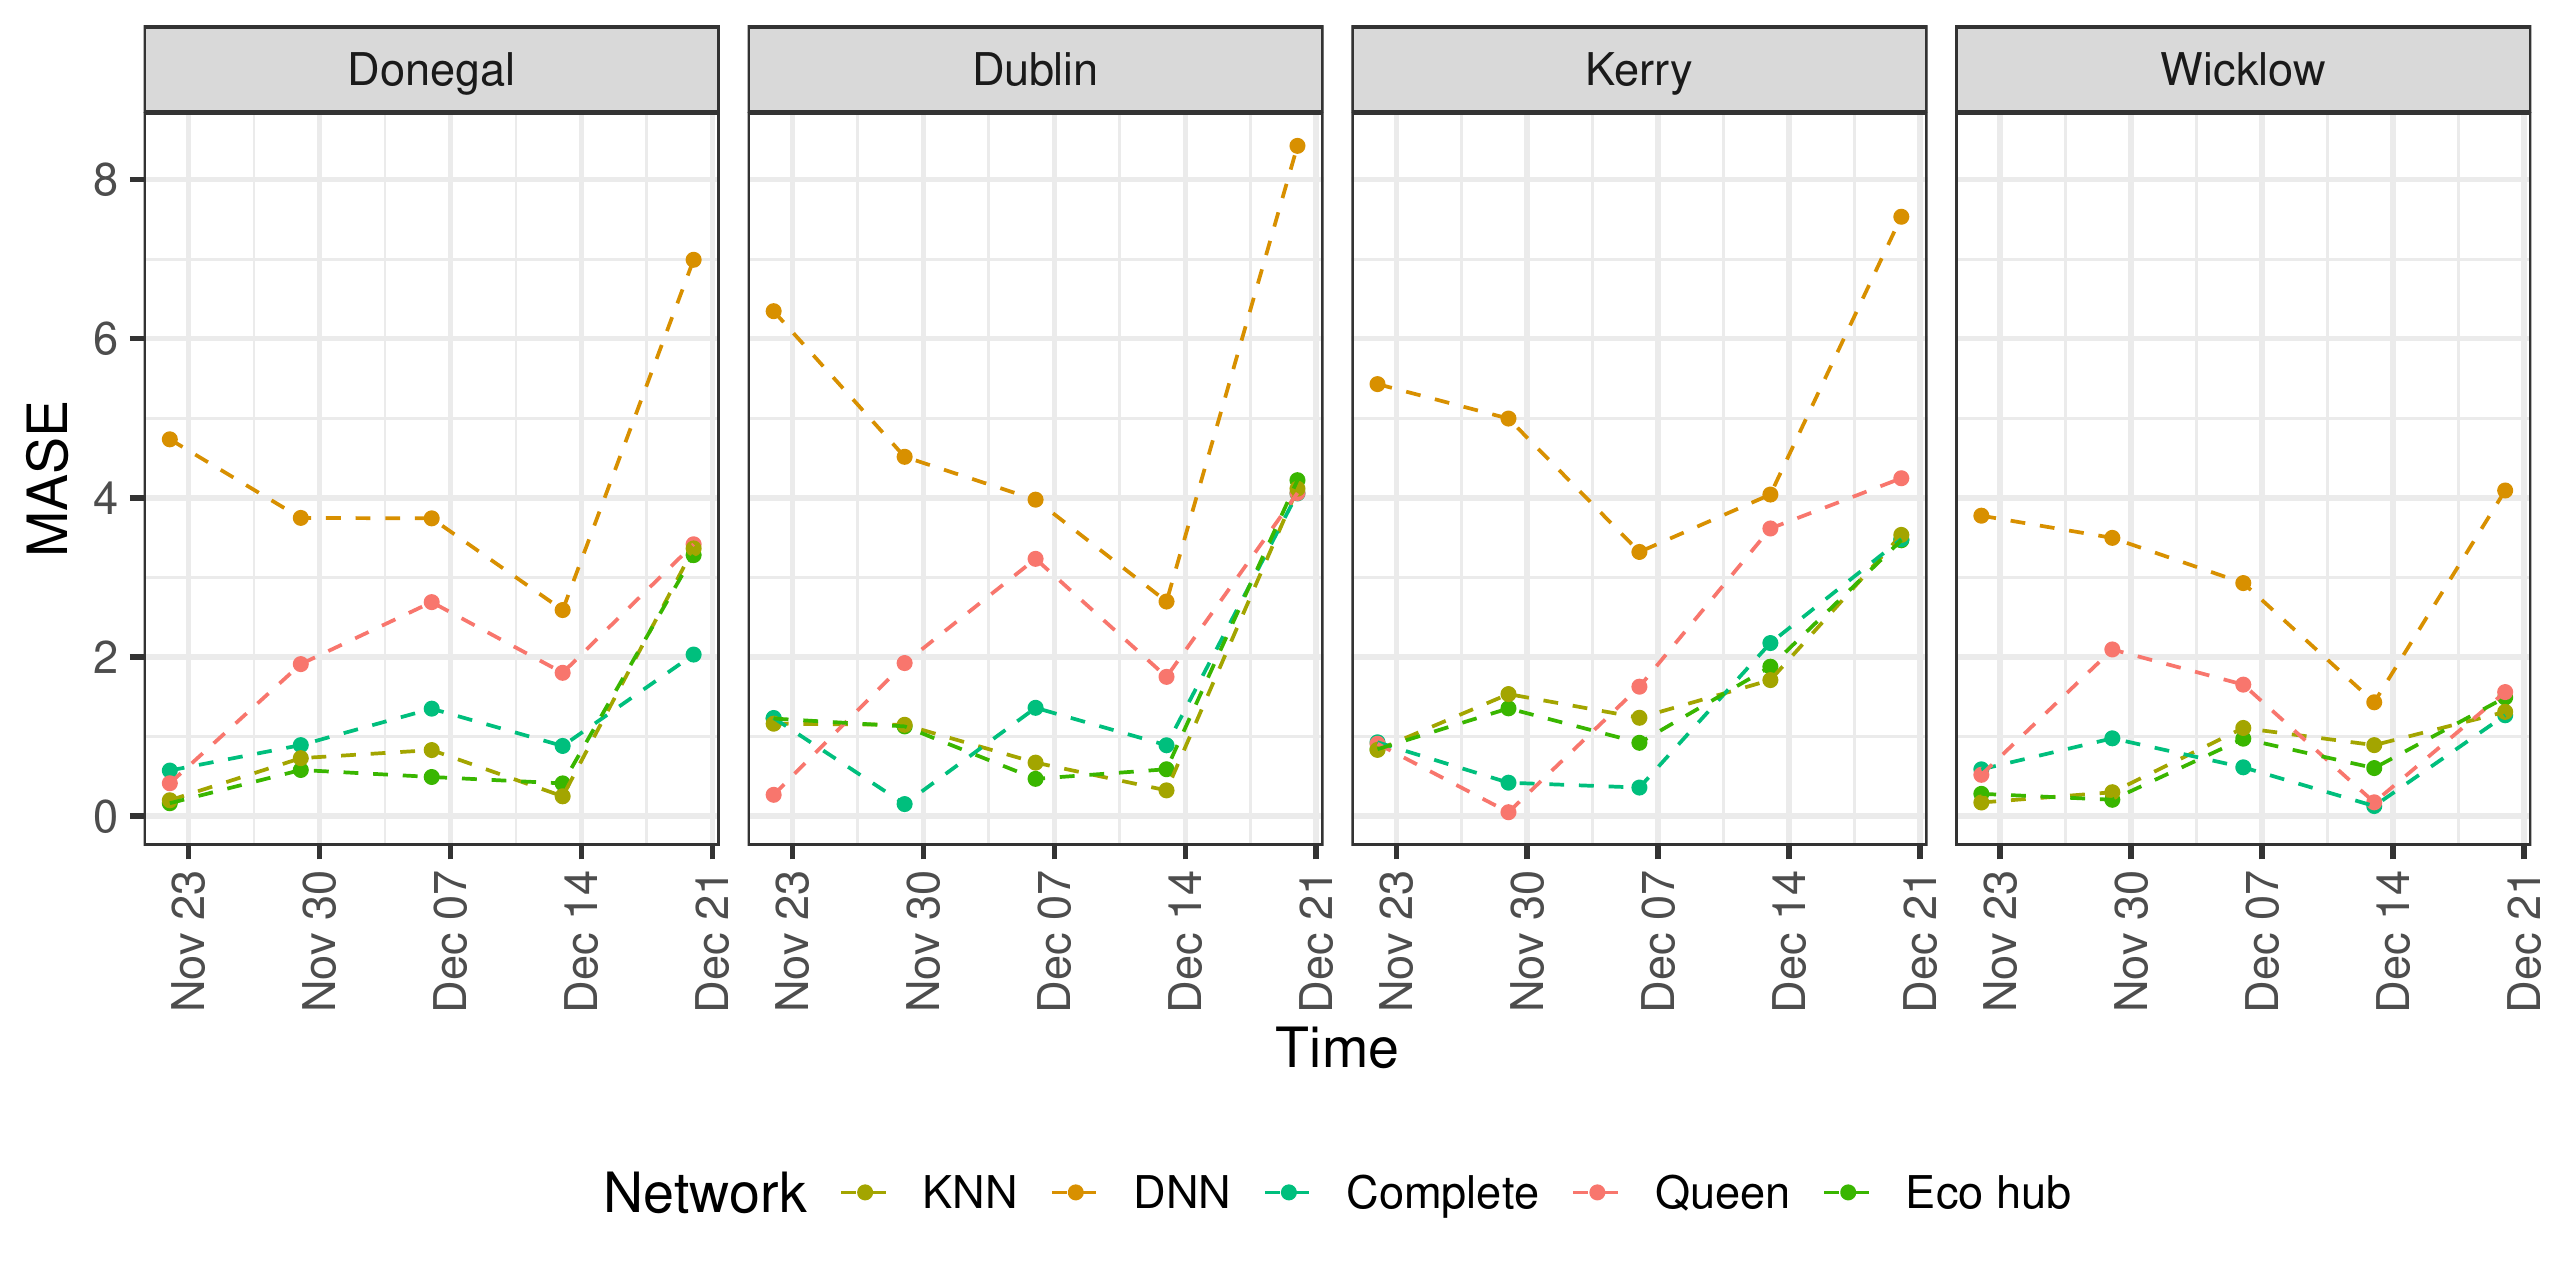}
  \caption{\textbf{KNN}, \textbf{DNN}, \textbf{Complete}, \textbf{Queen's contiguity} and \textbf{Economic hub} network}
\end{subfigure}
\caption{MASE values for data subset 2}
\label{fig:mase_subset_2}
\end{figure}

The majority of networks follow the same trajectory in predictive accuracy for dataset 3, but for the DNN and KNN network.
\begin{figure}[h!]
\centering
\begin{subfigure}{\textwidth}
  \centering
  \includegraphics[width = 0.7\textwidth]{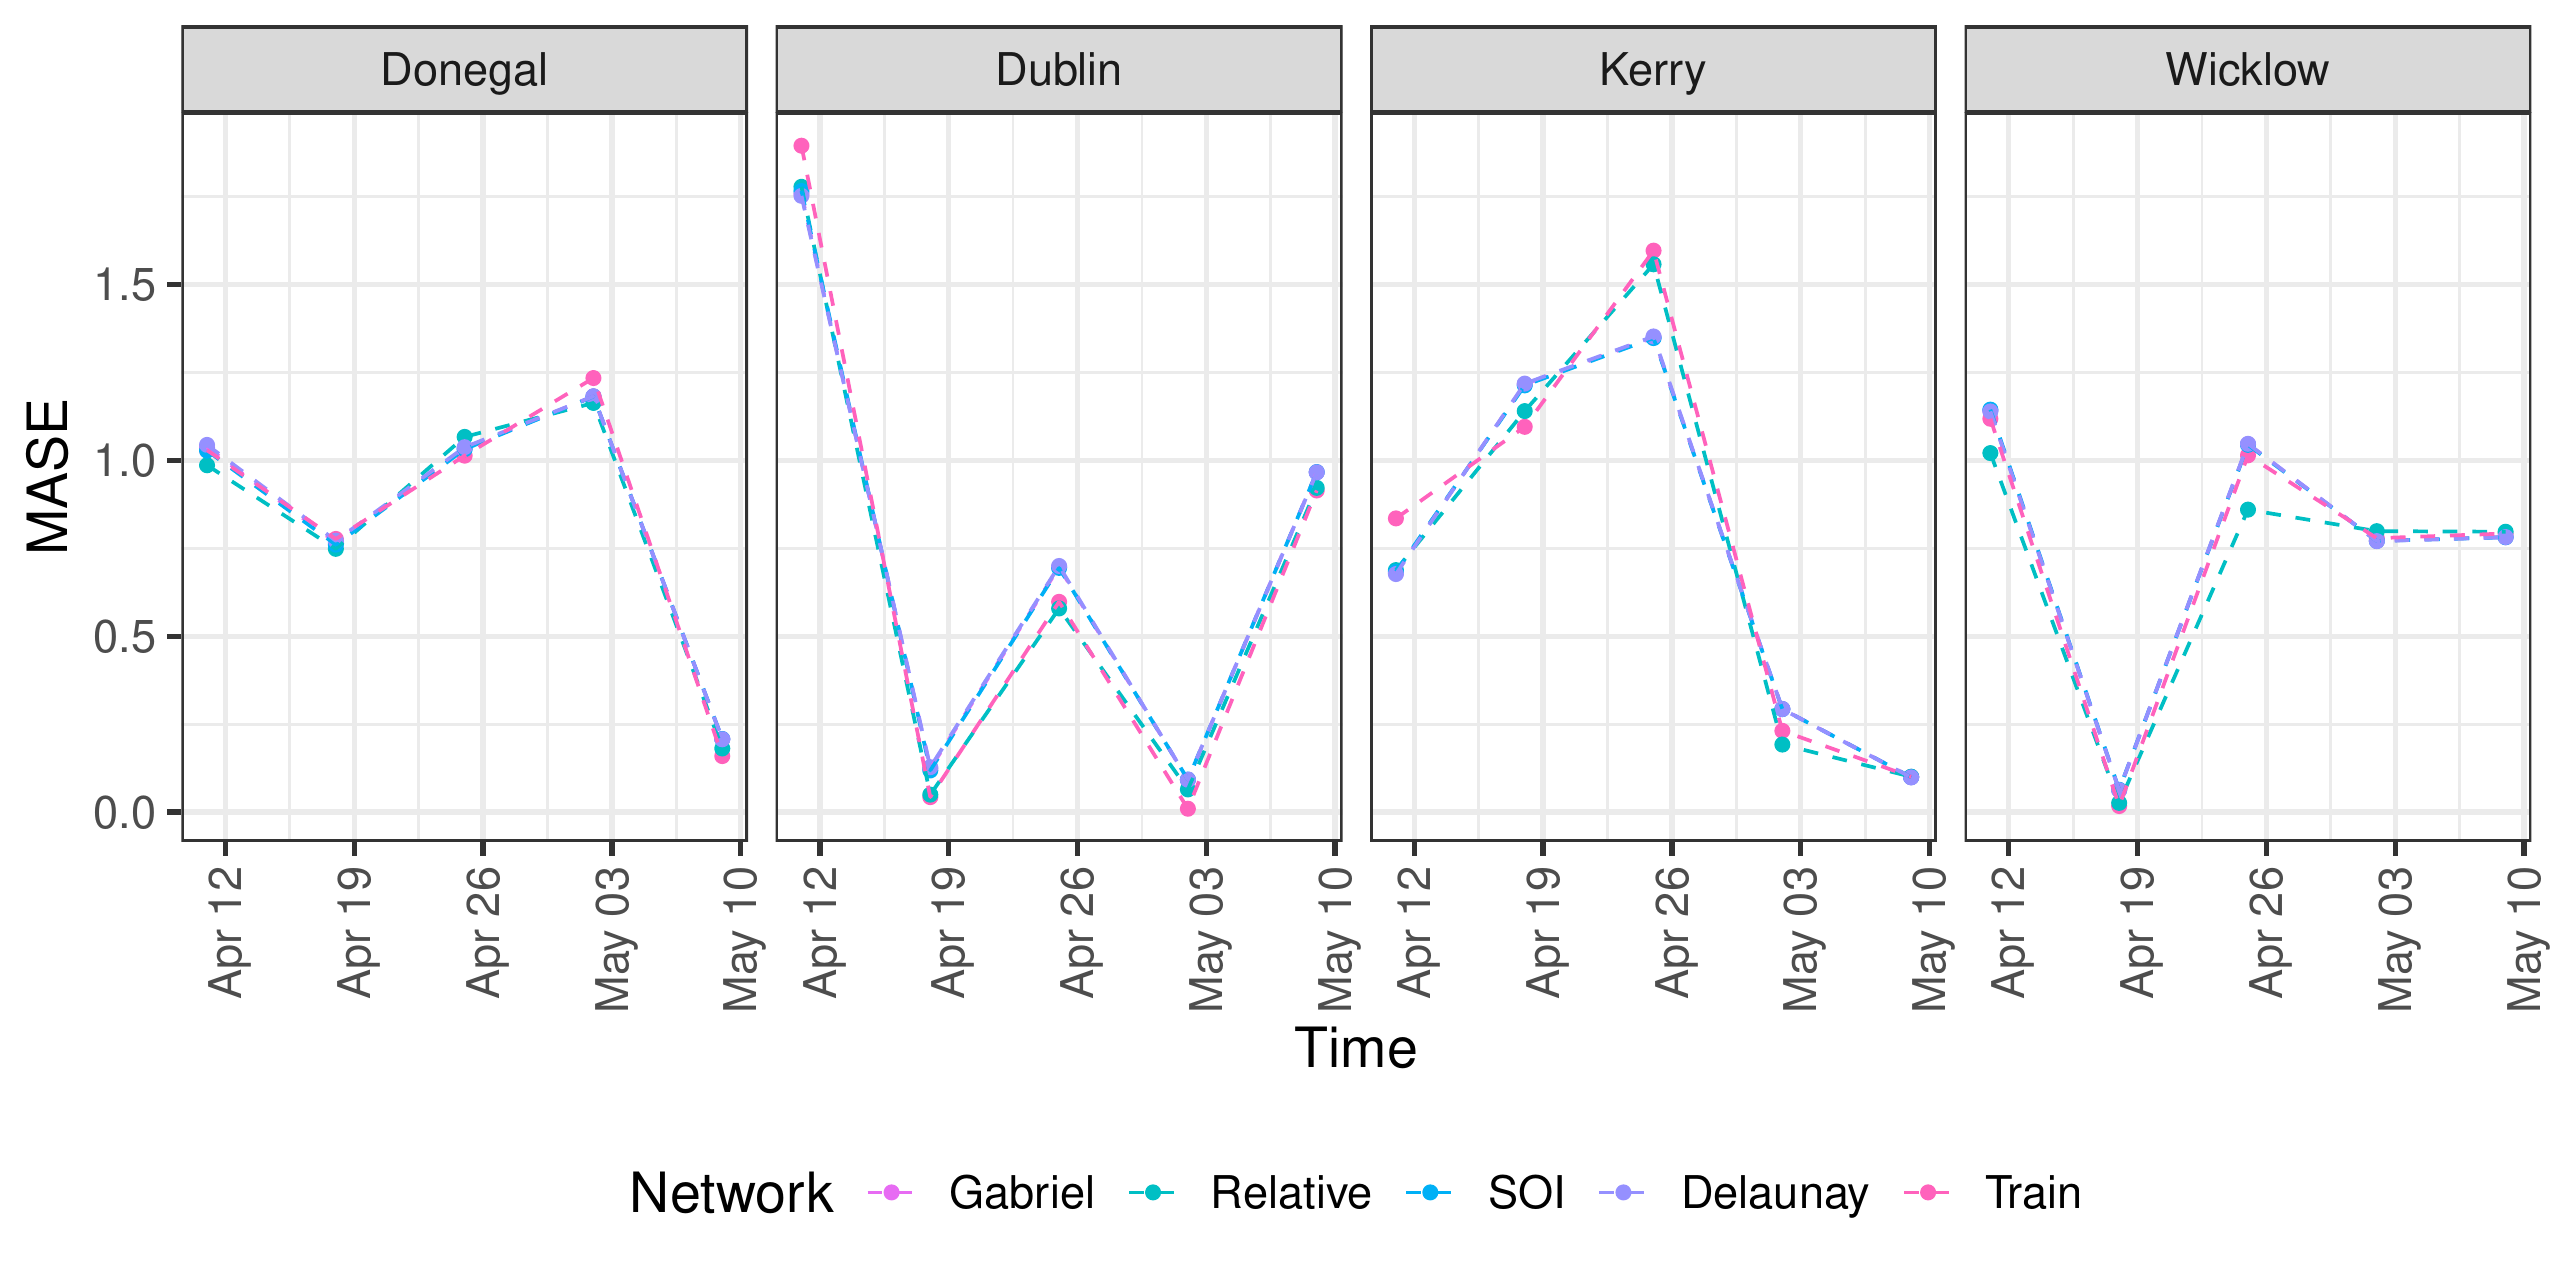}
  \caption{\textbf{Delaunay triangulation}, \textbf{Gabriel}, \textbf{Relative neighbourhood}, \textbf{SOI} and \textbf{Railway-based} network}
\end{subfigure}
\begin{subfigure}{\textwidth}
  \centering
  \includegraphics[width = 0.7\textwidth]{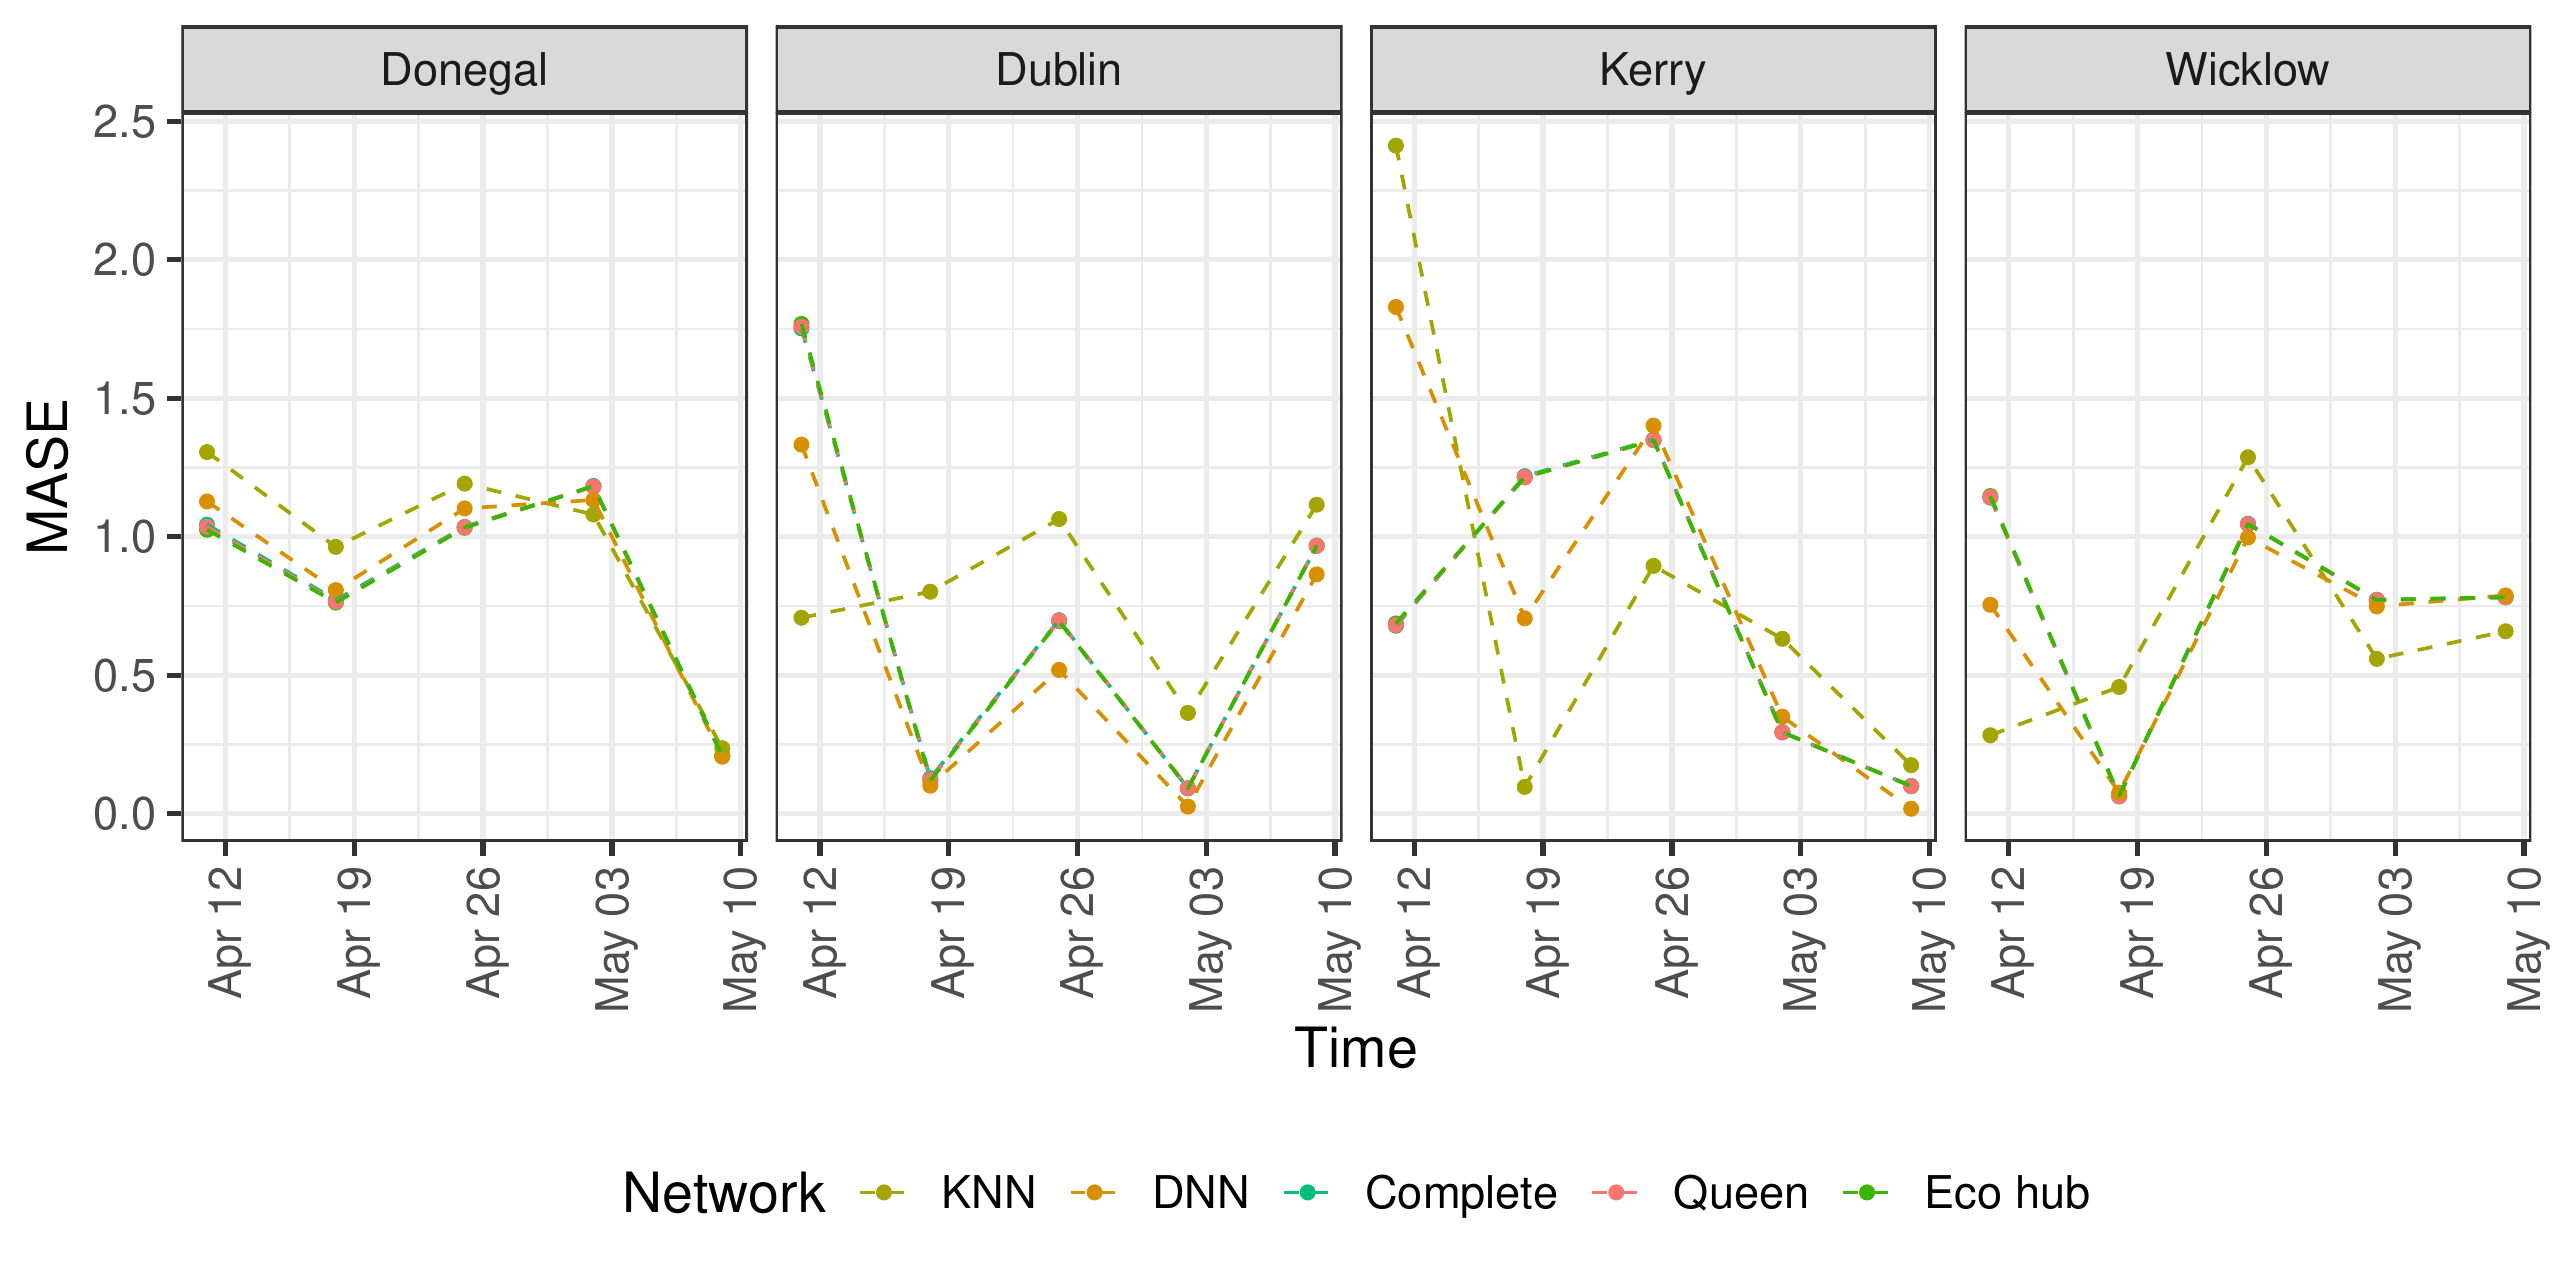}
  \caption{\textbf{KNN}, \textbf{DNN}, \textbf{Complete}, \textbf{Queen's contiguity} and \textbf{Economic hub} network}
\end{subfigure}
\caption{MASE values for data subset 3}
\label{fig:mase_subset_3}
\end{figure}

For data set 4, the suitability of the railway-based network again stands out. 
The high suitability of the railway-based network to predict the COVID-19 incidence during periods with few restrictions suggests human mobility as a driving force in disease spread. 
This is also emphasised by the difference in predictive performance between the Queen's and Economic hub network. 
\begin{figure}[h!]
\centering
\begin{subfigure}{\textwidth}
  \centering
  \includegraphics[width = 0.7\textwidth]{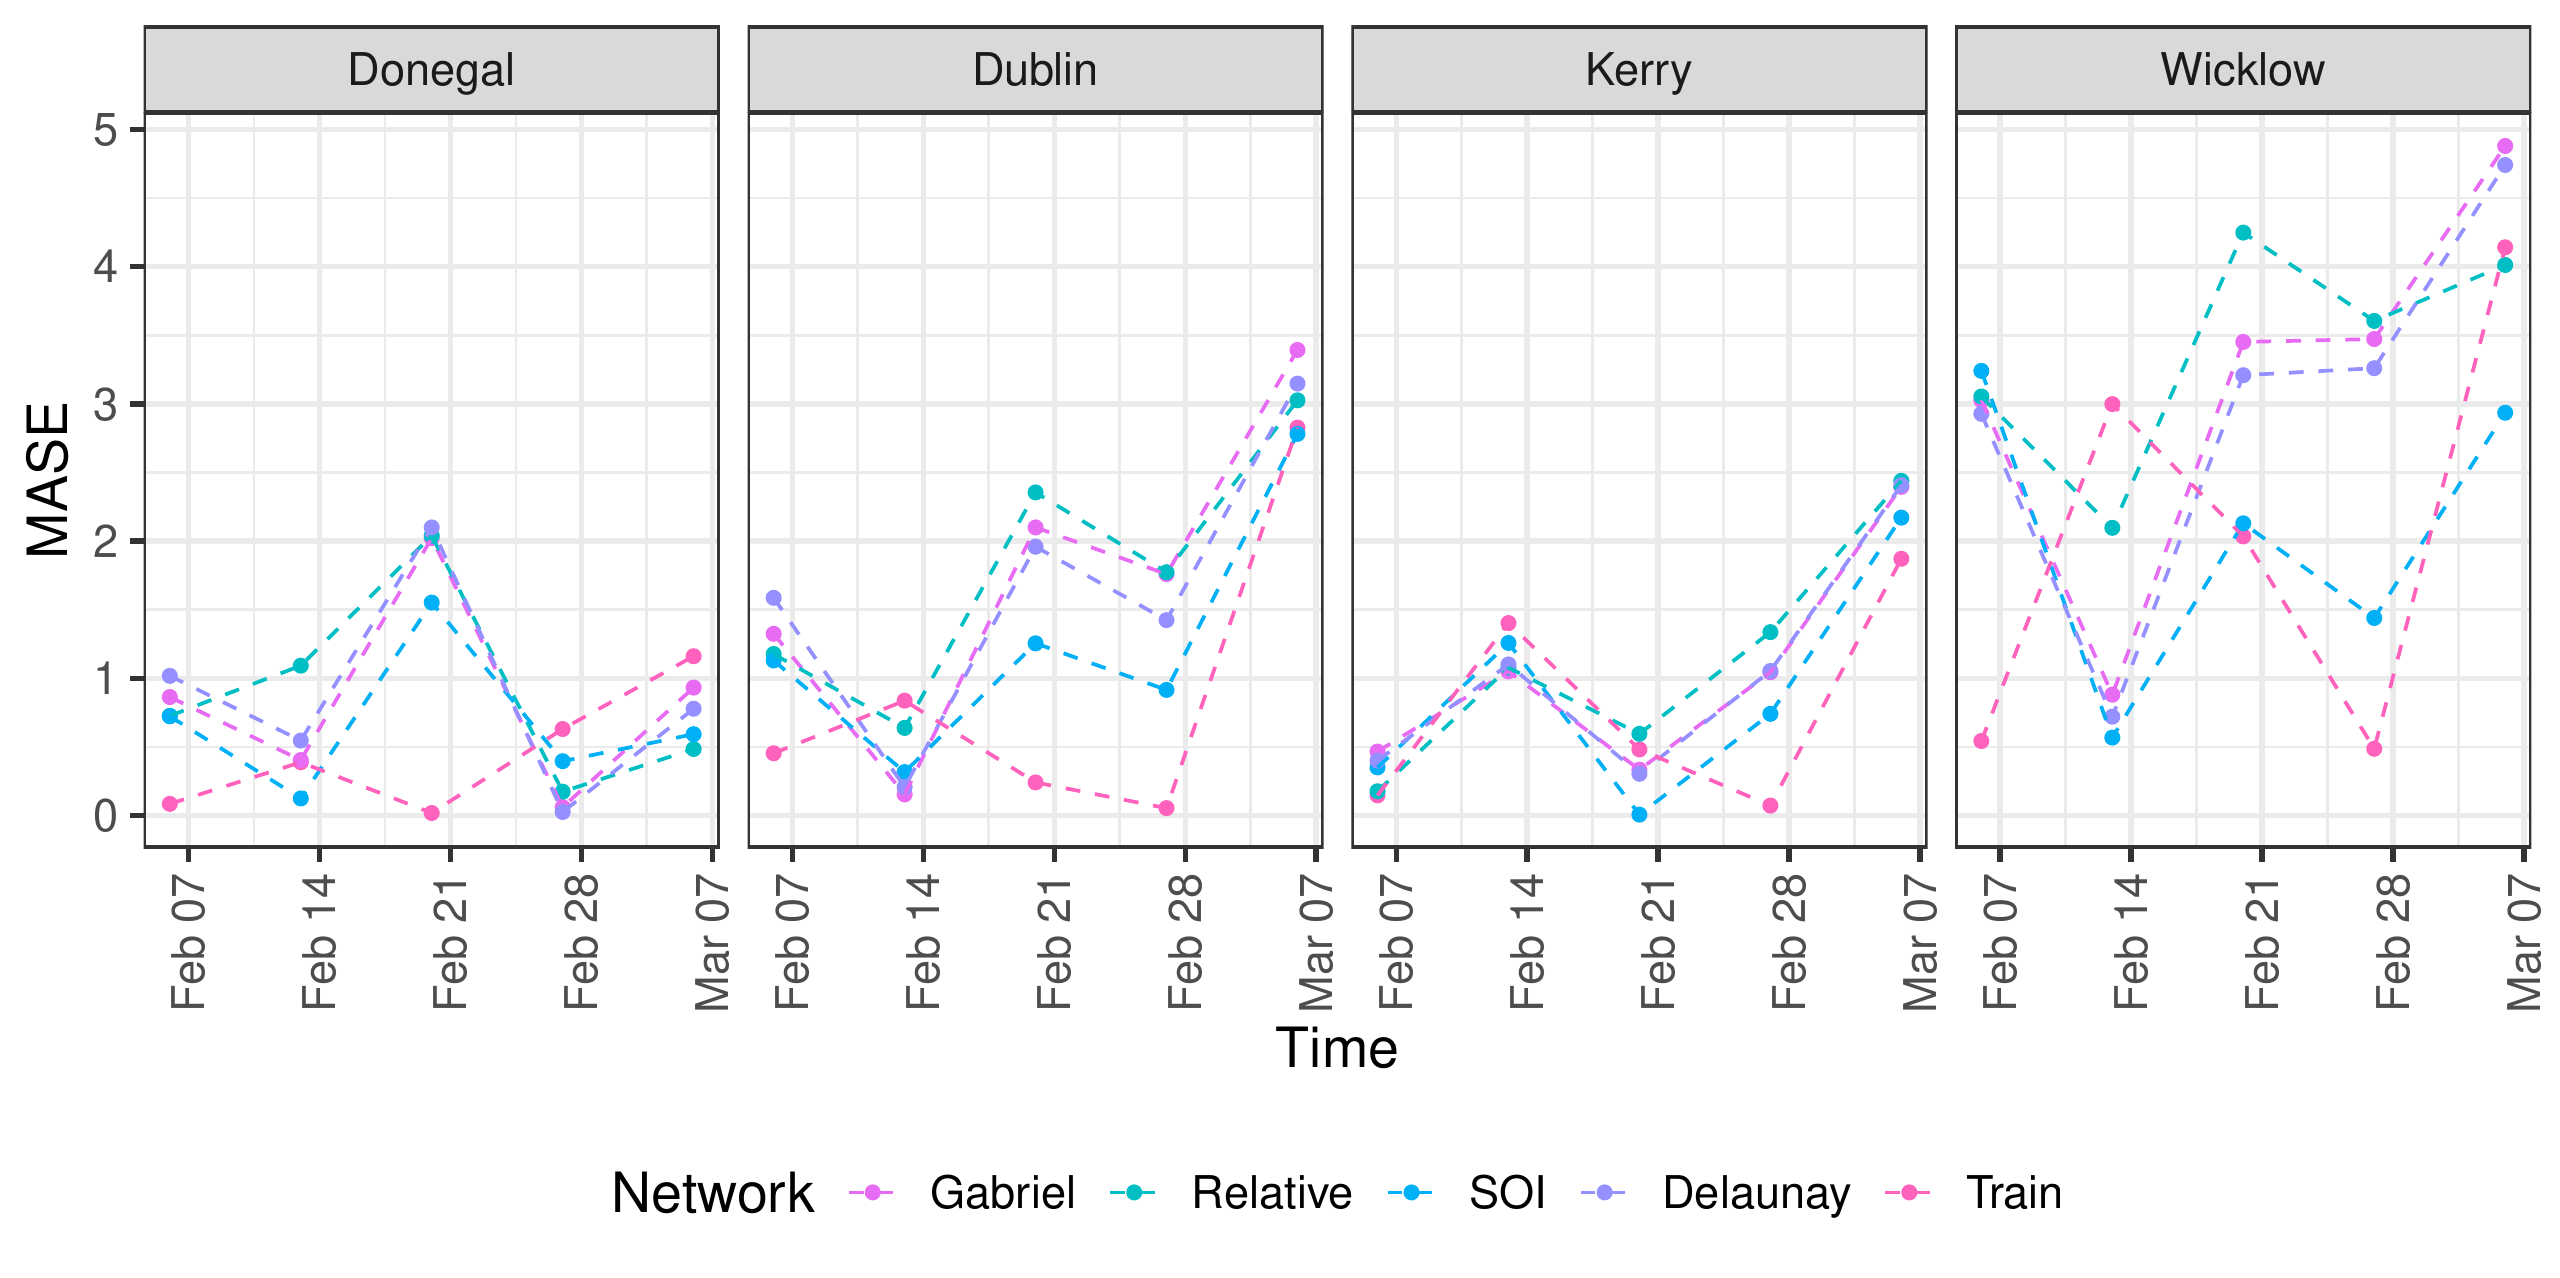}
  \caption{\textbf{Delaunay triangulation}, \textbf{Gabriel}, \textbf{Relative neighbourhood}, \textbf{SOI} and \textbf{Railway-based} network}
\end{subfigure}
\begin{subfigure}{\textwidth}
  \centering
  \includegraphics[width = 0.7\textwidth]{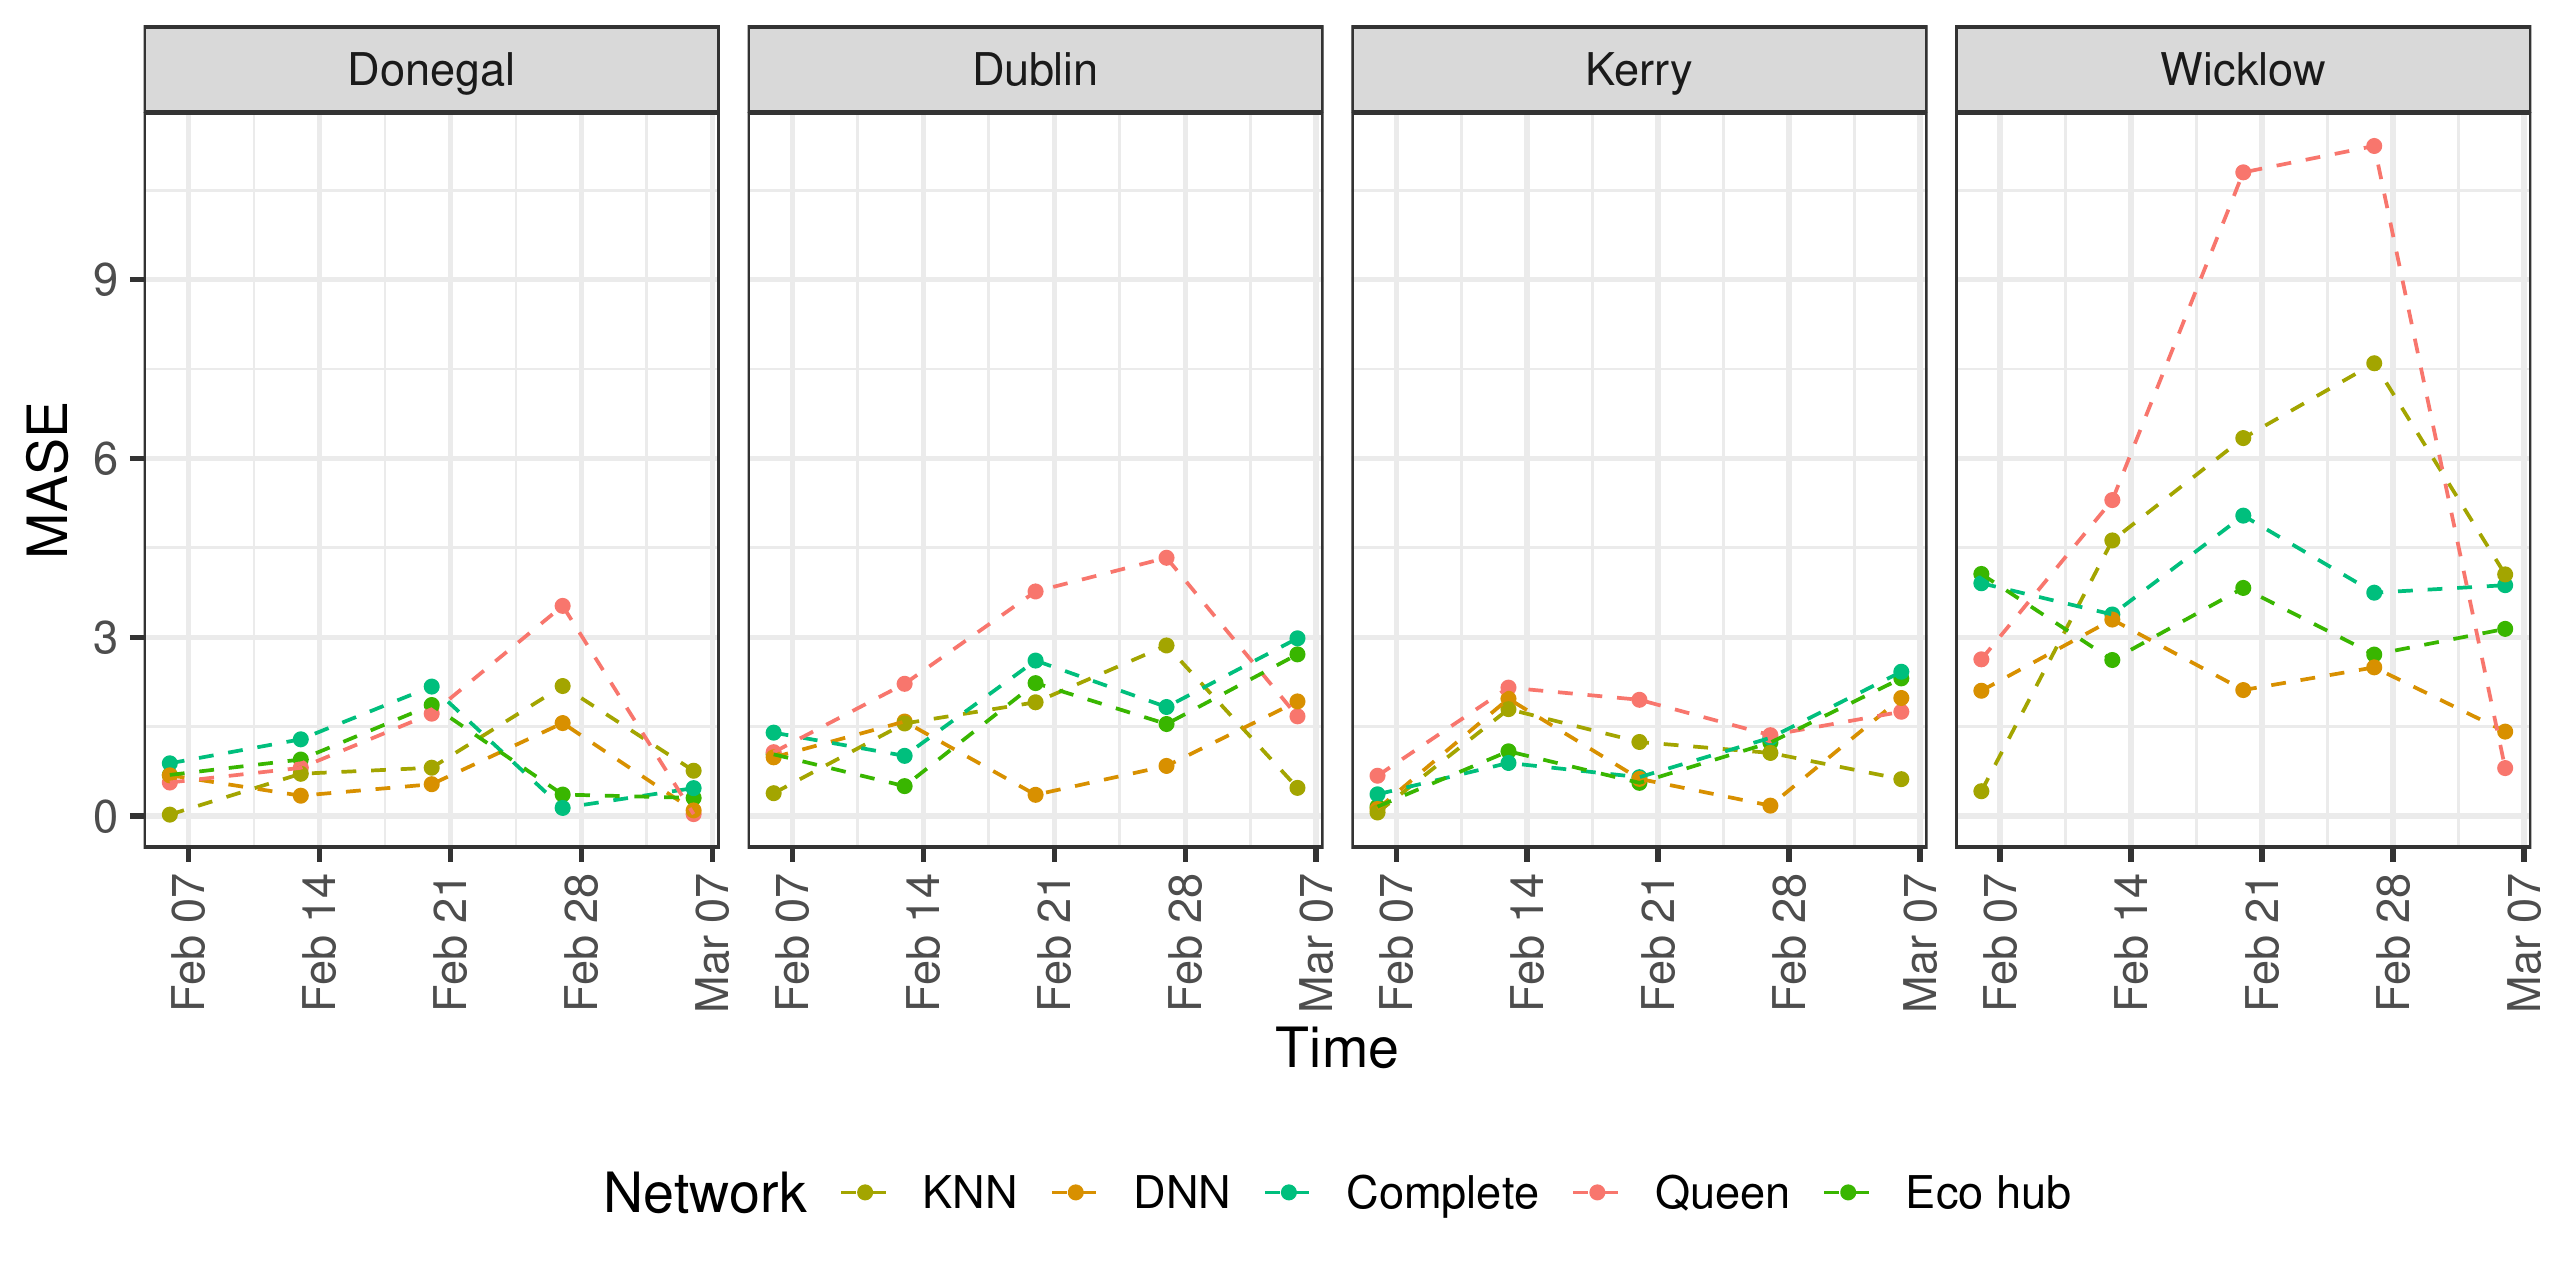}
  \caption{\textbf{KNN}, \textbf{DNN}, \textbf{Complete}, \textbf{Queen's contiguity} and \textbf{Economic hub} network}
\end{subfigure}
\caption{MASE values for data subset 4}
\label{fig:mase_subset_4}
\end{figure}

For data set 5, the Gabriel network performs particularly well. 
\begin{figure}[h!]
\centering
\begin{subfigure}{\textwidth}
  \centering
  \includegraphics[width = 0.7\textwidth]{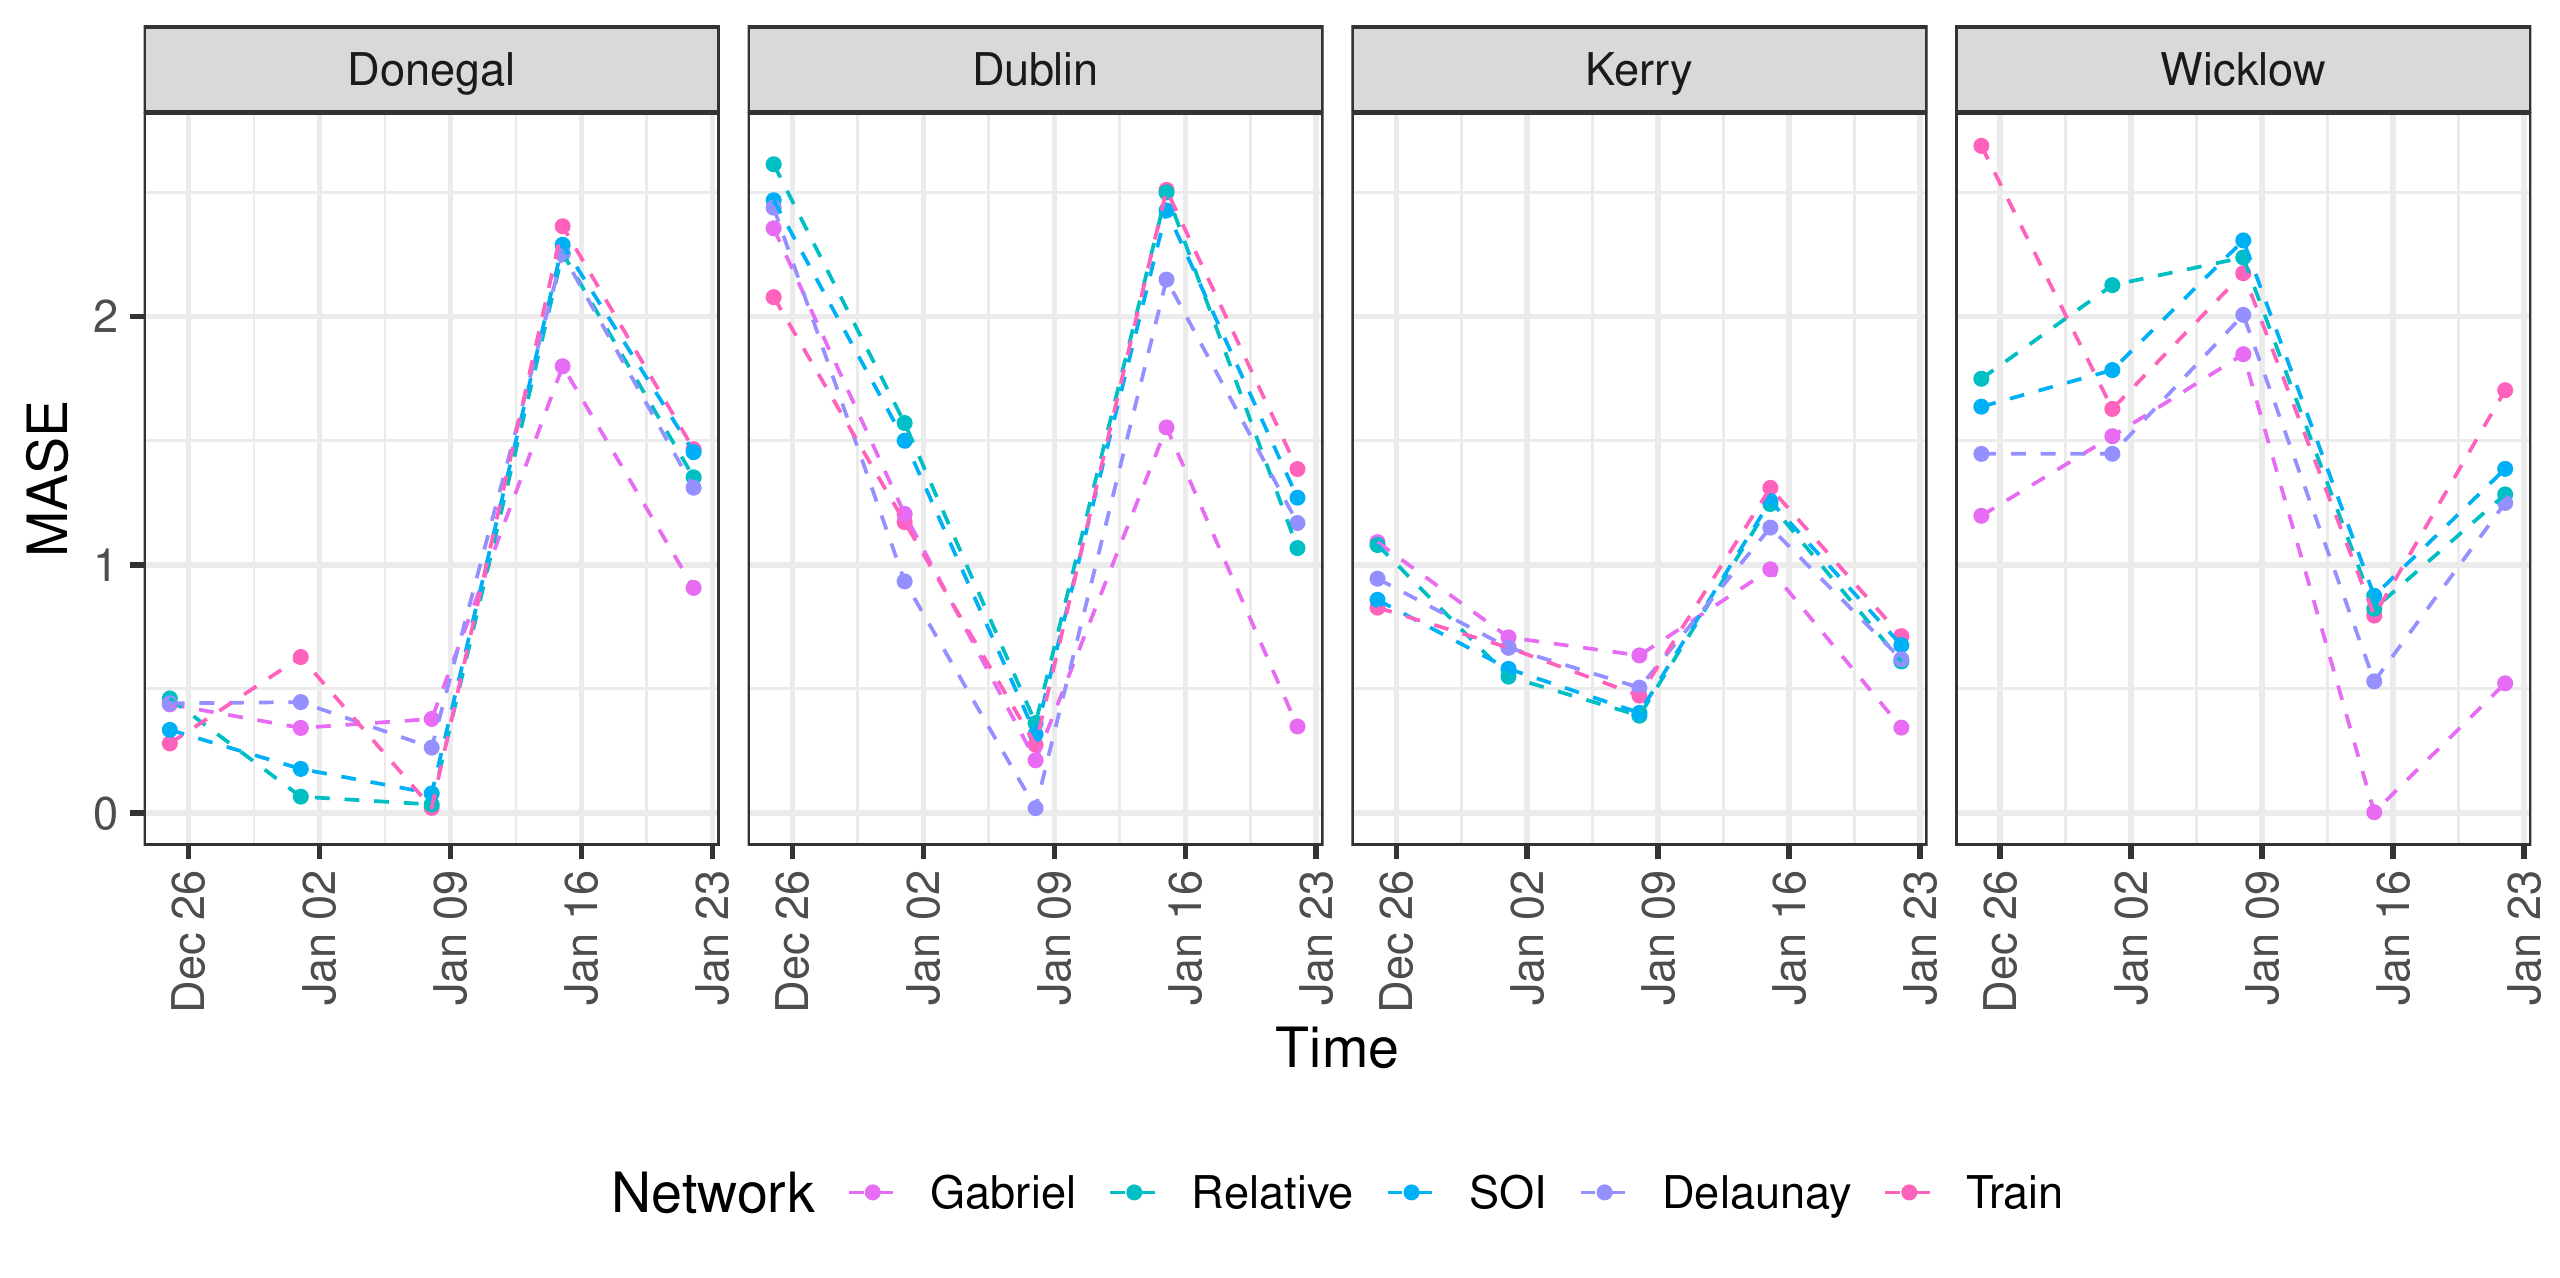}
  \caption{\textbf{Delaunay triangulation}, \textbf{Gabriel}, \textbf{Relative neighbourhood}, \textbf{SOI} and \textbf{Railway-based} network}
\end{subfigure}
\begin{subfigure}{\textwidth}
  \centering
  \includegraphics[width = 0.7\textwidth]{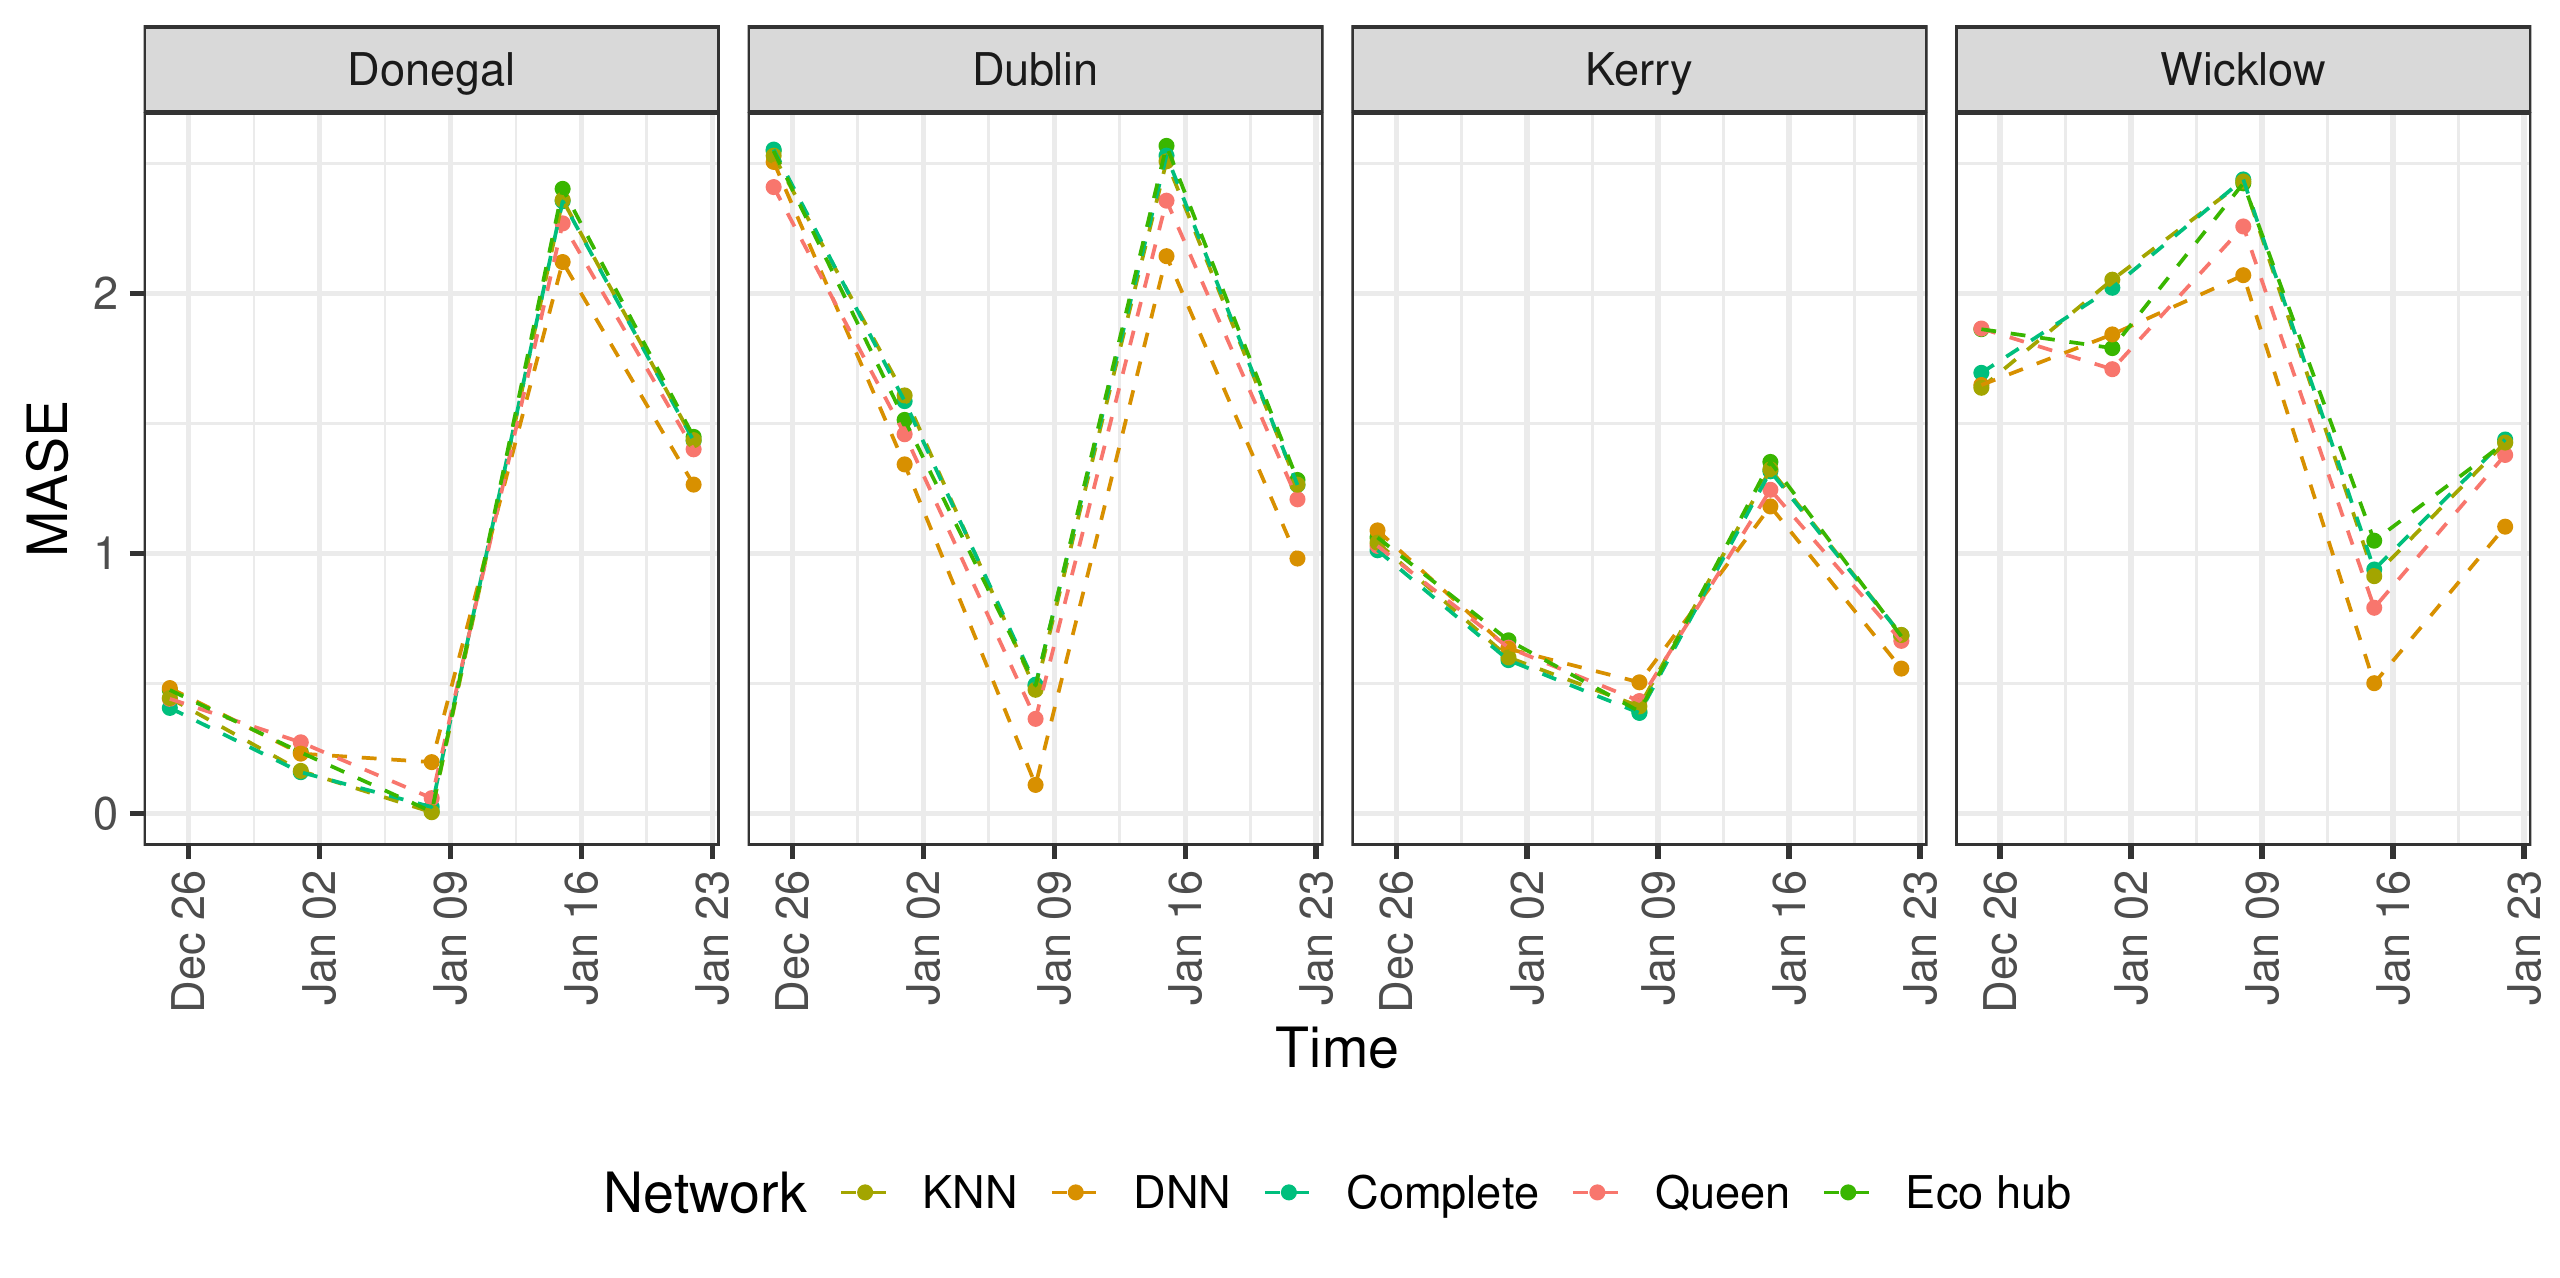}
  \caption{\textbf{KNN}, \textbf{DNN}, \textbf{Complete}, \textbf{Queen's contiguity} and \textbf{Economic hub} network}
\end{subfigure}
\caption{MASE values for data subset 5}
\label{fig:mase_subset_5}
\end{figure}

The QQ plots for the residuals of the optimal GNAR model for each data subset imply Non-Gaussian error, in particular around the boundaries.
The Kolmogorov-Smirnov test disproves this observation only for dataset 1 ($p = 0.3261$).
\begin{figure}[h!]
\centering
\subcaptionbox{Subset 1}{\includegraphics[width=0.3\textwidth]{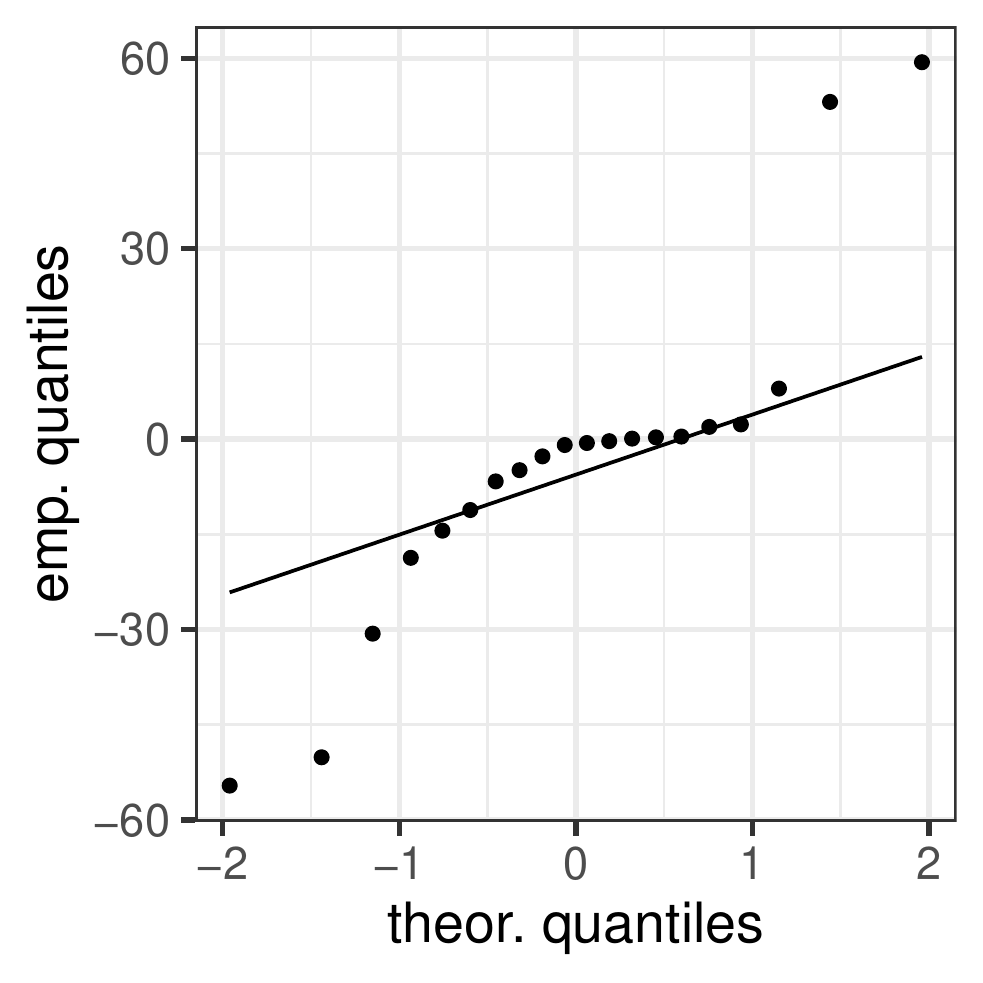}}%
\hspace{1em}
\subcaptionbox{Subset 2}{\includegraphics[width=0.3\textwidth]{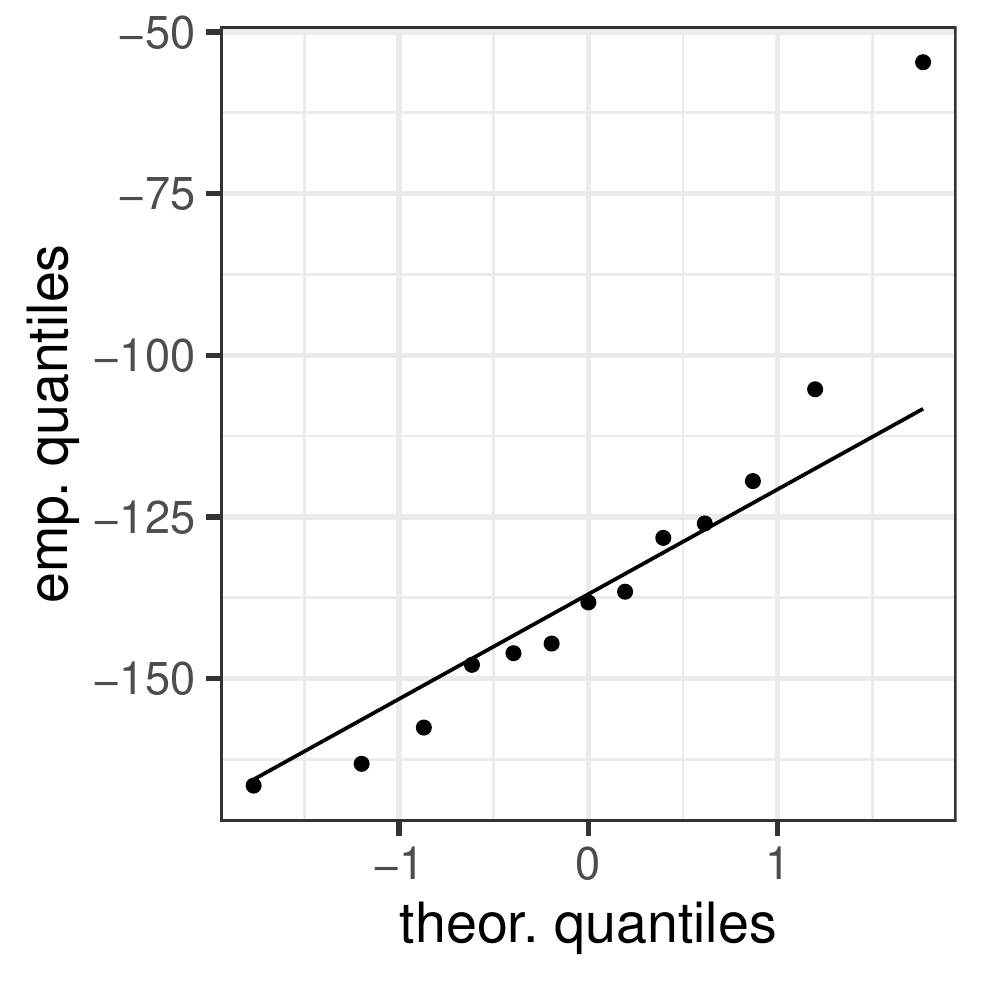}}%
\hspace{1em}
\subcaptionbox{Subset 3}{\includegraphics[width=0.3\textwidth]{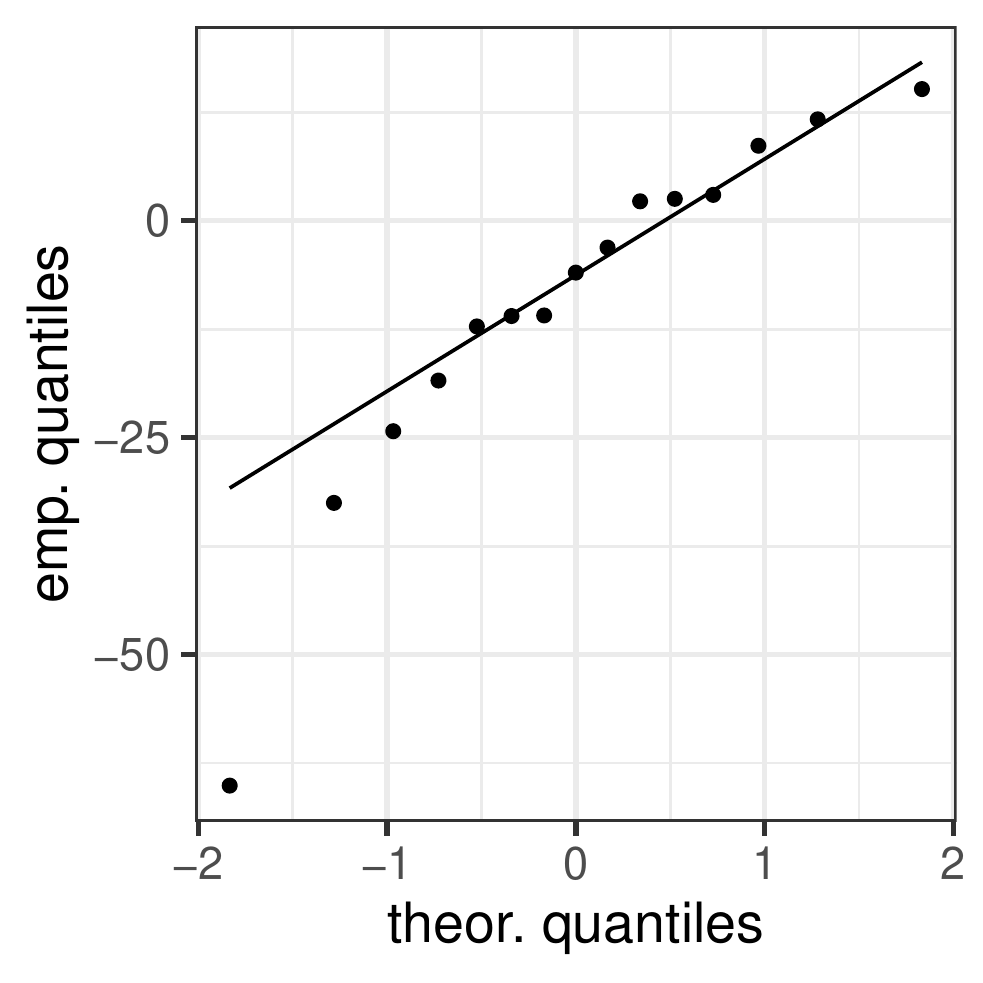}}%
\\
\subcaptionbox{Subset 4}{\includegraphics[width=0.3\textwidth]{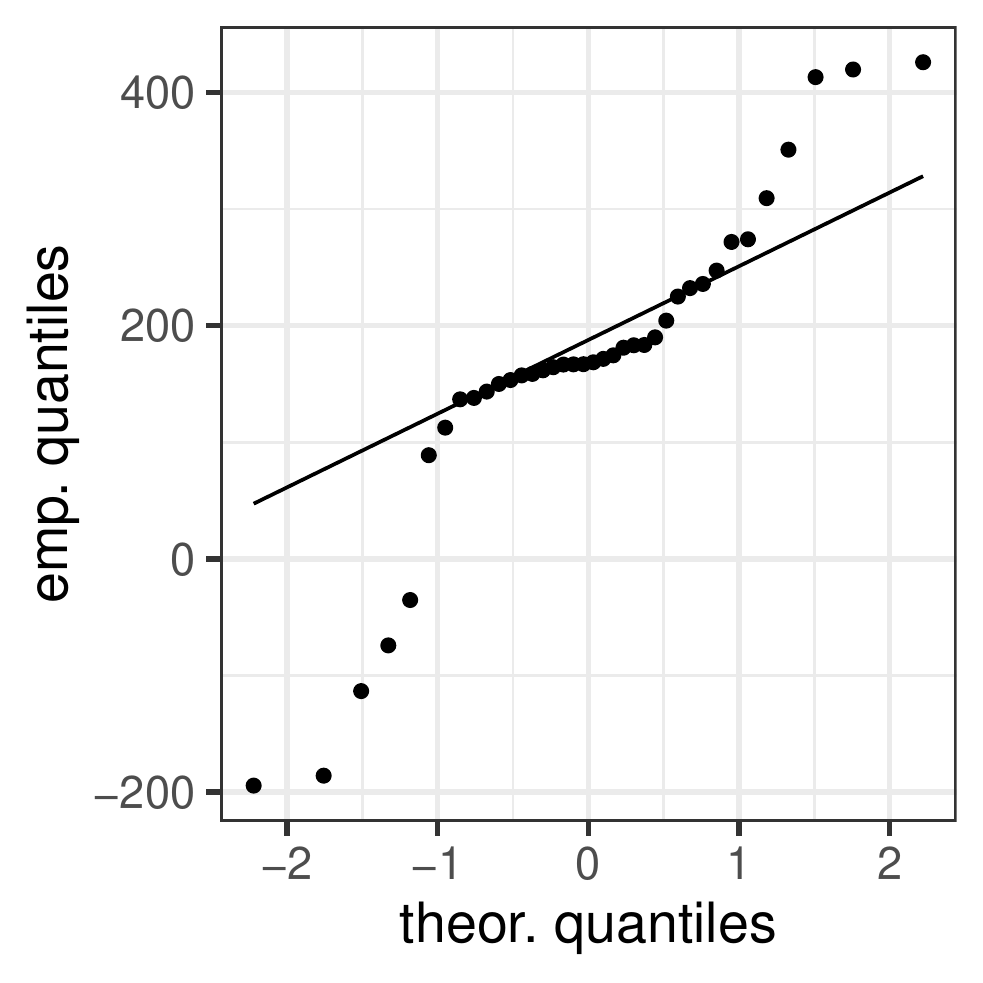}}%
\hspace{1em}
\subcaptionbox{Subset 5}{\includegraphics[width=0.3\textwidth]{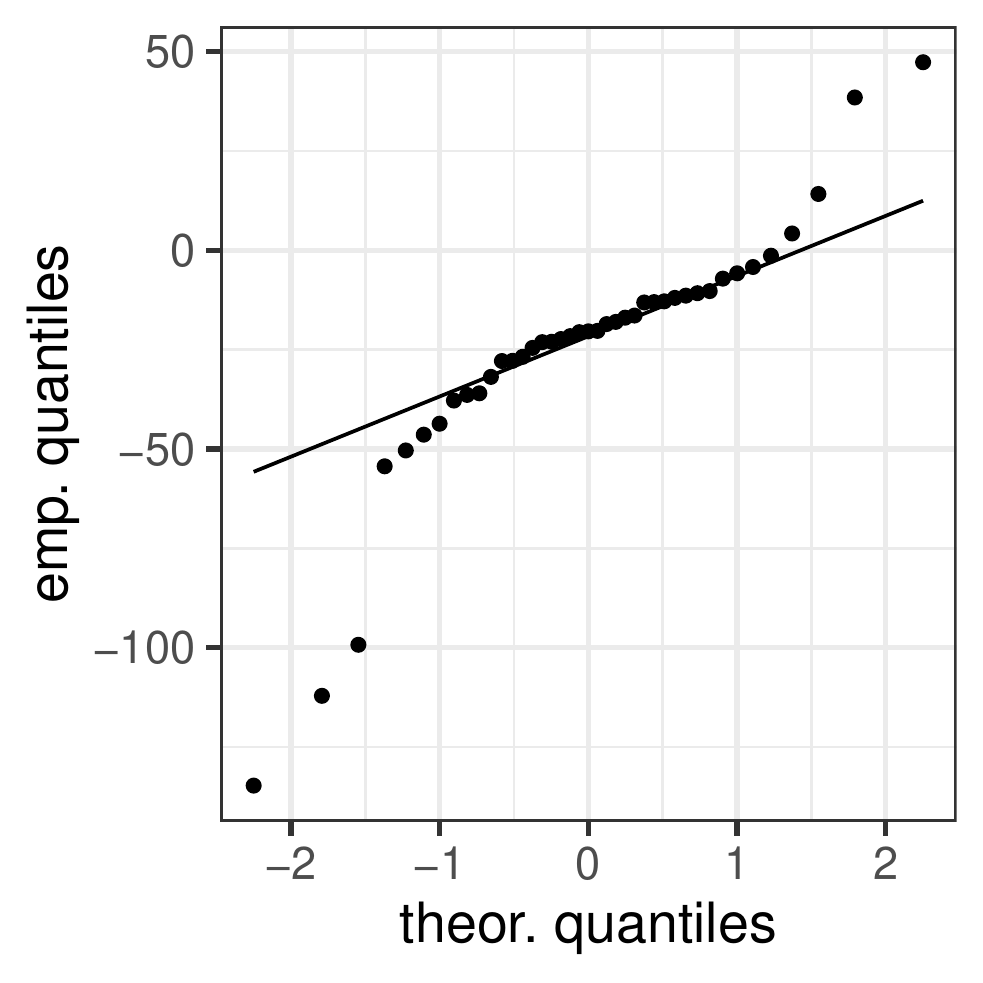}}%
\caption{QQ plot for the residuals from the best performing GNAR model and network for dataset 1-5; shown for county Dublin only}
\label{fig:qq_subsets_dublin}
\end{figure}

\clearpage

\section{Additional Information: Influence of COVID-19 restrictions}
\label{app:development_coefficients}
The following plots analyse how the parameter values for the best performing GNAR model for each network develop throughout the COVID-19 pandemic. 
In particular, we are interested if the effectiveness of regulations, introduced to contain COVID-19, is mirrored by smaller values for $\beta$-order coefficients as a representation of decreasing spatial dependence. 
This hypothesis is not supported. 
While the estimates for the $\beta$-order coefficients do not systematically decrease in value, their do decrease in absolute value for dataset 1 and 3 compared to datasets 2, 4 and 5. 
This indicates a weaker spatial dependence in COVID-19 ID for pandemic periods in which inter-county travel was restricted.
\begin{figure}[h!]
\centering
\begin{subfigure}{\textwidth}
  \centering
  \includegraphics[scale = 0.4]{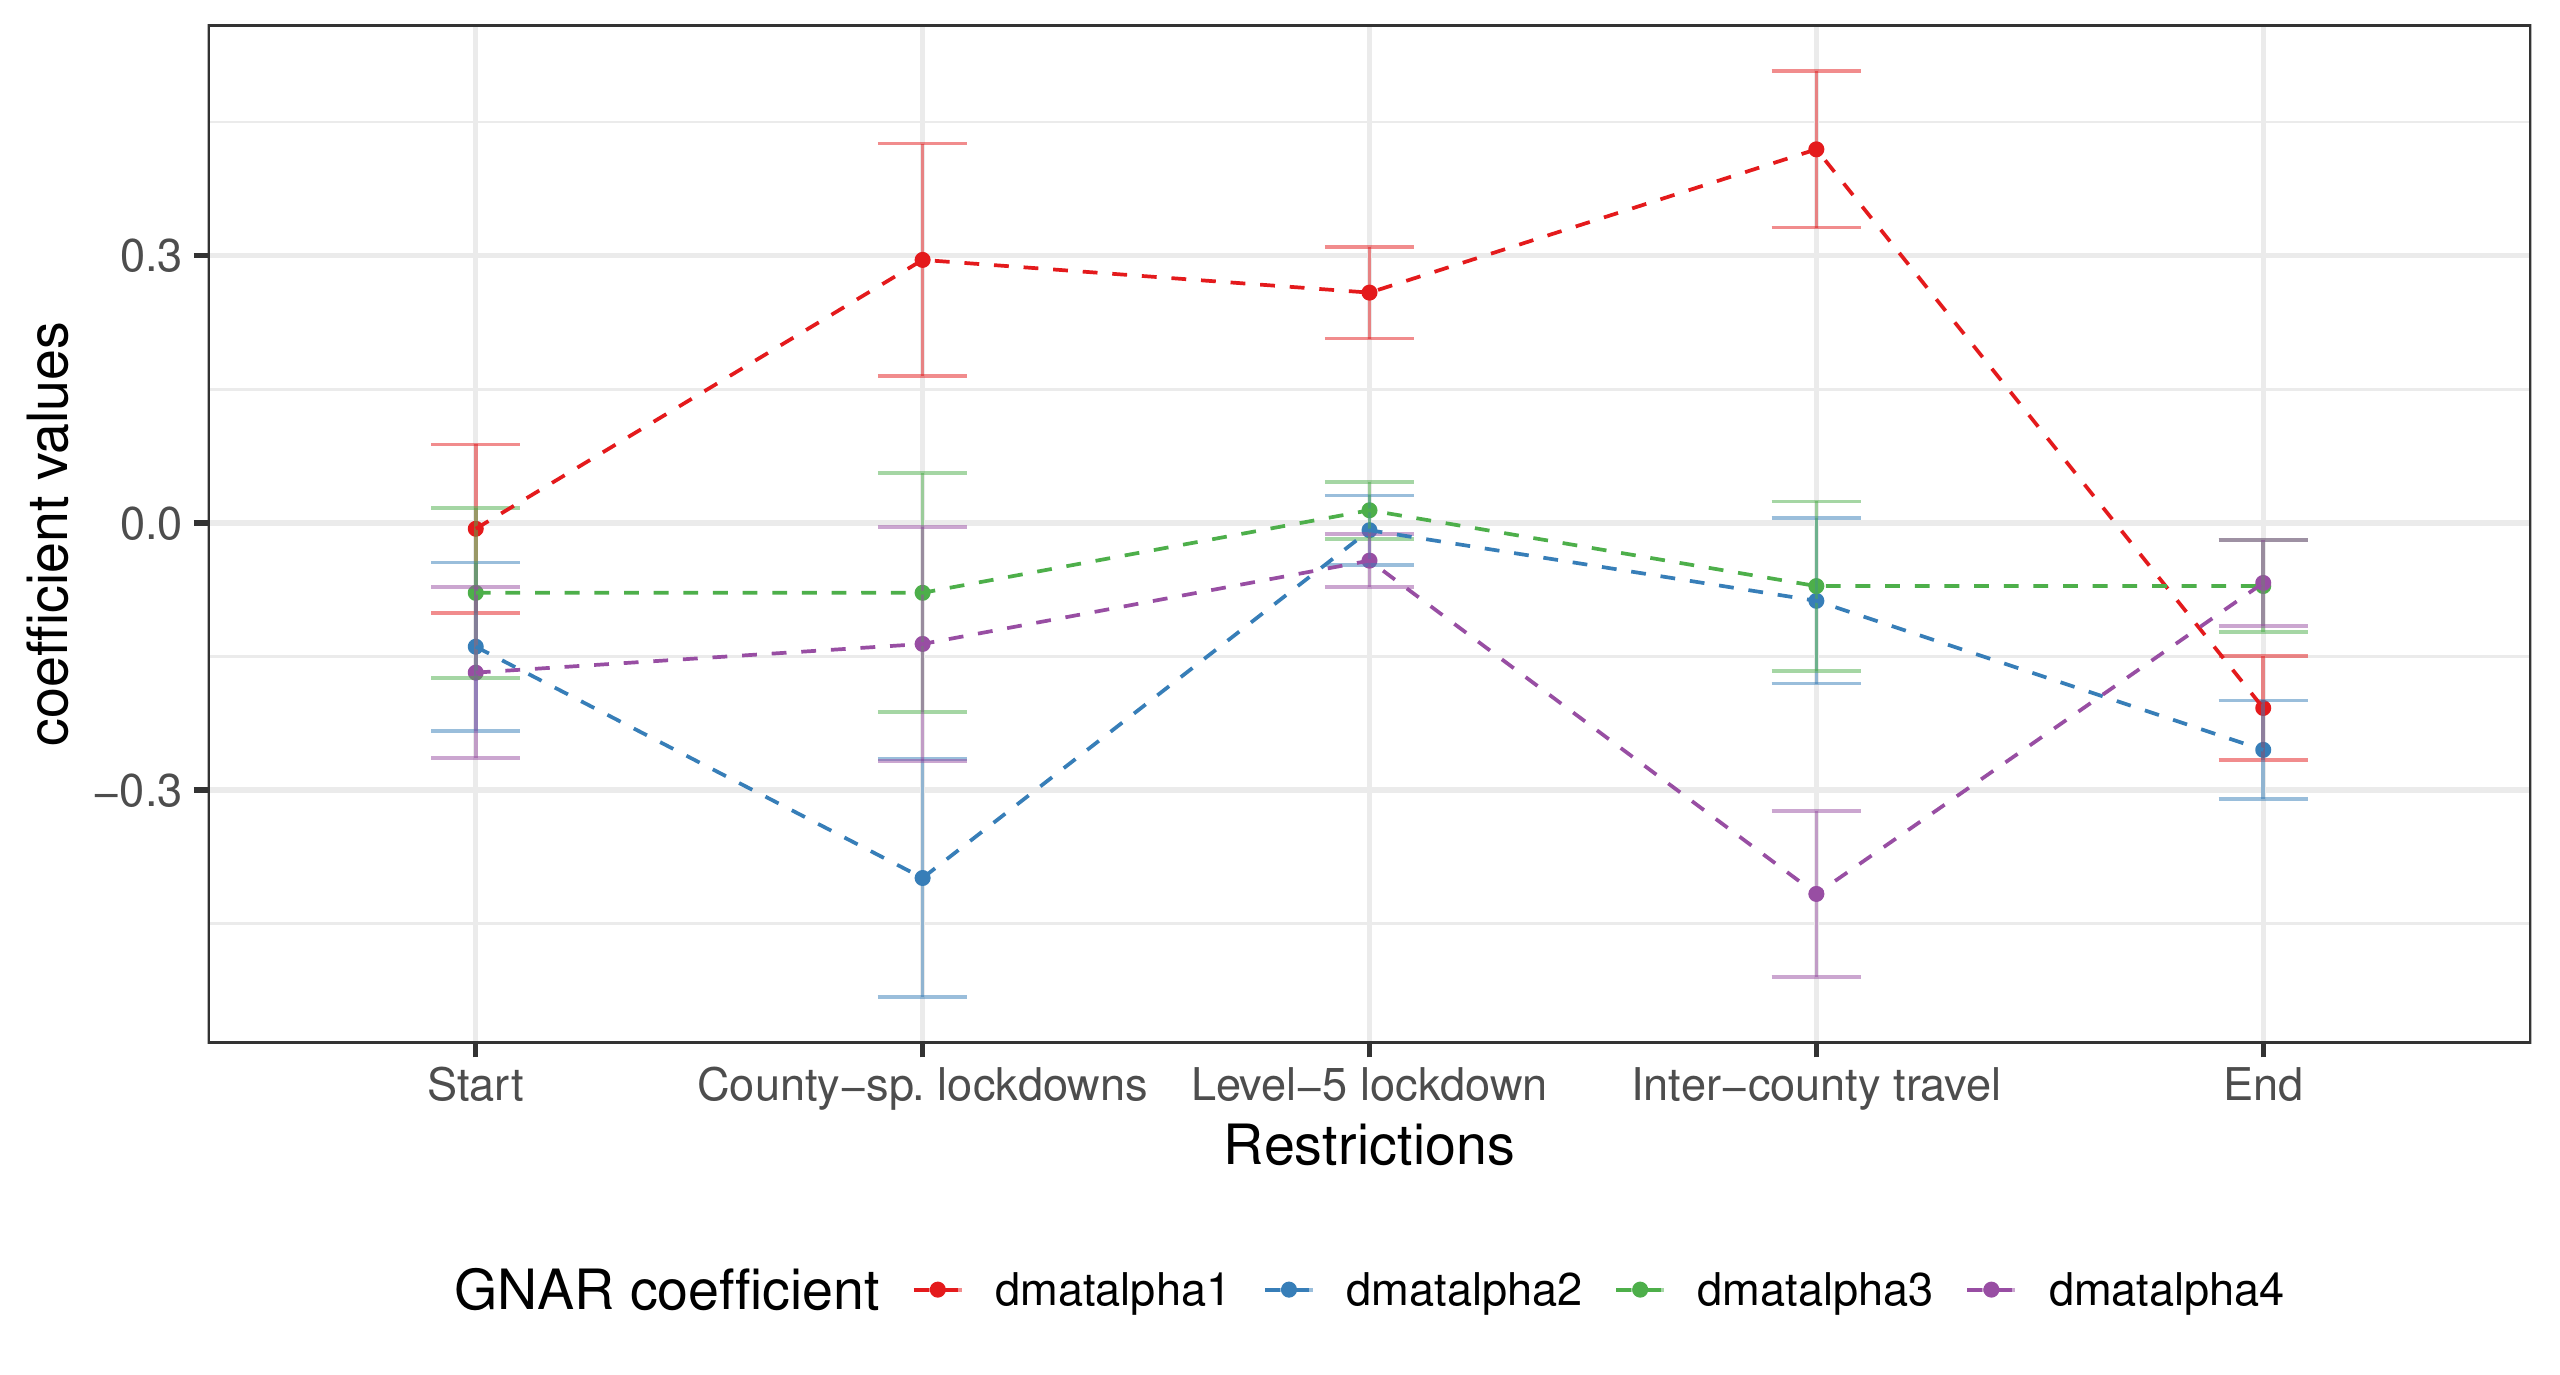}
  \caption{$\alpha$-order}
\end{subfigure}
\begin{subfigure}{\textwidth}
  \centering
  \includegraphics[scale = 0.4]{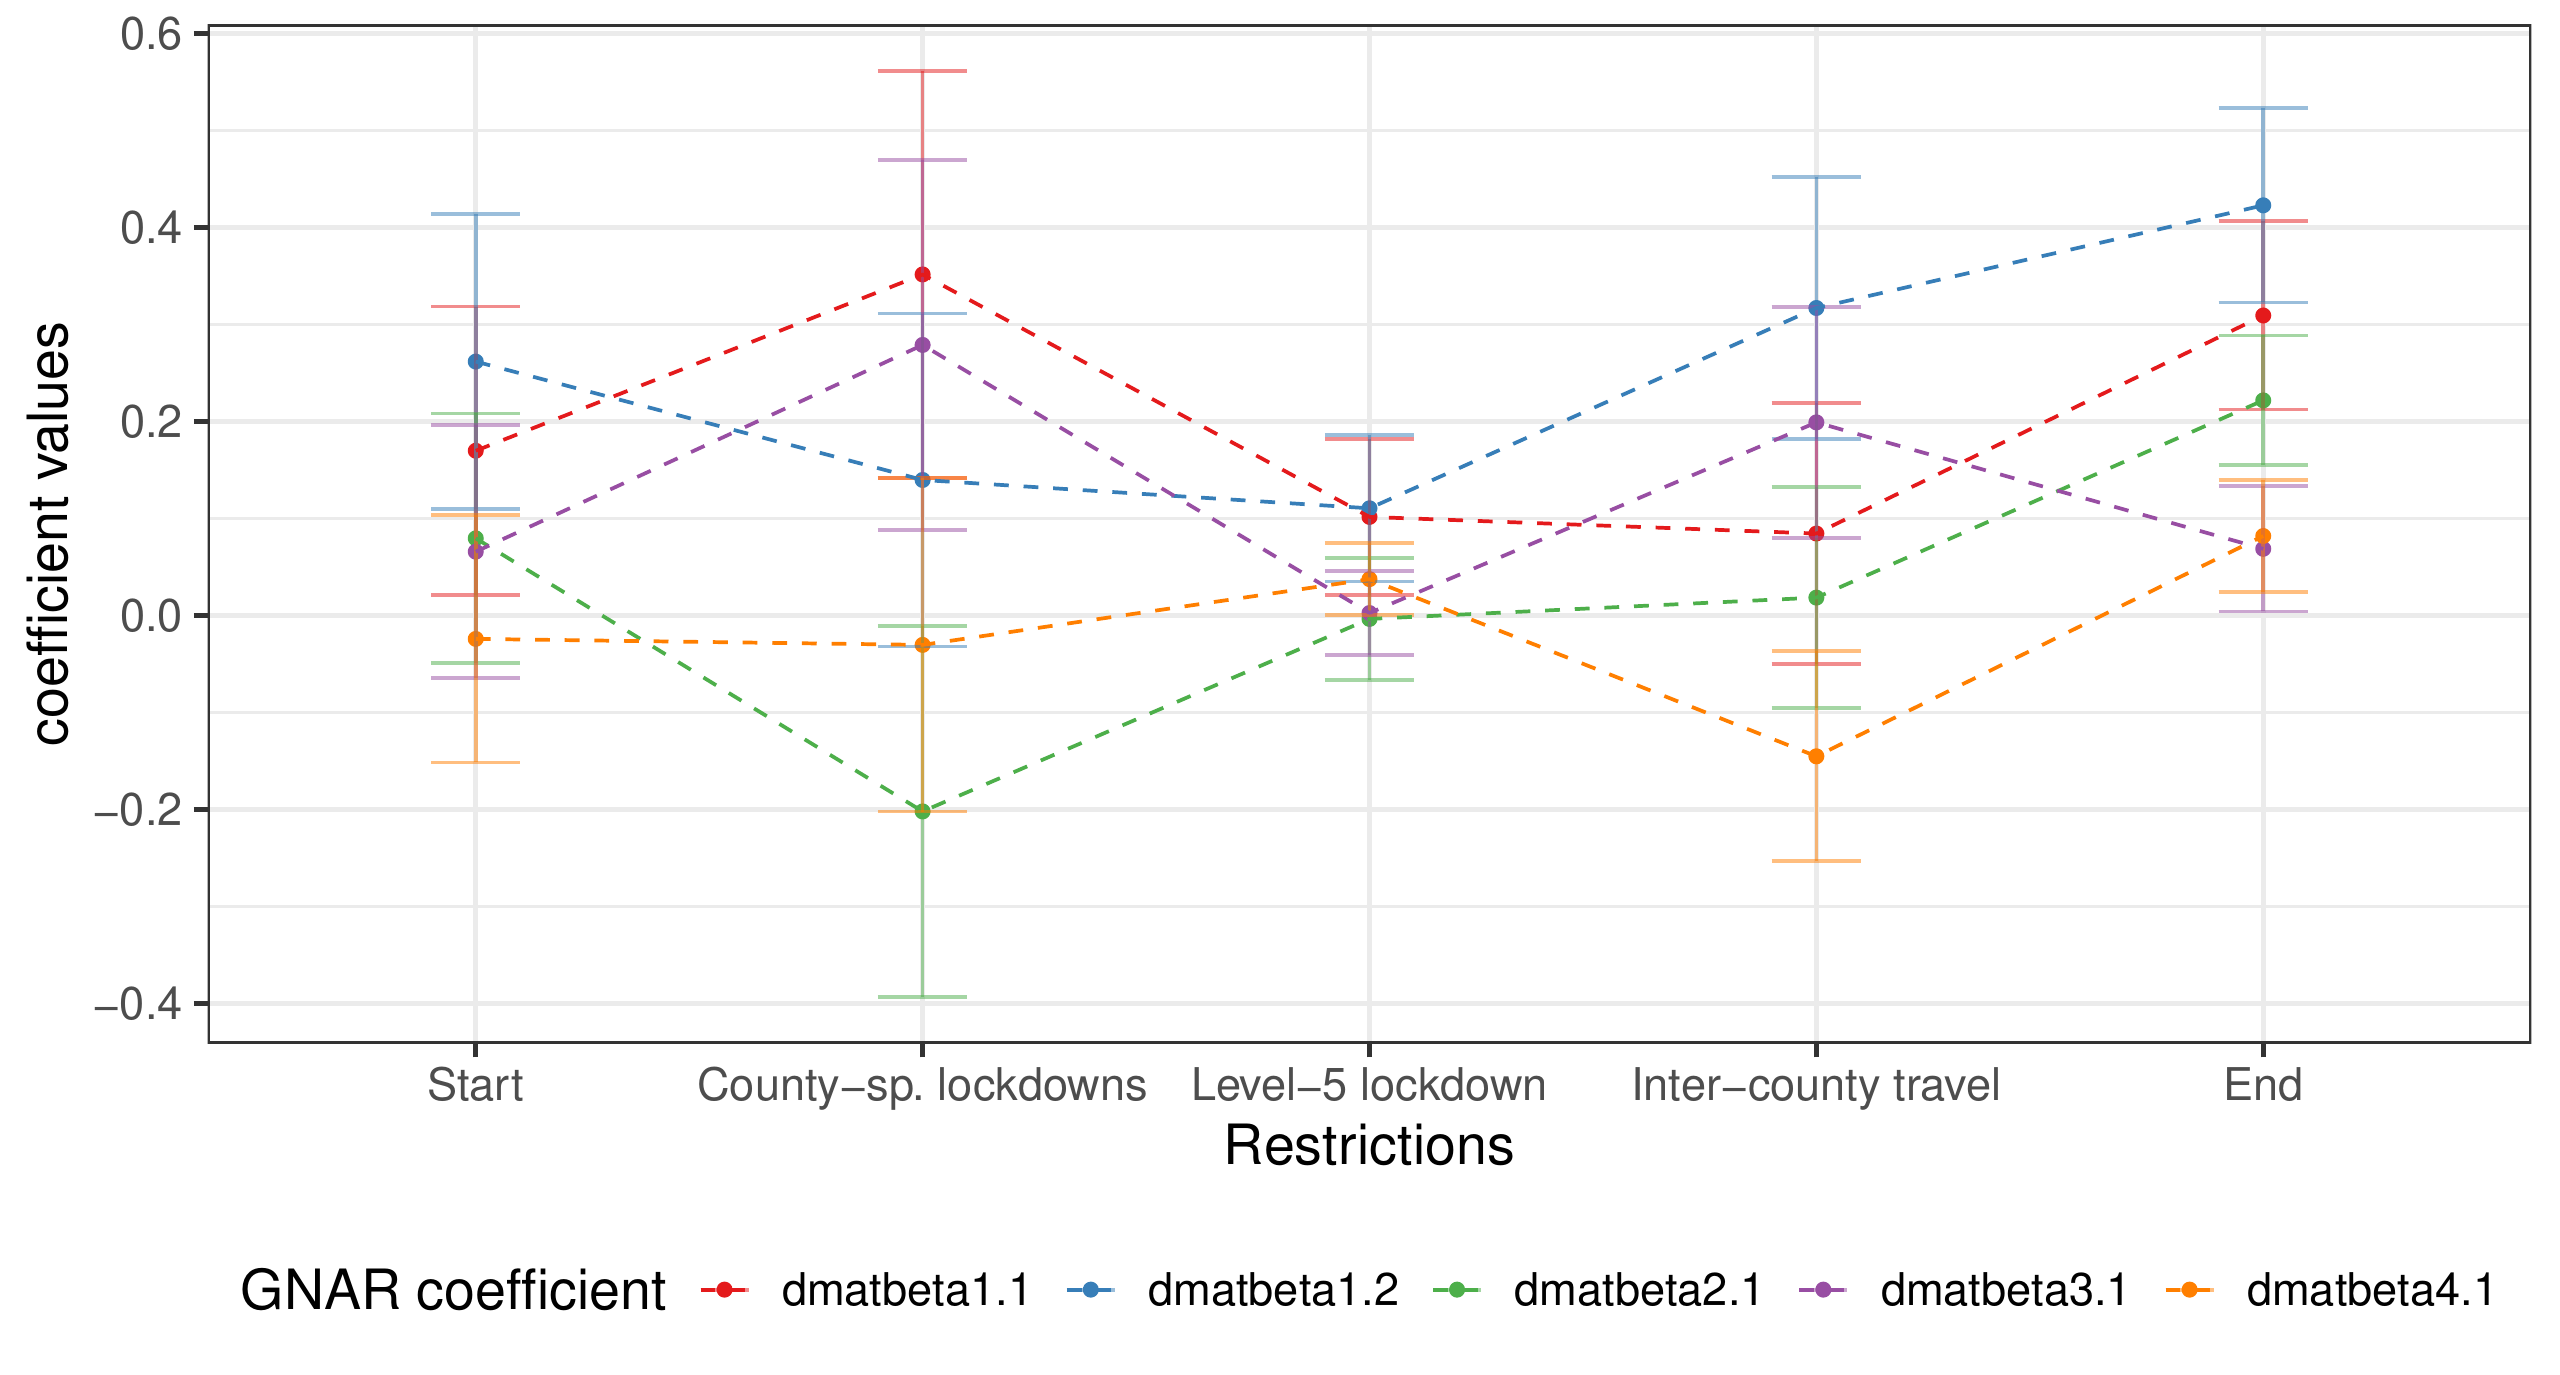}
  \caption{$\beta$-order}
\end{subfigure}
\caption[Change in GNAR models coefficients for COVID-19 regulations for Gabriel network]{Change in coefficients for the global-$\alpha$ \code{GNAR(4,[2, 1, 1, 1])} model across COVID-19 regulations for the \textbf{Gabriel} network}
\label{fig:parameter_gabriel}
\end{figure}

\begin{figure}[h!]
\centering
\begin{subfigure}{\textwidth}
  \centering
  \includegraphics[scale = 0.4]{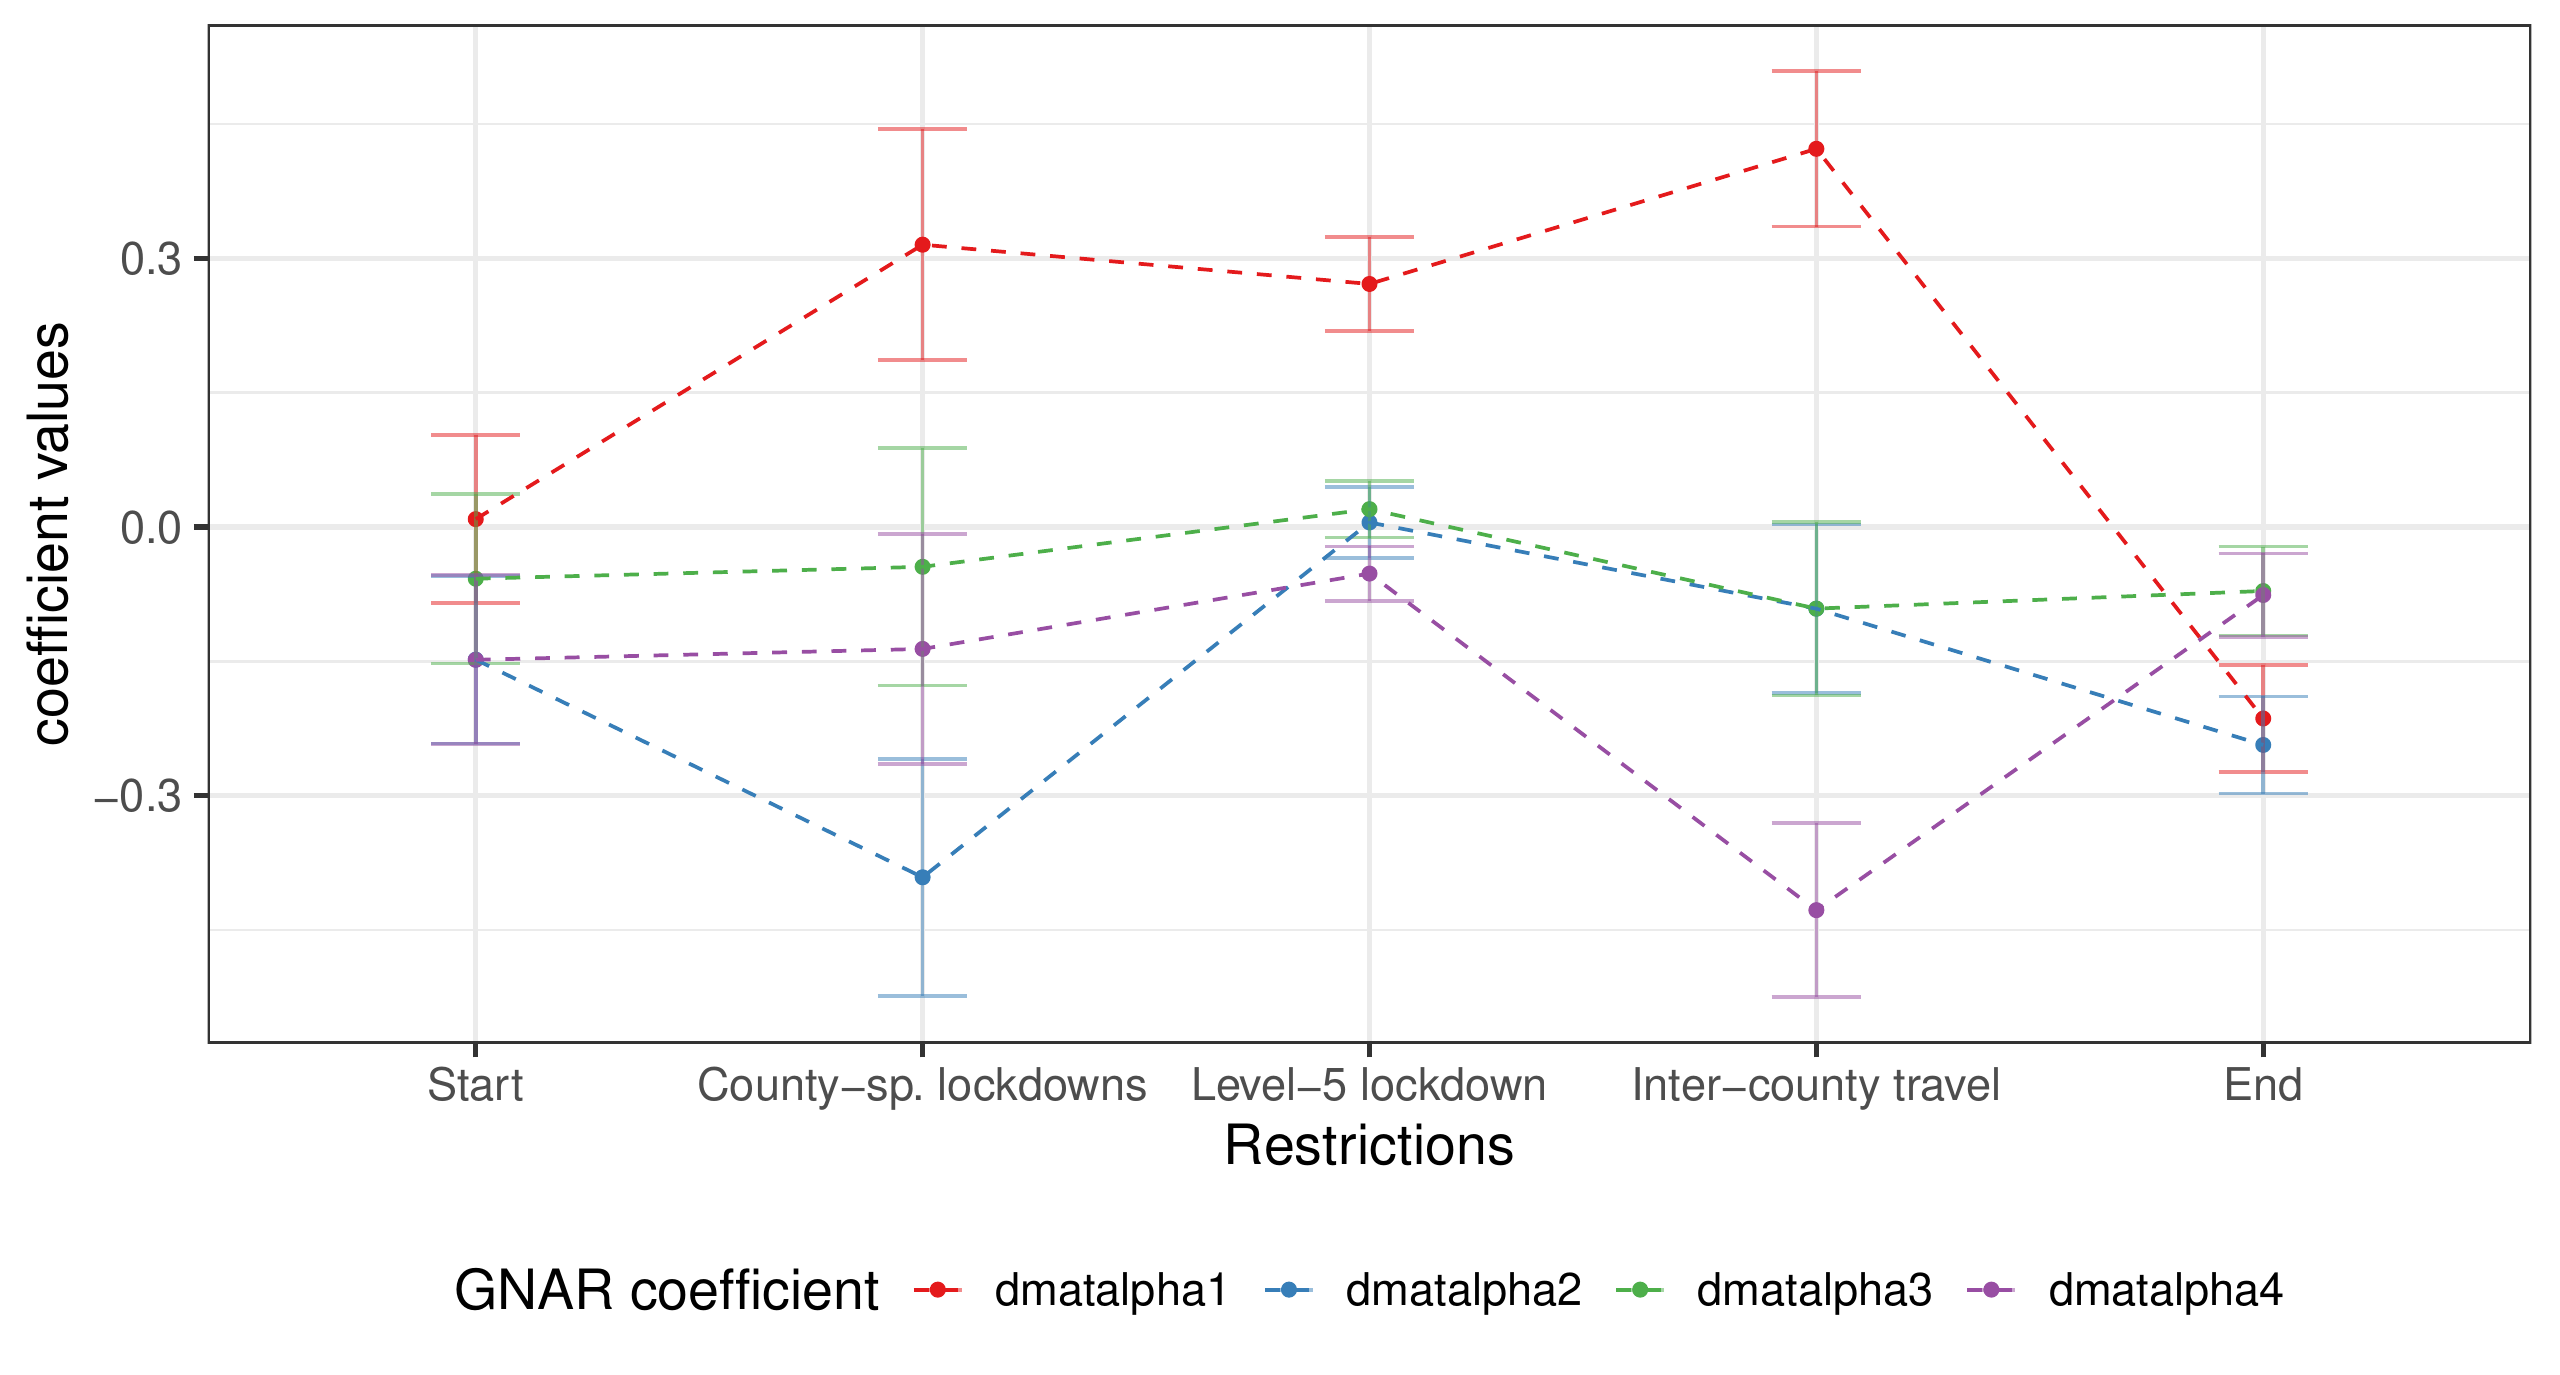}
  \caption{$\alpha$-order}
\end{subfigure}
\begin{subfigure}{\textwidth}
  \centering
  \includegraphics[scale = 0.4]{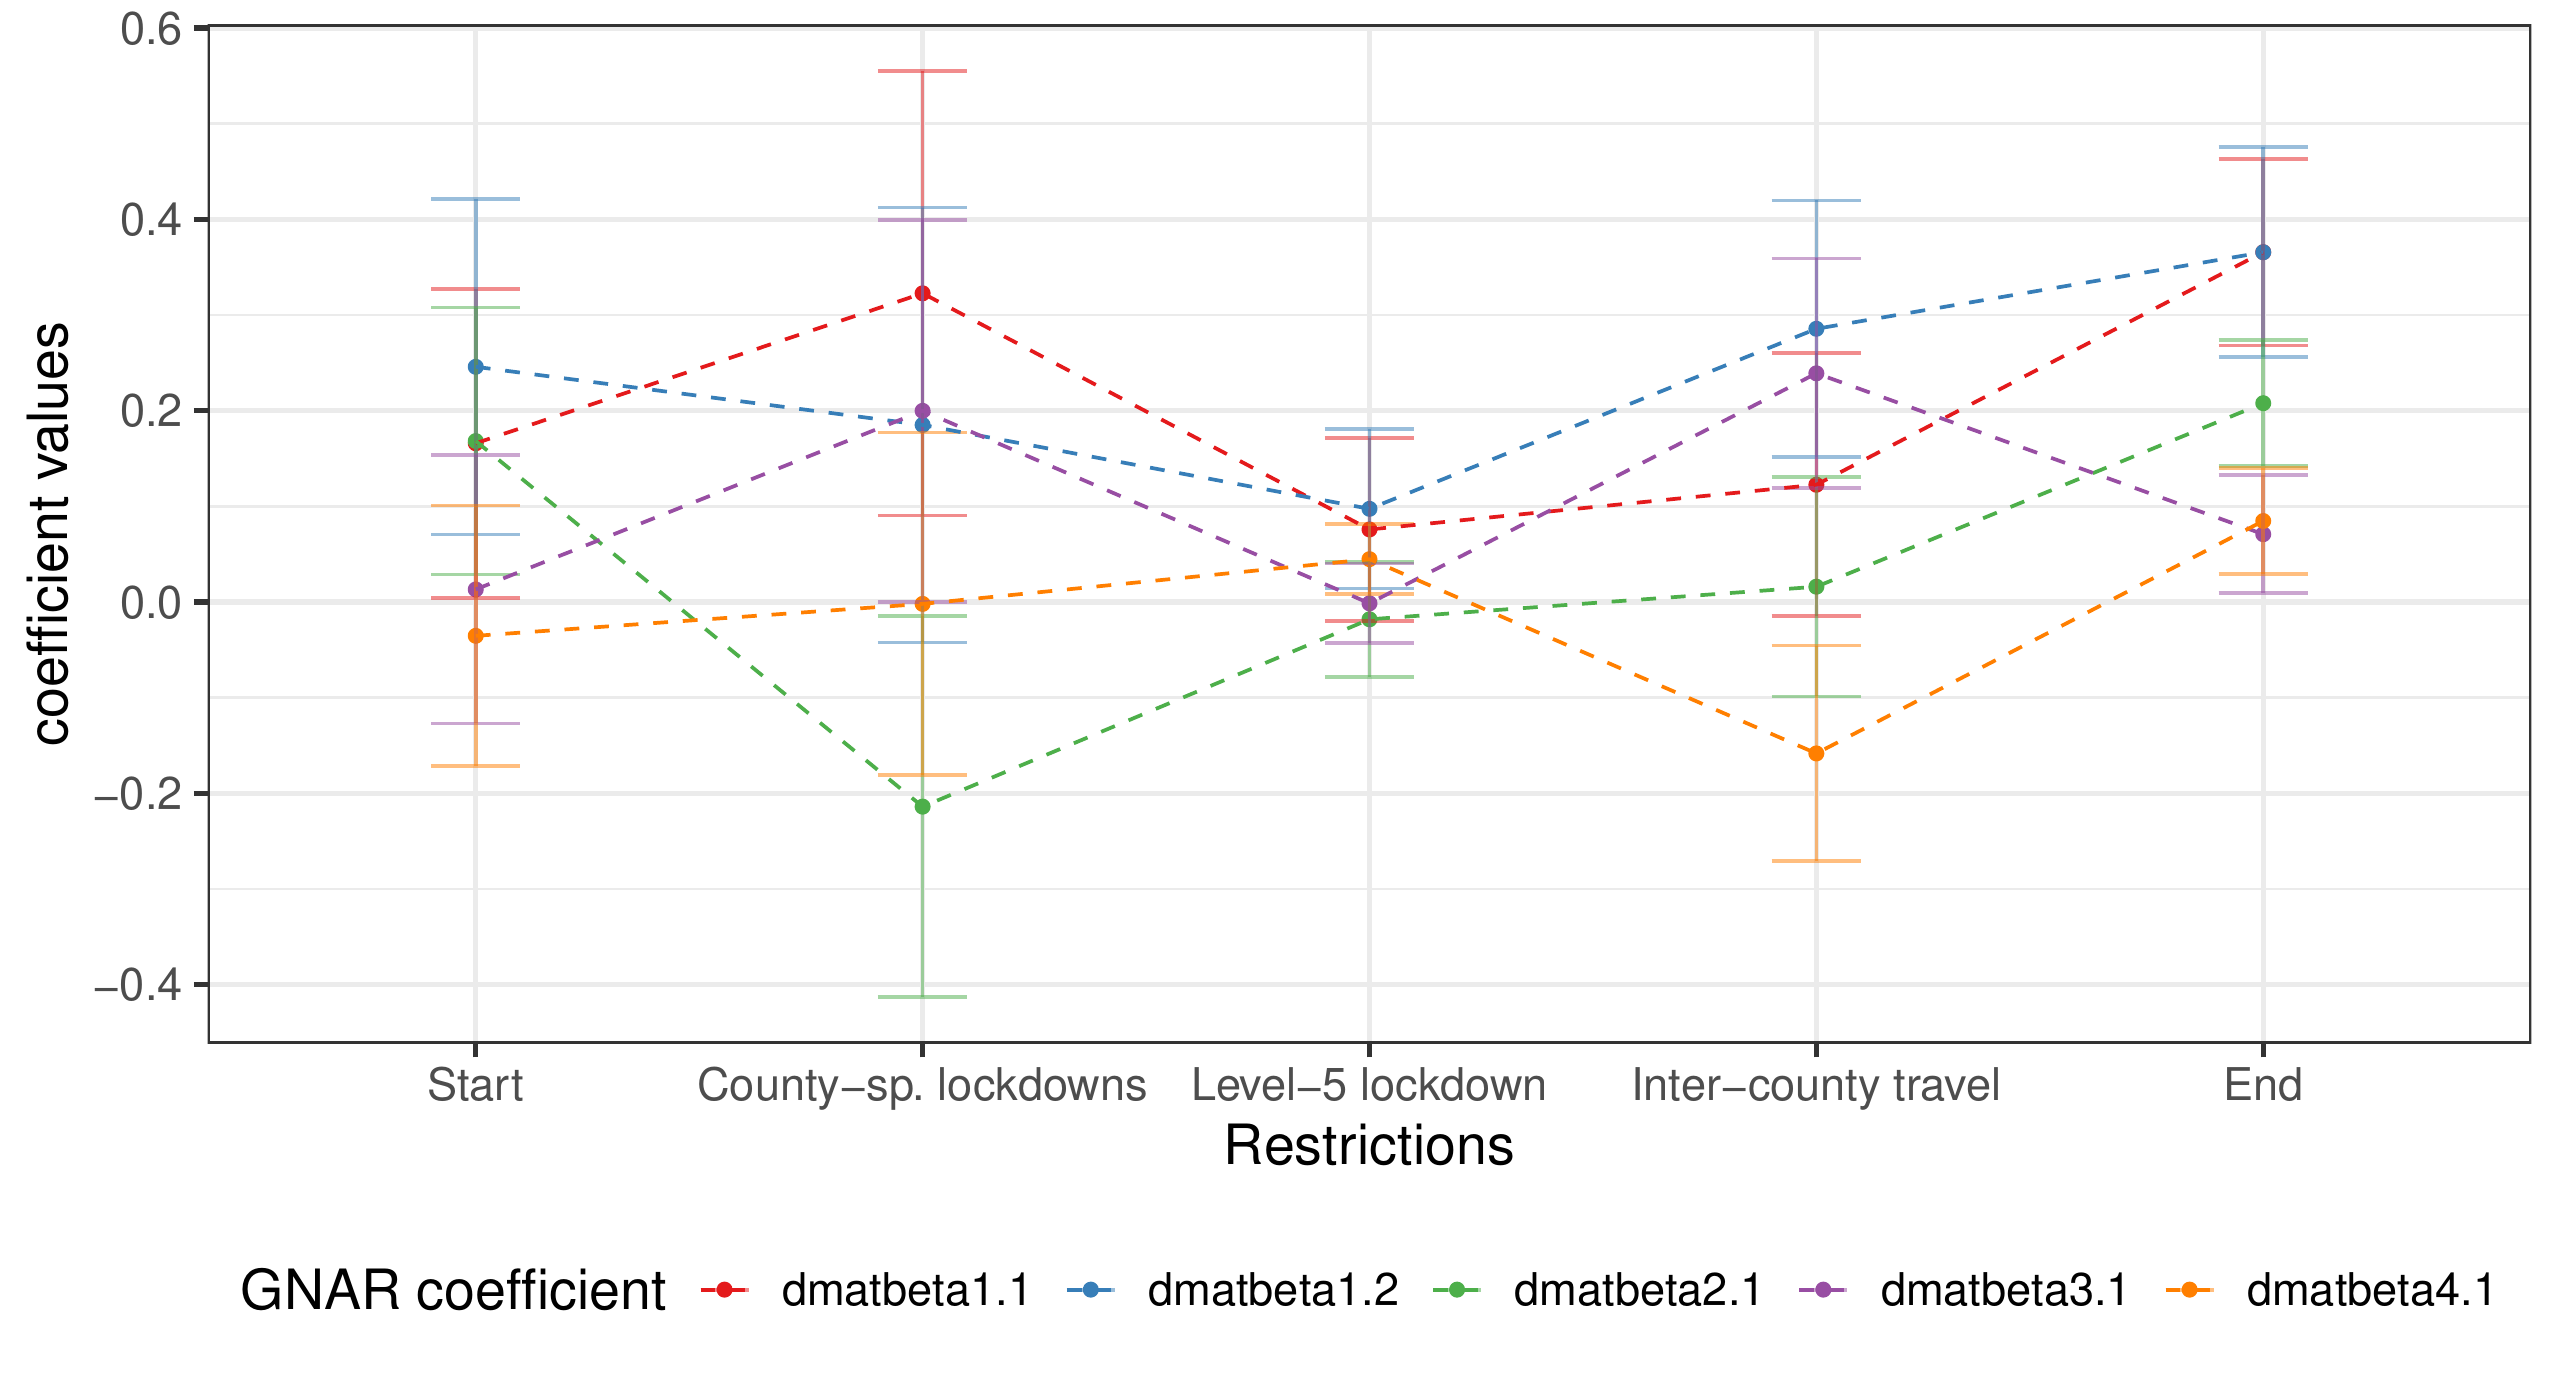}
  \caption{$\beta$-order}
\end{subfigure}
\caption[Change in GNAR model coefficients for COVID-19 regulations for SOI network]{Change in coefficients for the global-$\alpha$ \code{GNAR(4,[2,1,1,1])} model across COVID-19 regulations for the \textbf{SOI} network}
\label{fig:parameter_soi}
\end{figure}

\begin{figure}[h!]
\centering
\begin{subfigure}{\textwidth}
  \centering
  \includegraphics[scale = 0.4]{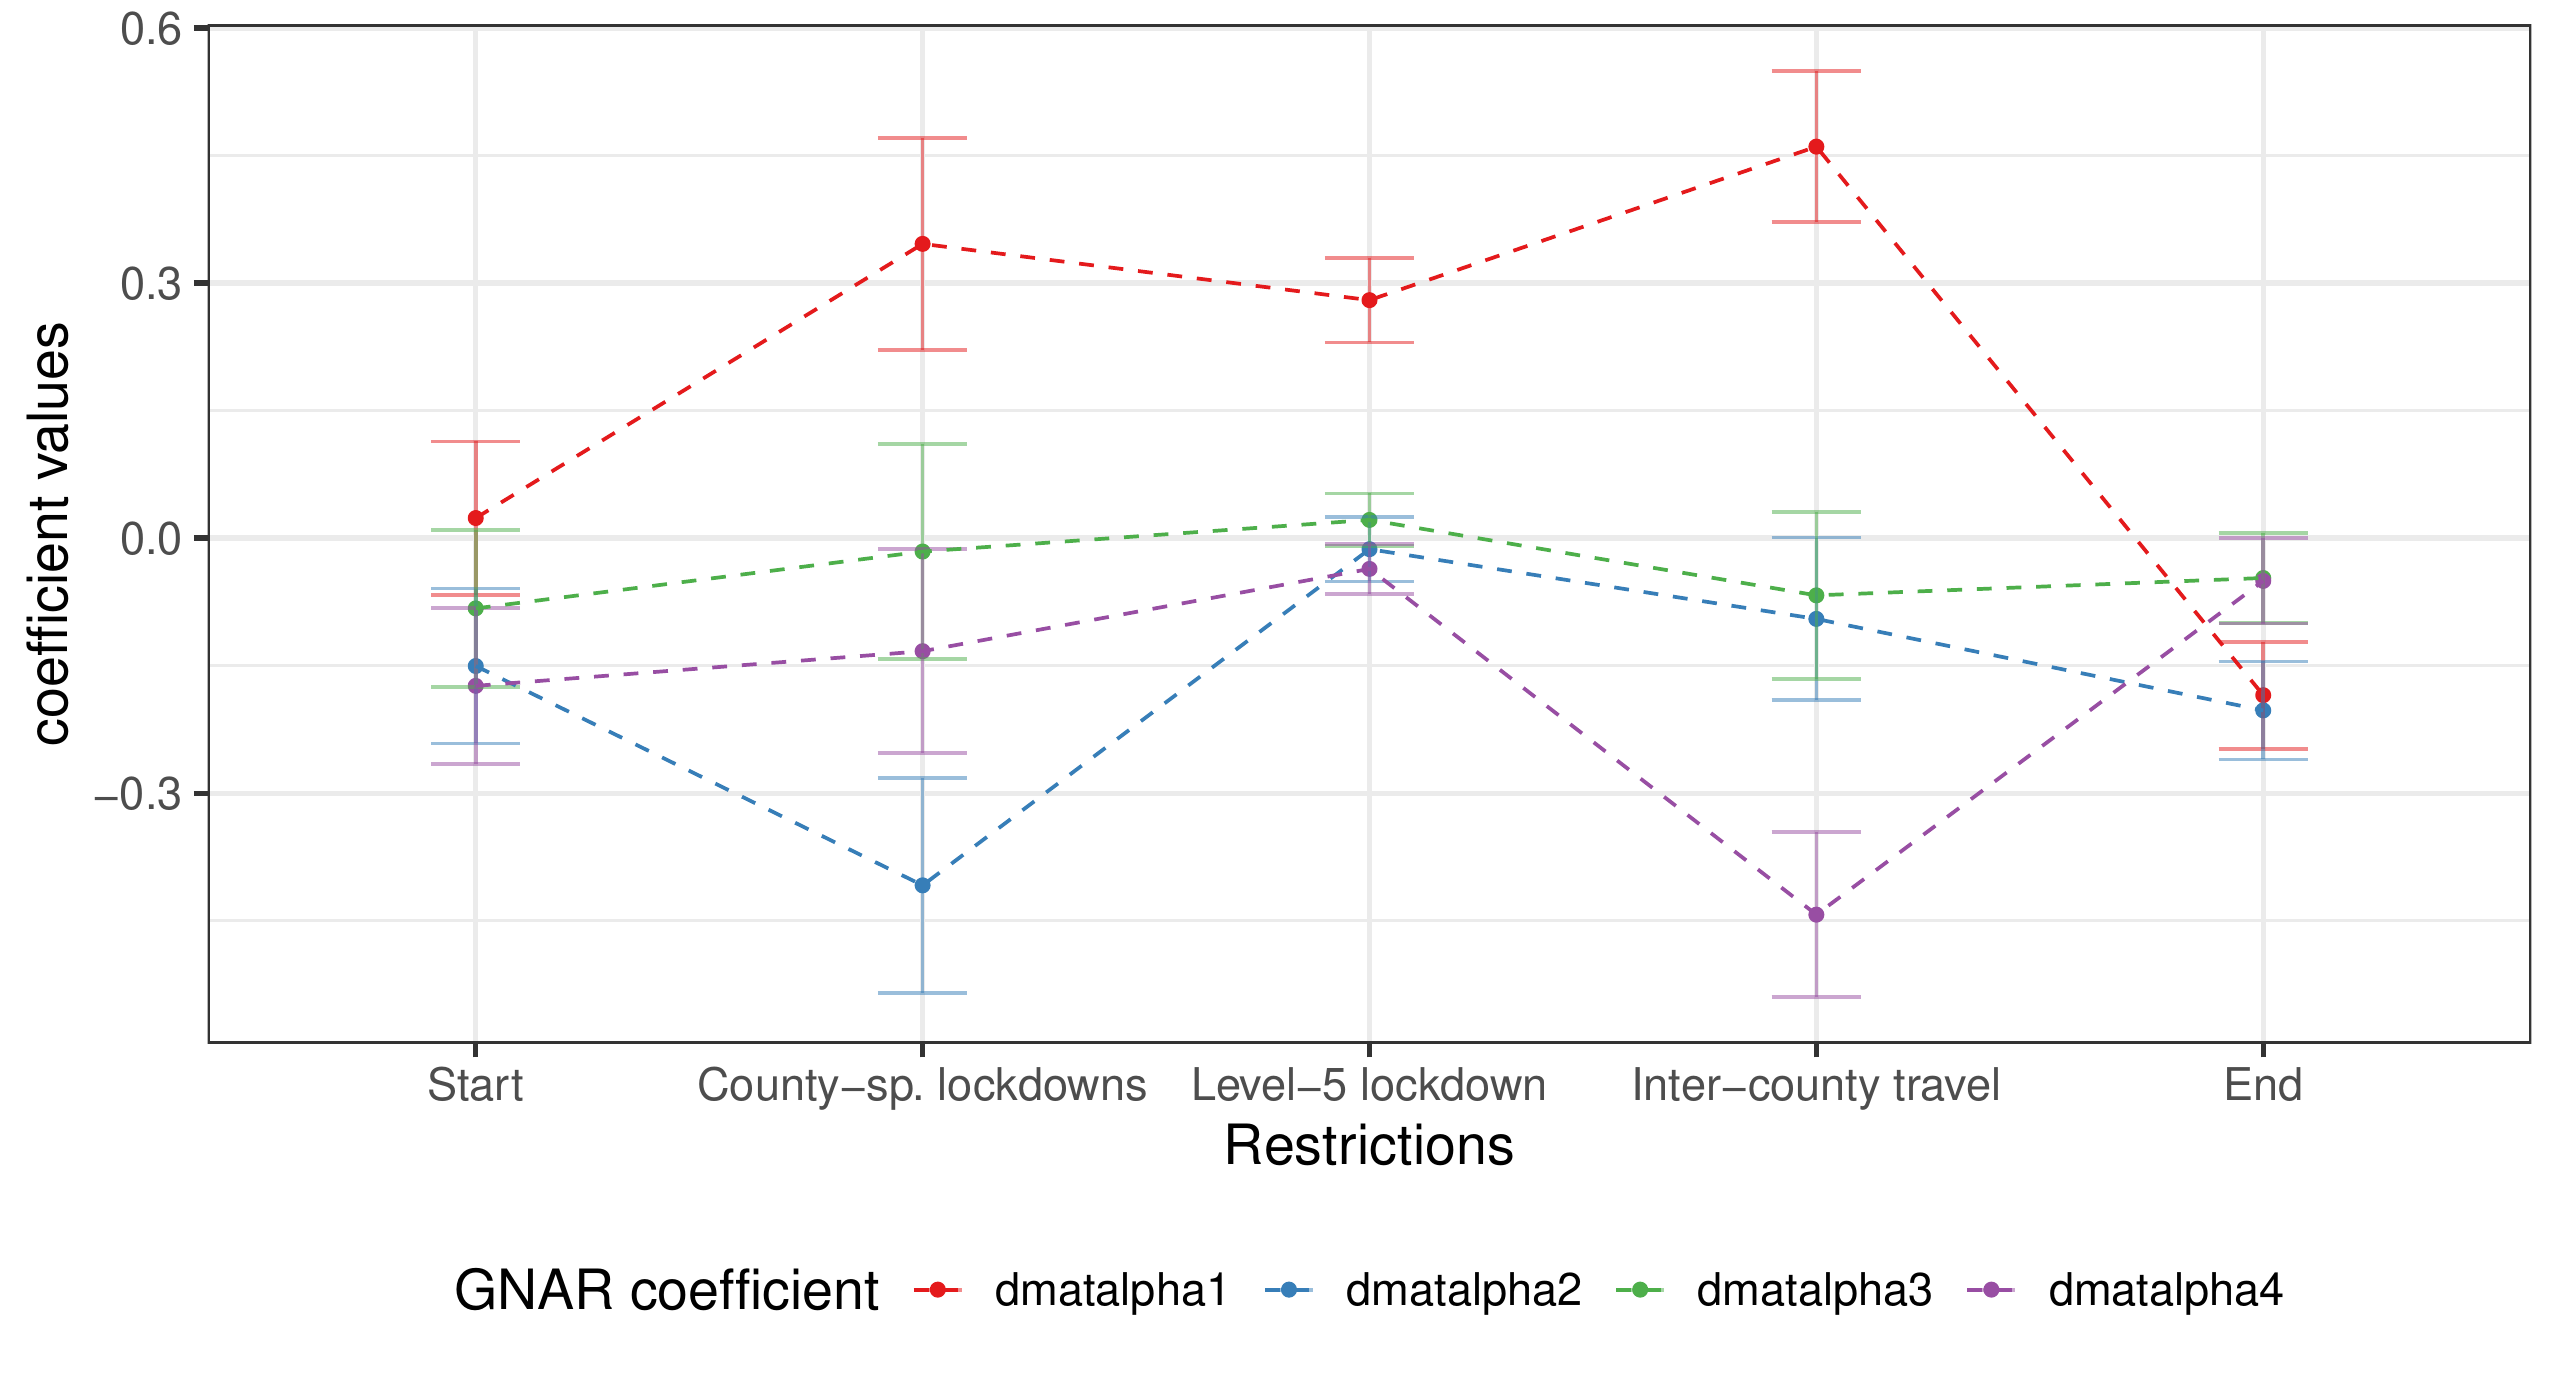}
  \caption{$\alpha$-order}
\end{subfigure}
\begin{subfigure}{\textwidth}
  \centering
  \includegraphics[scale = 0.4]{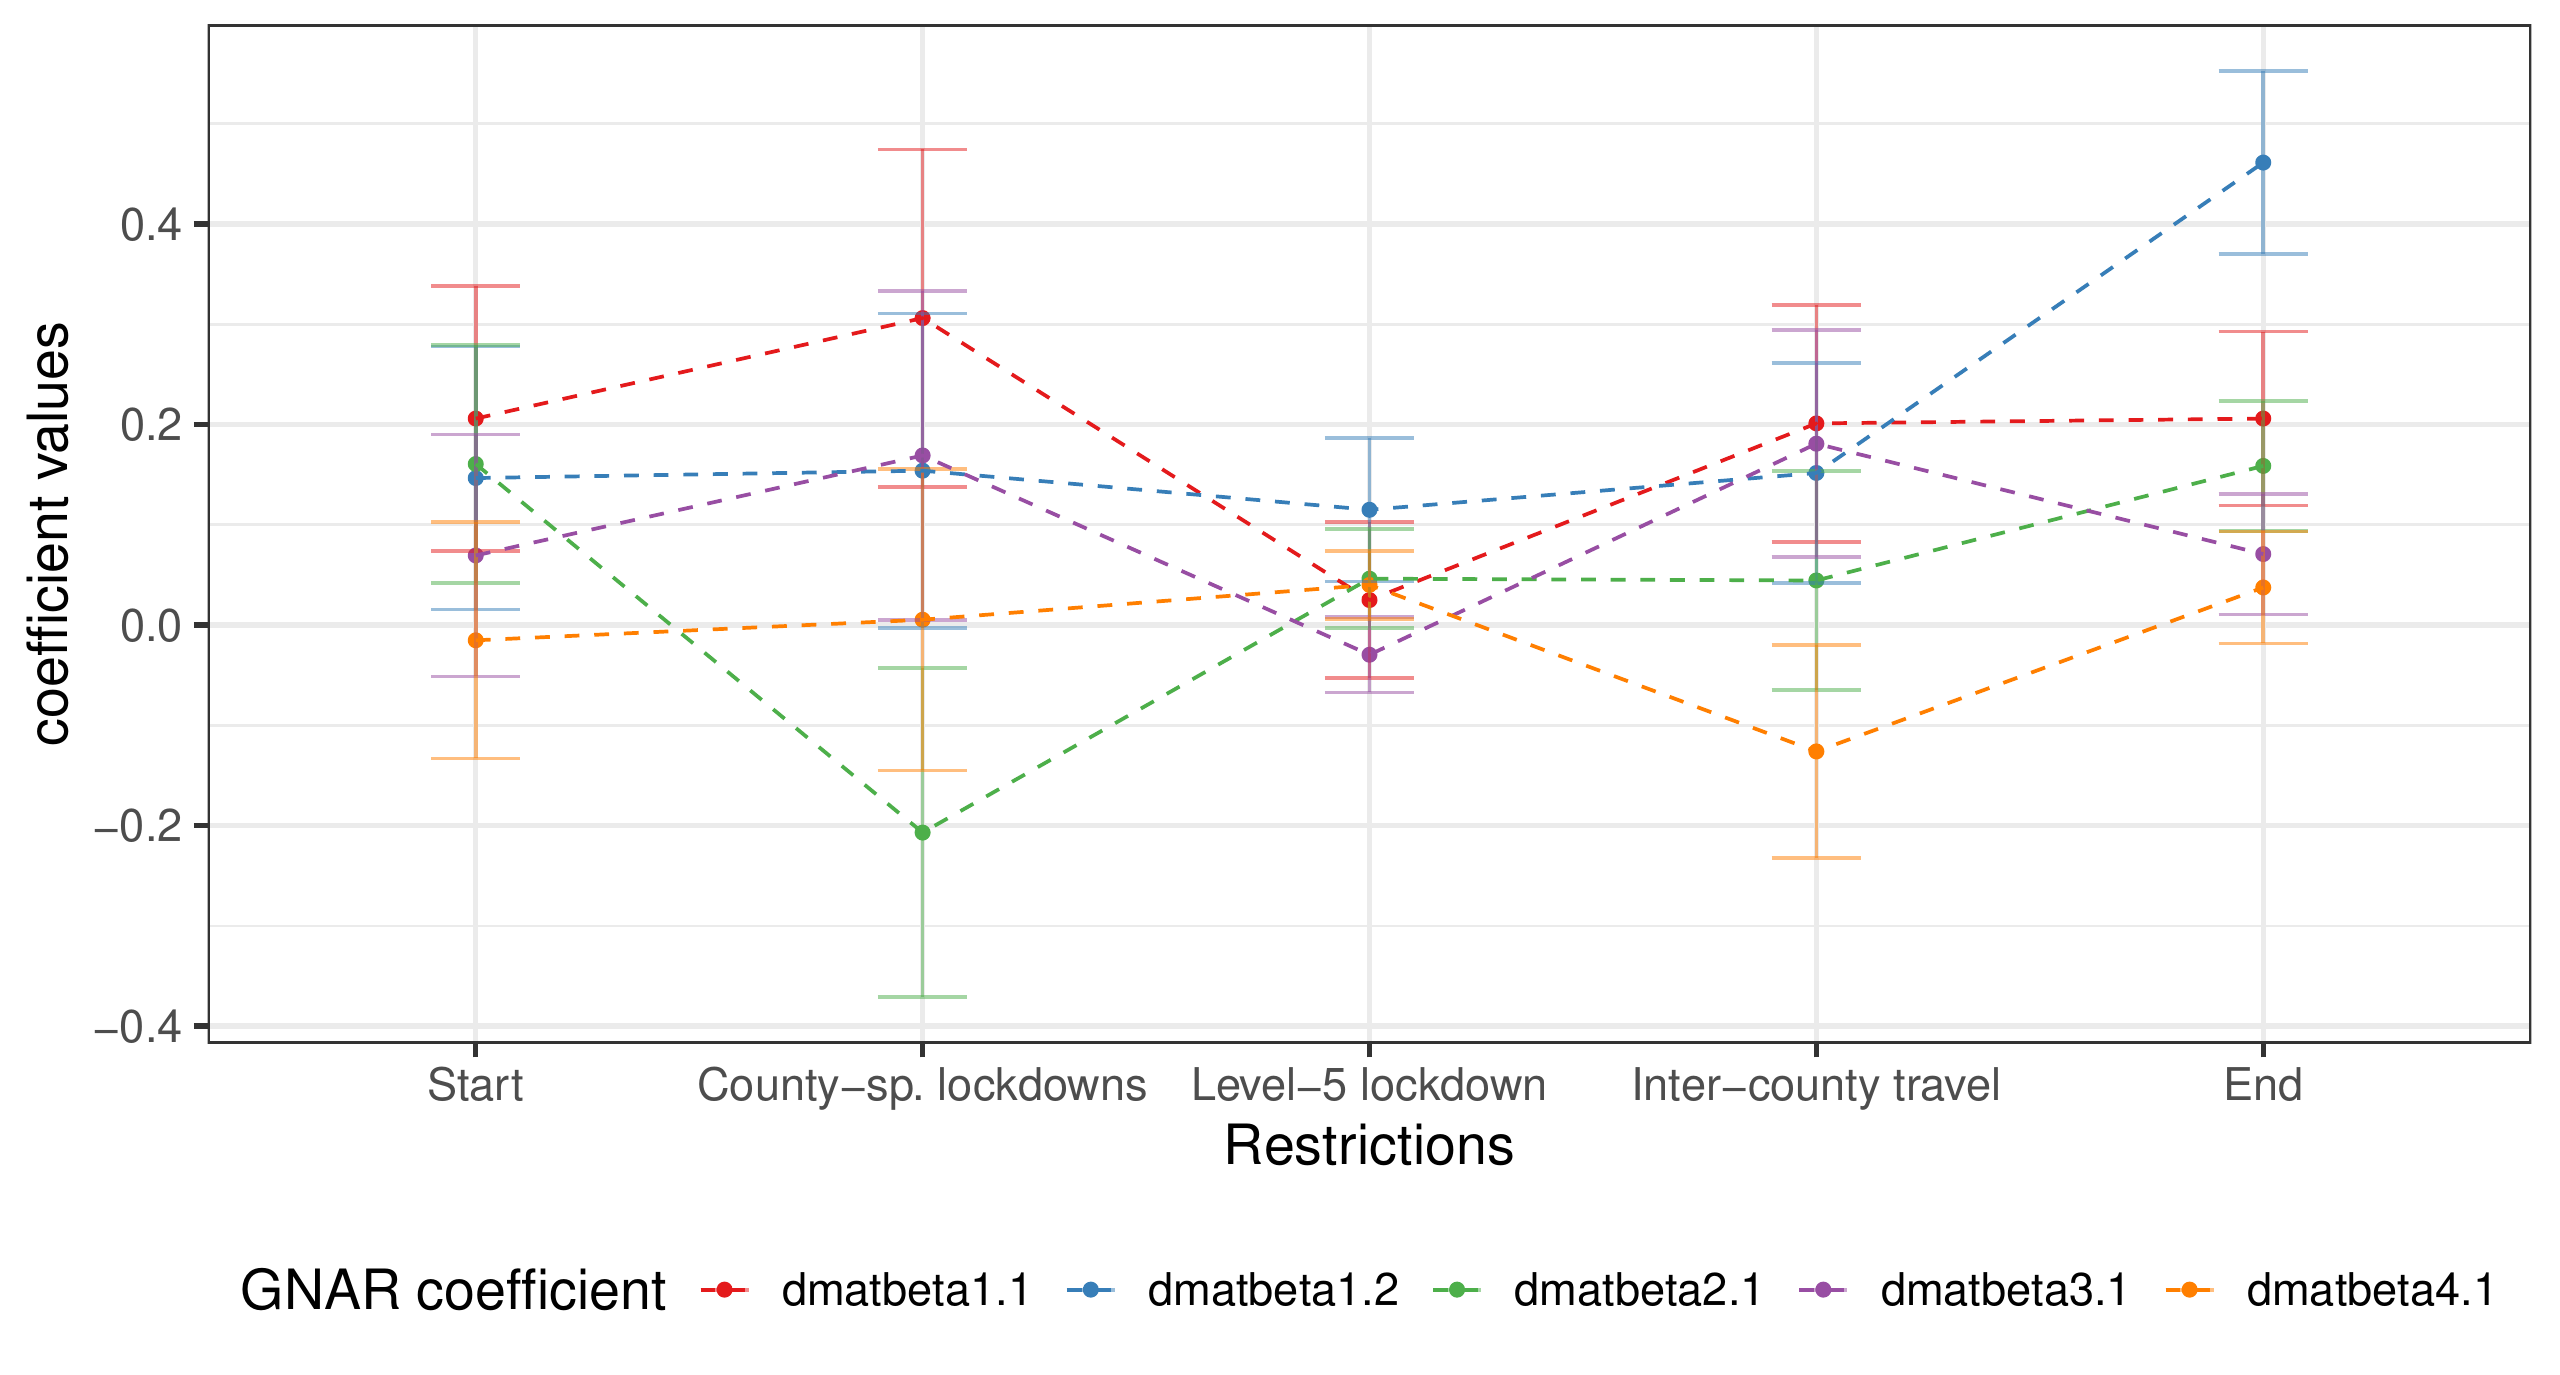}
  \caption{$\beta$-order}
\end{subfigure}
\caption[Change in GNAR model coefficients for COVID-19 regulations for Relative neighbourhood network]{Change in coefficients for the global-$\alpha$ \code{GNAR(4,[2,1,1,1])} model across COVID-19 regulations for the \textbf{Relative neighbourhood} network}
\label{fig:parameter_relative}
\end{figure}

\begin{figure}[h!]
\centering
\begin{subfigure}{\textwidth}
  \centering
  \includegraphics[scale = 0.4]{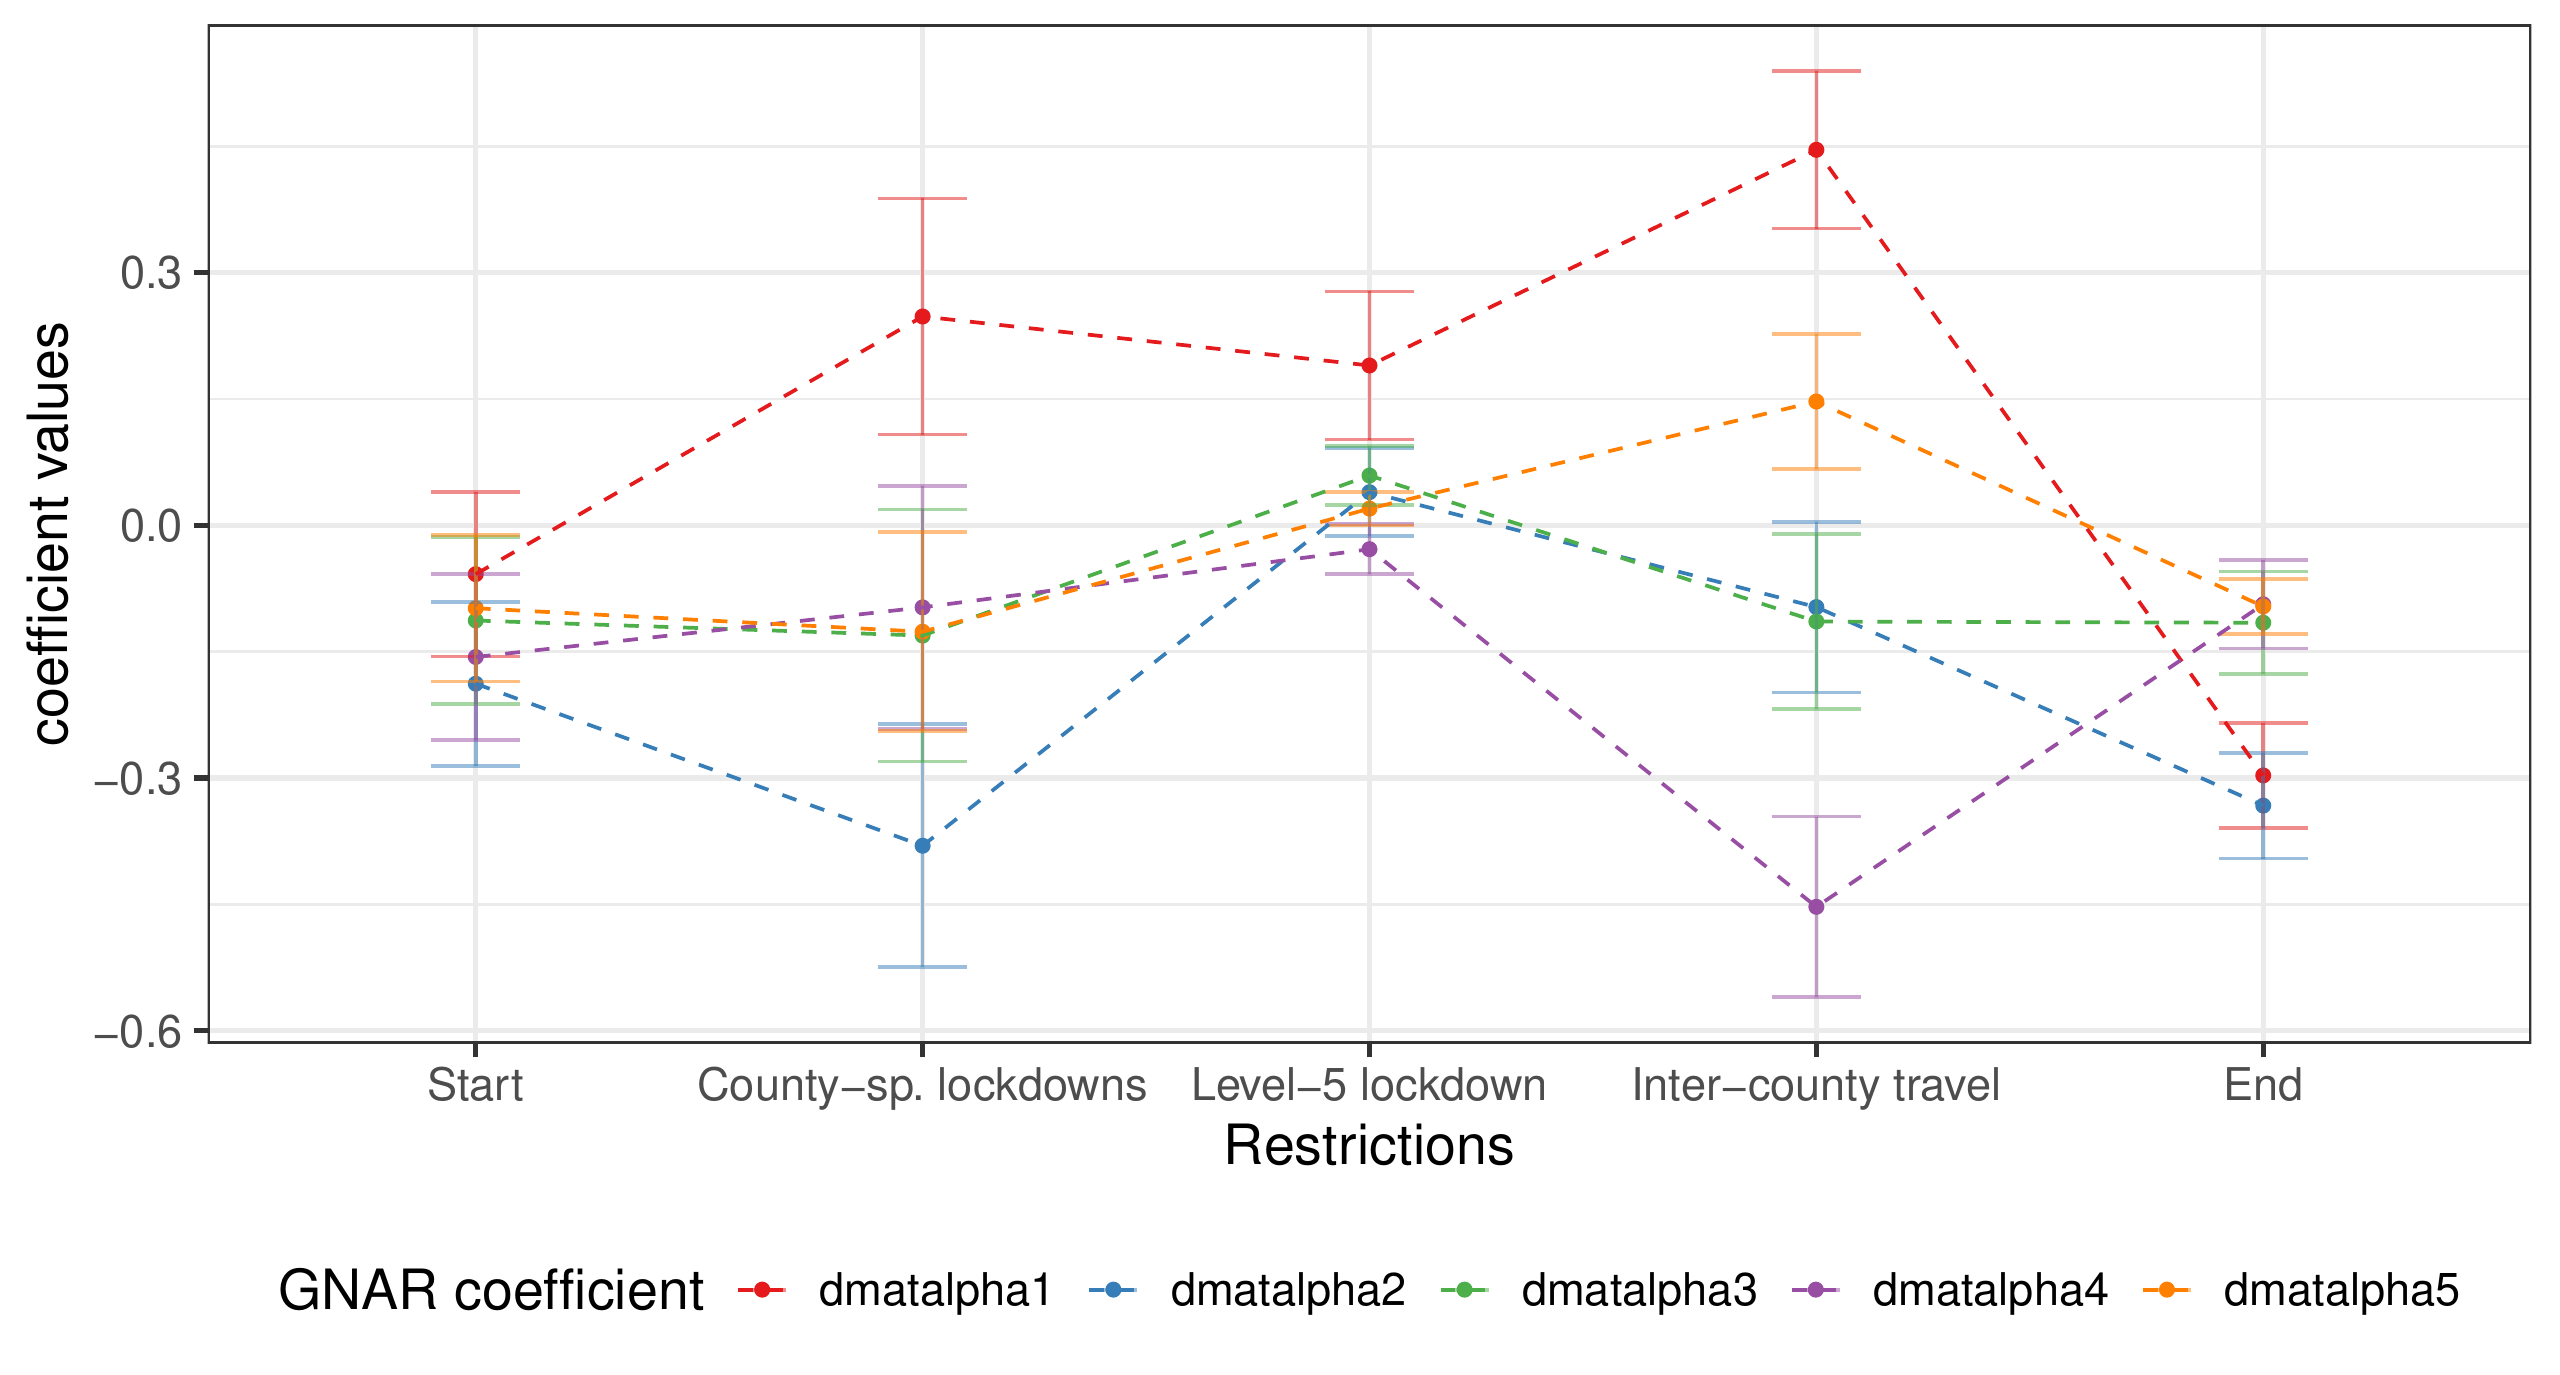}
  \caption{$\alpha$-order}
\end{subfigure}
\begin{subfigure}{\textwidth}
  \centering
  \includegraphics[scale = 0.4]{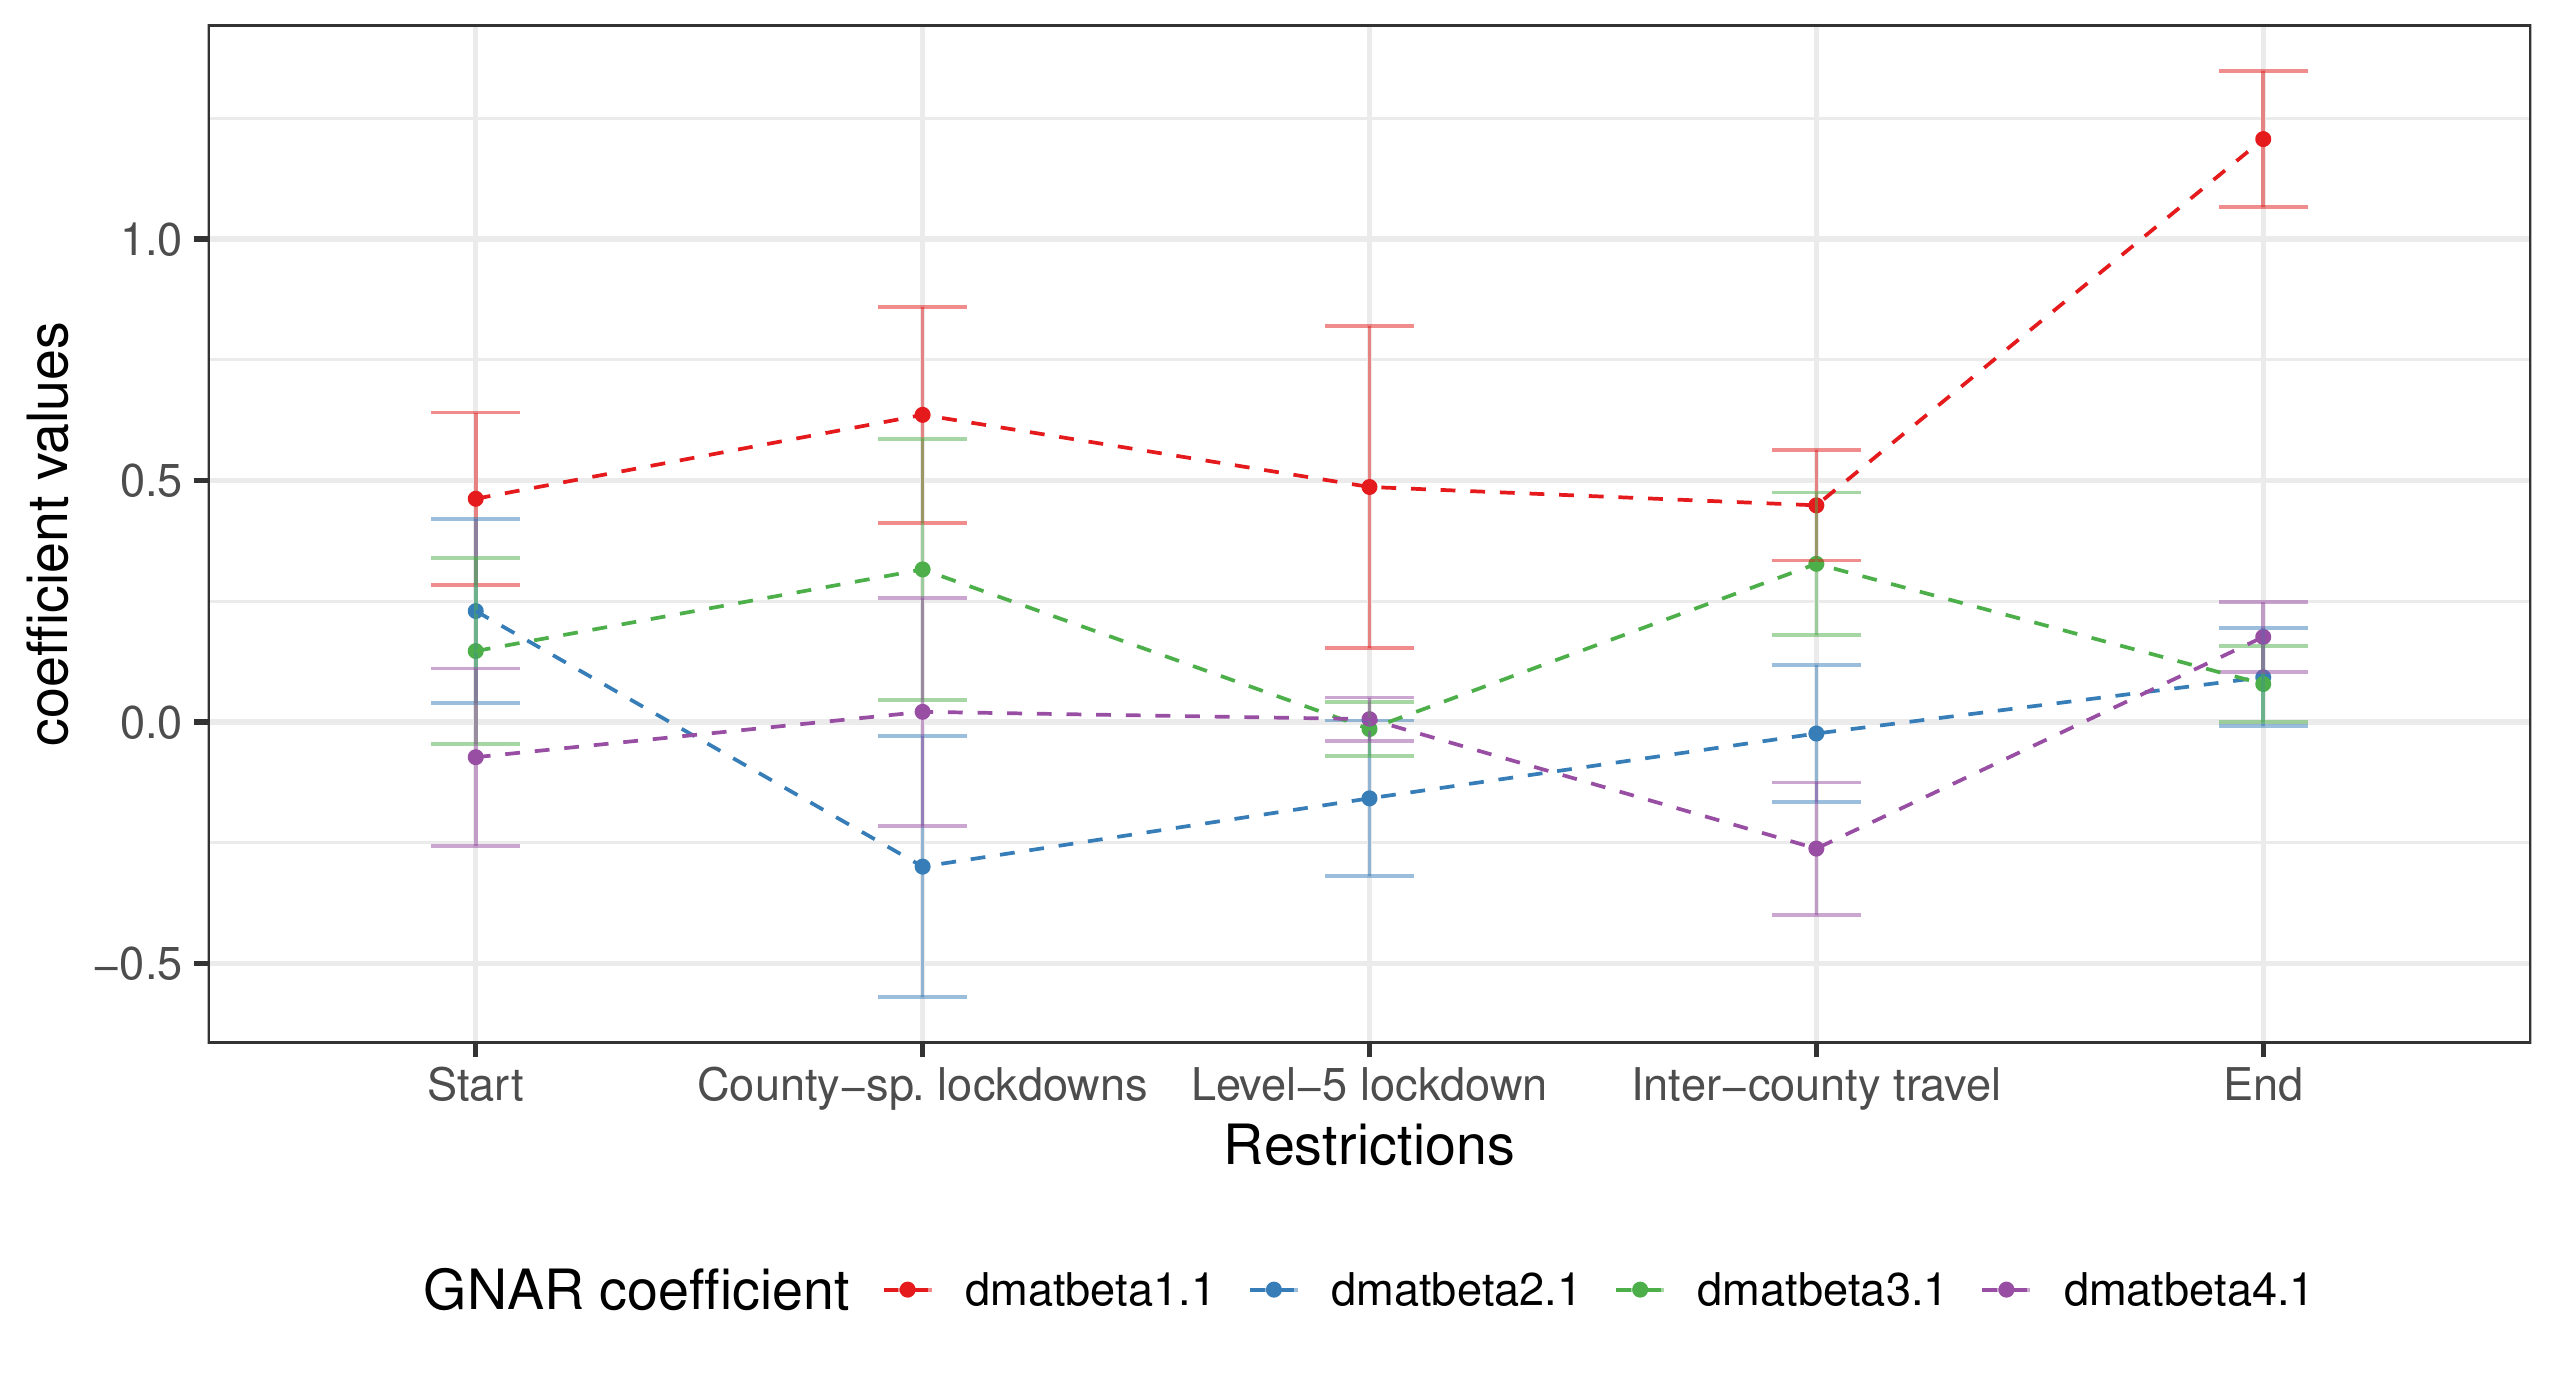}
  \caption{$\beta$-order}
\end{subfigure}
\caption[Change in GNAR model coefficients for COVID-19 regulations for Complete network]{Development of coefficients for global-$\alpha$ \code{GNAR(5,[1,1,1,1,0])} model across COVID-19 regulations for \textbf{Complete} network}
\label{fig:parameter_complete}
\end{figure}

\begin{figure}[h!]
\centering
\begin{subfigure}{\textwidth}
  \centering
  \includegraphics[scale = 0.4]{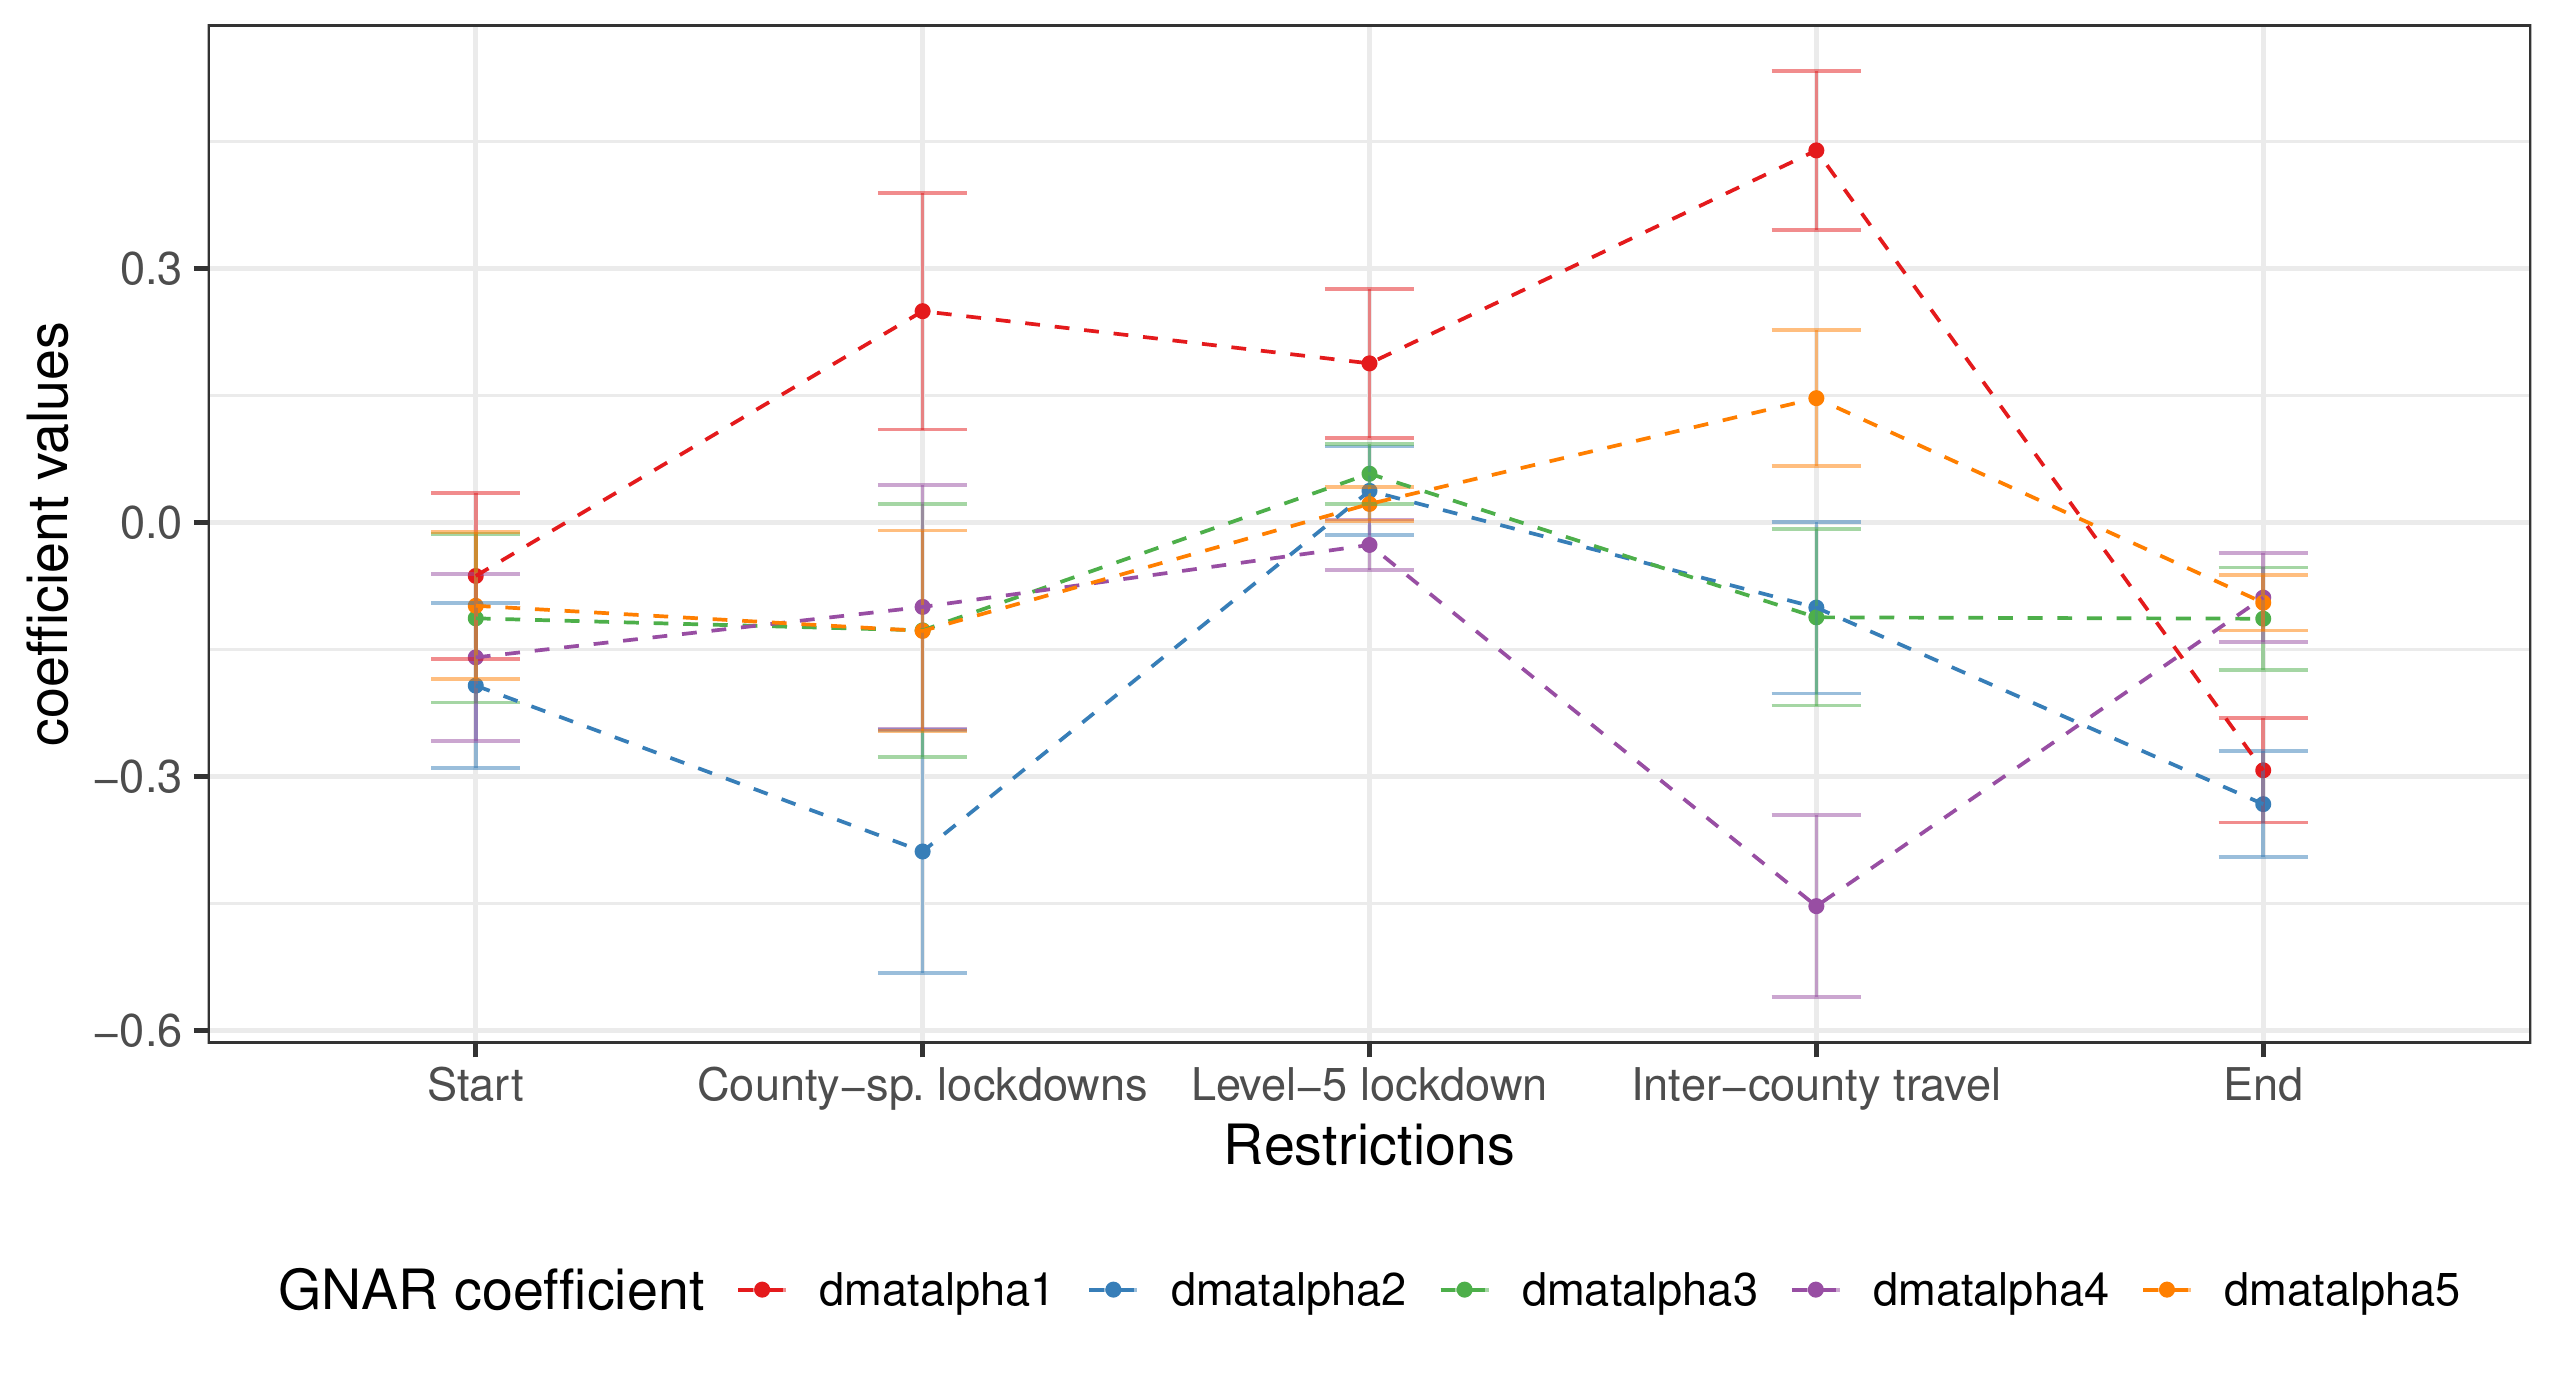}
  \caption{$\alpha$-order}
\end{subfigure}
\begin{subfigure}{\textwidth}
  \centering
  \includegraphics[scale = 0.4]{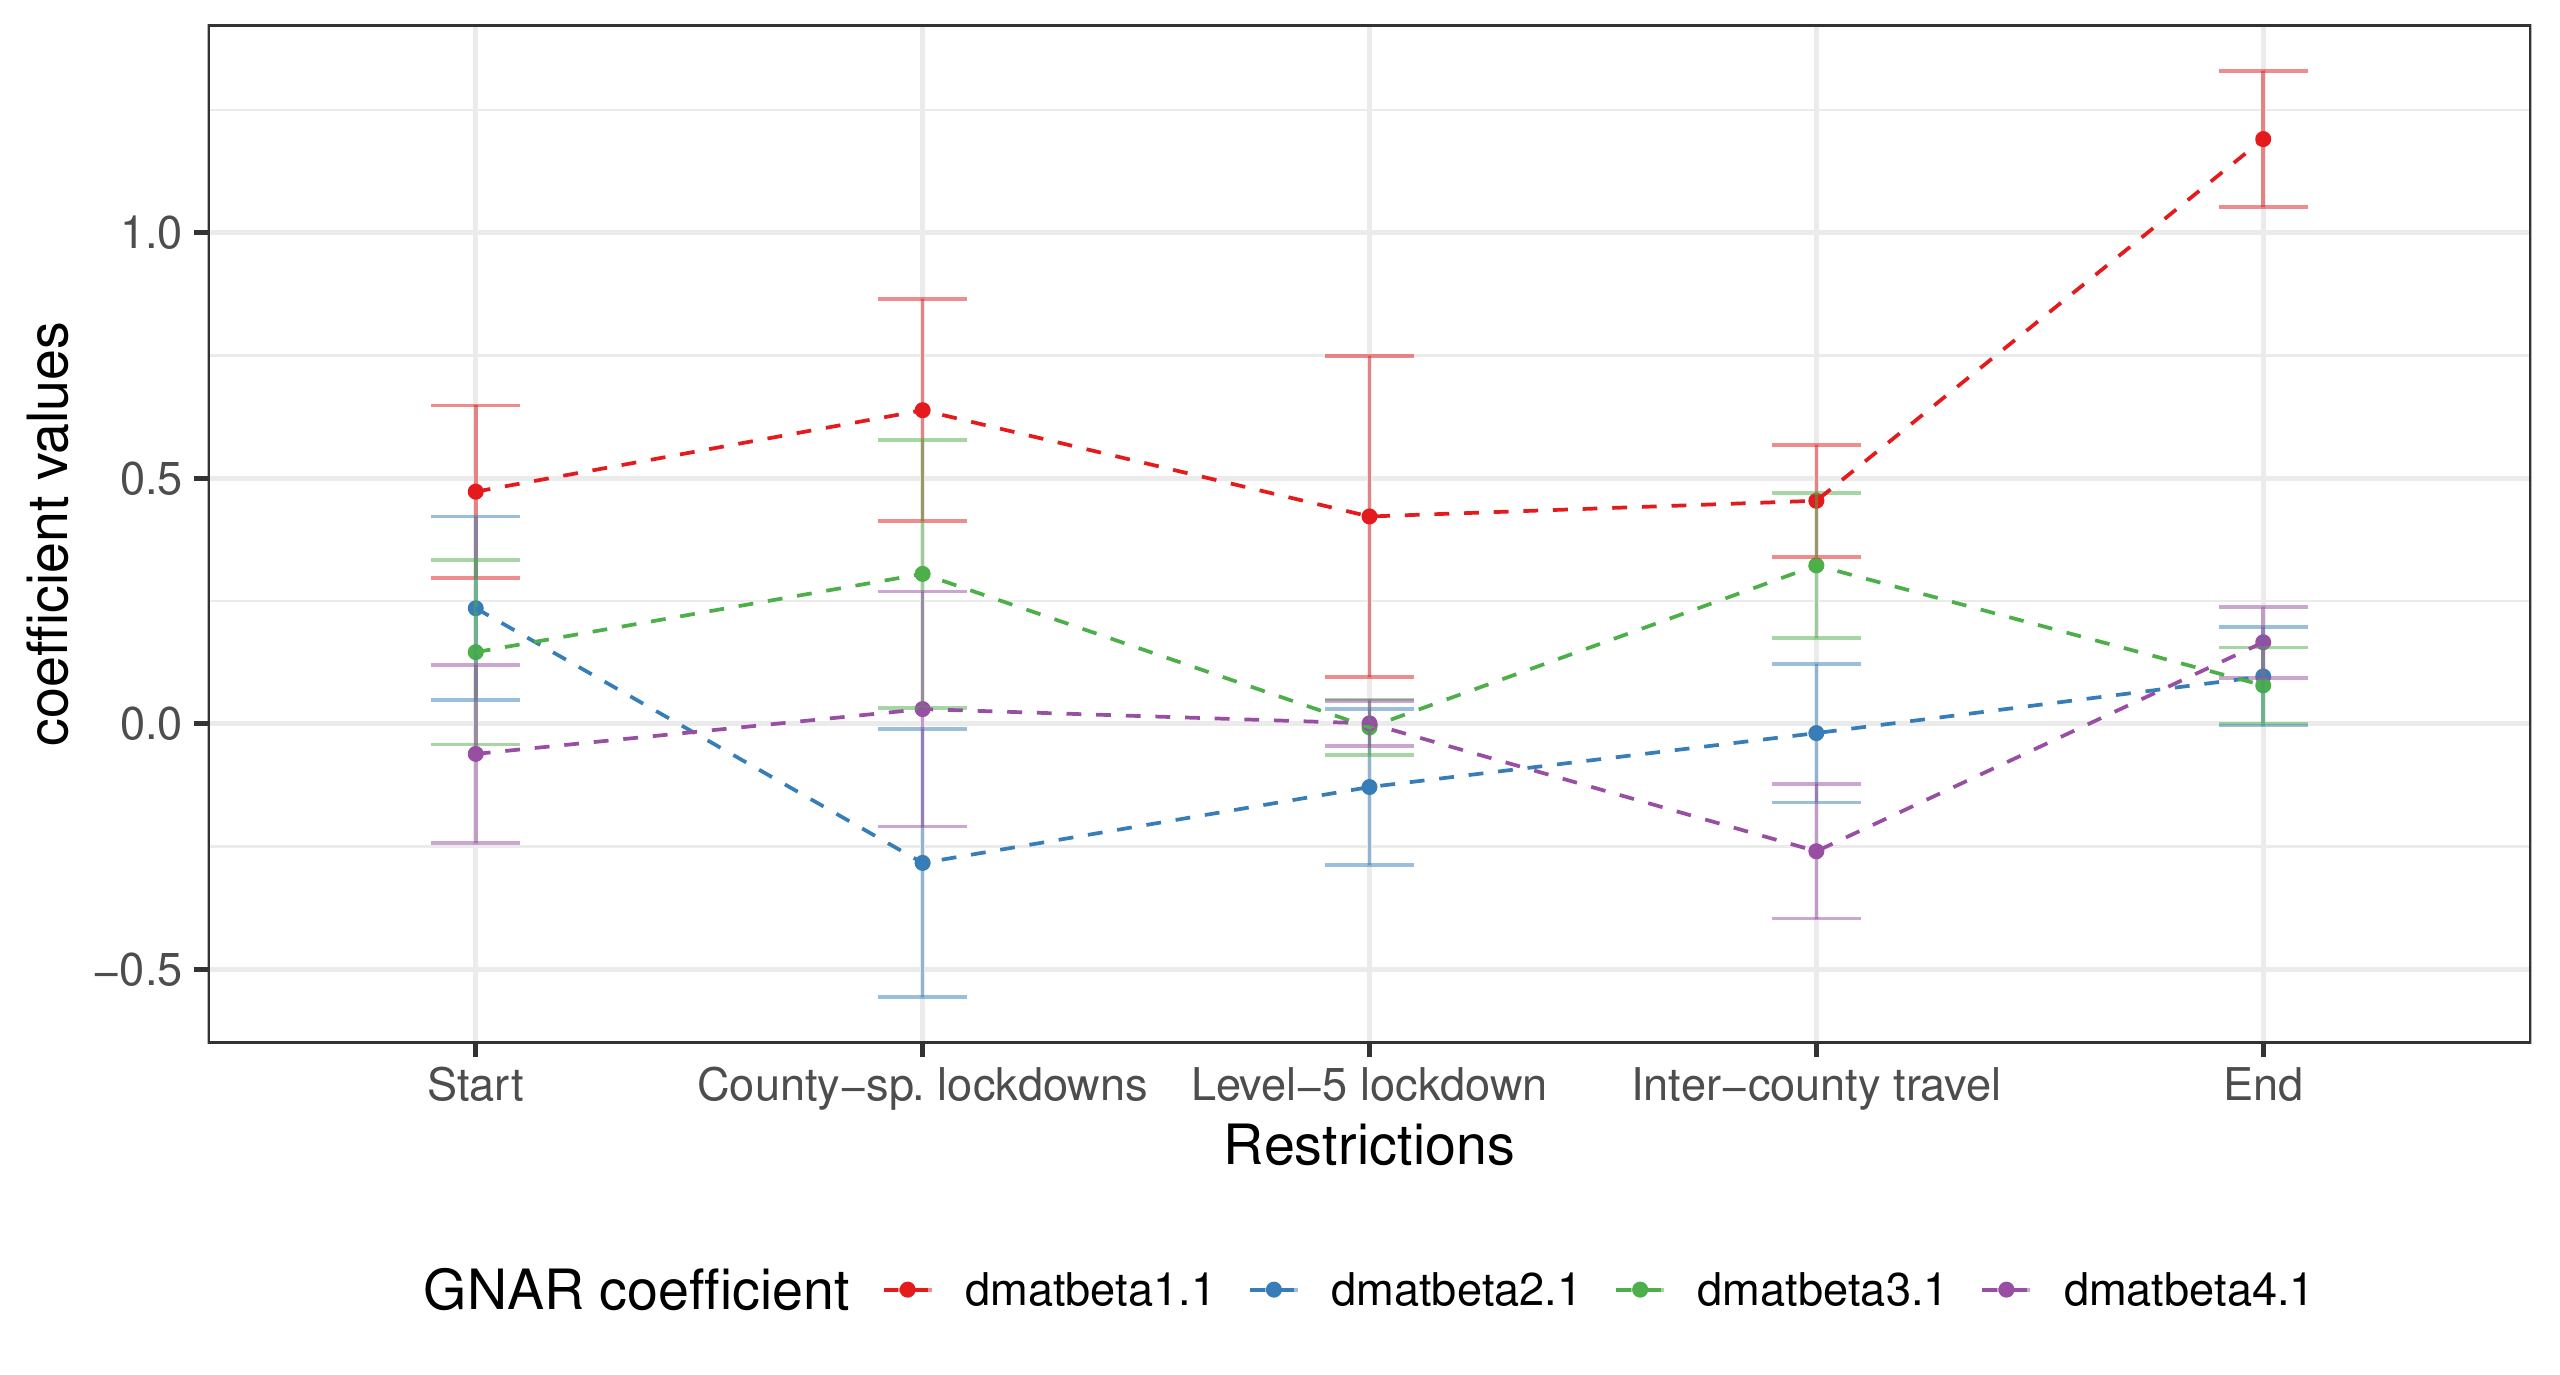}
  \caption{$\beta$-order}
\end{subfigure}
\caption[Change in GNAR model coefficients for COVID-19 regulations for KNN network]{Development of coefficients for global-$\alpha$ \code{GNAR(5,[1,1,1, 1,0])} model across COVID-19 regulations for \textbf{KNN} network}
\label{fig:parameter_knn}
\end{figure}

\begin{figure}[h!]
\centering
\begin{subfigure}{\textwidth}
  \centering
  \includegraphics[scale = 0.4]{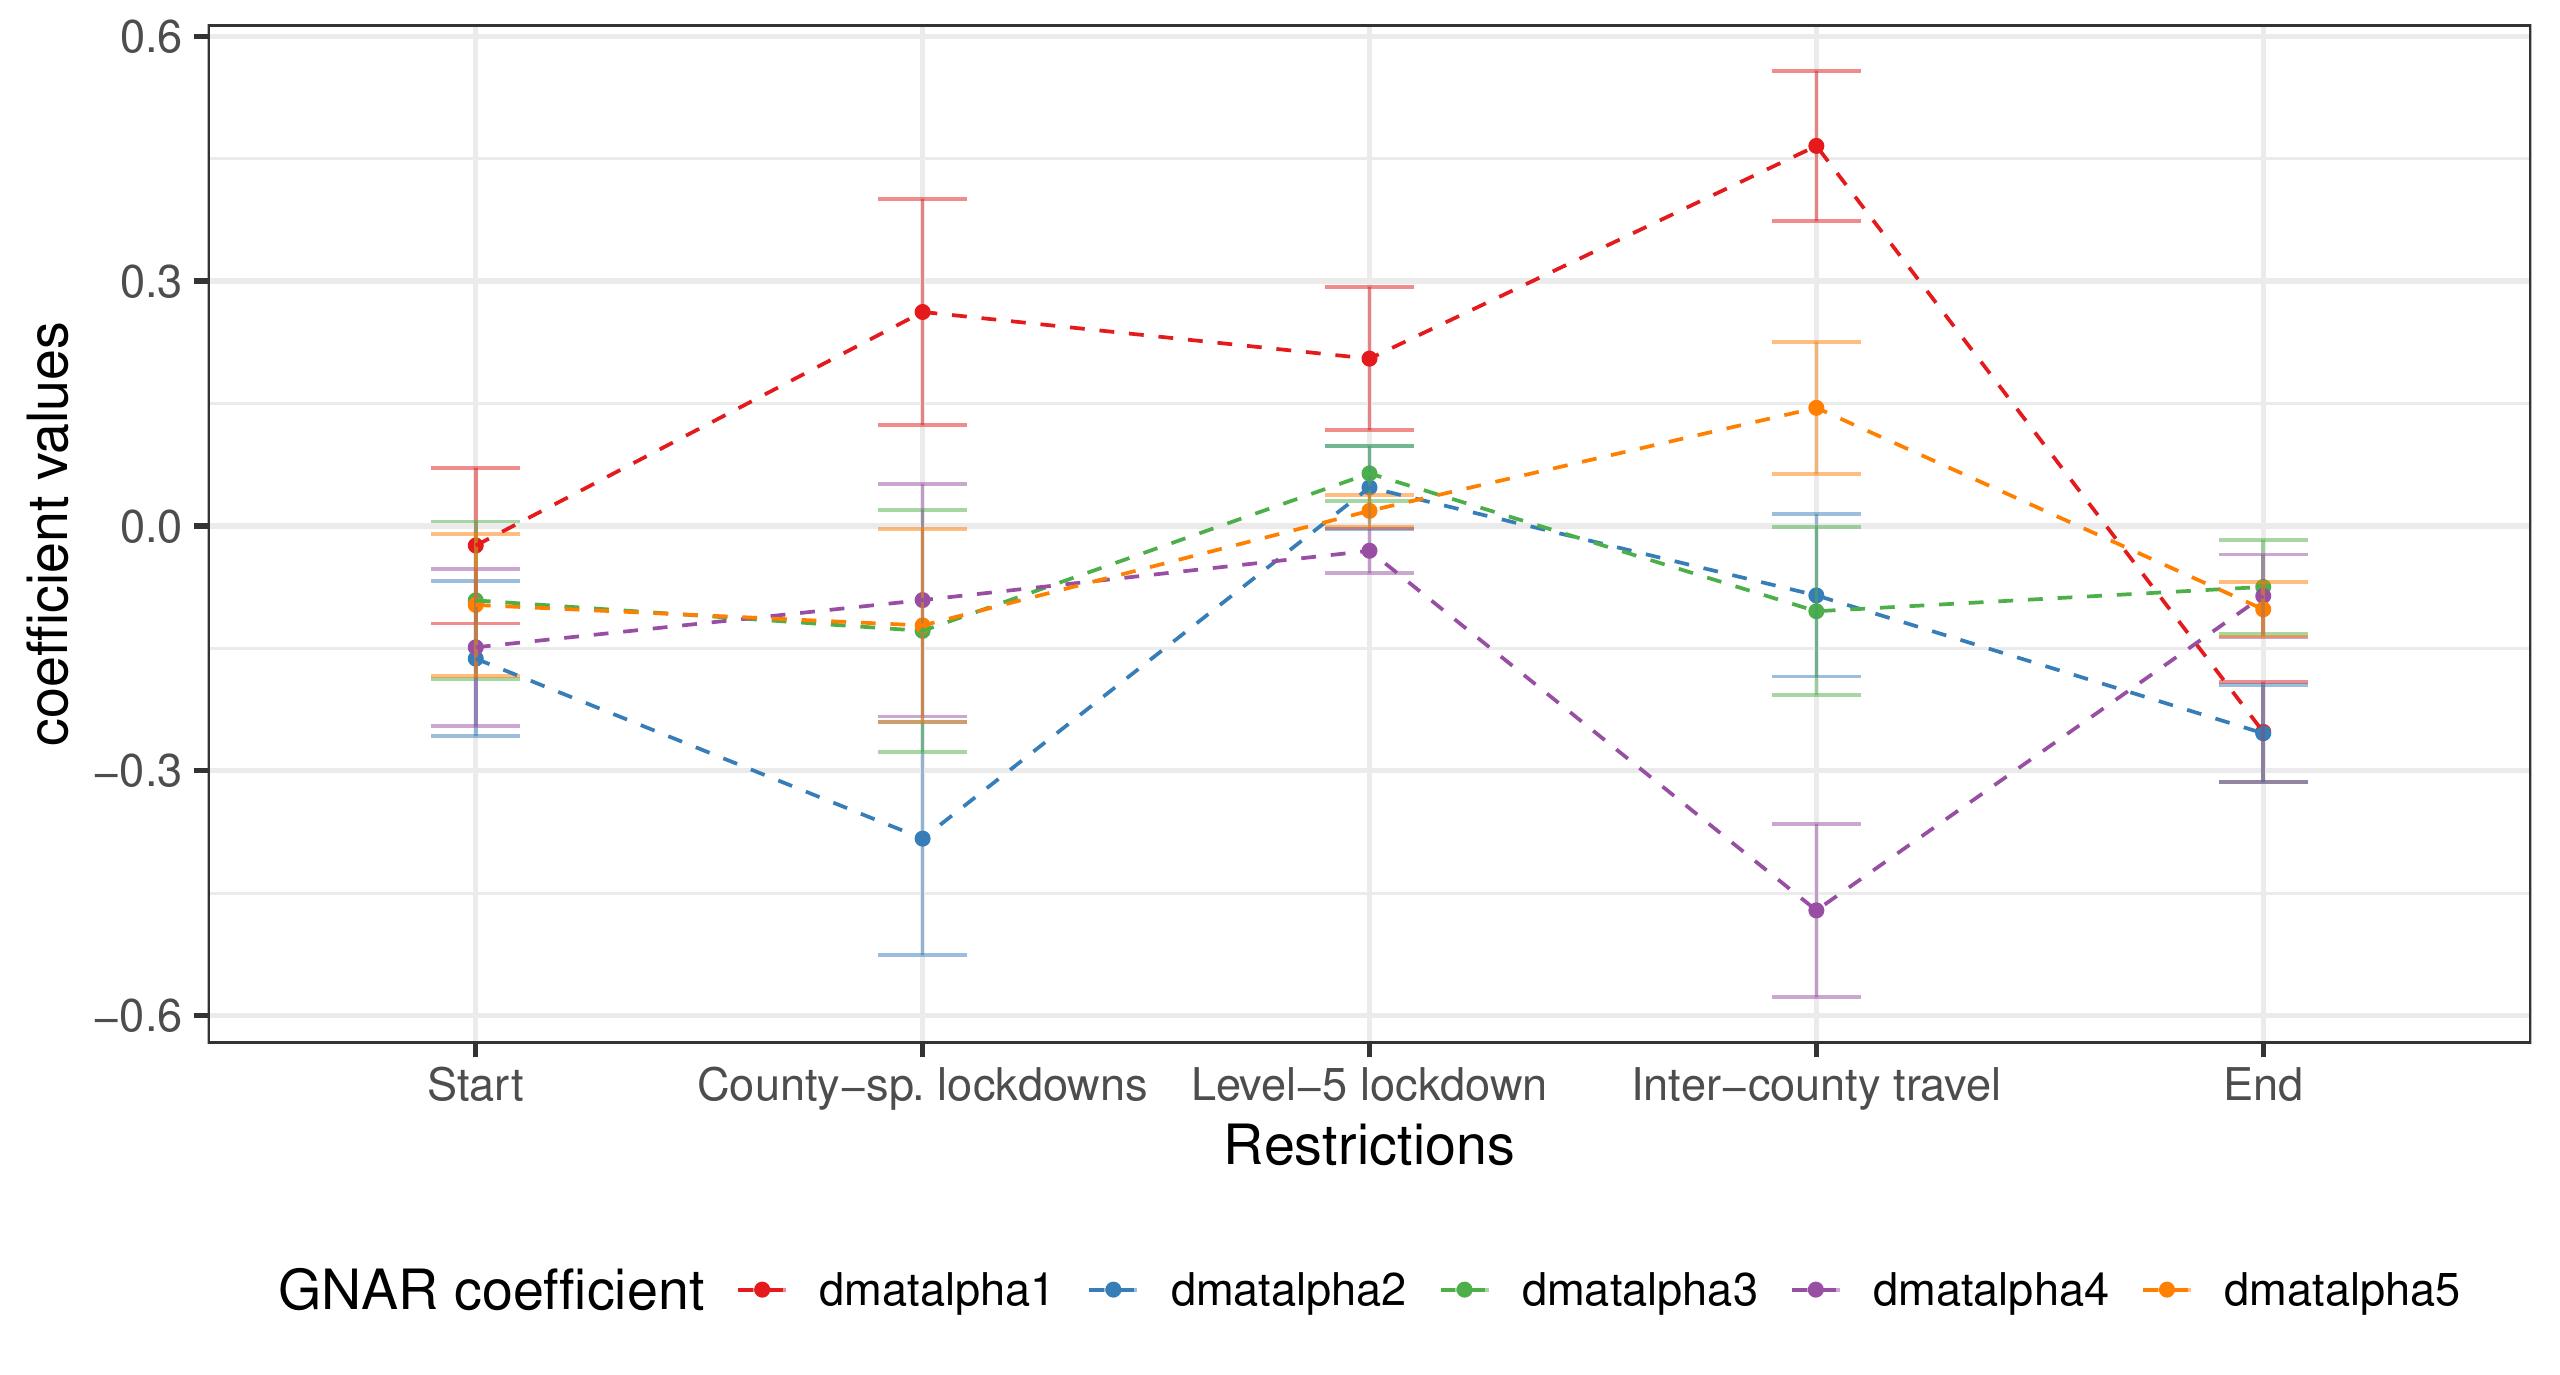}
  \caption{$\alpha$-order}
\end{subfigure}
\begin{subfigure}{\textwidth}
  \centering
  \includegraphics[scale = 0.4]{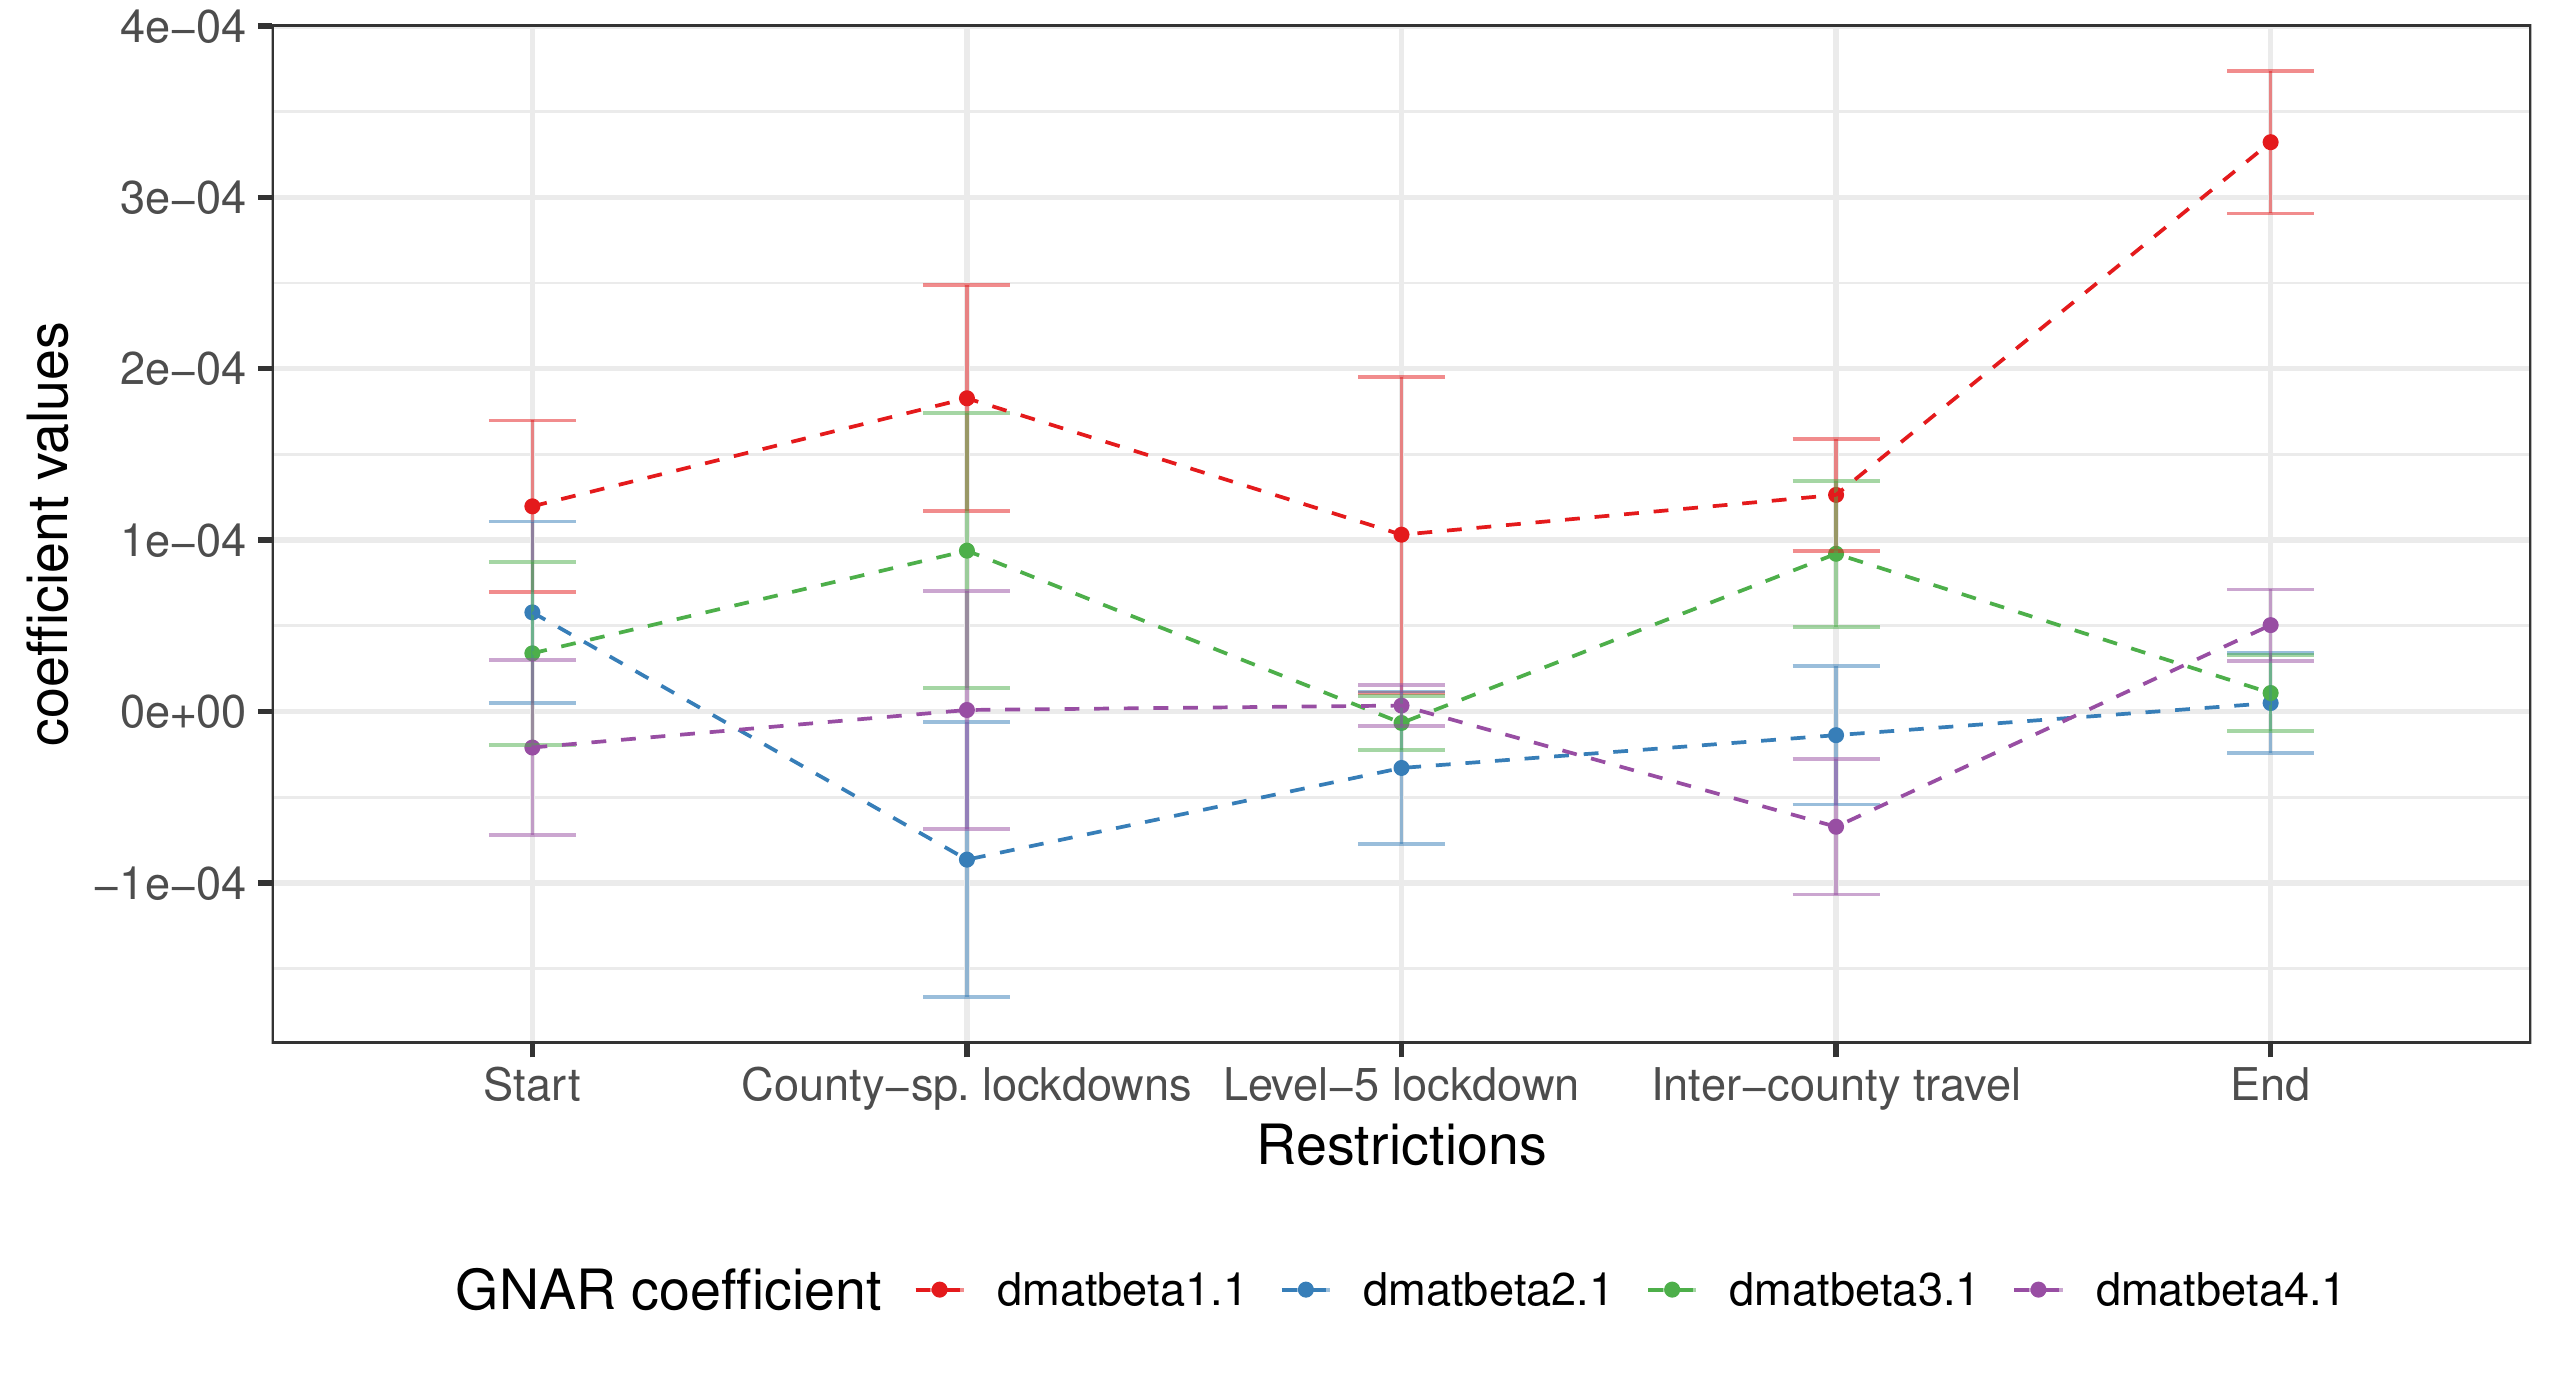}
  \caption{$\beta$-order}
\end{subfigure}
\caption[Change in GNAR model coefficients for COVID-19 regulations for DNN network]{Change in coefficients for the global-$\alpha$ \code{GNAR(5,[1,1,1, 1,0])} model across COVID-19 regulations for the \textbf{DNN} network}
\label{fig:parameter_dnn}
\end{figure}

\begin{figure}[h!]
\centering
\begin{subfigure}{\textwidth}
  \centering
  \includegraphics[scale = 0.4]{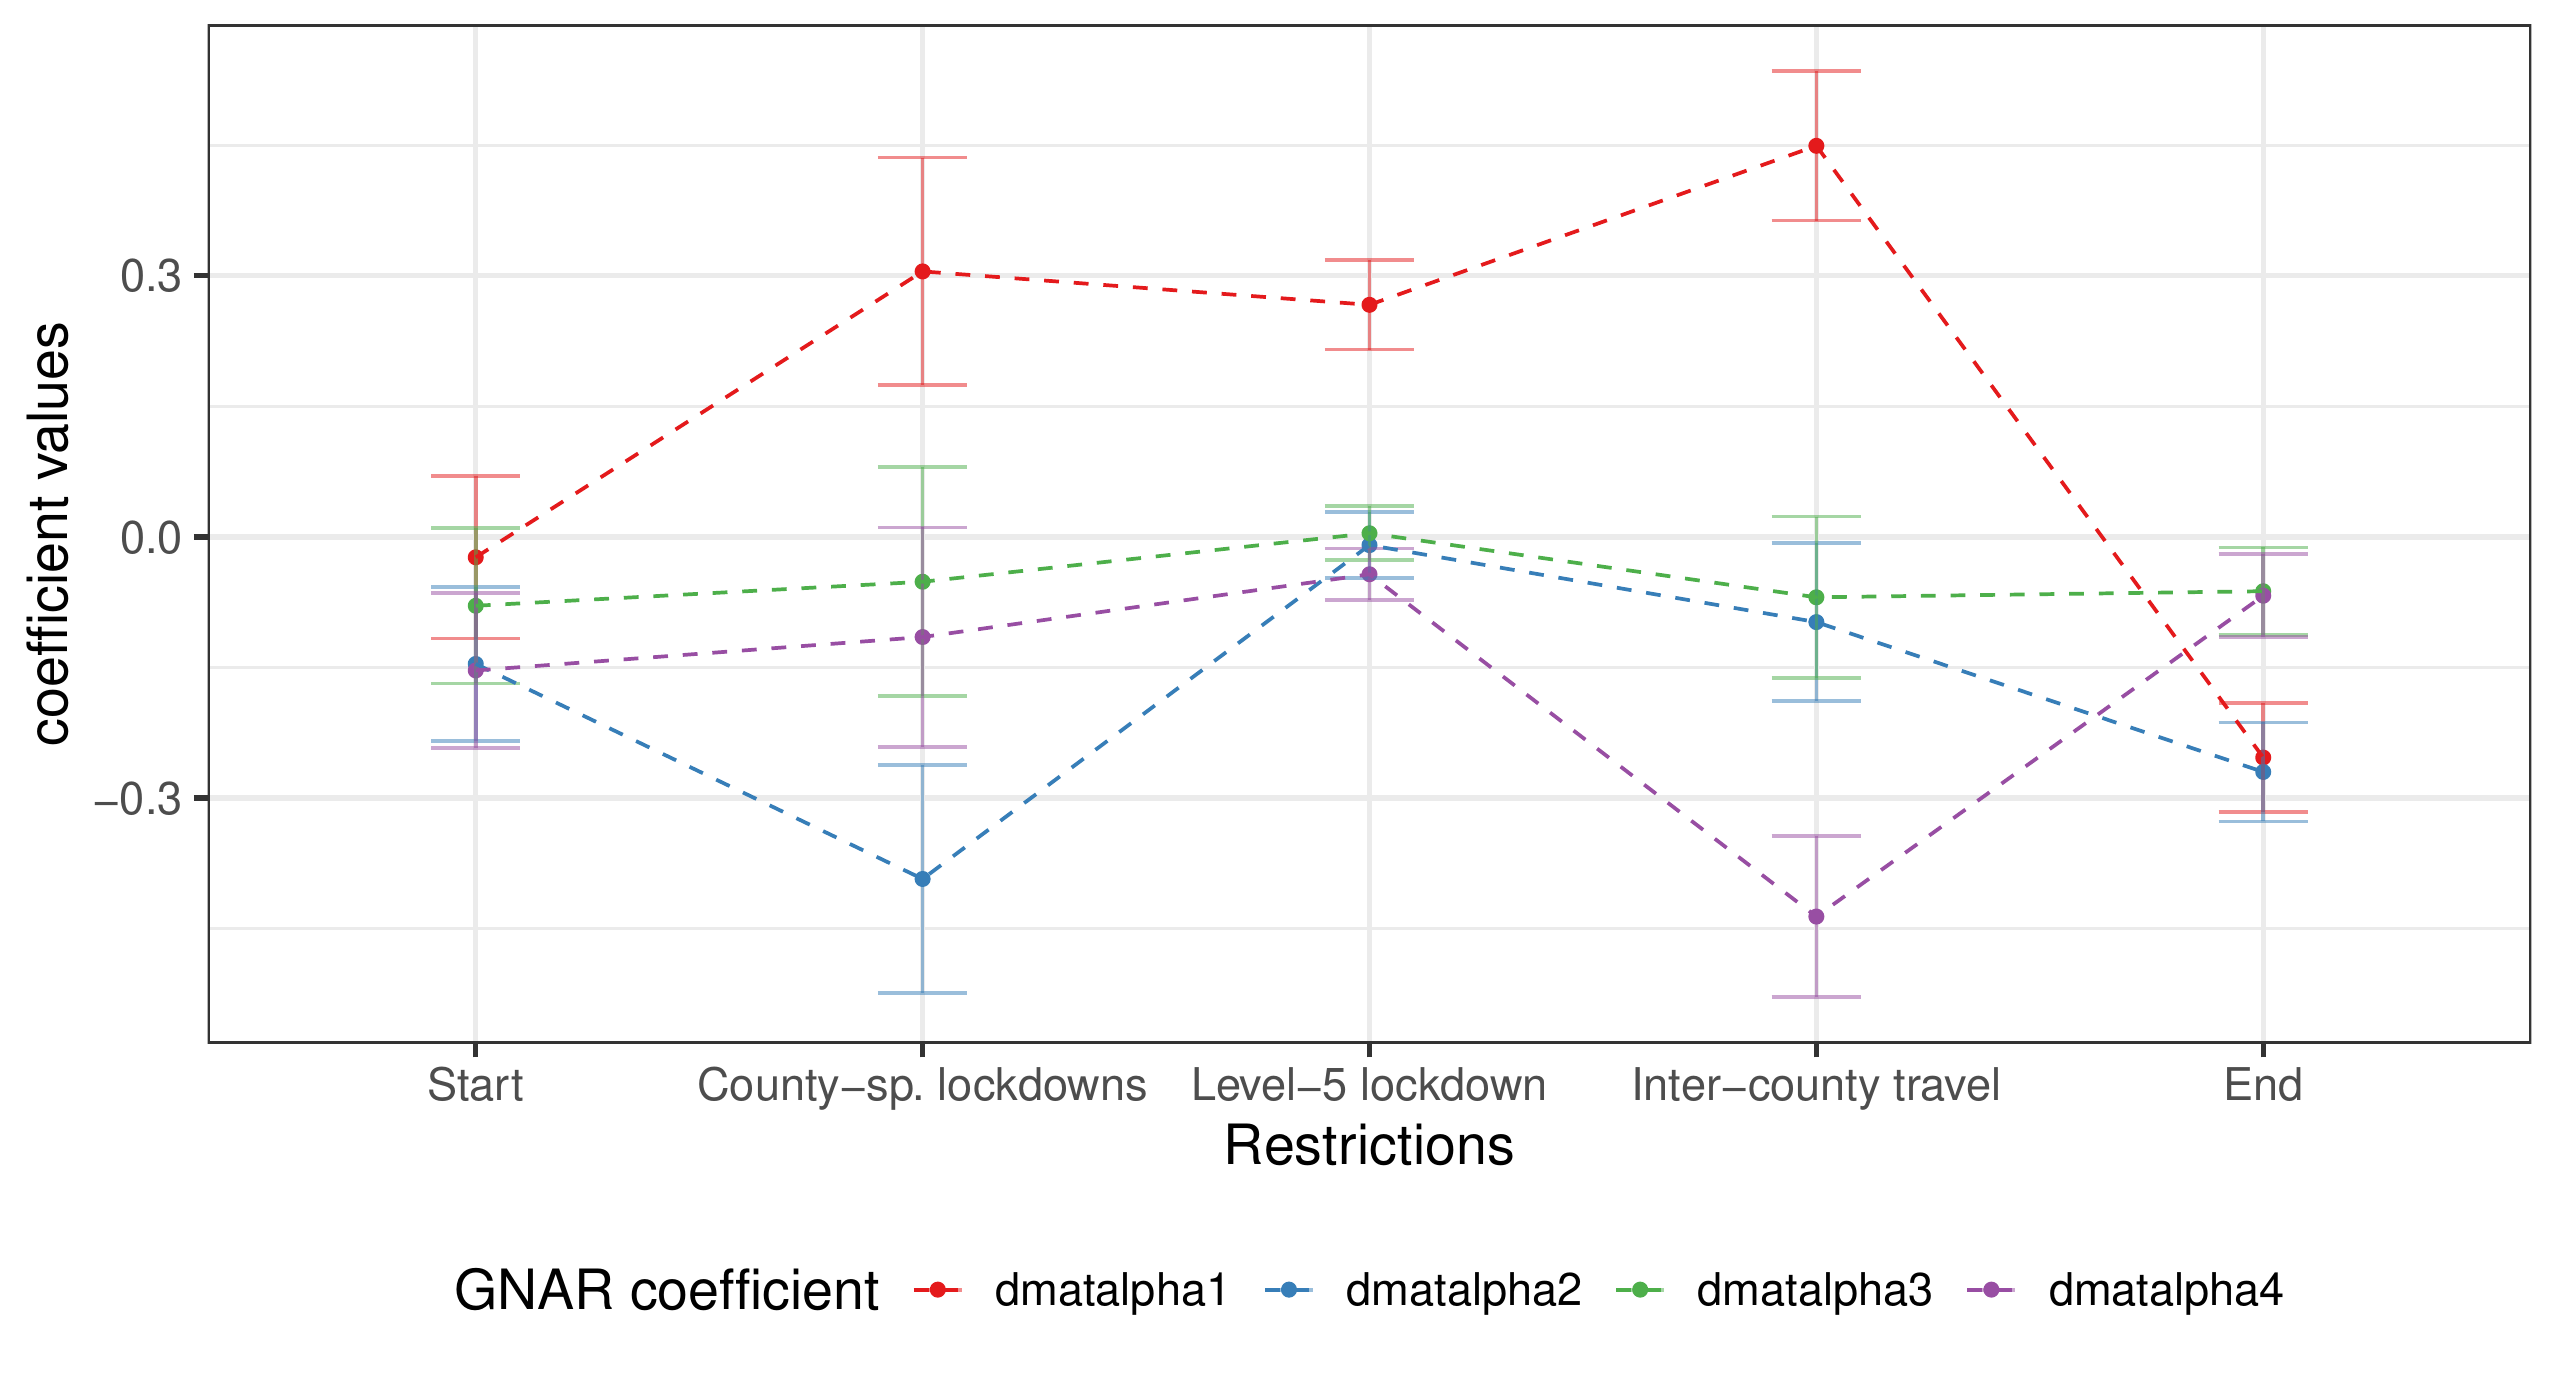}
  \caption{$\alpha$-order}
\end{subfigure}
\begin{subfigure}{\textwidth}
  \centering
  \includegraphics[scale = 0.4]{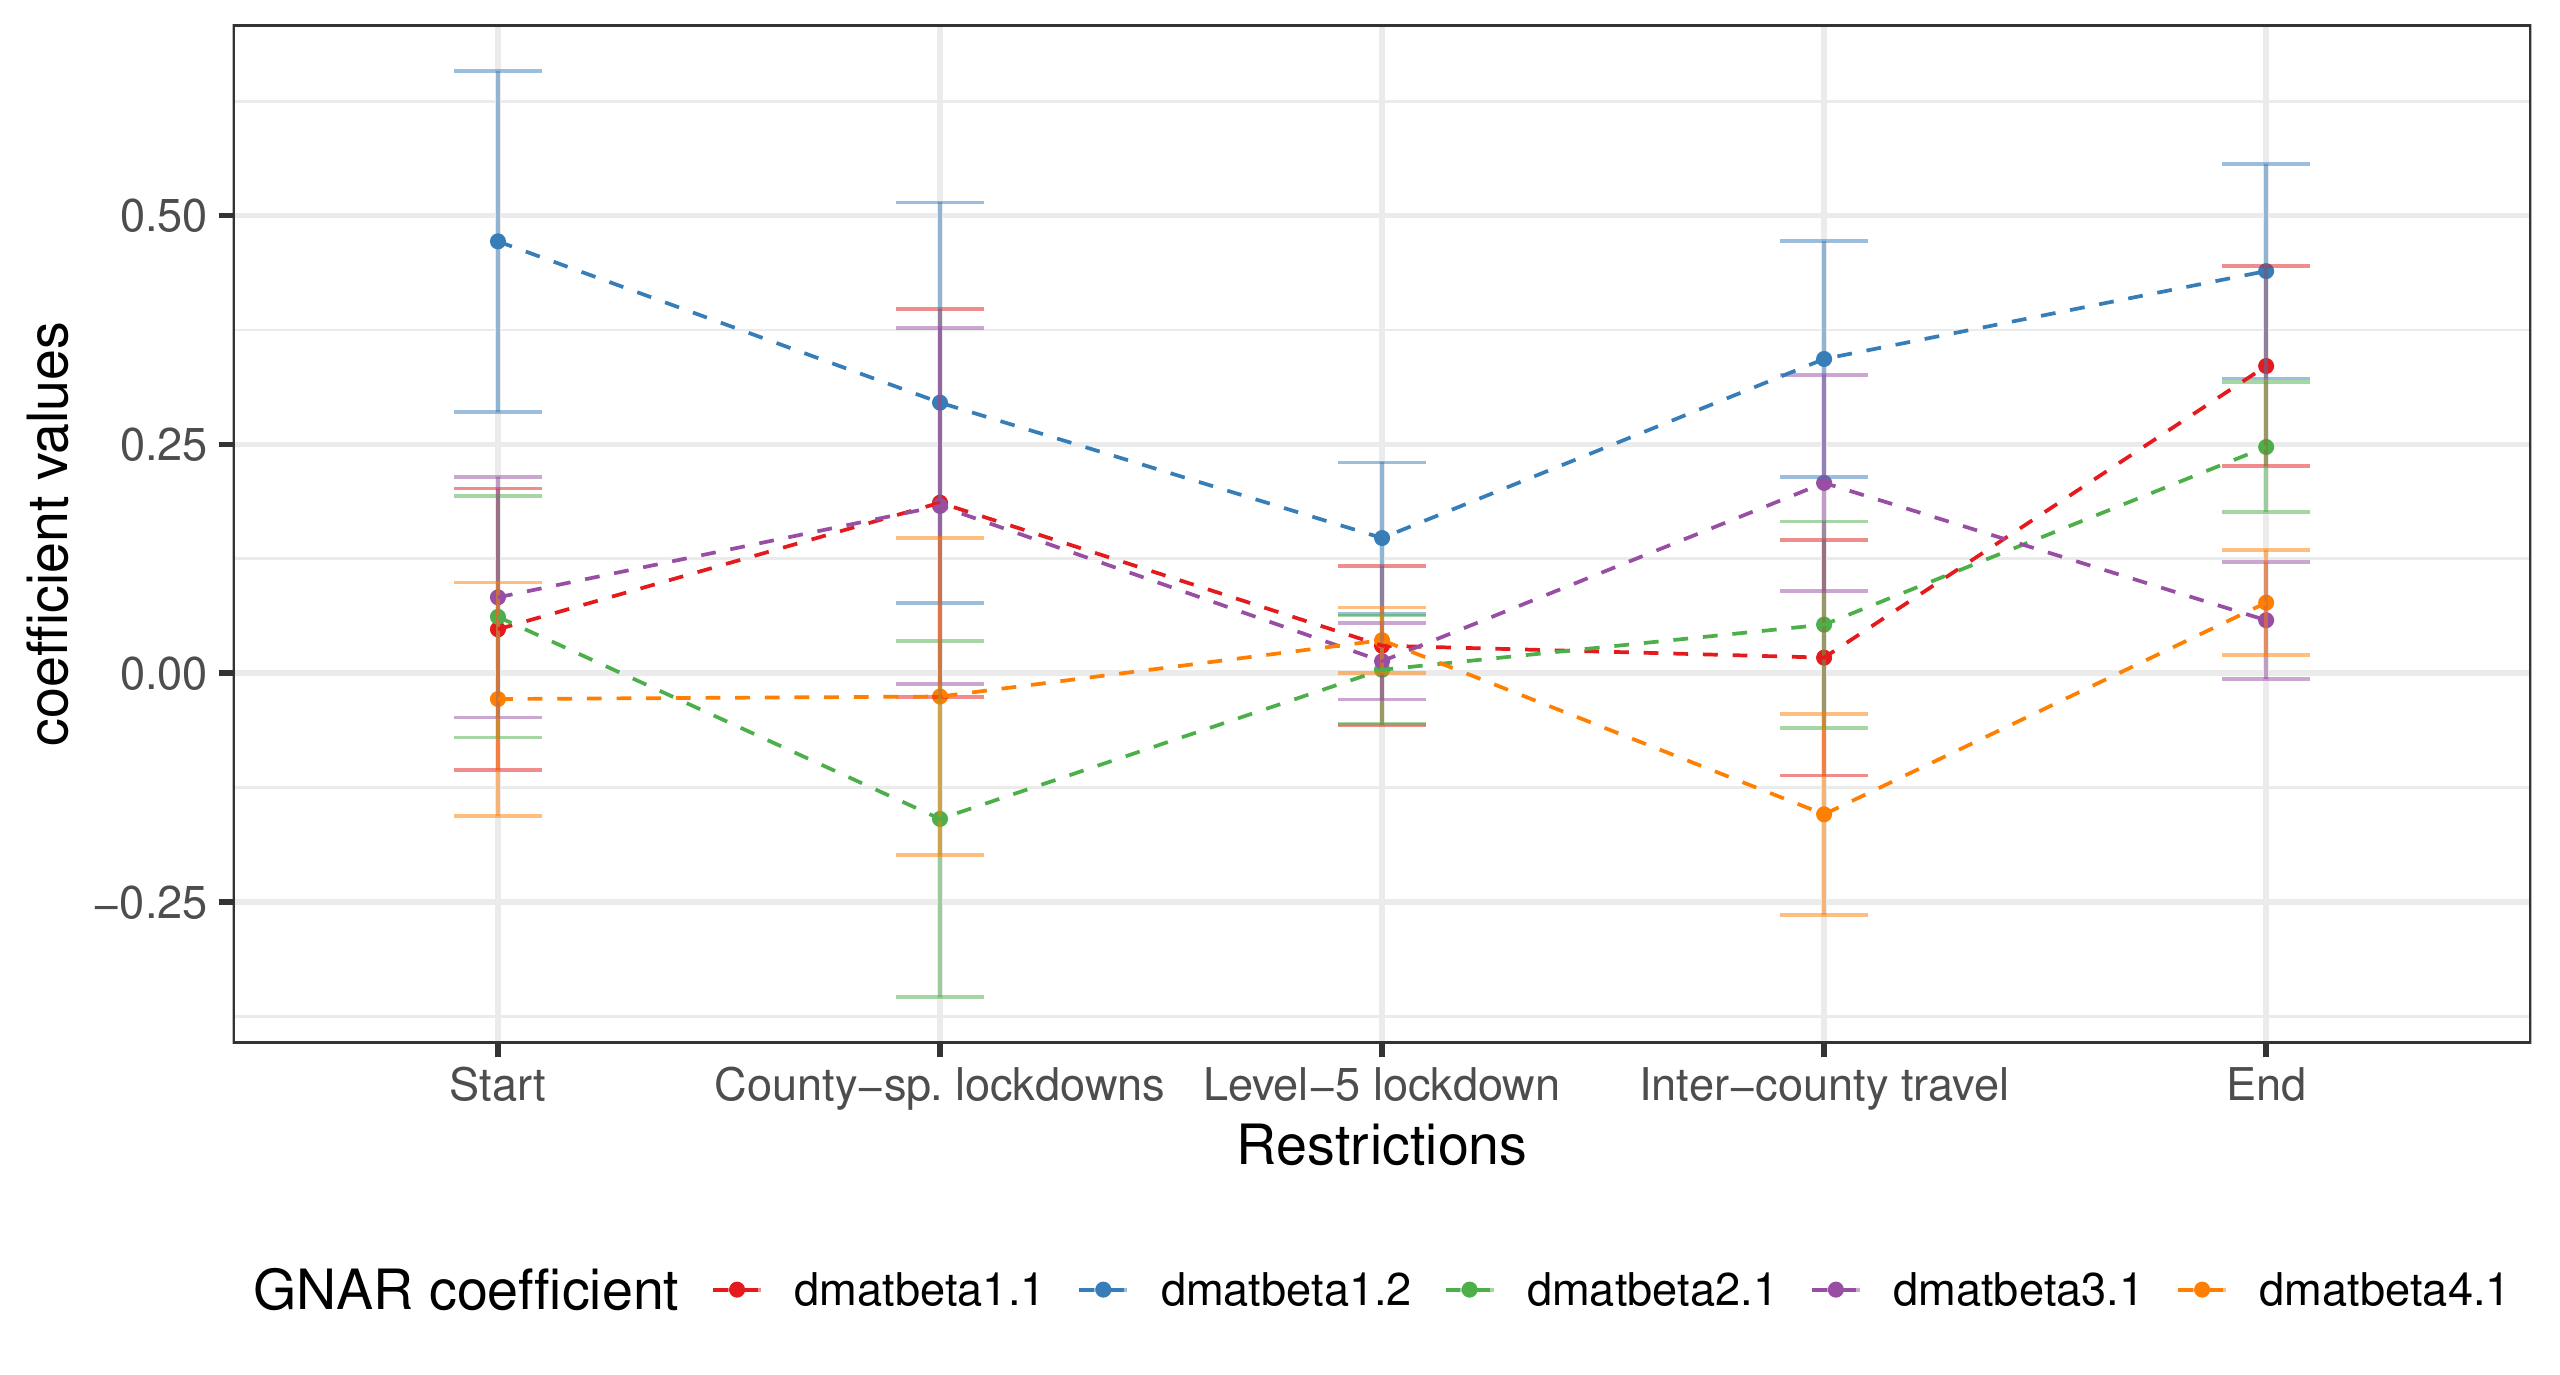}
  \caption{$\beta$-order}
\end{subfigure}
\caption[Change in GNAR model coefficients for COVID-19 regulations for Queen's contiguity network]{Change in coefficients for the global-$\alpha$ \code{GNAR(4,[2,1,1,1])} model across COVID-19 regulations for the \textbf{Queen's contiguity} network}
\label{fig:parameter_queen}
\end{figure}

\begin{figure}[h!]
\centering
\begin{subfigure}{\textwidth}
  \centering
  \includegraphics[scale = 0.4]{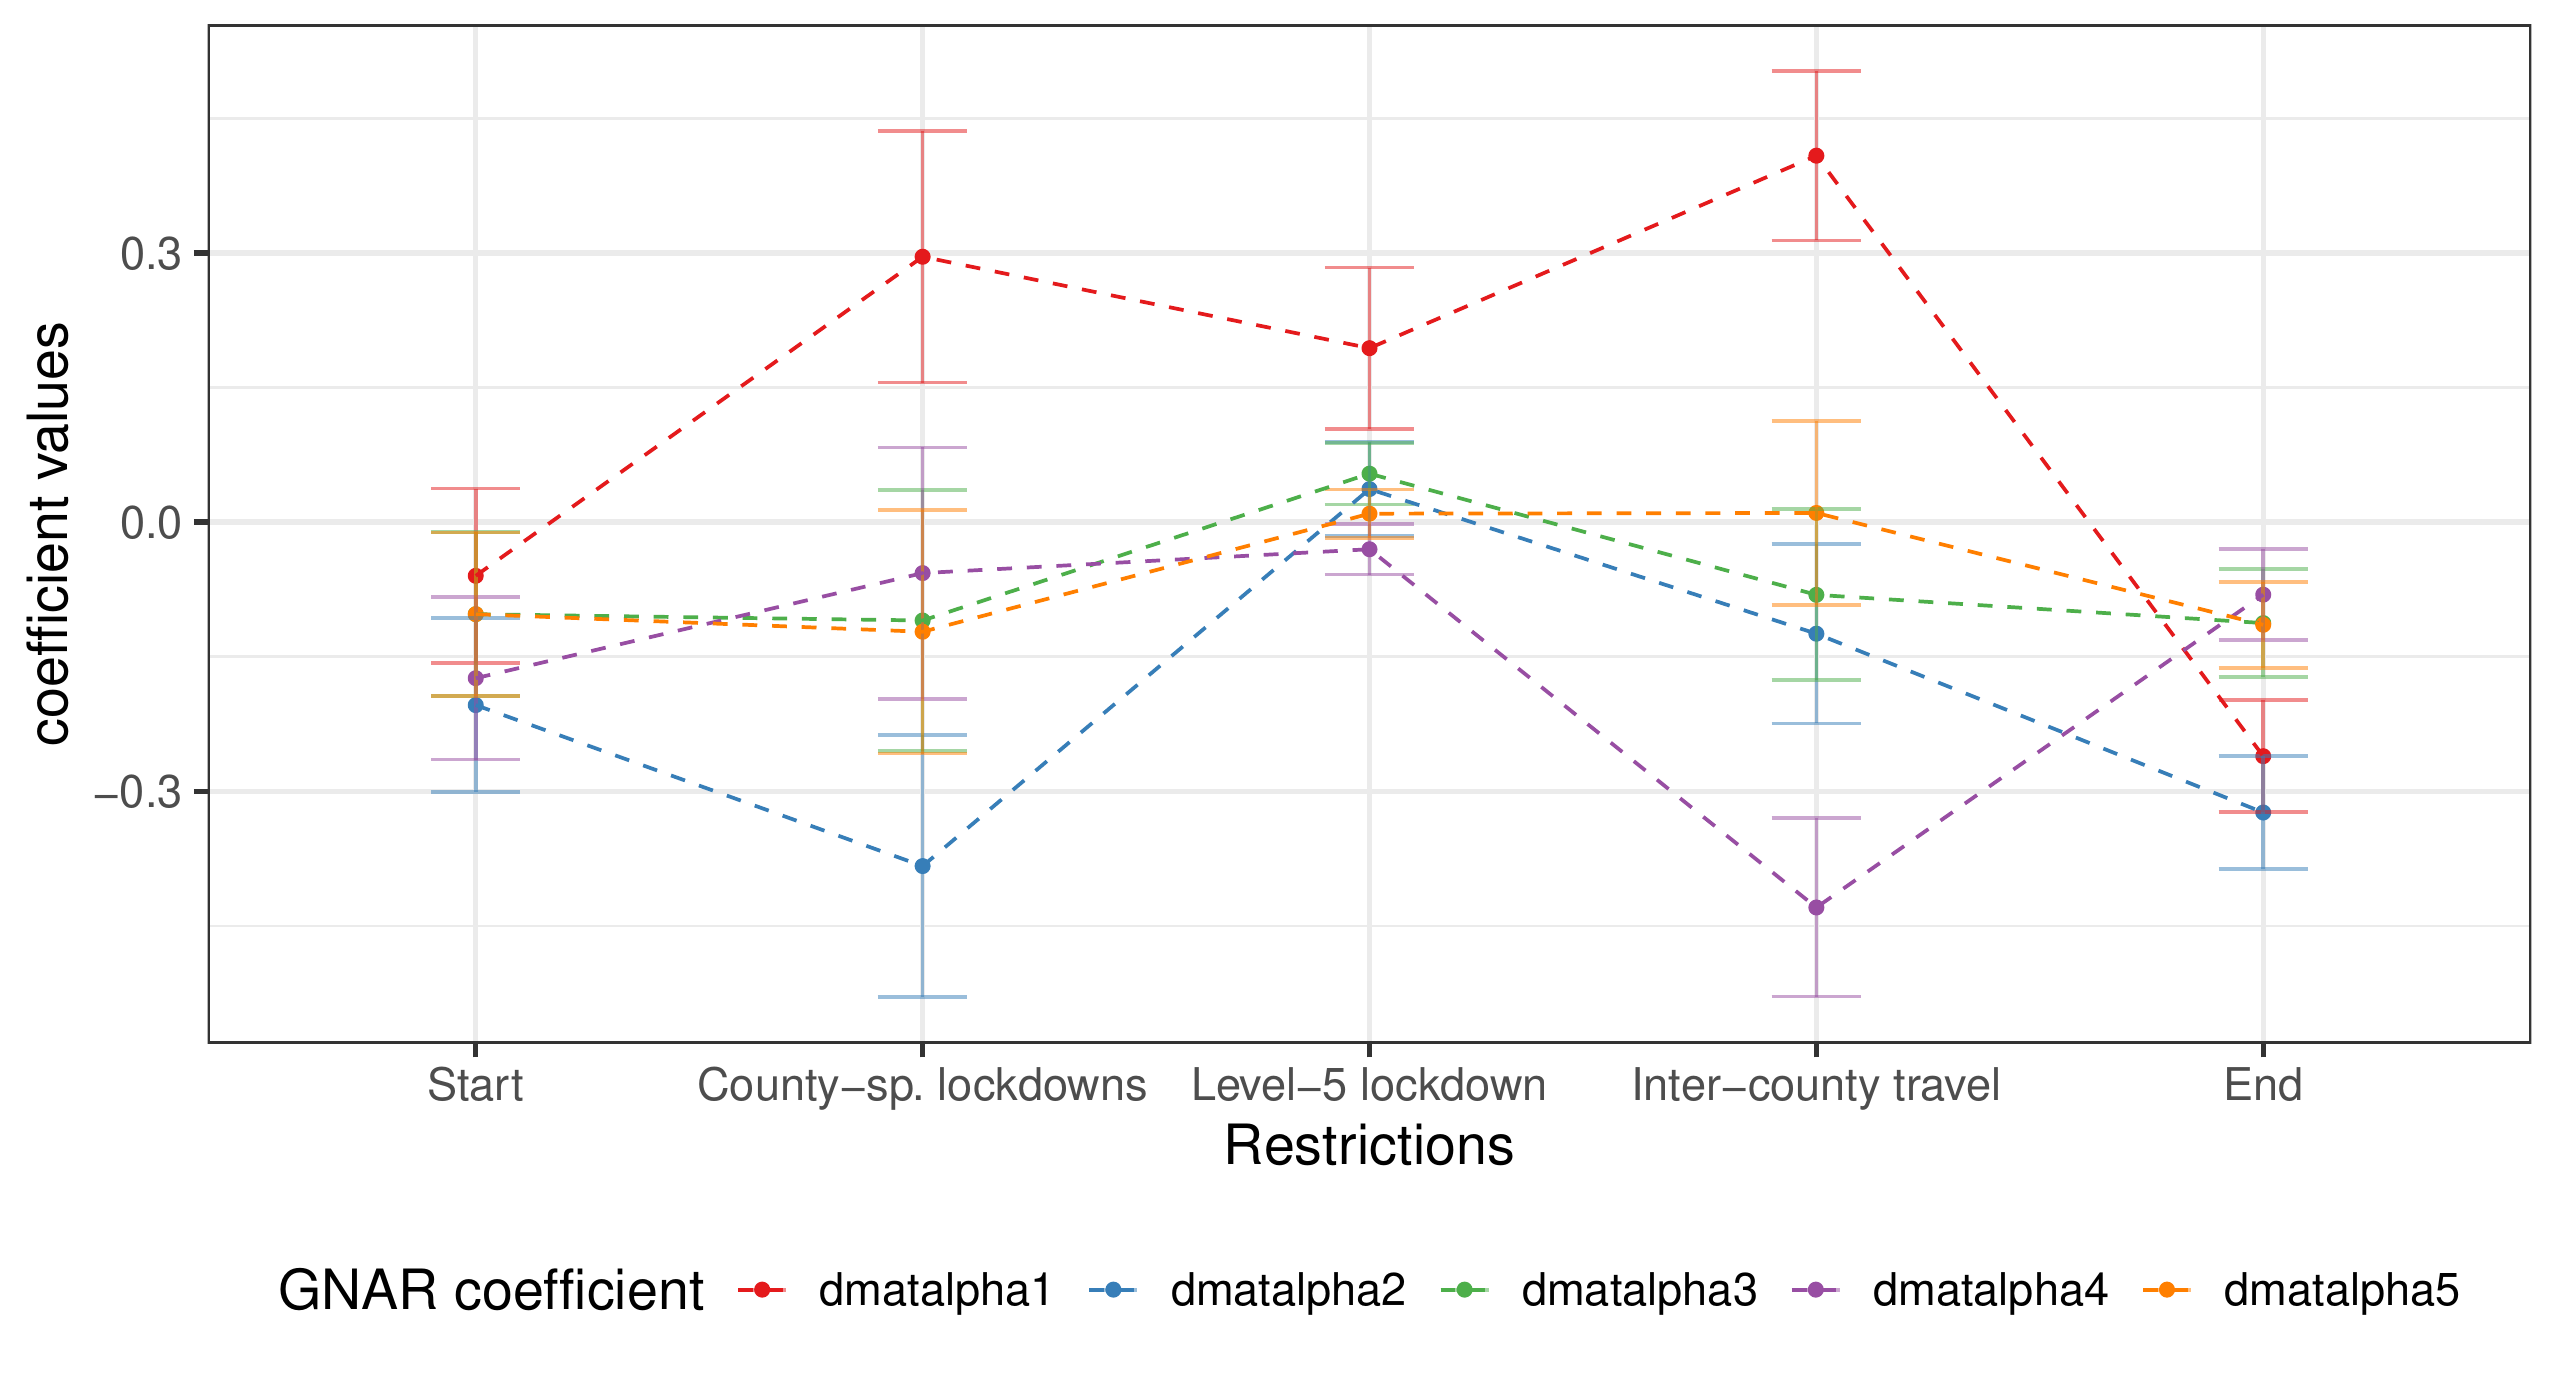}
  \caption{$\alpha$-order}
\end{subfigure}
\begin{subfigure}{\textwidth}
  \centering
  \includegraphics[scale = 0.4]{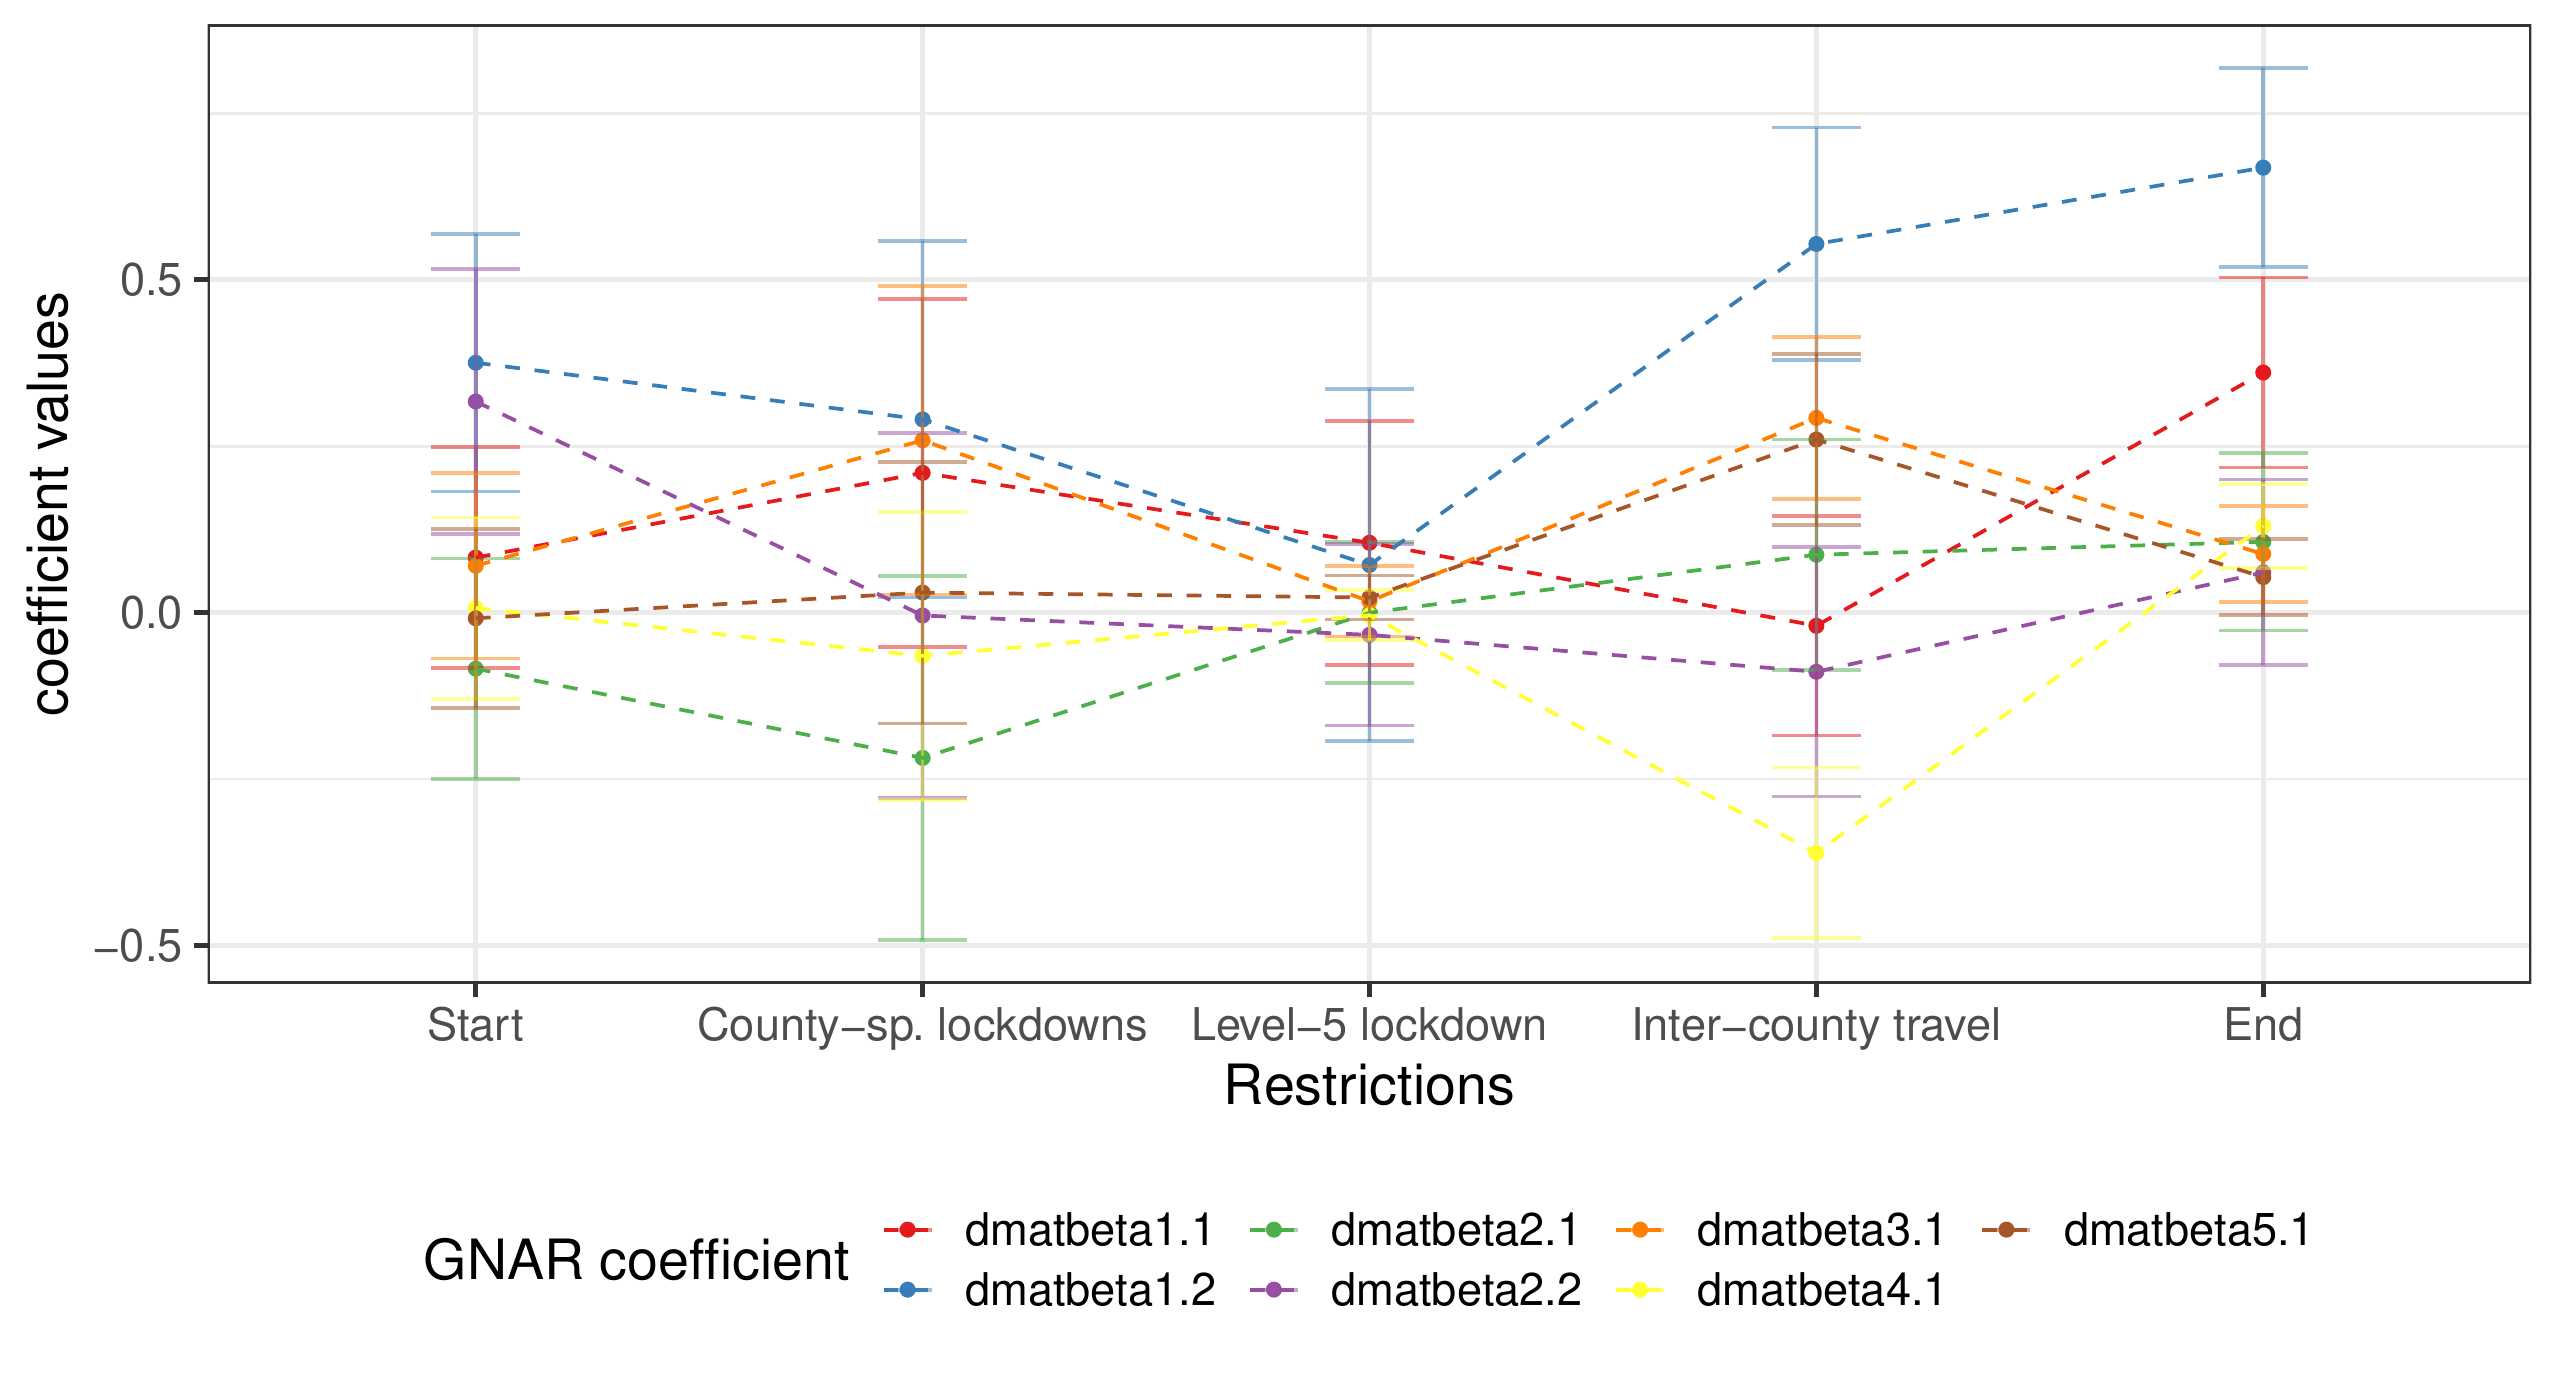}
  \caption{$\beta$-order}
\end{subfigure}
\caption[Change in GNAR model coefficients for COVID-19 regulations for Economic hub network]{Change in coefficients for the global-$\alpha$ \code{GNAR(5,[2,2, 1, 1, 1])} model across COVID-19 regulations for the \textbf{Economic hub} network}
\label{fig:parameter_eco_hub}
\end{figure}

\begin{figure}[h!]
\centering
\begin{subfigure}{\textwidth}
  \centering
  \includegraphics[scale = 0.4]{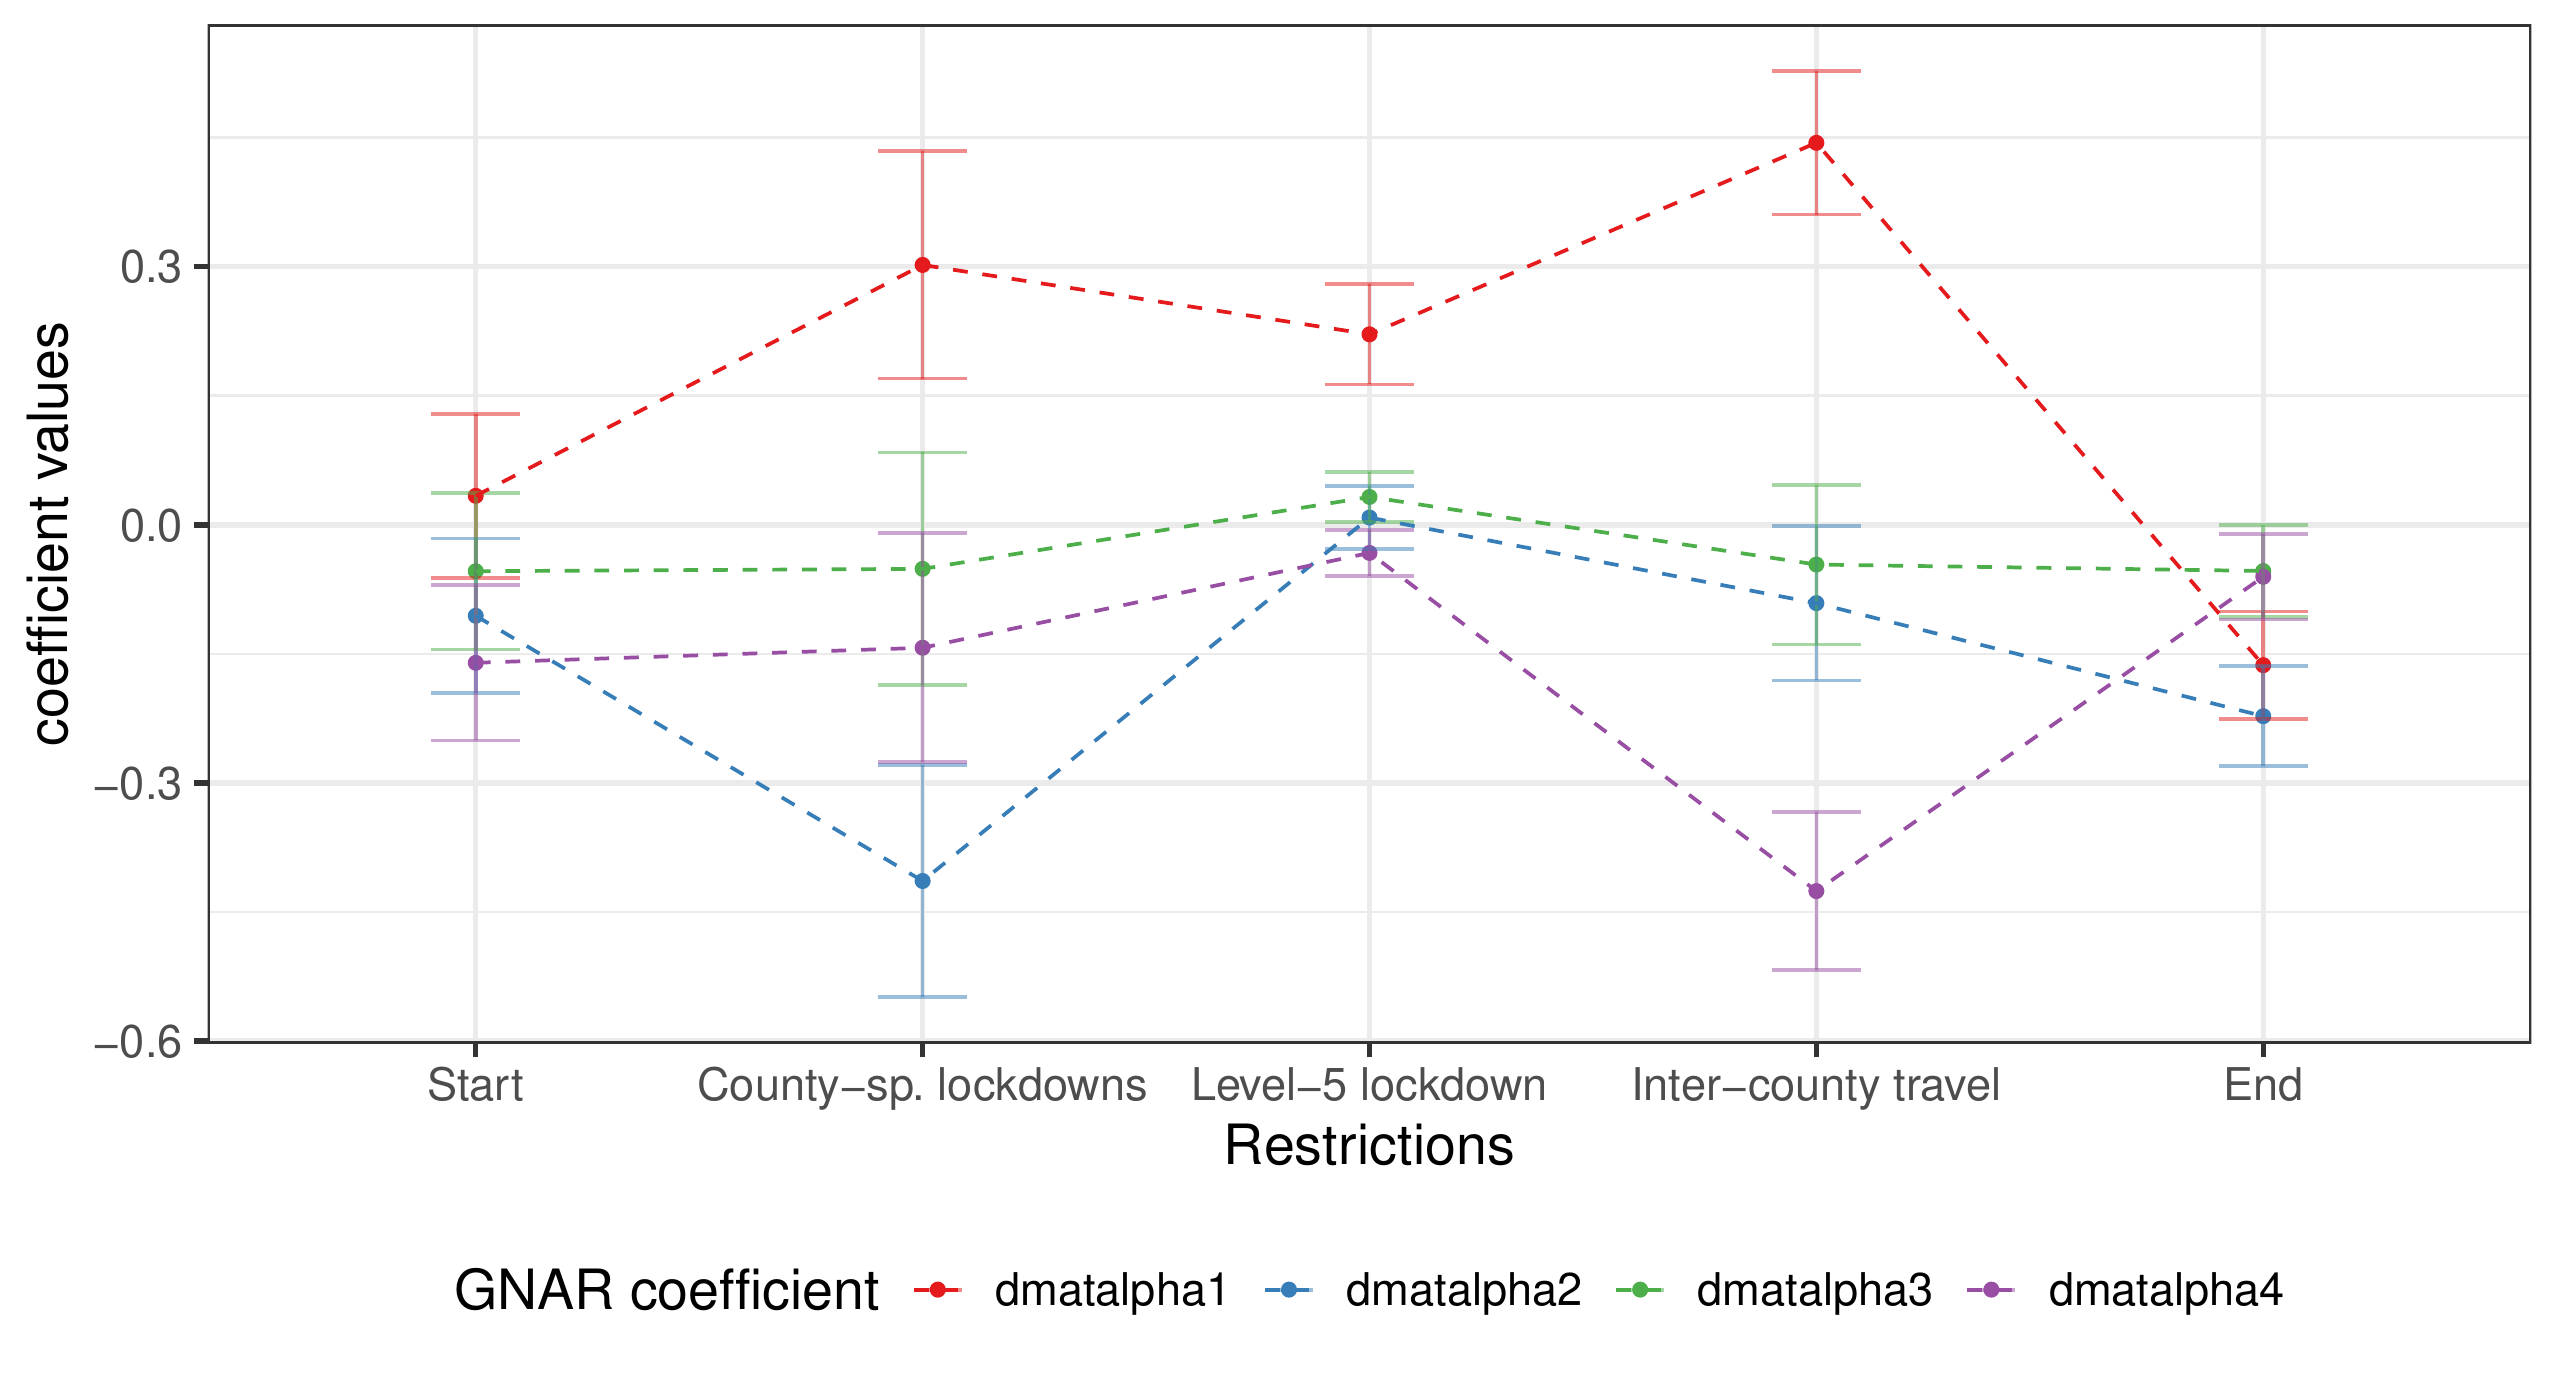}
  \caption{$\alpha$-order}
\end{subfigure}
\begin{subfigure}{\textwidth}
  \centering
  \includegraphics[scale = 0.4]{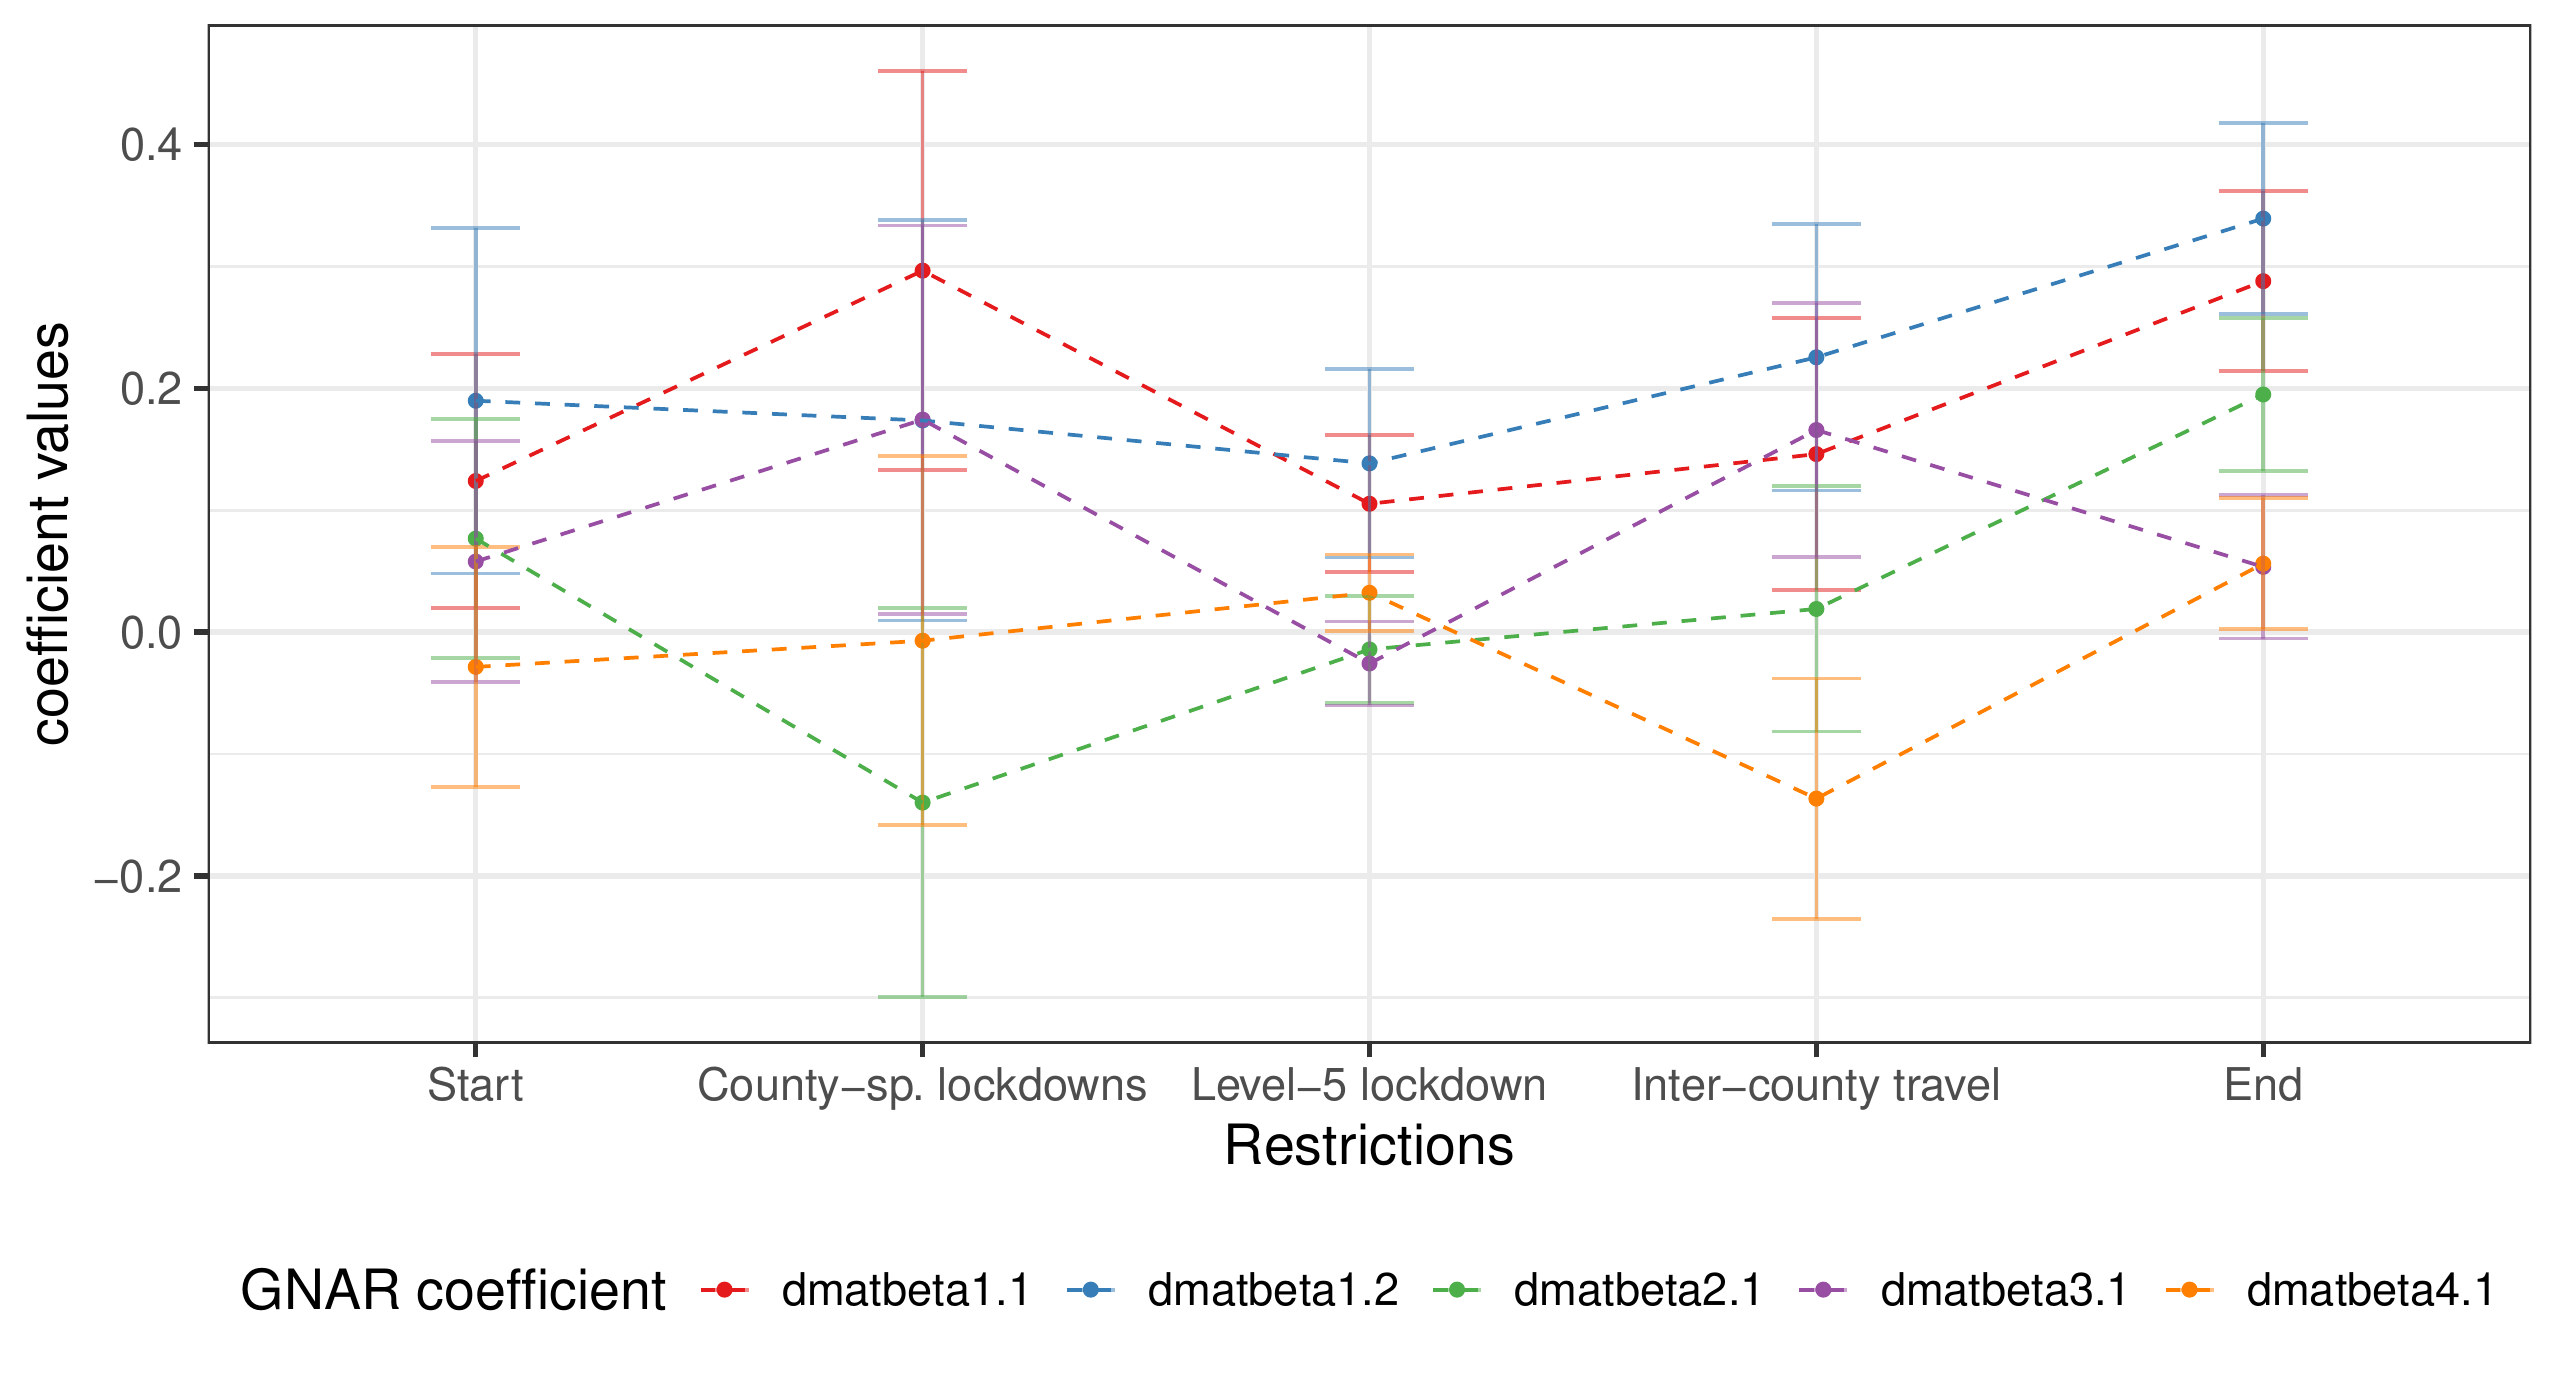}
  \caption{$\beta$-order}
\end{subfigure}
\caption[Change in GNAR model coefficients for COVID-19 regulations for Railway-based network]{Change in coefficients for the global-$\alpha$ \code{GNAR(4,[2,1,1,1])} model across COVID-19 regulations for the \textbf{Railway-based} network}
\label{fig:parameter_train}
\end{figure}

\clearpage

The residuals for other counties (examples Kerry, Wicklow and Donegal) seem Non-Gaussian for the  optimal GNAR models and networks for each data subset, in particular around the boundaries. 
The Kolmogorov-Smirnov test obtains an insignificant result only for dataset 1 across Kerry ($p = 0.9465$), Wicklow ($p = 0.4666$) and Donegal ($p = 0.3099$).
\begin{figure}[h!]
\centering
\subcaptionbox{Subset 1}{\includegraphics[width=0.3\textwidth]{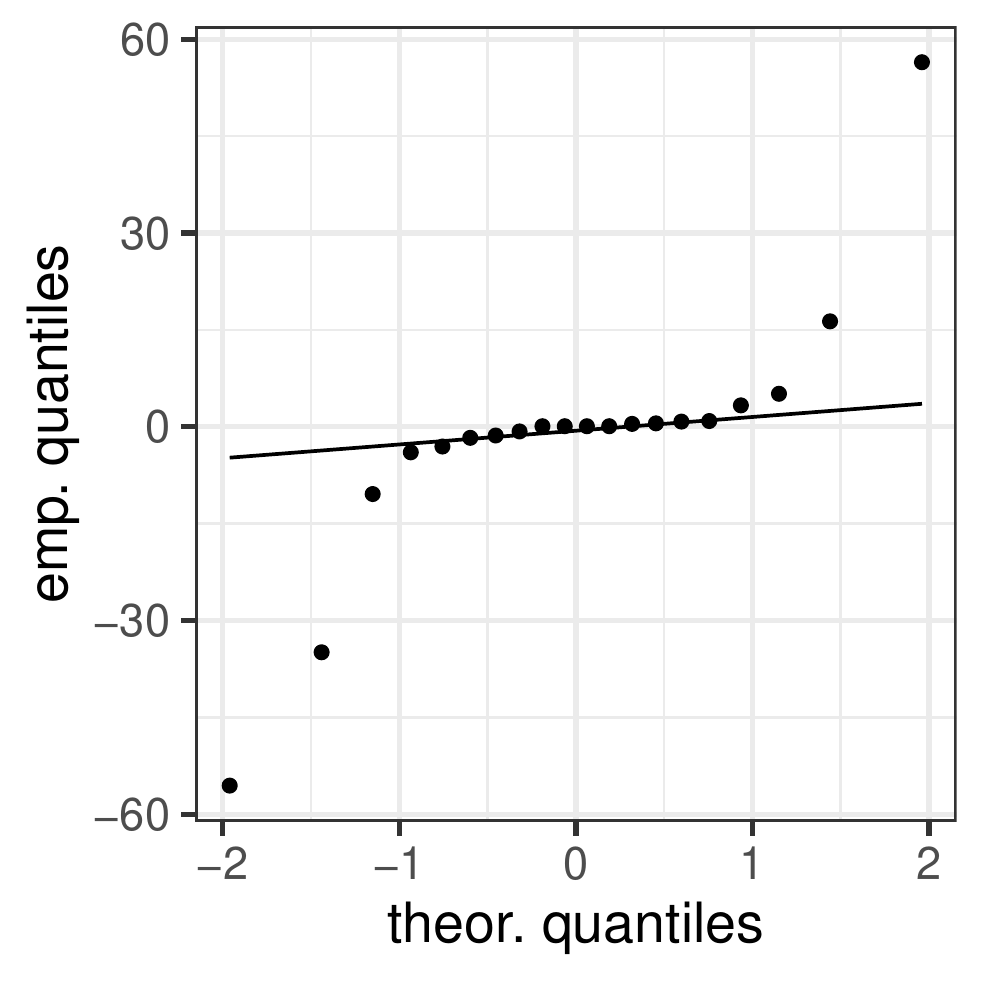}}%
\hspace{1em}
\subcaptionbox{Subset 2}{\includegraphics[width=0.3\textwidth]{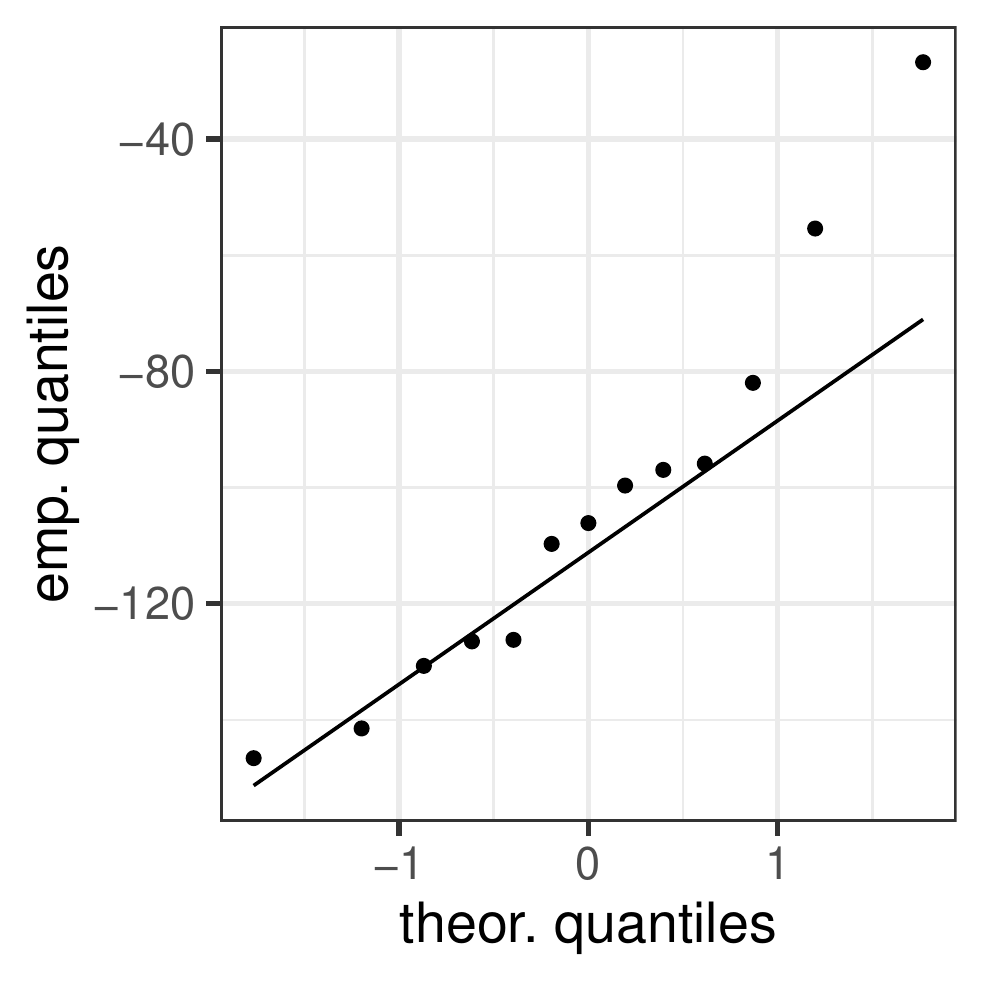}}%
\hspace{1em}
\subcaptionbox{Subset 3}{\includegraphics[width=0.3\textwidth]{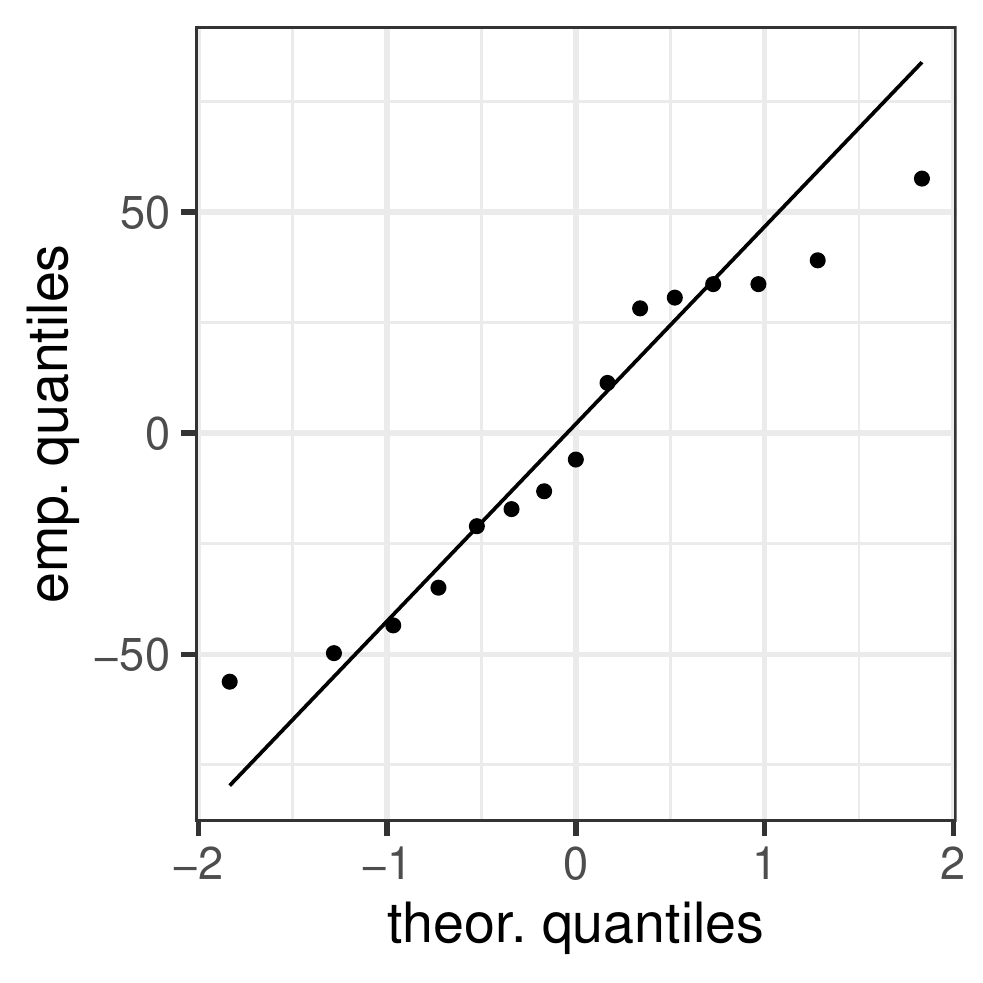}}%
\\
\subcaptionbox{Subset 4}{\includegraphics[width=0.3\textwidth]{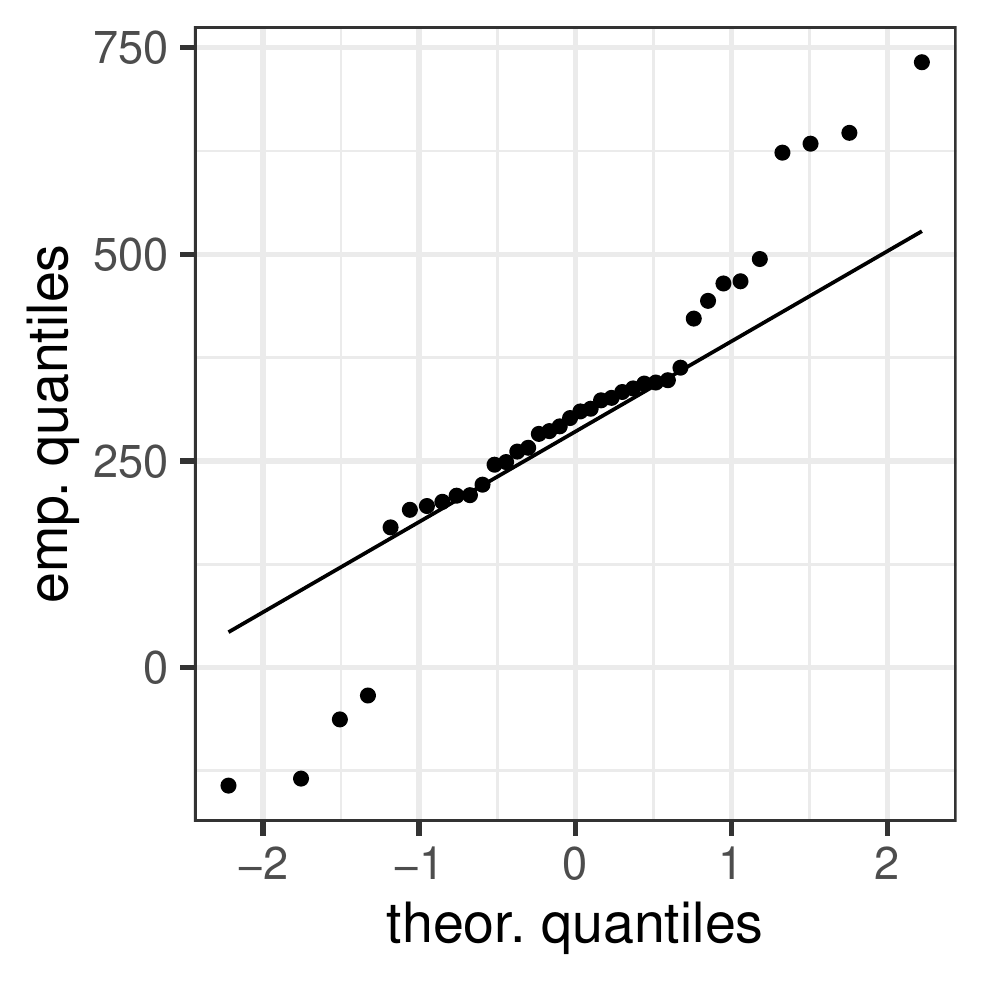}}%
\hspace{1em}
\subcaptionbox{Subset 5}{\includegraphics[width=0.3\textwidth]{Figures/qq_subset_5_eco_hub_county_Dublin.pdf}}%
\caption{QQ plot for the residuals from the best performing GNAR model and network for dataset 1-5; shown for county Donegal}
\label{fig:qq_subsets_donegal}
\end{figure}

\begin{figure}[h!]
\centering
\subcaptionbox{Subset 1}{\includegraphics[width=0.3\textwidth]{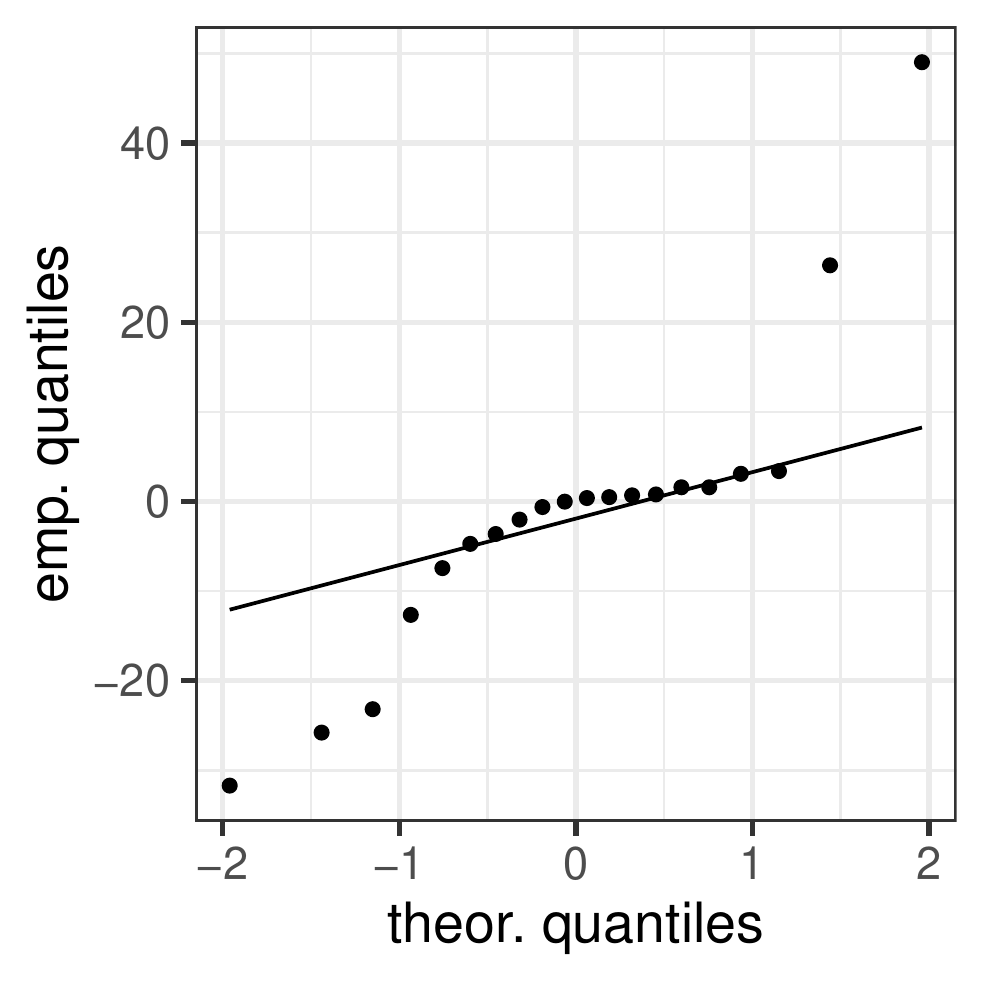}}%
\hspace{1em}
\subcaptionbox{Subset 2}{\includegraphics[width=0.3\textwidth]{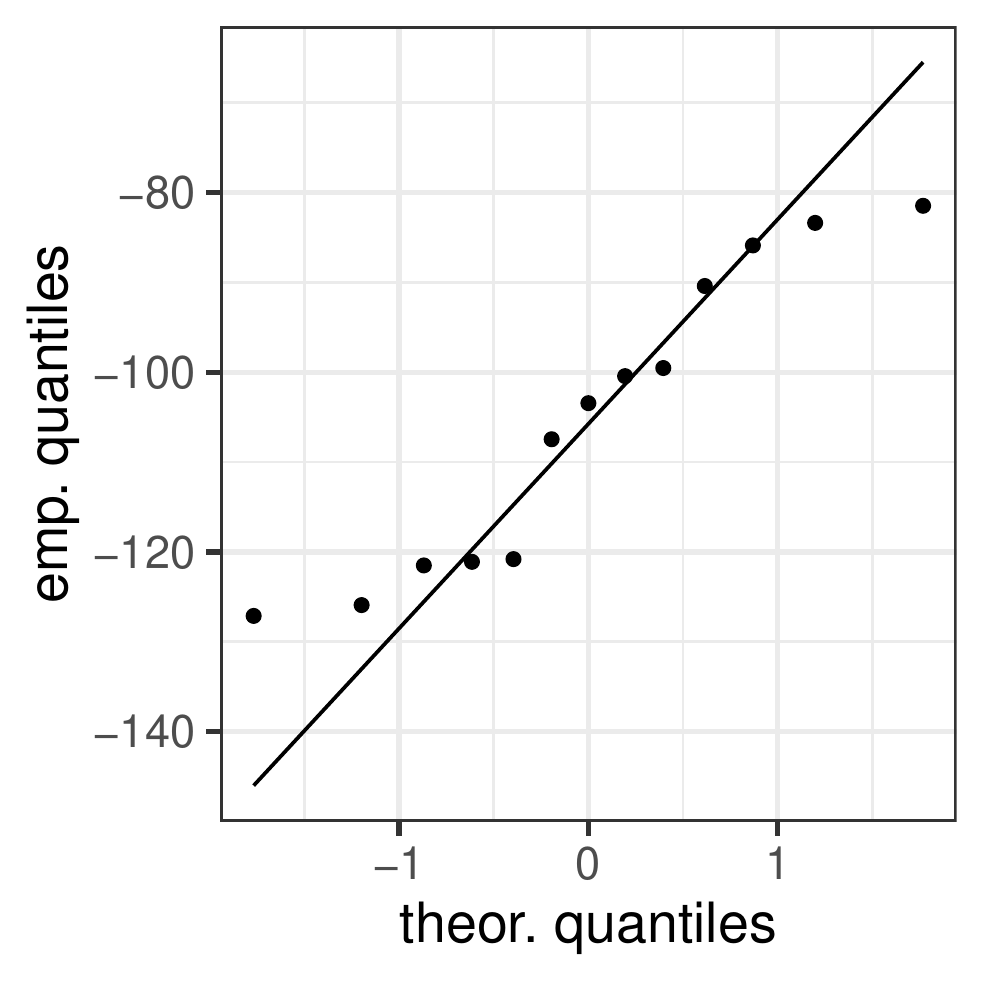}}%
\hspace{1em}
\subcaptionbox{Subset 3}{\includegraphics[width=0.3\textwidth]{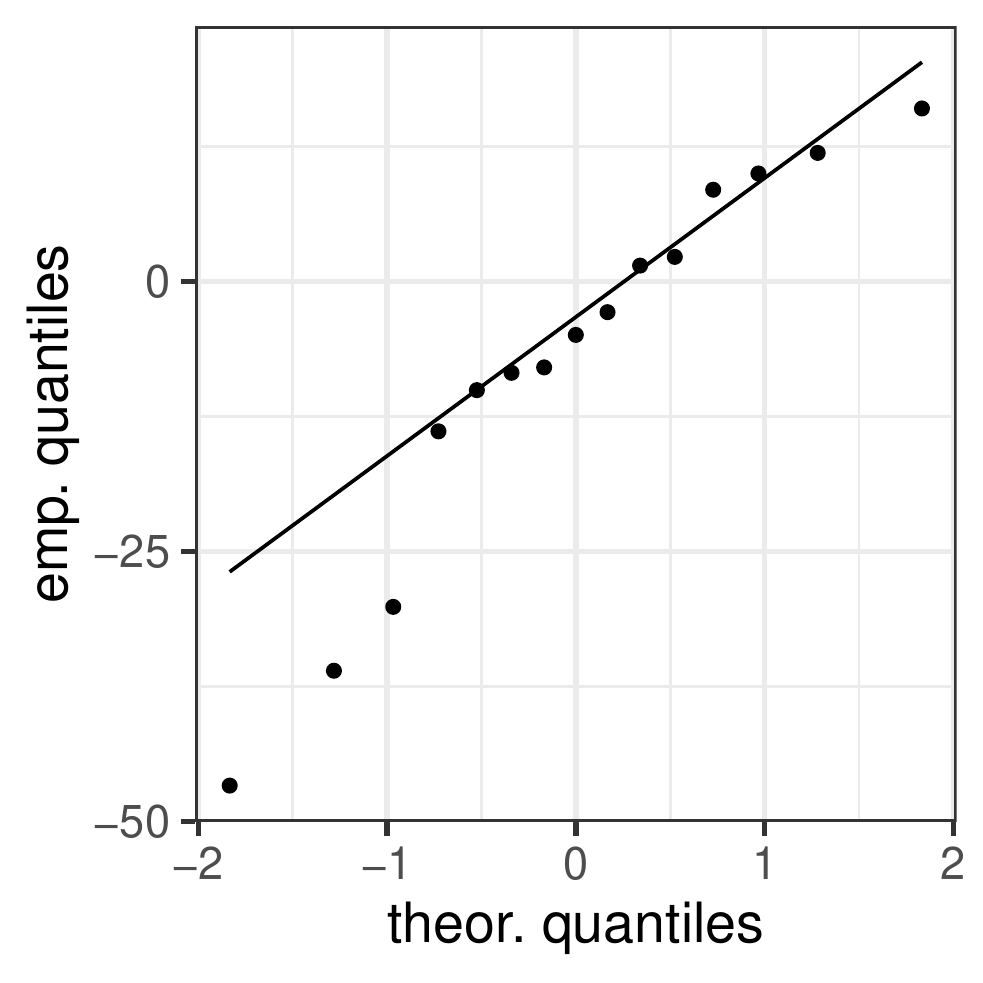}}%
\\
\subcaptionbox{Subset 4}{\includegraphics[width=0.3\textwidth]{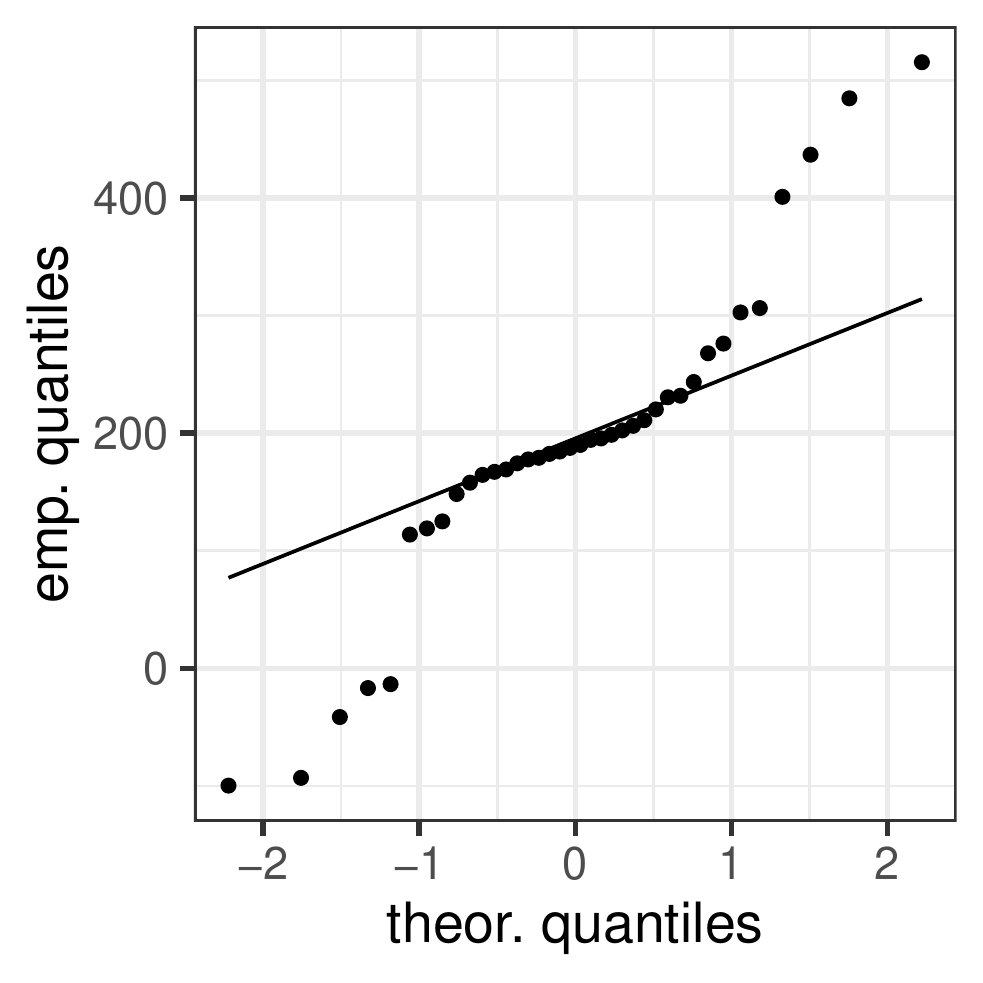}}%
\hspace{1em}
\subcaptionbox{Subset 5}{\includegraphics[width=0.3\textwidth]{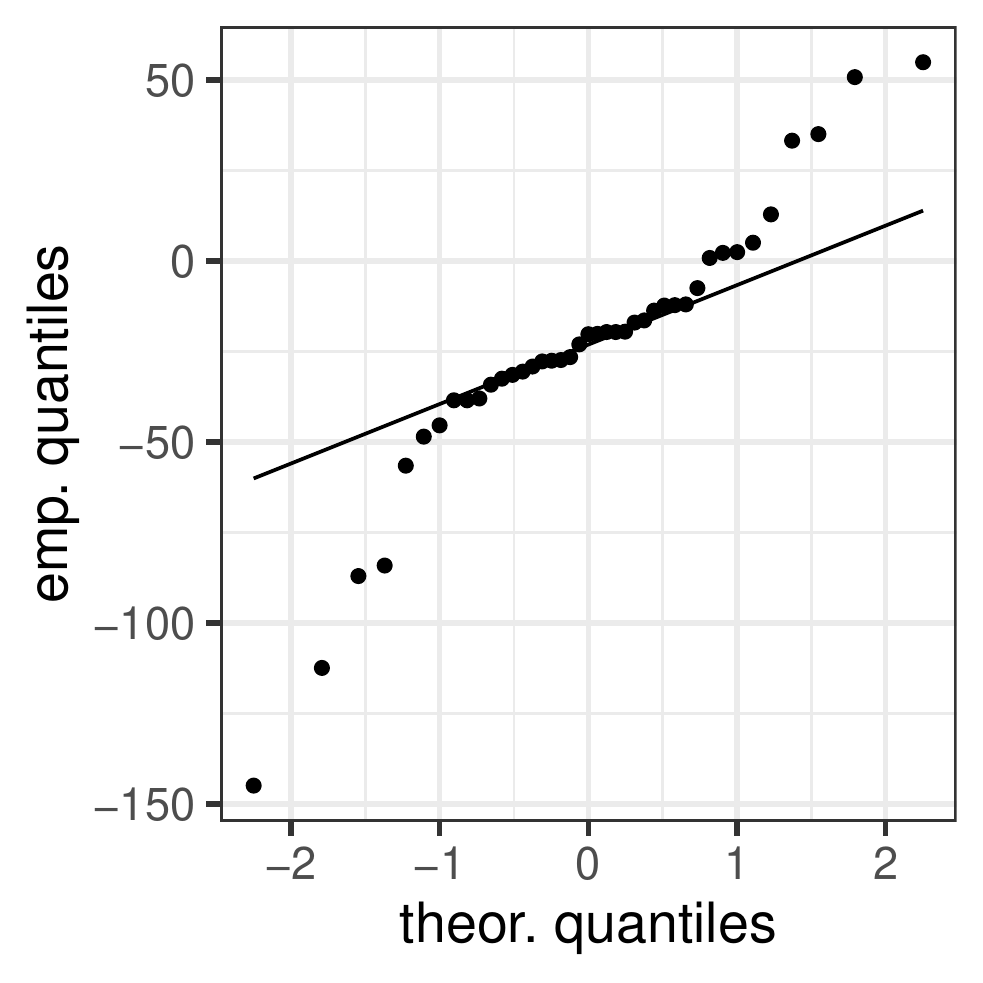}}%
\caption{QQ plot for the residuals from the best performing GNAR model and network for dataset 1-5; shown for county Wicklow}
\label{fig:qq_subsets_wicklow}
\end{figure}

\begin{figure}[h!]
\centering
\subcaptionbox{Subset 1}{\includegraphics[width=0.3\textwidth]{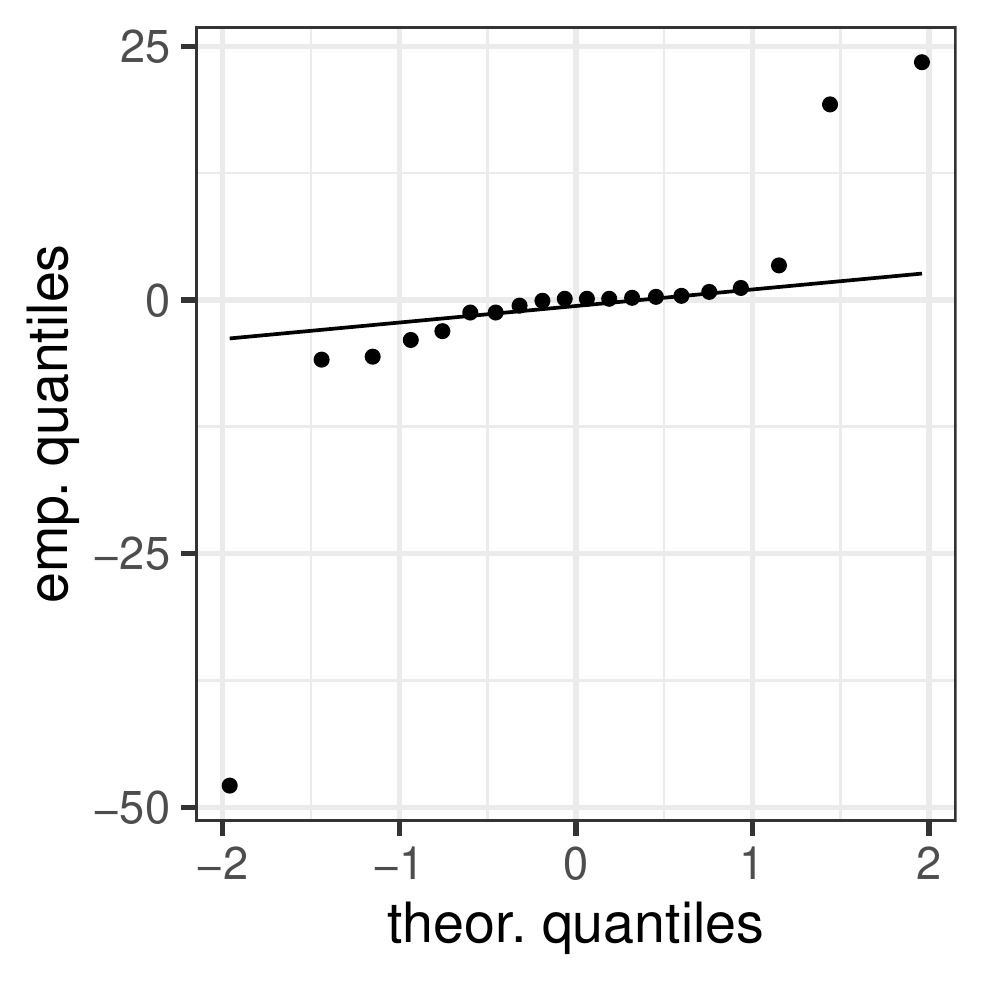}}%
\hspace{1em}
\subcaptionbox{Subset 2}{\includegraphics[width=0.3\textwidth]{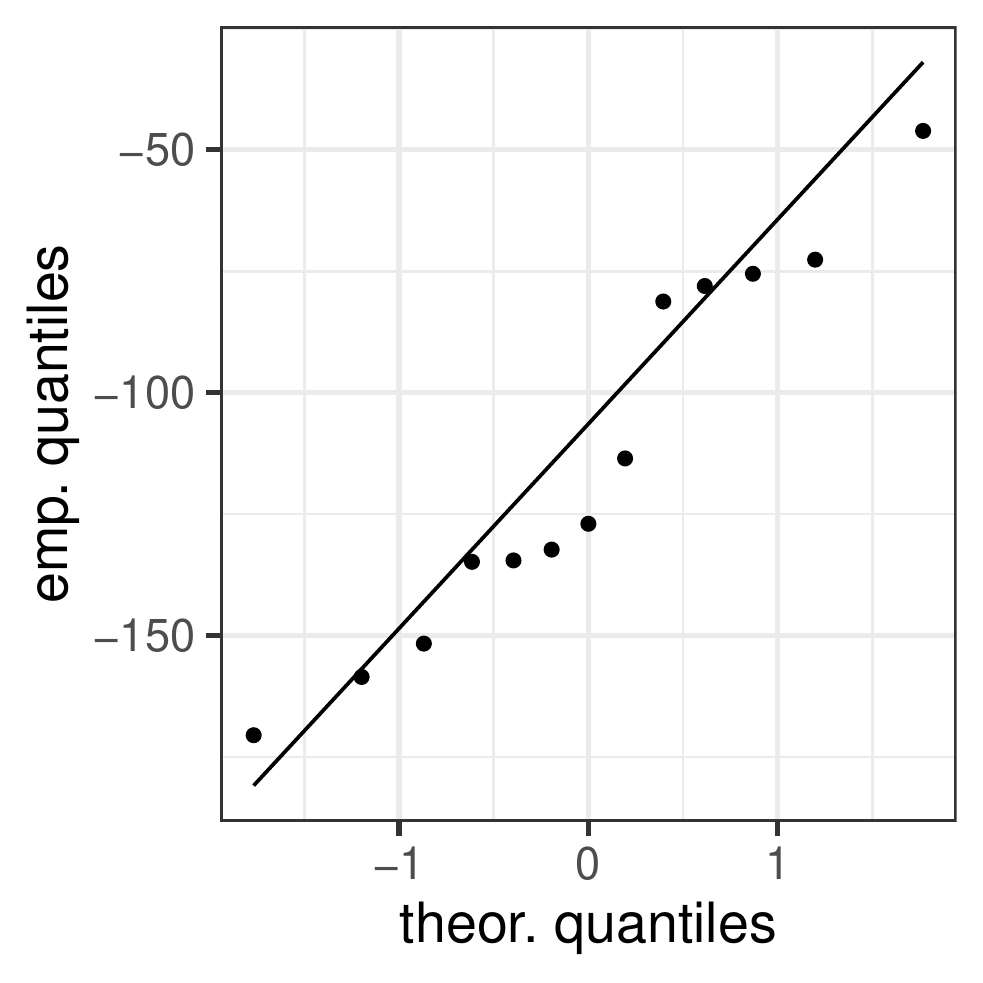}}%
\hspace{1em}
\subcaptionbox{Subset 3}{\includegraphics[width=0.3\textwidth]{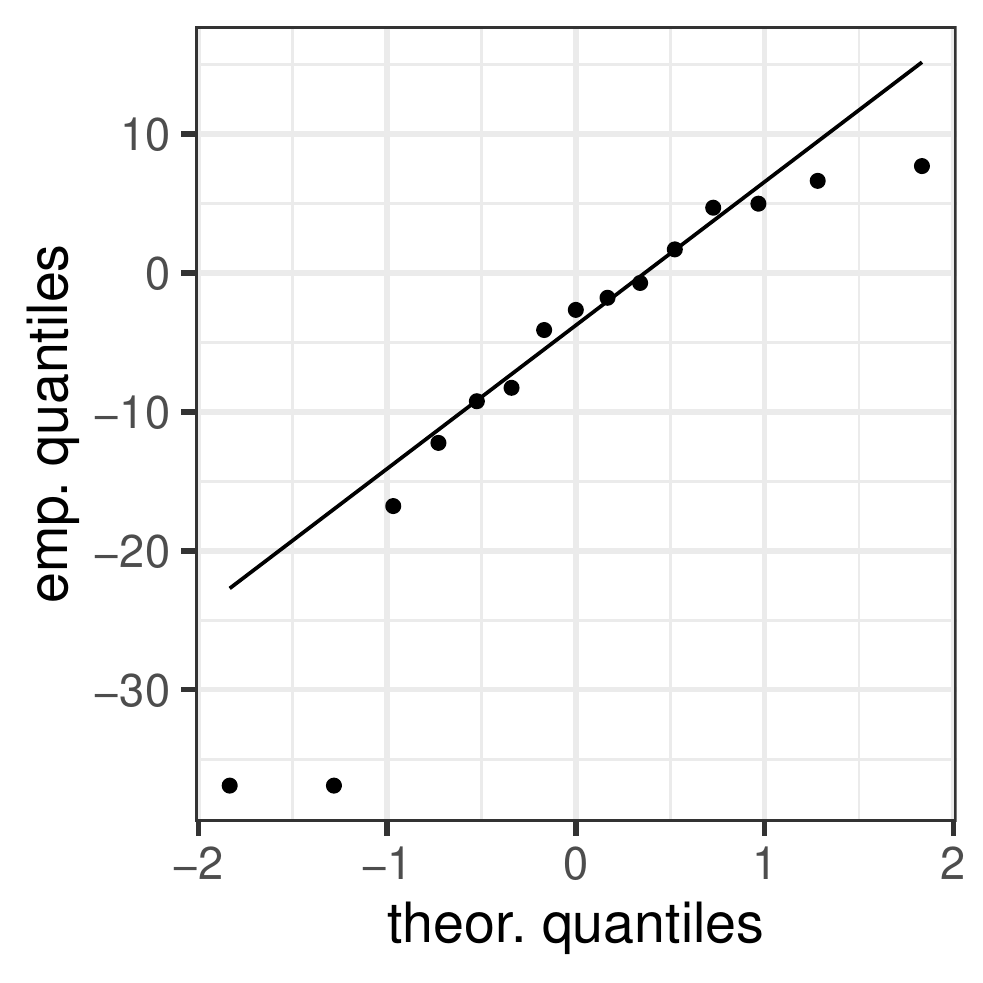}}%
\\
\subcaptionbox{Subset 4}{\includegraphics[width=0.3\textwidth]{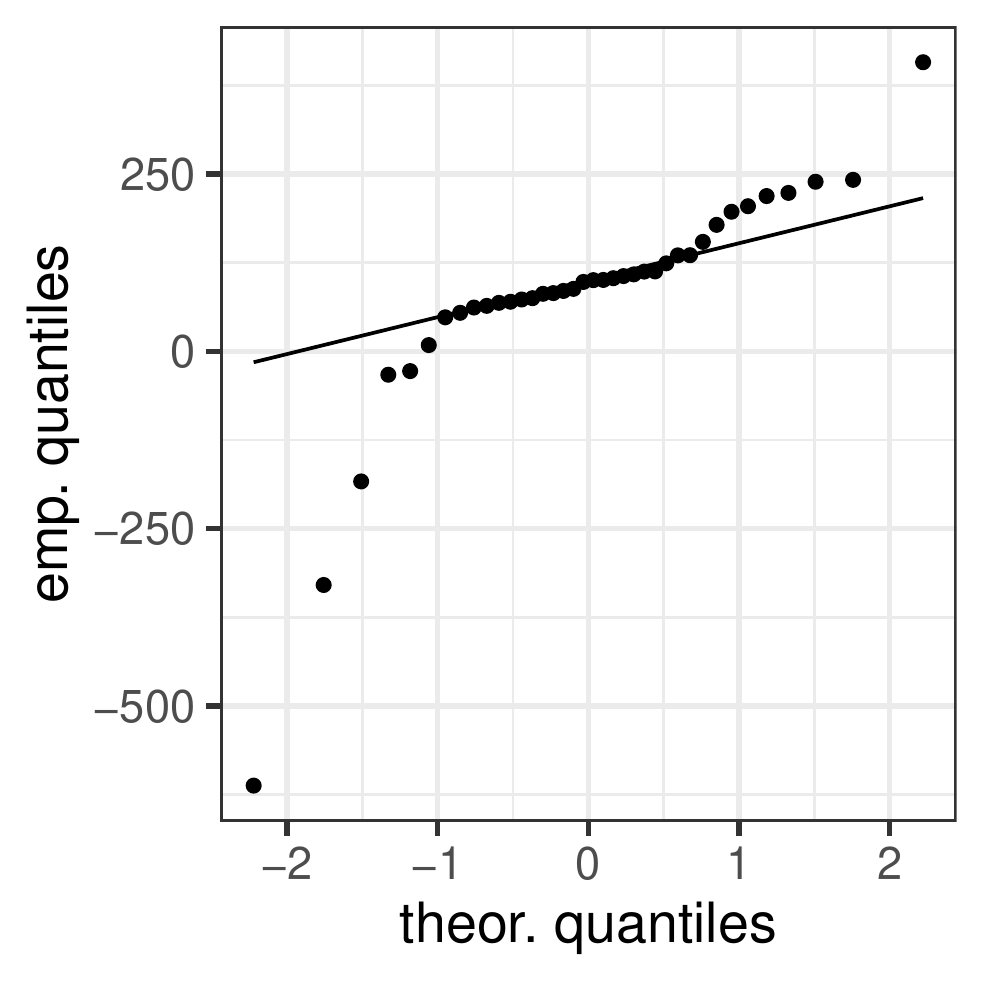}}%
\hspace{1em}
\subcaptionbox{Subset 5}{\includegraphics[width=0.3\textwidth]{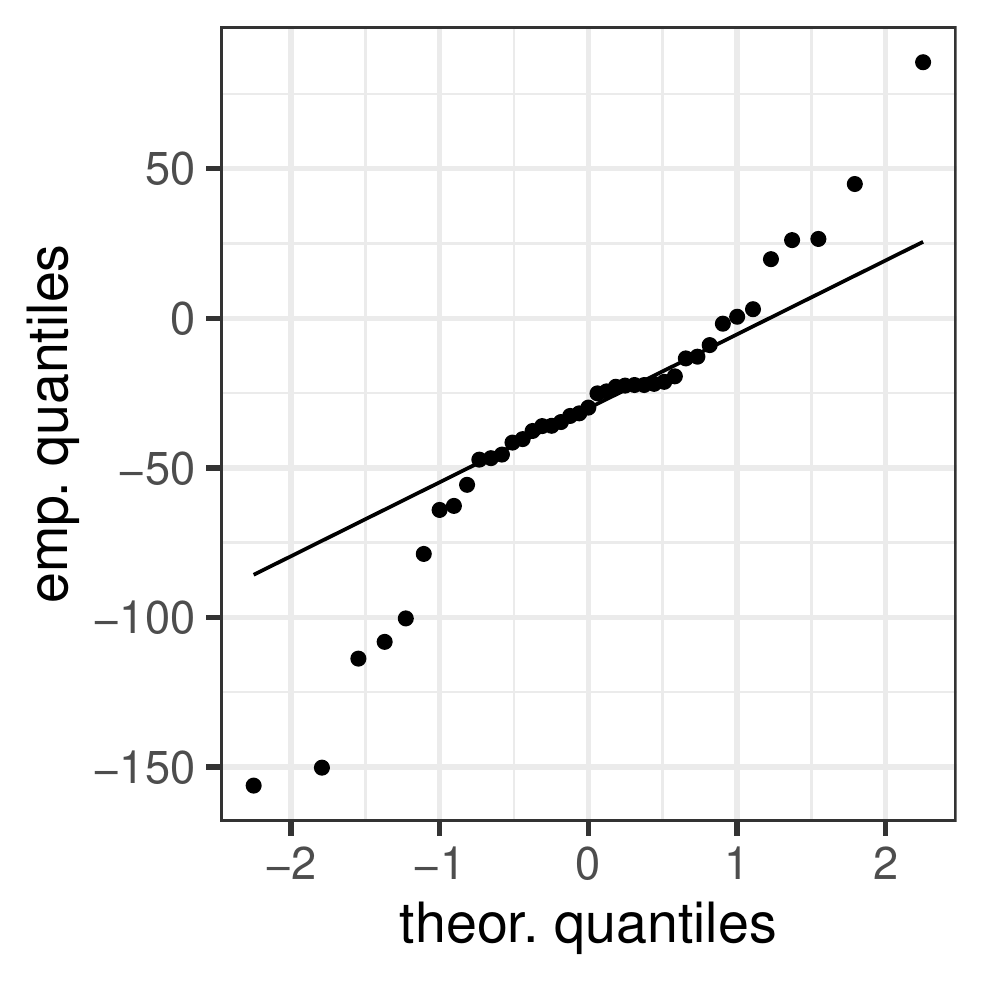}}%
\caption{QQ plot for the residuals from the best performing GNAR model and network for dataset 1-5; shown for county Kerry}
\label{fig:qq_subsets_kerry}
\end{figure}
