# Supplementary material for: COVID-19 incidence in the Republic of Ireland: A case study for network-based time series models
Source: arXiv:2307.06199 source file (2024-06-05)
Supplement: Supplementary file 4 [file Simulation.tex]

\section{Simulation}
\label{app:simulation}
To establish how well the GNAR model in general can reconstruct the data generating method, data is simulated according to the \code{GNAR-5-21111} model on the Queen's contiguity network. 
Choosing $s = (2, 1, 1, 1, 1)$, iid.\,error term $\varepsilon_{i, t} \sim N(0, \sigma^2)$ with $\sigma^2 = 0.01$ and $\sigma^2 = 0.001$ and SPL weights, i.e.\,$\omega_{i, q} = \frac{1}{|N^{(r)}(i)|}$ where $| N^{(r)}(i)|$ denotes the number of vertices in the $r^{\,th}$-stage neighbourhood for $i$ and the first 5 time points are initialized as $X_{i, t} \sim N(10, \sigma^2)$ iid., the outcome $X_i$ for county $i$ and timesteps $t = 6, \dots, 1000$ follows from
\begin{align*}
    X_{i, t} = \sum_{j = 1}^5 \left( \alpha_{i,j} X_{i, t-j} + \sum_{r = 1}^{s_j} \sum_{q \in N^{(r)}(i)} \beta_{j, r} \, \omega_{i, q} \, X_{q, t-j} \right) + \varepsilon_{i, t} 
\end{align*}
The simulated data is leveraged to train a GNAR model on the Queen's contiguity network.
Tables \ref{tab:coef_testing_queen_01} ($\sigma^2 = 0.01$) and \ref{tab:coef_testing_queen_001} ($\sigma^2 = 0.001$) compare the true and estimated GNAR model coefficients. 
The estimated confidence interval contains the true coefficient value only for no coefficient in the setting $\sigma^2 = 0.01$ and for one coefficients, $\alpha_4$, in the setting $\sigma^2 = 0.001$. 
Despite small noise, the GNAR model is incapable of correctly detecting the temporal and spatial dependence in the simulated data.

\begin{table}[ht]
\centering
\begin{tabular}{c|rr}
  \toprule 
 Coefficient & real value & re-computed value [95\% CI] \\
 \midrule 
 $\alpha_1$ & 0.18 & 0.22 [0.21, 0.23] \\ 
  $\beta_{1, 1}$ & 0.14 & 0.01 [-0.01, 0.03] \\ 
  $\beta_{1, 2}$ & 0.41 & -0.04 [-0.06, -0.02] \\ 
  $\alpha_2$ & -0.19 & -0.02 [-0.03, -0.01] \\ 
  $\beta_{2, 1}$ & -0.07 & -0.05 [-0.06, -0.03] \\ 
  $\alpha_3$ & -0.09 & 0.26 [0.25, 0.27] \\ 
  $\beta_{3, 1}$ & 0.03 & -0.03 [-0.04, -0.01] \\ 
  $\alpha_4$ & -0.17 & 0.17 [0.15, 0.18] \\ 
  $\beta_{4, 1}$ & 0.14 & 0.02 [0.01, 0.04] \\ 
  $\alpha_5$ & -0.11 & 0.09 [0.08, 0.1] \\ 
  $\beta_{5, 1}$ & 0.01 & -0.02 [-0.03, -0.01] \\ 
   \bottomrule 
\end{tabular}
\caption{Coefficients for the \code{GNAR} model serving the data simulation 
and their re-computed values after fitting the \code{GNAR} model to the simulated data 
and their 95\% confidence interval (CI) for the \textbf{Queen's contiguity} network; 
the variance for the random error is set to $\sigma^2 = 0.01$.} 
\label{tab:coef_testing_queen_01}
\end{table}

\begin{table}[ht]
\centering
\begin{tabular}{c|rr}
  \toprule 
 Coefficient & real value & re-computed value [95\% CI] \\
 \midrule 
 $\alpha_1$ & 0.18 & -0.04 [-0.05, -0.03] \\ 
  $\beta_{1, 1}$  & 0.14 & 0 [-0.02, 0.01] \\ 
  $\beta_{1, 2}$  & 0.41 & 0.04 [0.02, 0.06] \\ 
  $\alpha_2$ & -0.19 & -0.08 [-0.09, -0.07] \\ 
  $\beta_{2, 1}$  & -0.07 & -0.11 [-0.12, -0.1] \\ 
  $\alpha_3$ & -0.09 & 0 [-0.01, 0.01] \\ 
  $\beta_{3, 1}$  & 0.03 & -0.08 [-0.09, -0.07] \\ 
  \textbf{$\alpha_4$} & -0.17 & -0.18 [-0.19, -0.17] \\ 
  $\beta_{4, 1}$  & 0.14 & 0.03 [0.02, 0.04] \\ 
  $\alpha_5$ & -0.11 & 0.21 [0.2, 0.22] \\ 
  $\beta_{5, 1}$  & 0.01 & -0.03 [-0.04, -0.02] \\ 
   \bottomrule 
\end{tabular}
\caption{Coefficients for the \code{GNAR} model serving the data simulation 
and their re-computed values after fitting the \code{GNAR} model to the simulated data 
and their 95\% confidence interval (CI) for the \textbf{Queen's contiguity} network; 
the variance for the random error is set to $\sigma^2 = 0.001$.} 
\label{tab:coef_testing_queen_001}
\end{table}
