# Supplementary material for: COVID-19 incidence in the Republic of Ireland: A case study for network-based time series models
Source: arXiv:2307.06199 source file (2024-06-05)
Supplement: Supplementary file 5 [file Add_GNAR_pandemic_phases.tex]

\clearpage
